# Supplementary material for: Overcoming the limitations of the MARTINI force field in Molecular Dynamics simulations of polysaccharides
Source: arXiv:1704.03773 ancillary file (2017-06-27)

beads: 1 2 4

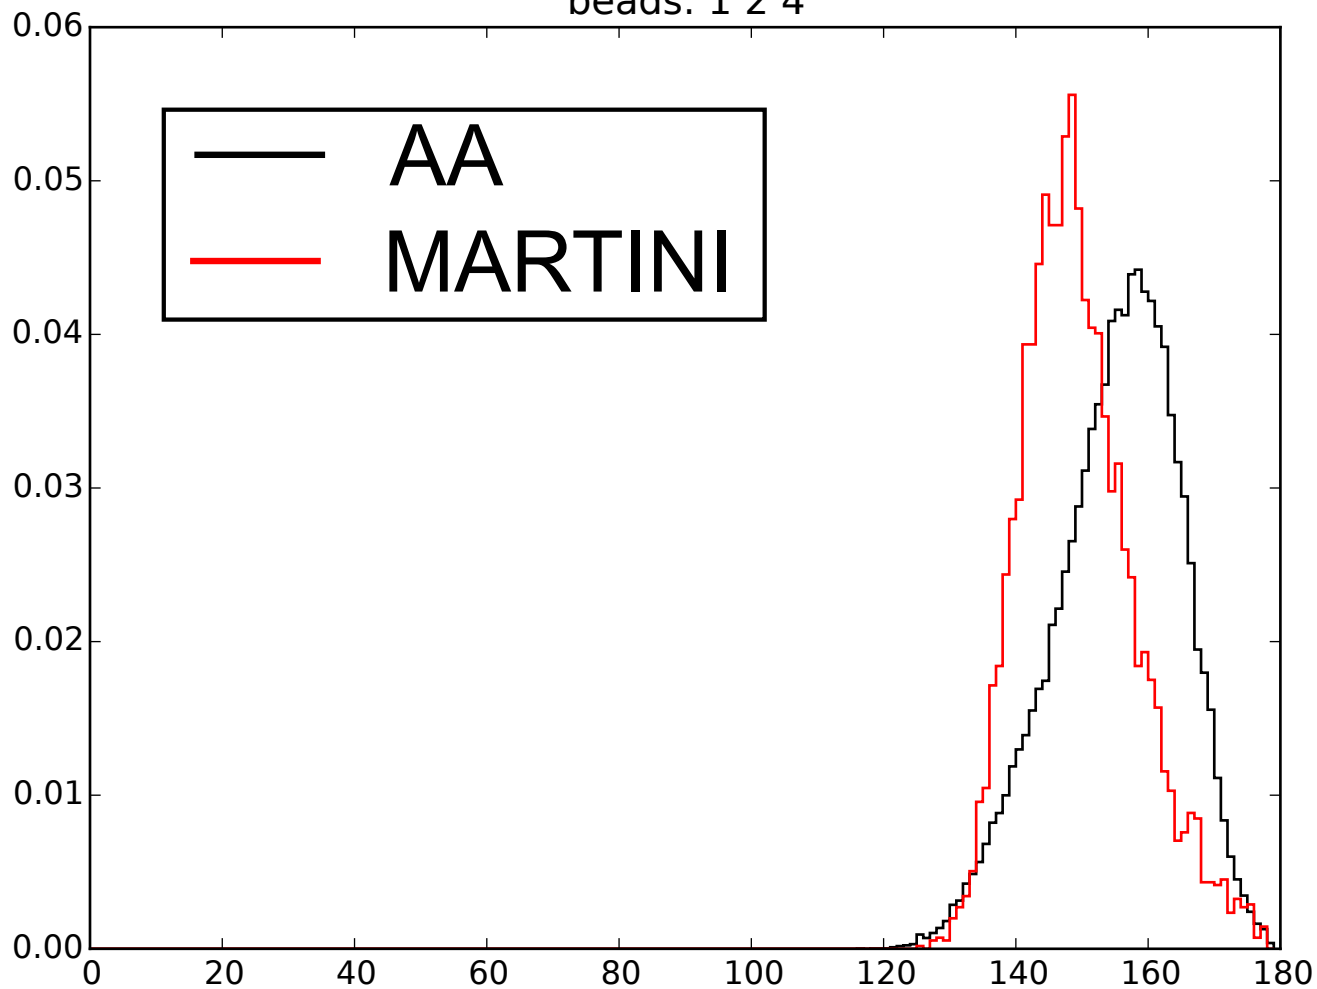

beads: 2 3 5

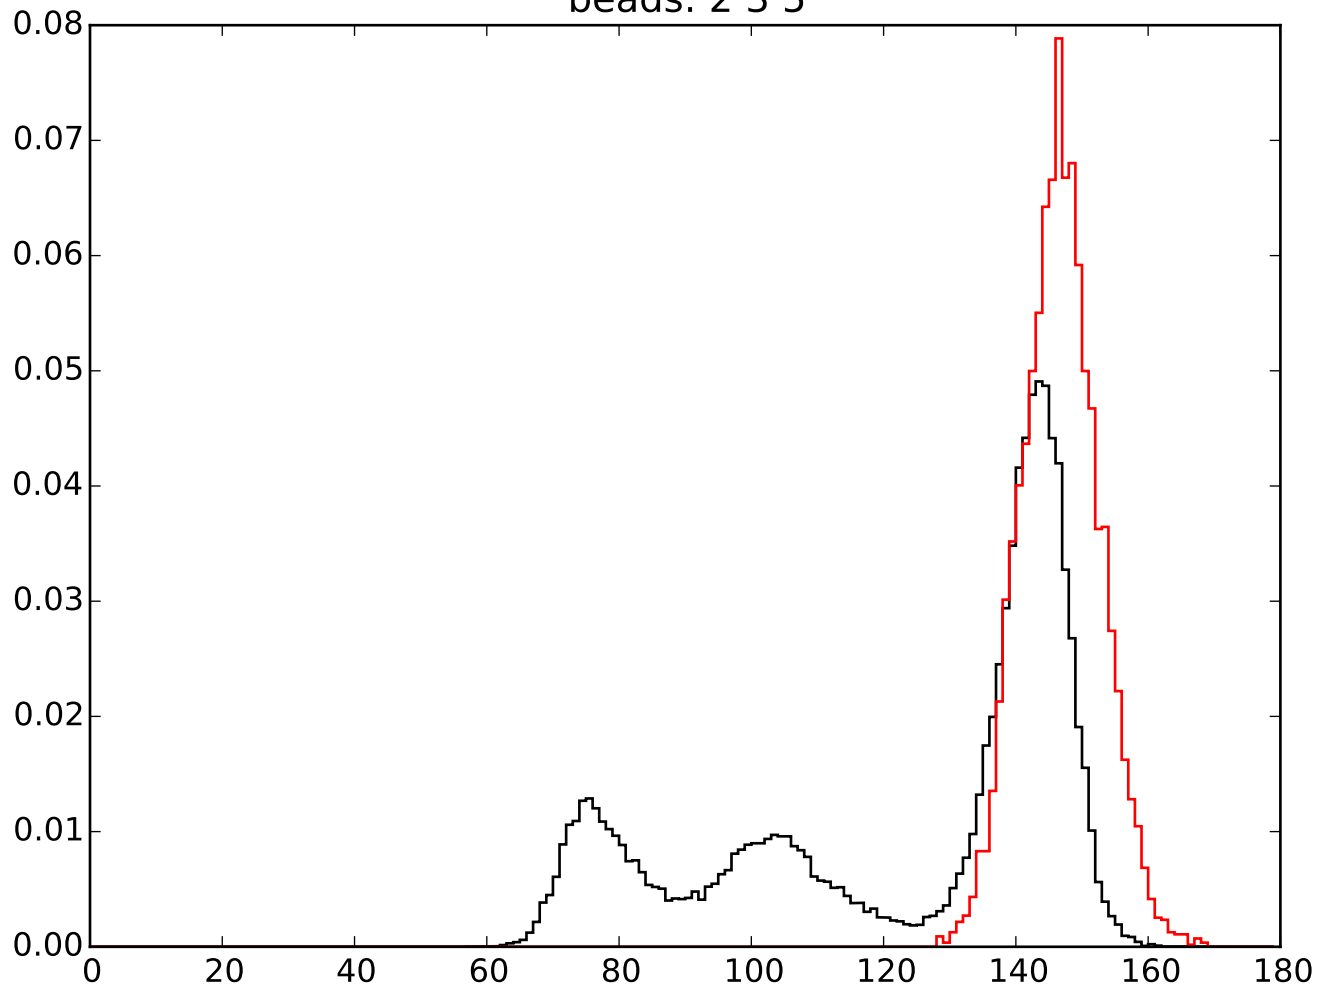

beads: 3 5 6

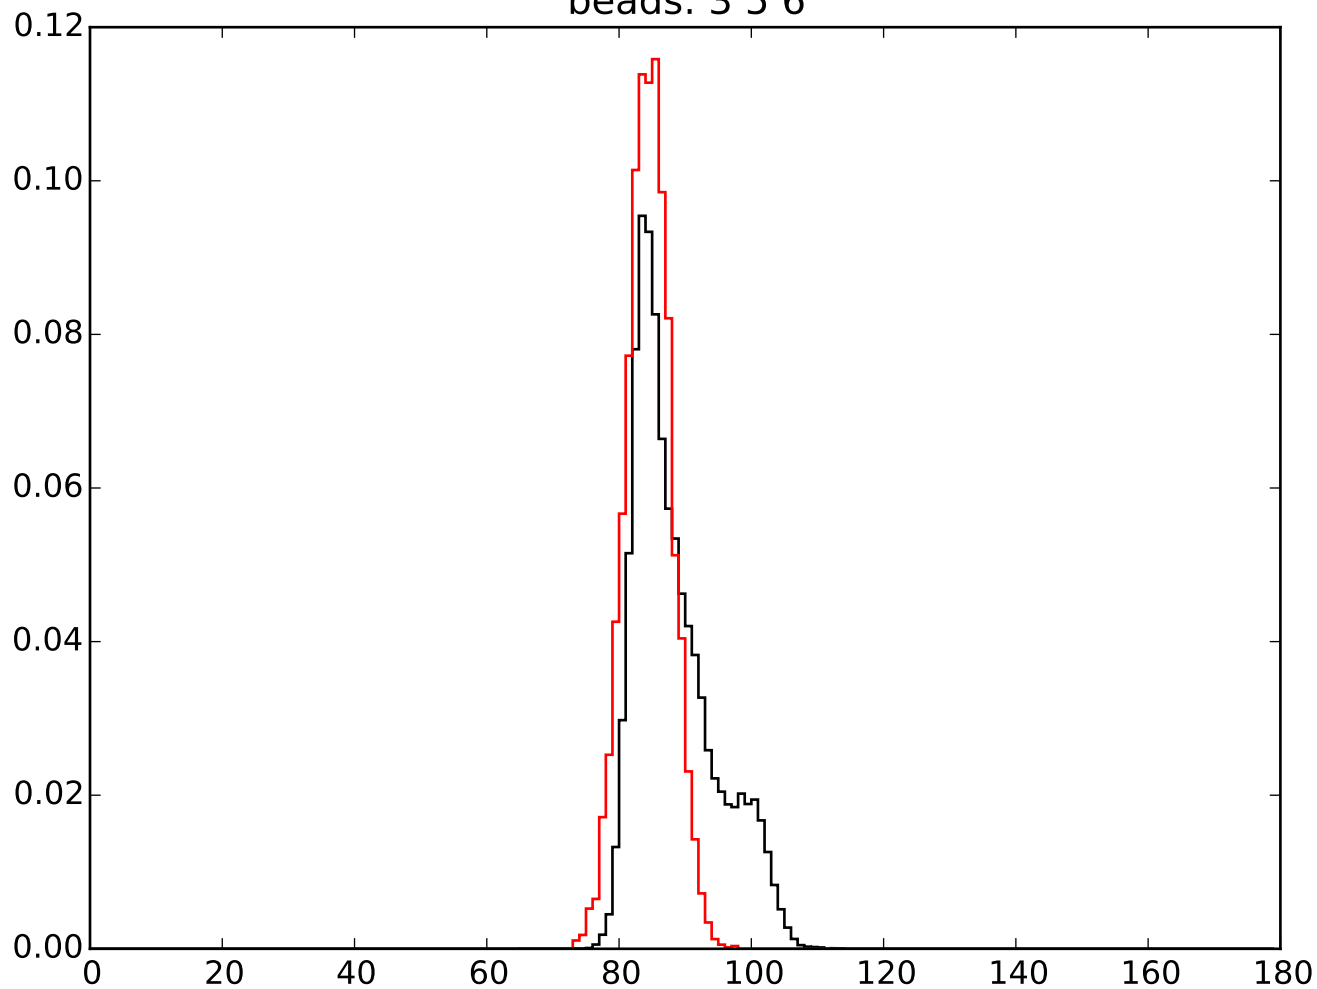

beads: 1 2 3

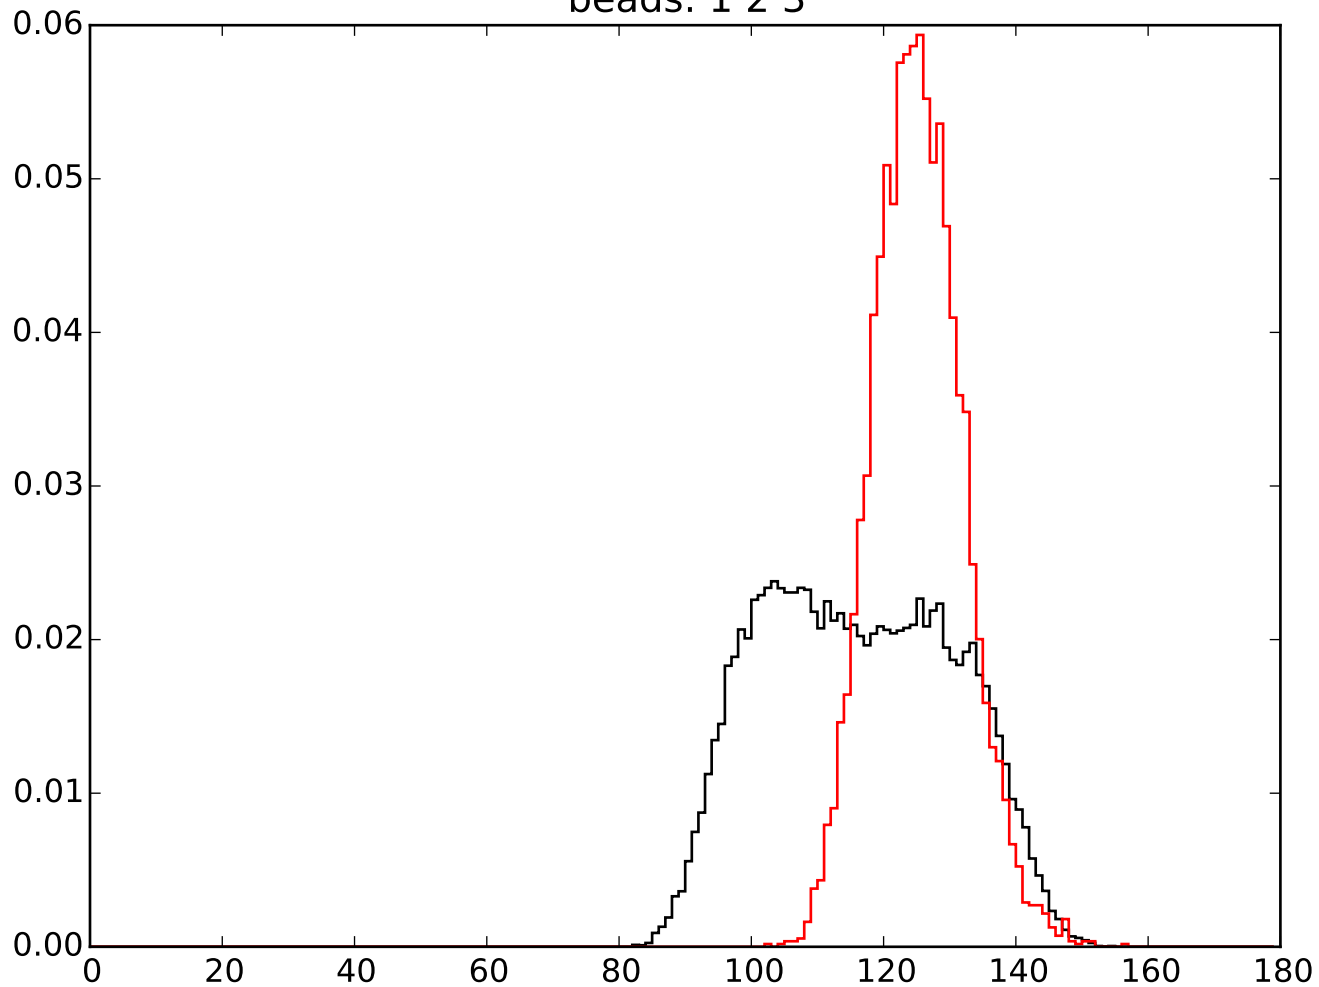

beads: 3 5 7

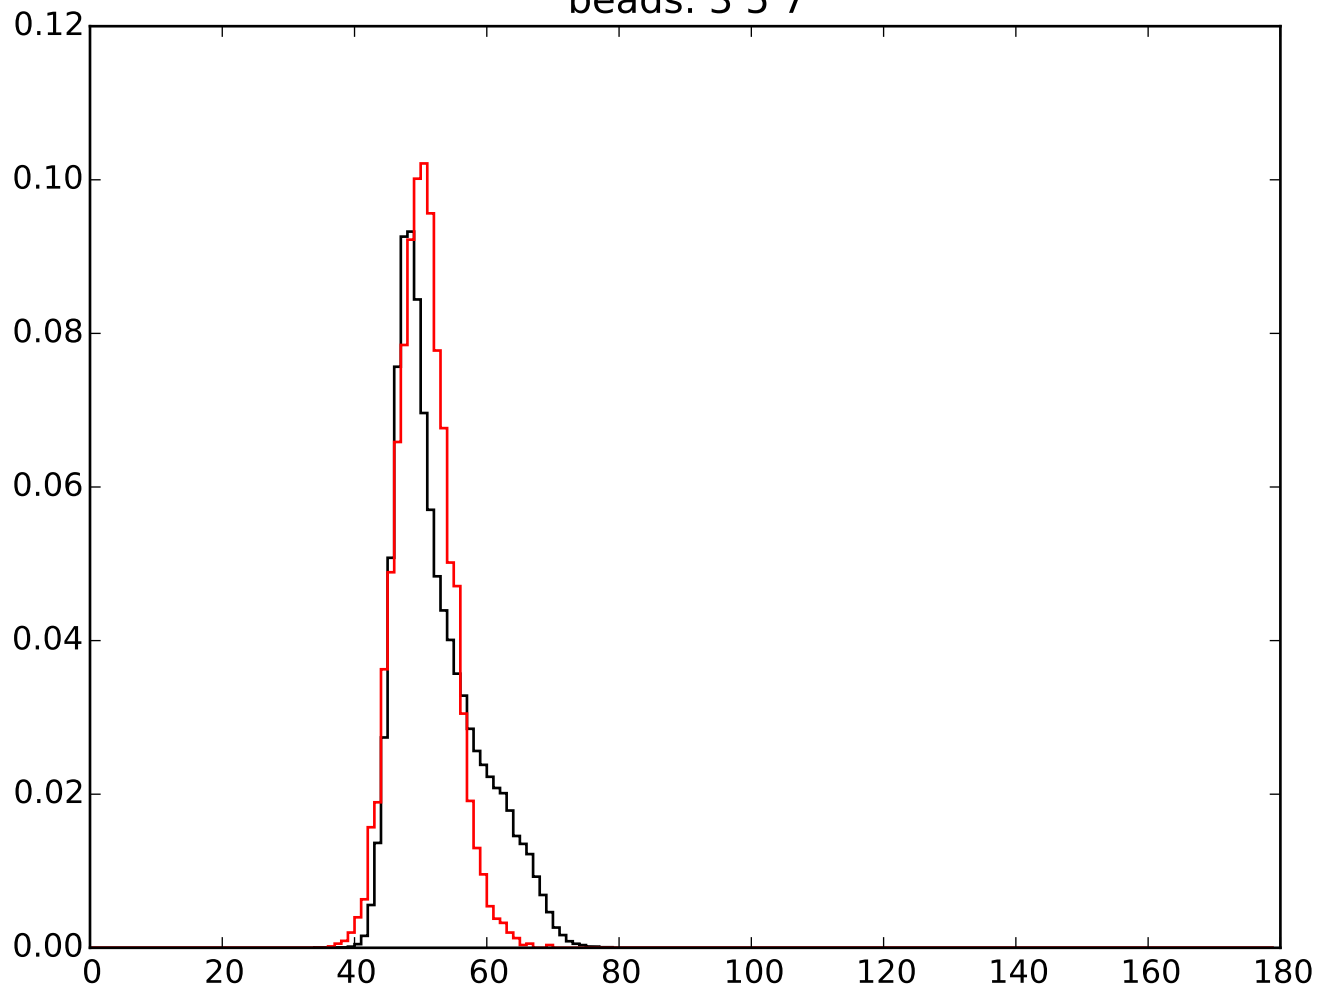

beads: 4 3 5

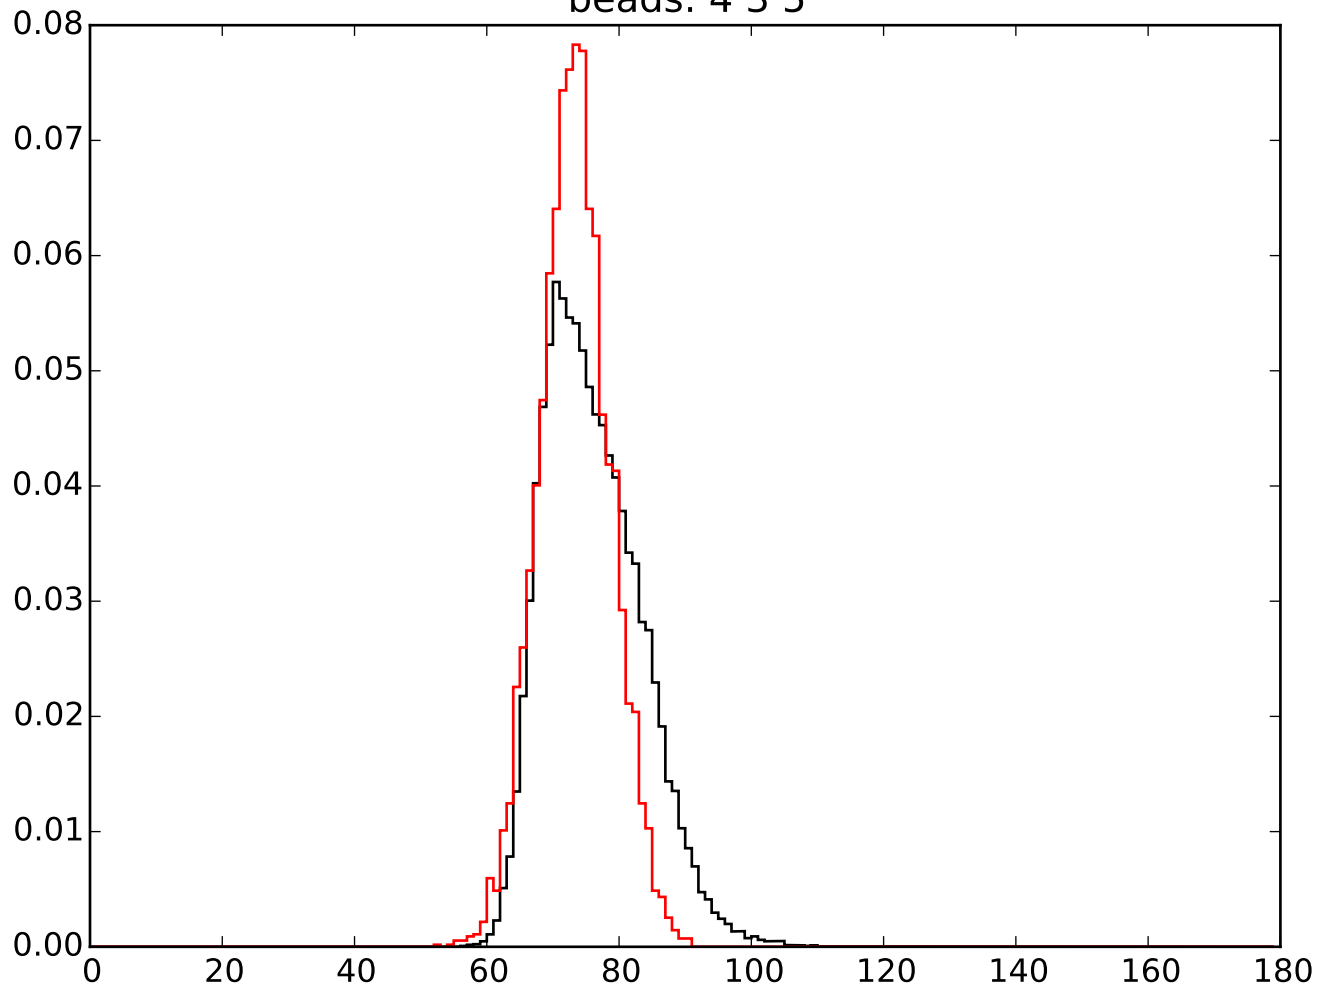

beads: 5 6 8

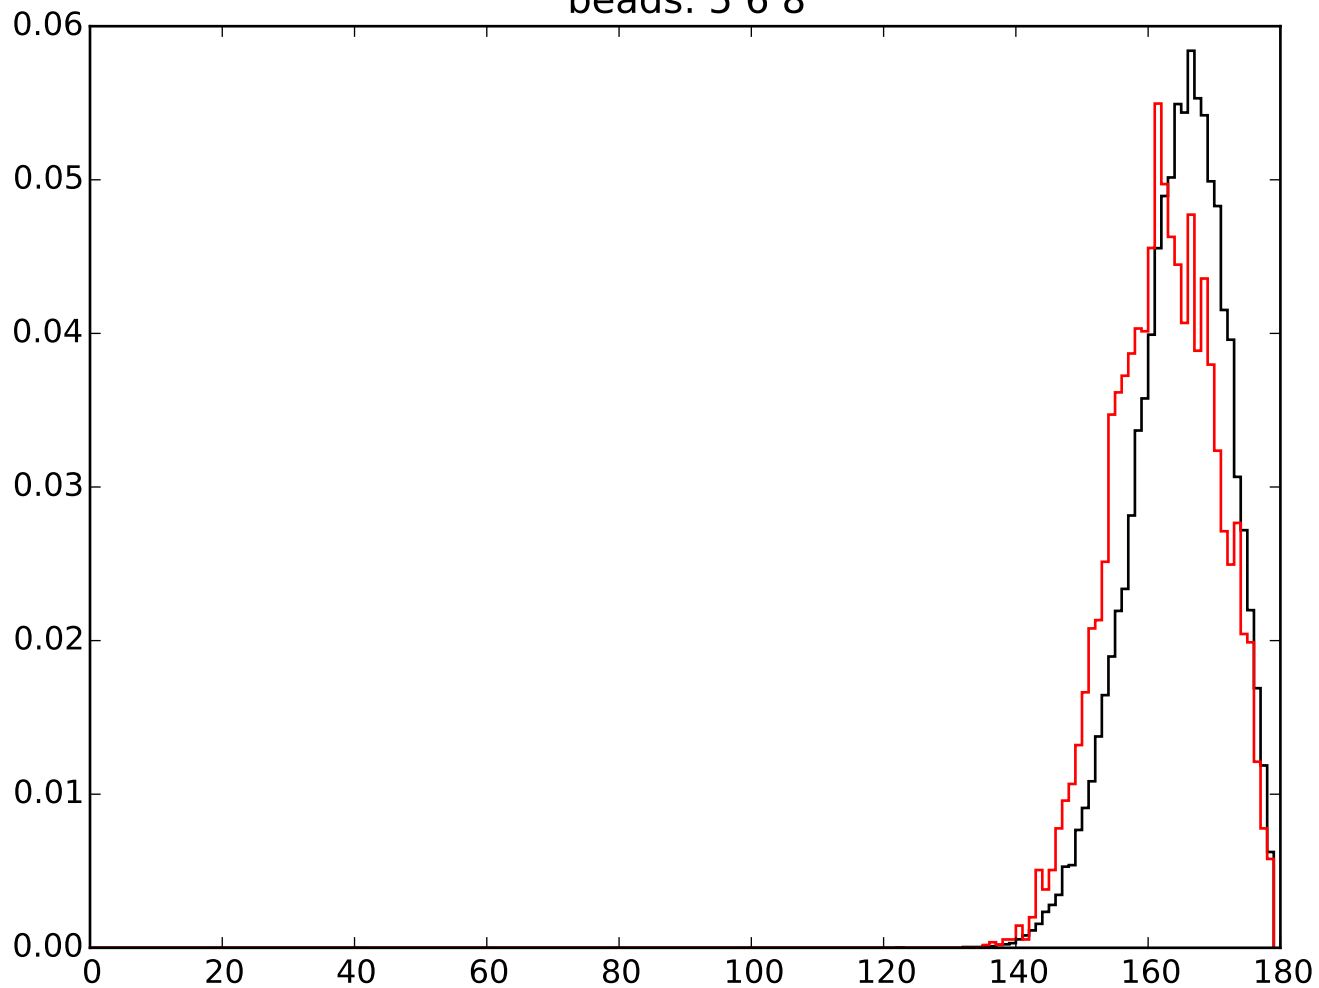

beads: 6 8 9

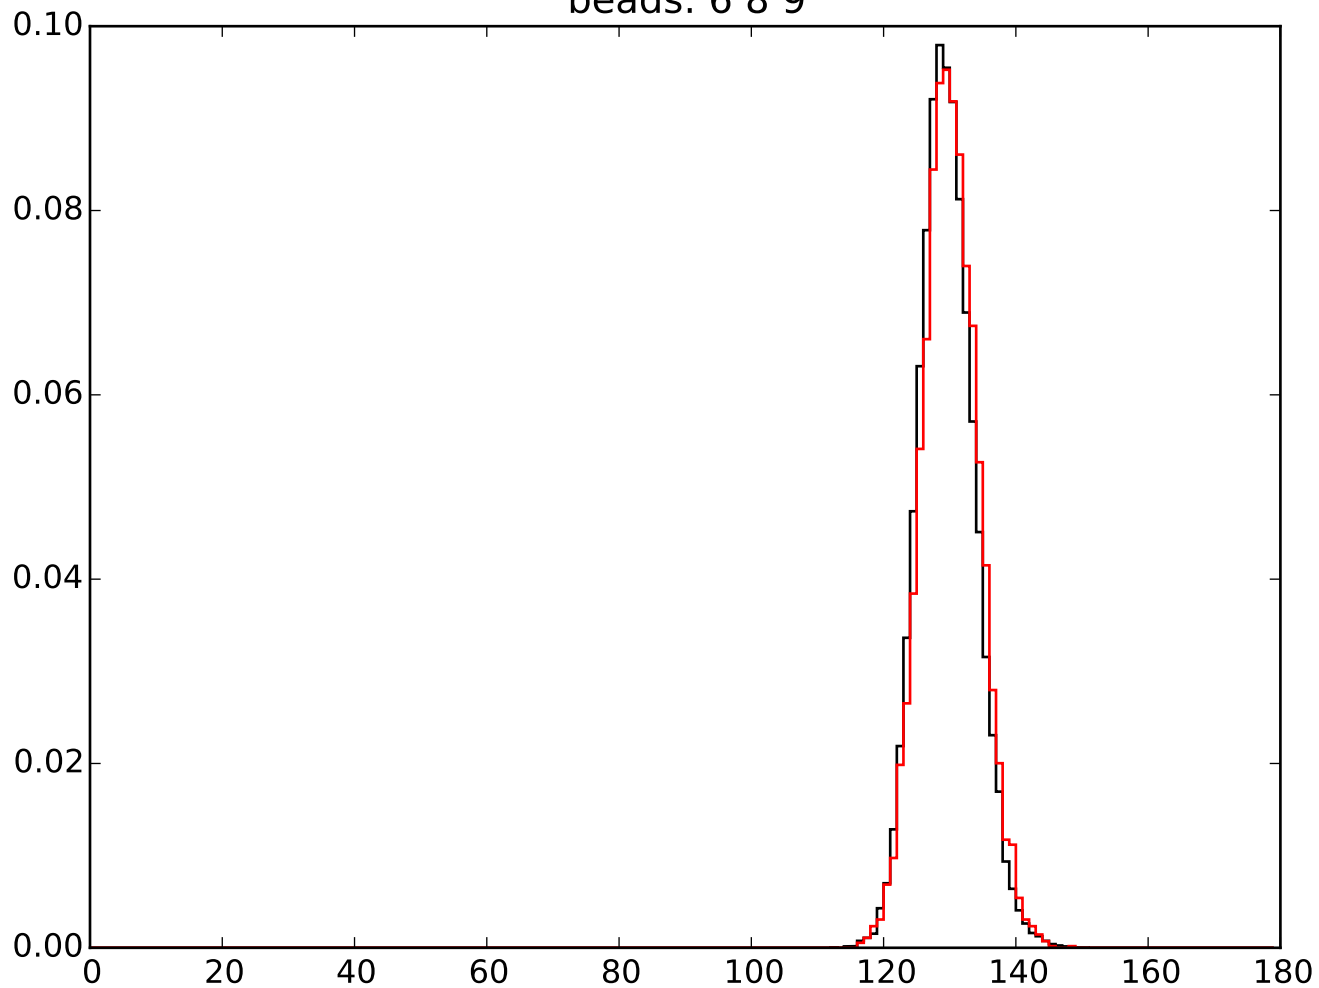



beads: 6 8 10

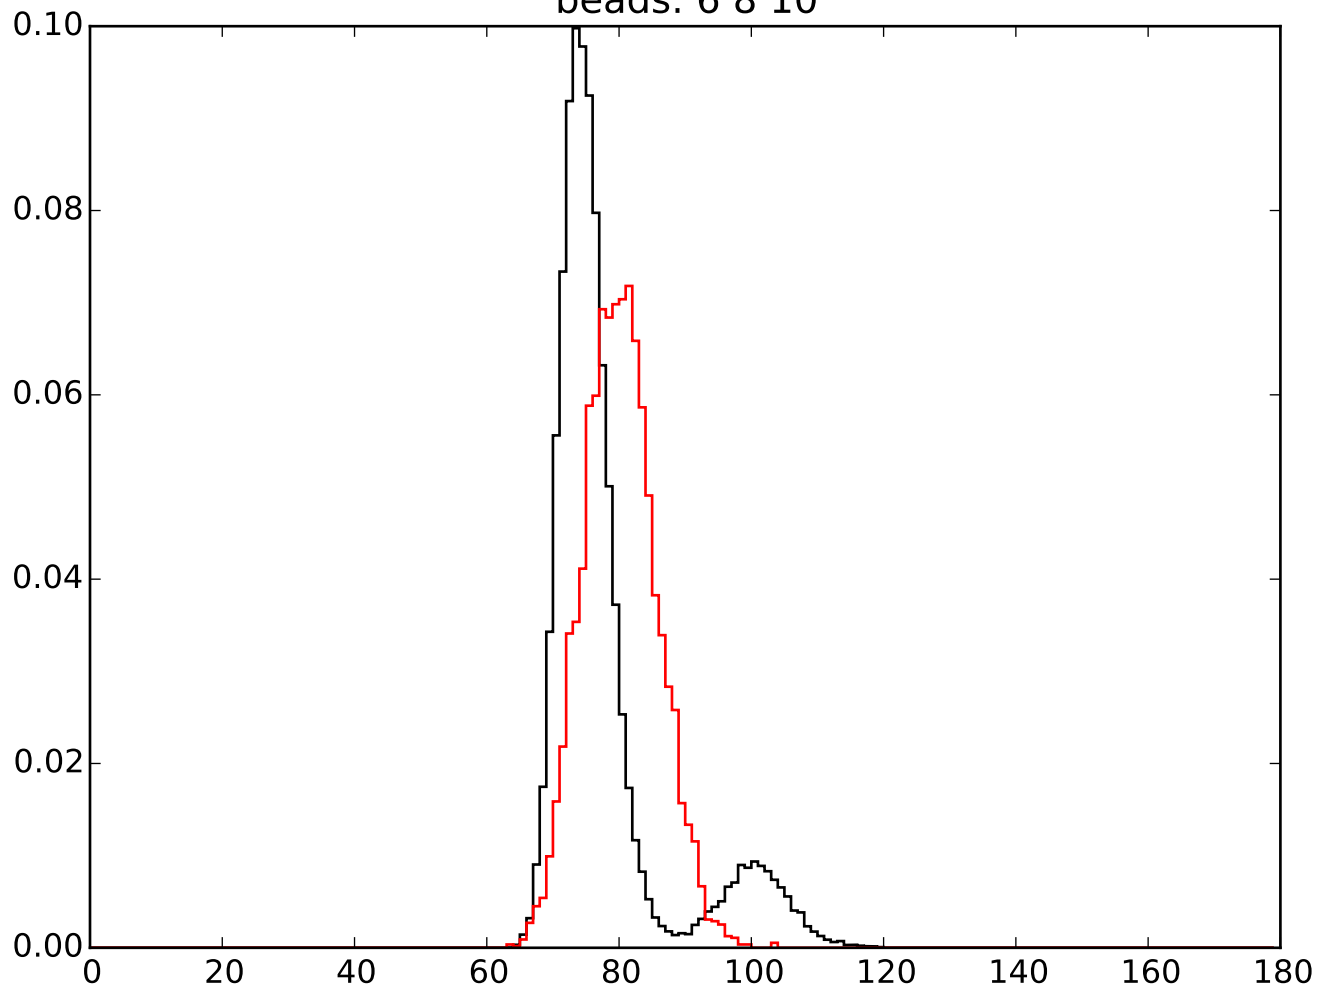

beads: 7 6 8

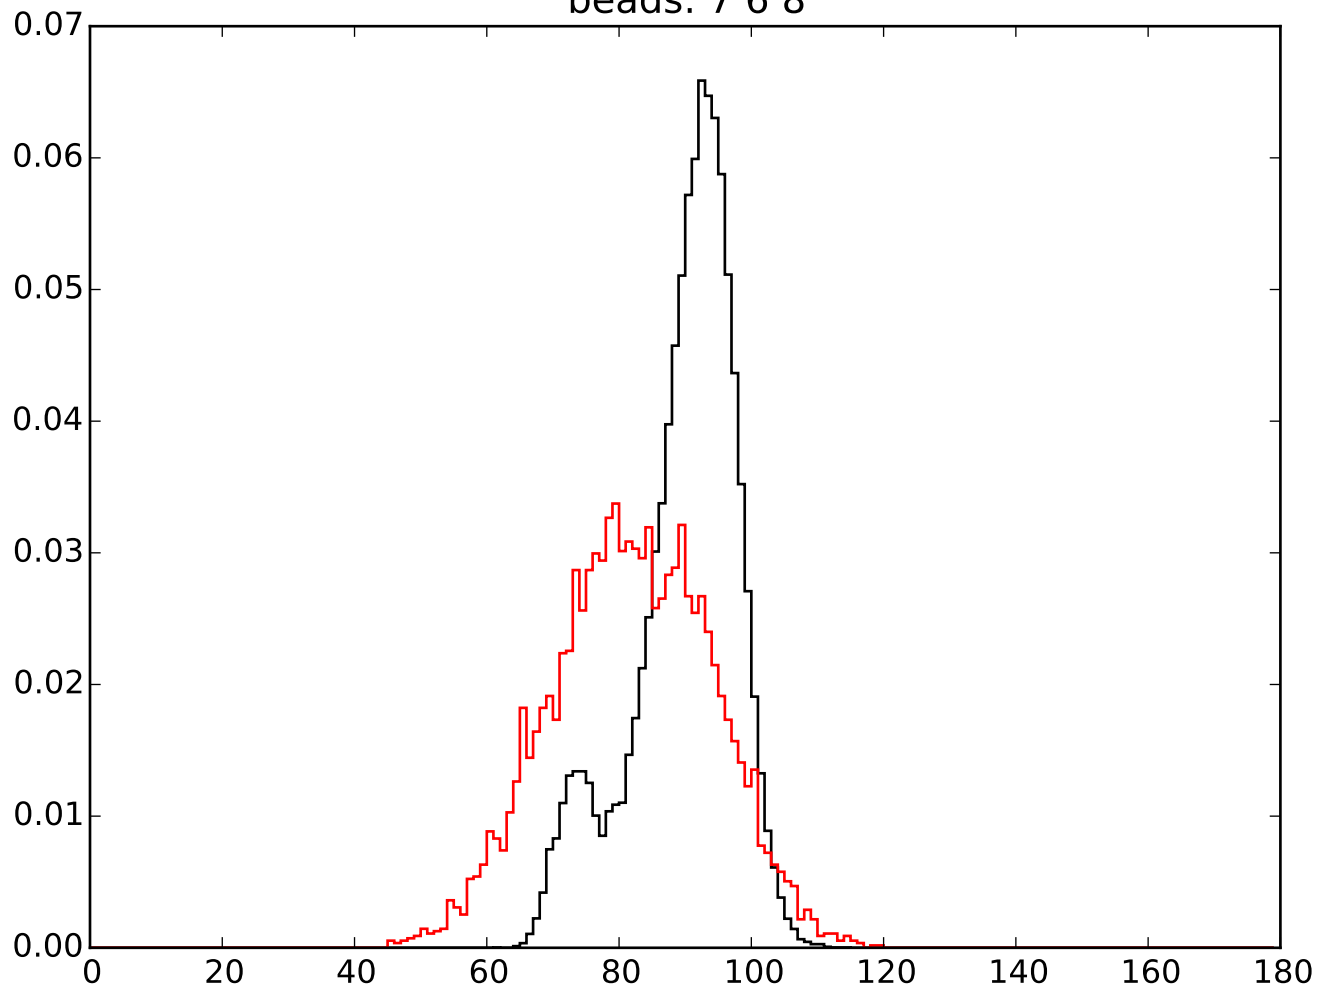

beads: 8 9 11

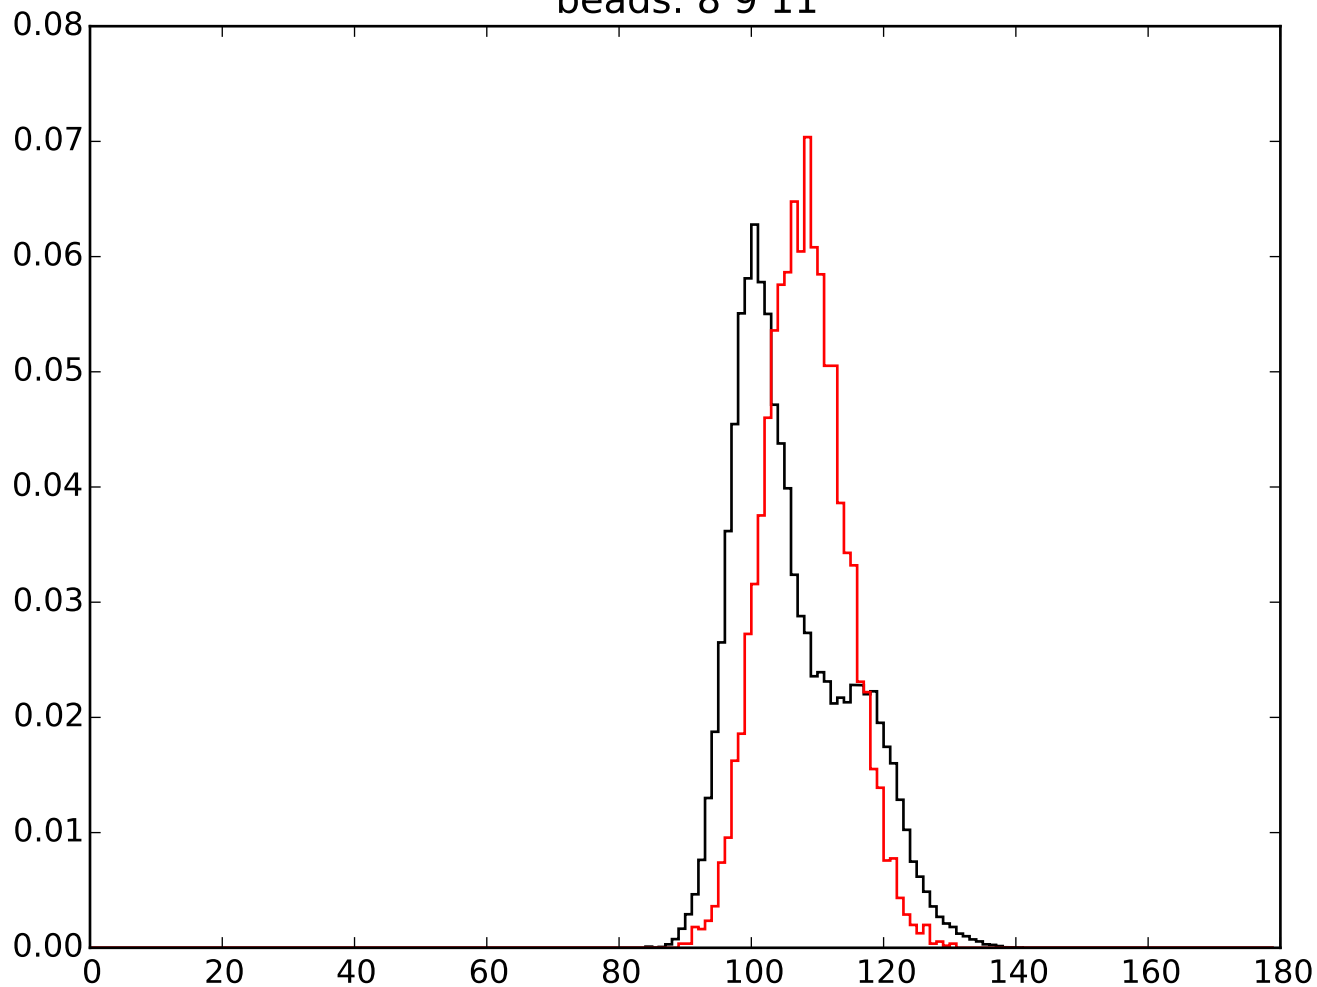

beads: 8 10 14

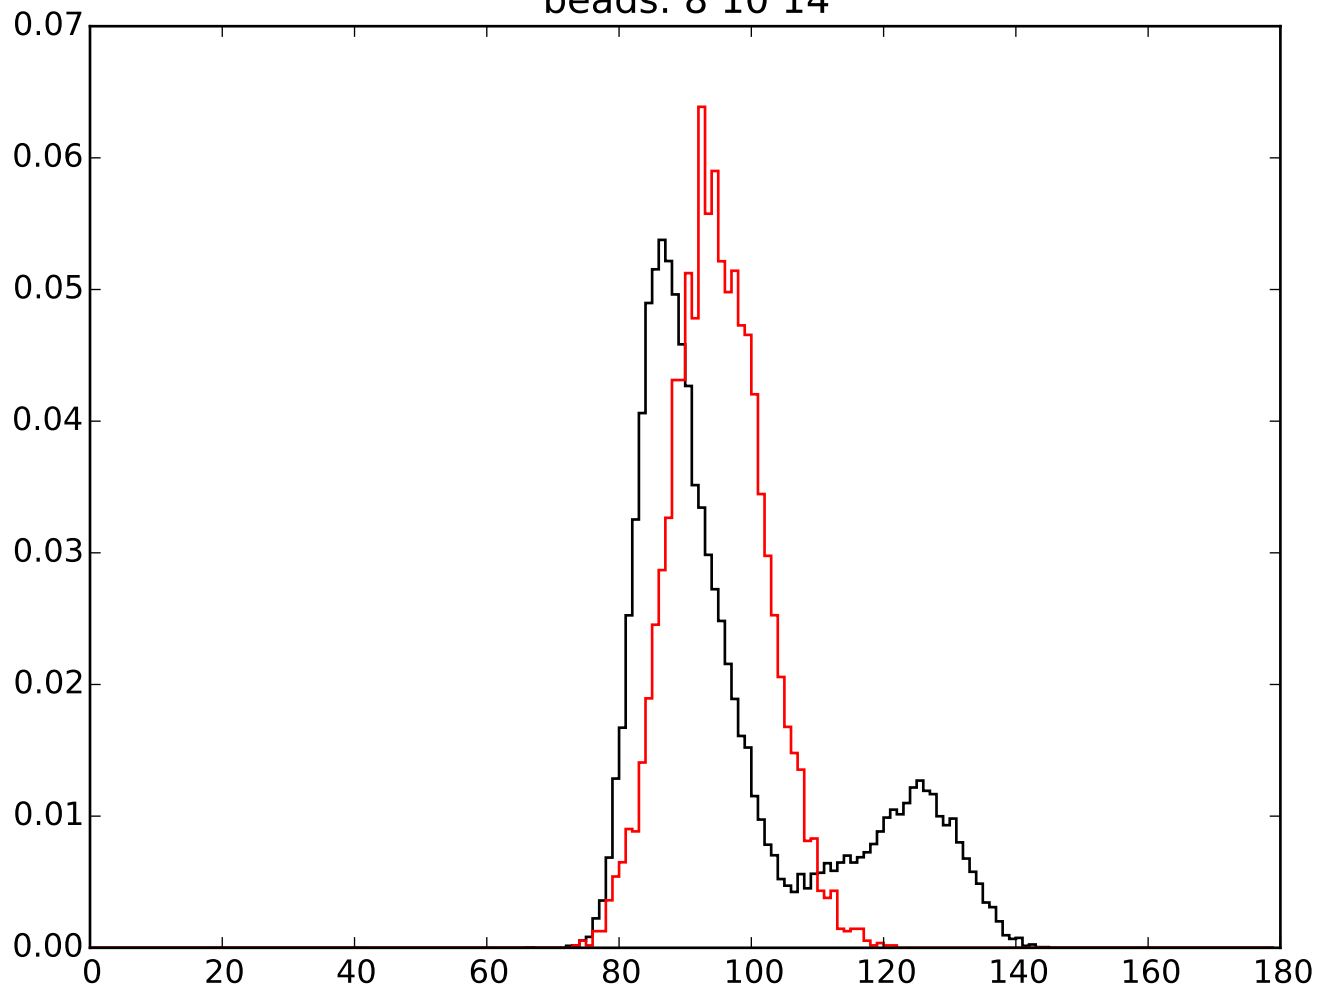

beads: 9 10 14

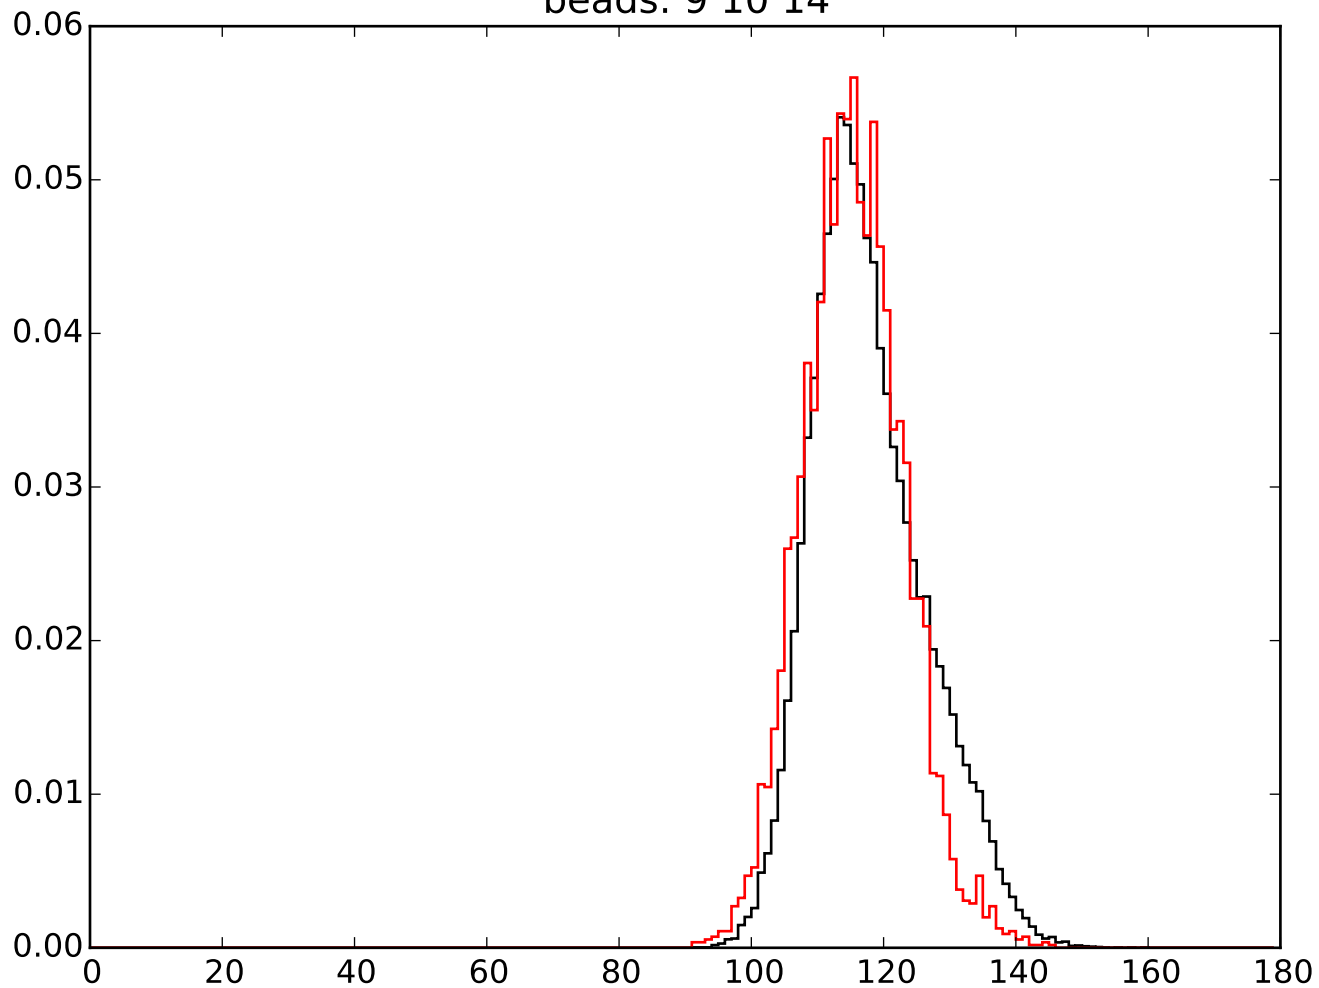

beads: 9 11 12

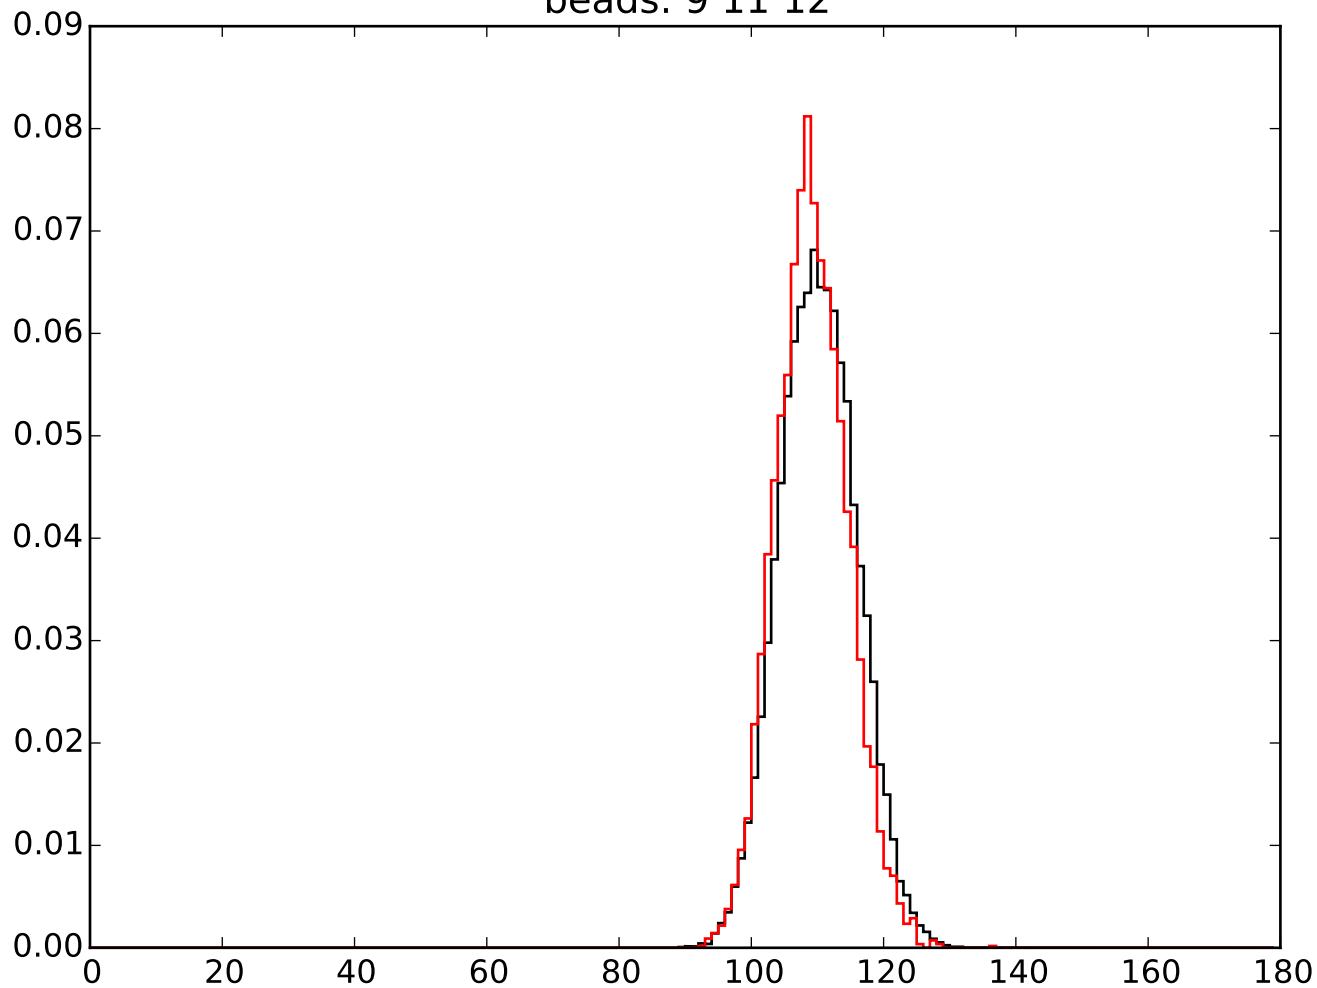

beads: 9 11 13

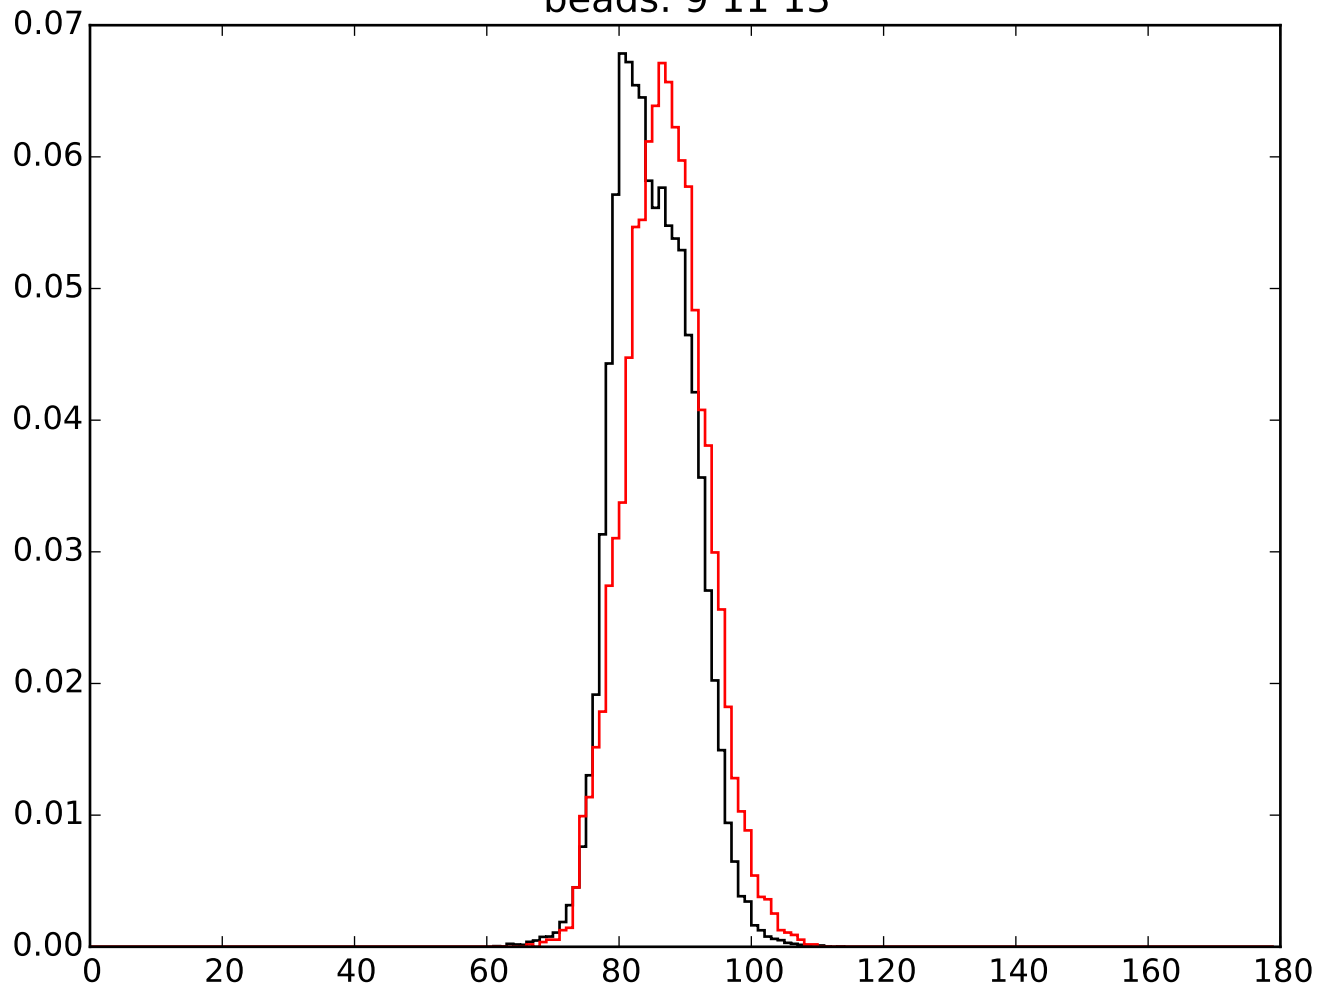

beads: 9 11 17

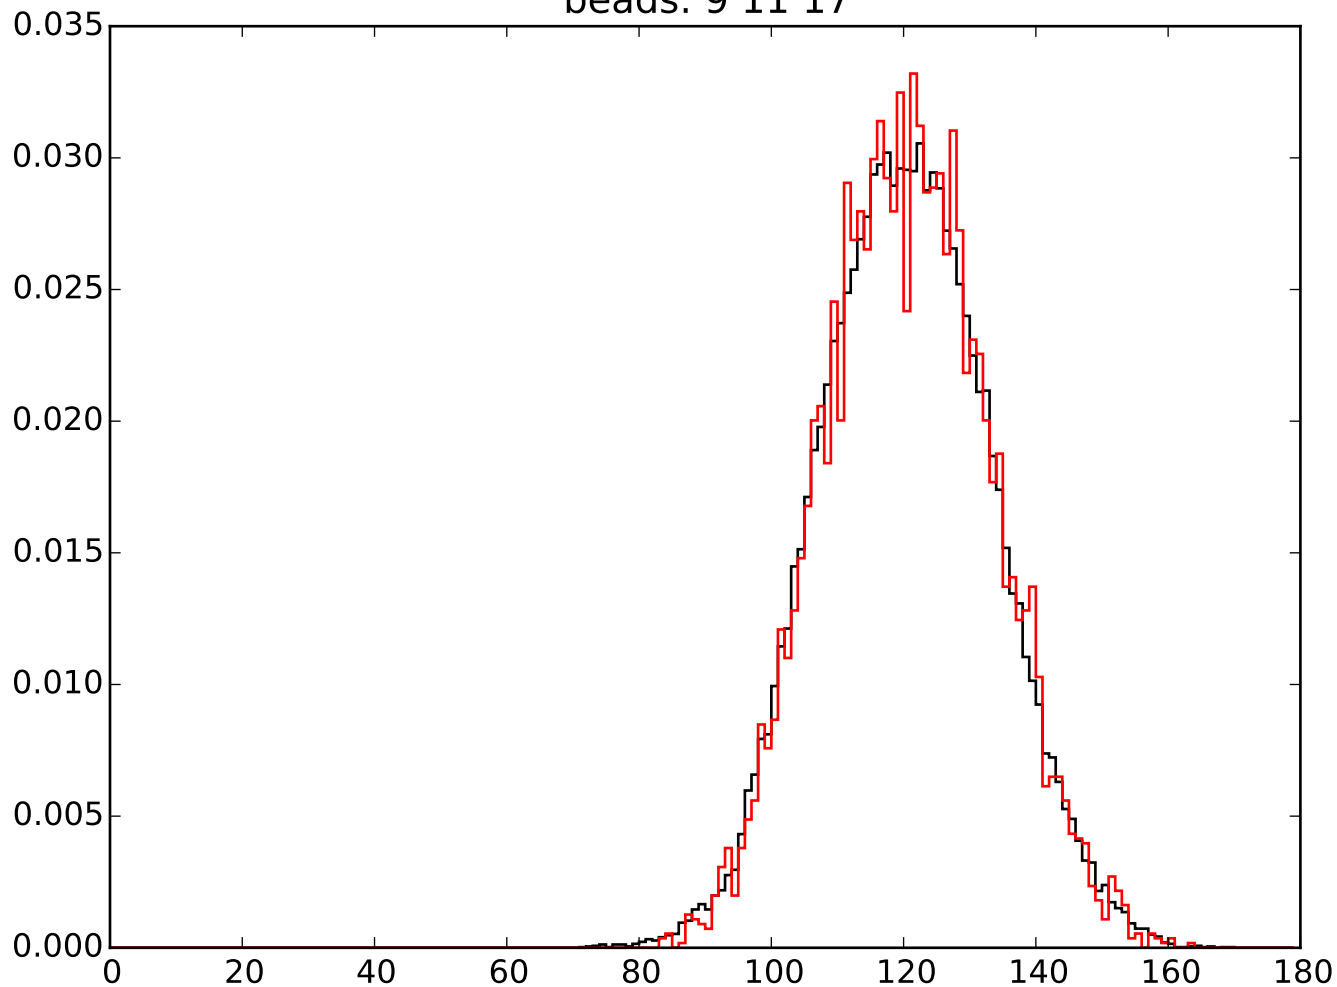



beads: 10 9 11

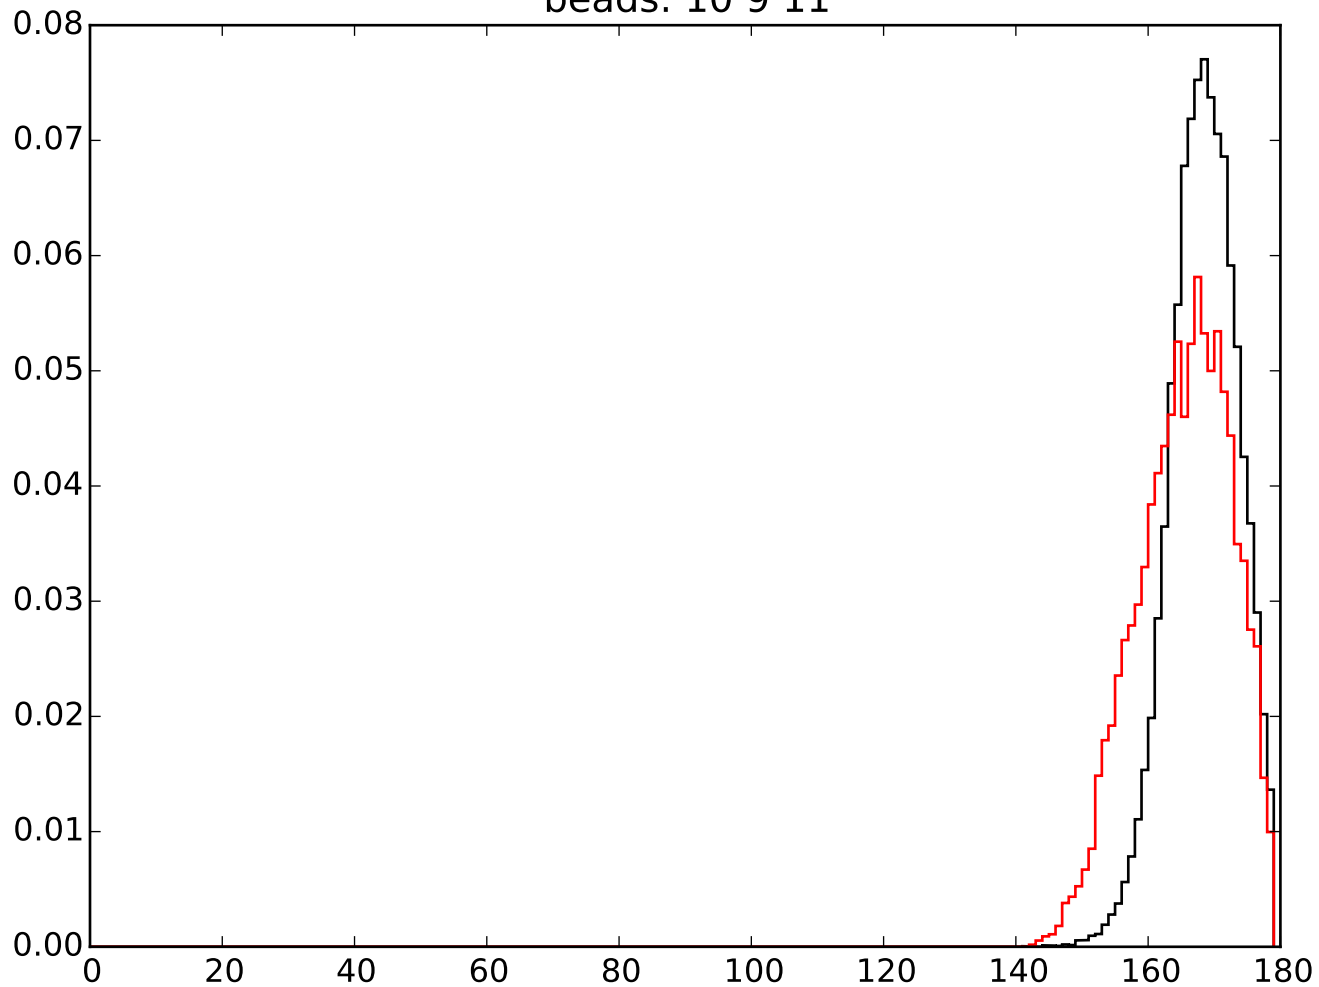

beads: 10 14 15

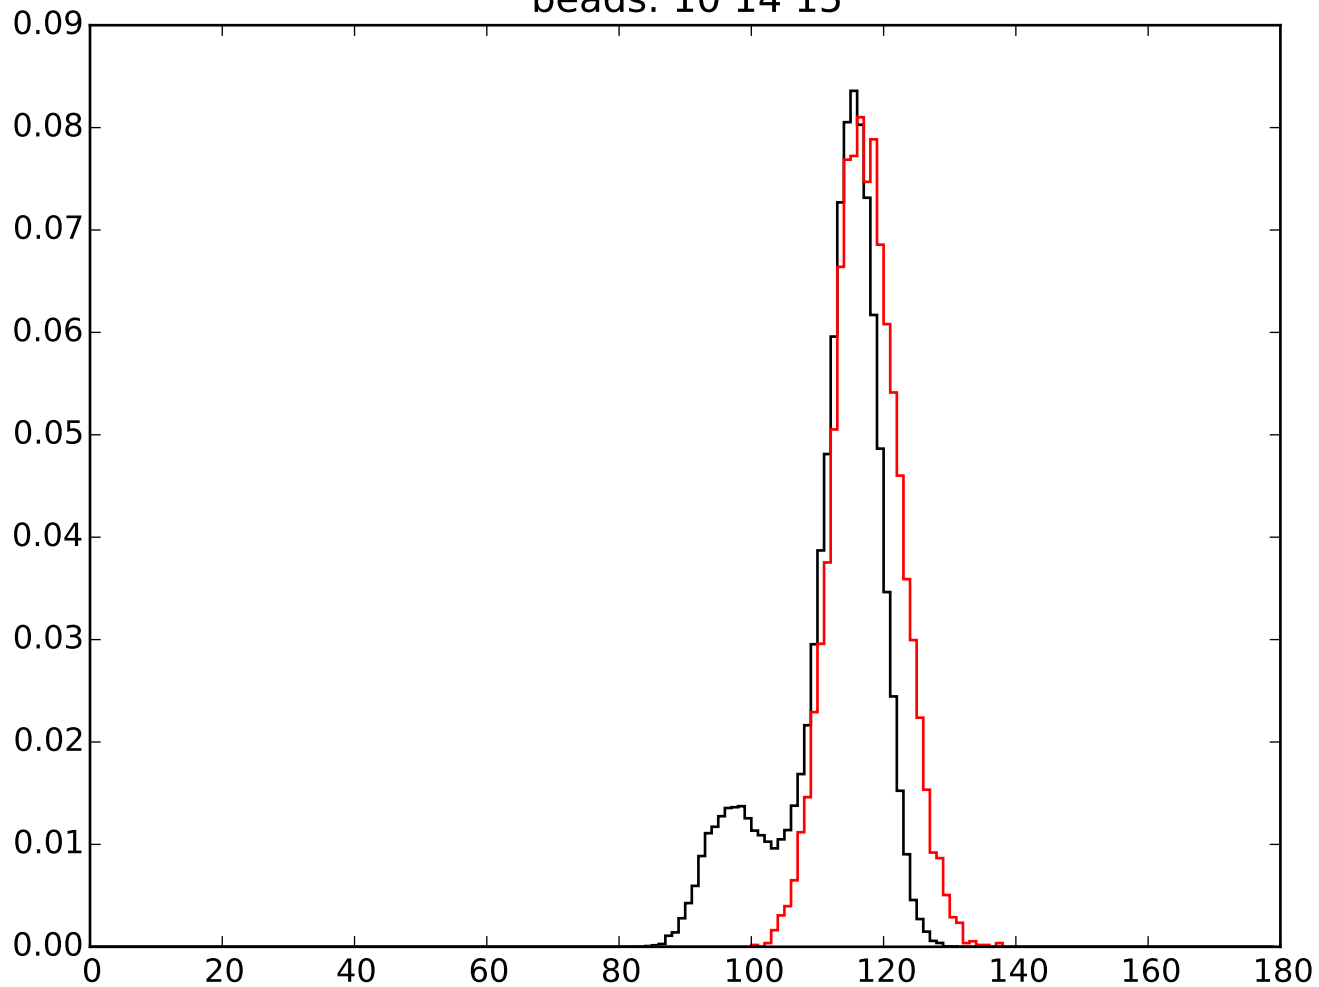

beads: 10 14 16

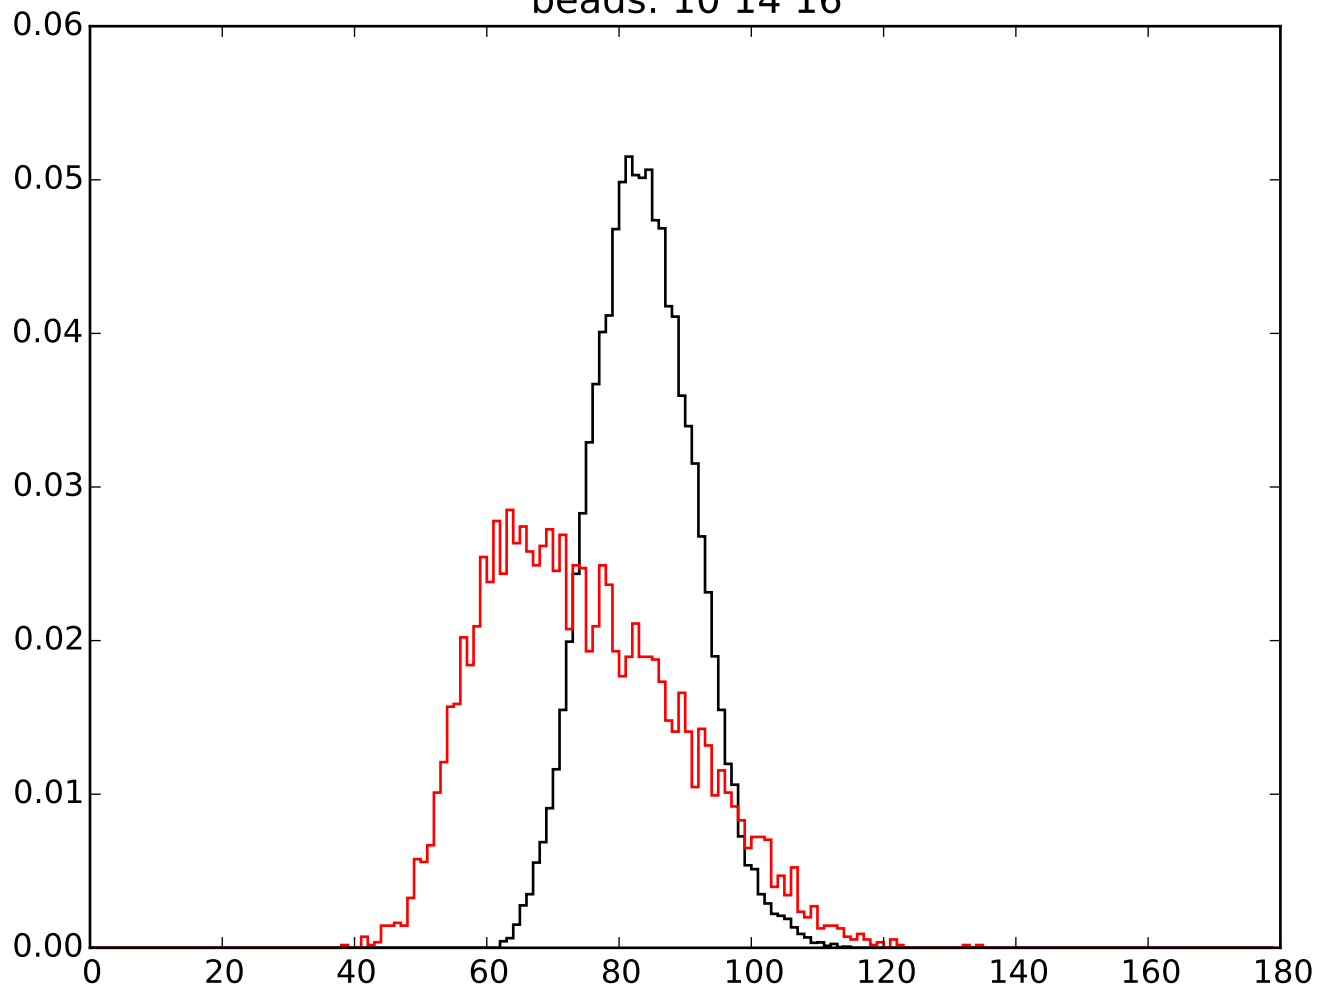

beads: 10 14 28

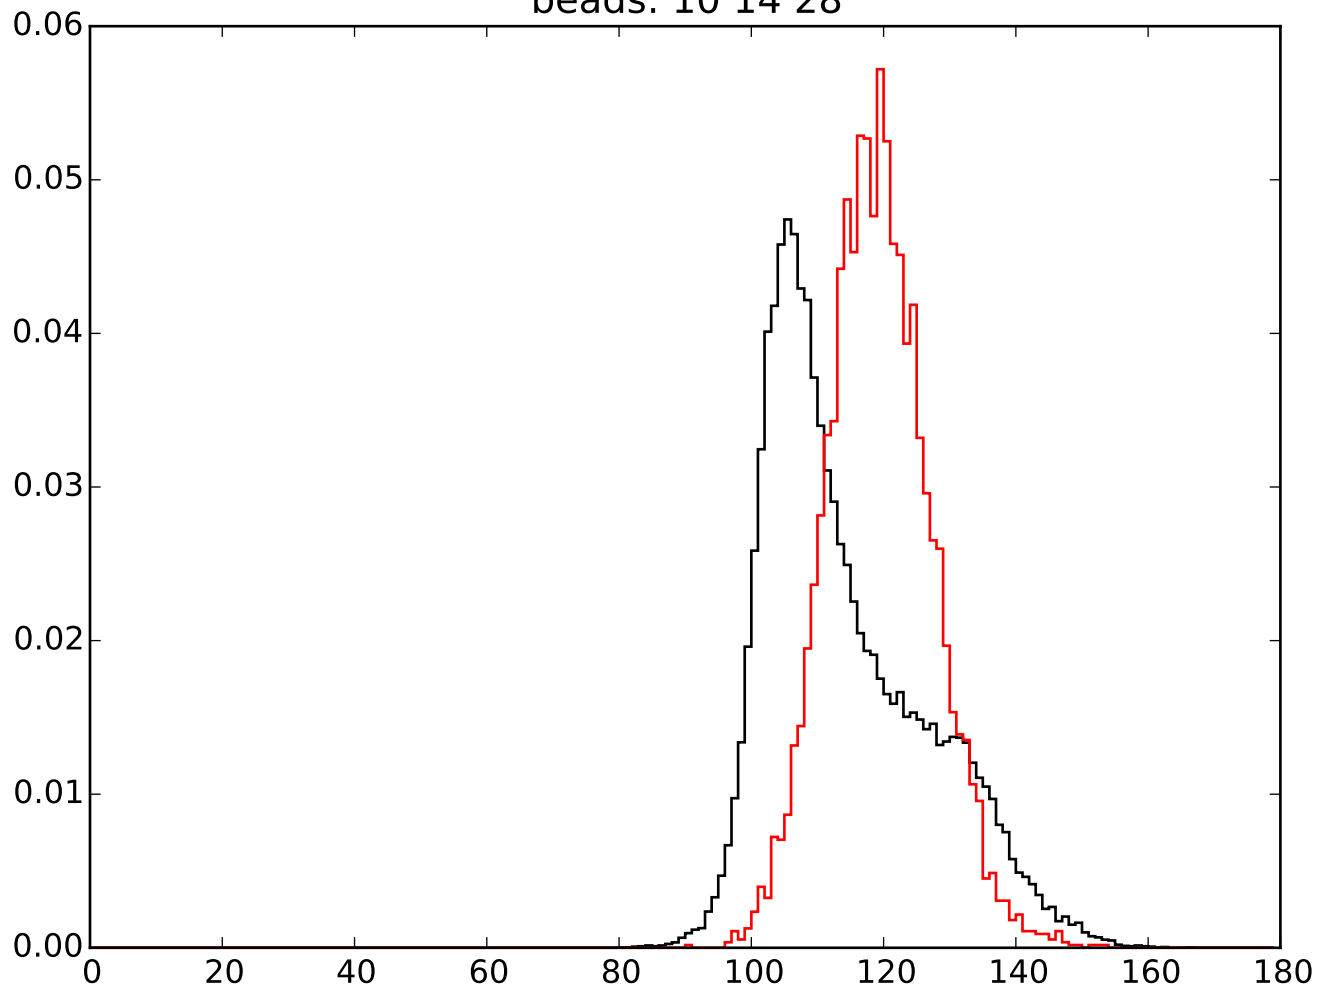

beads: 11 17 18

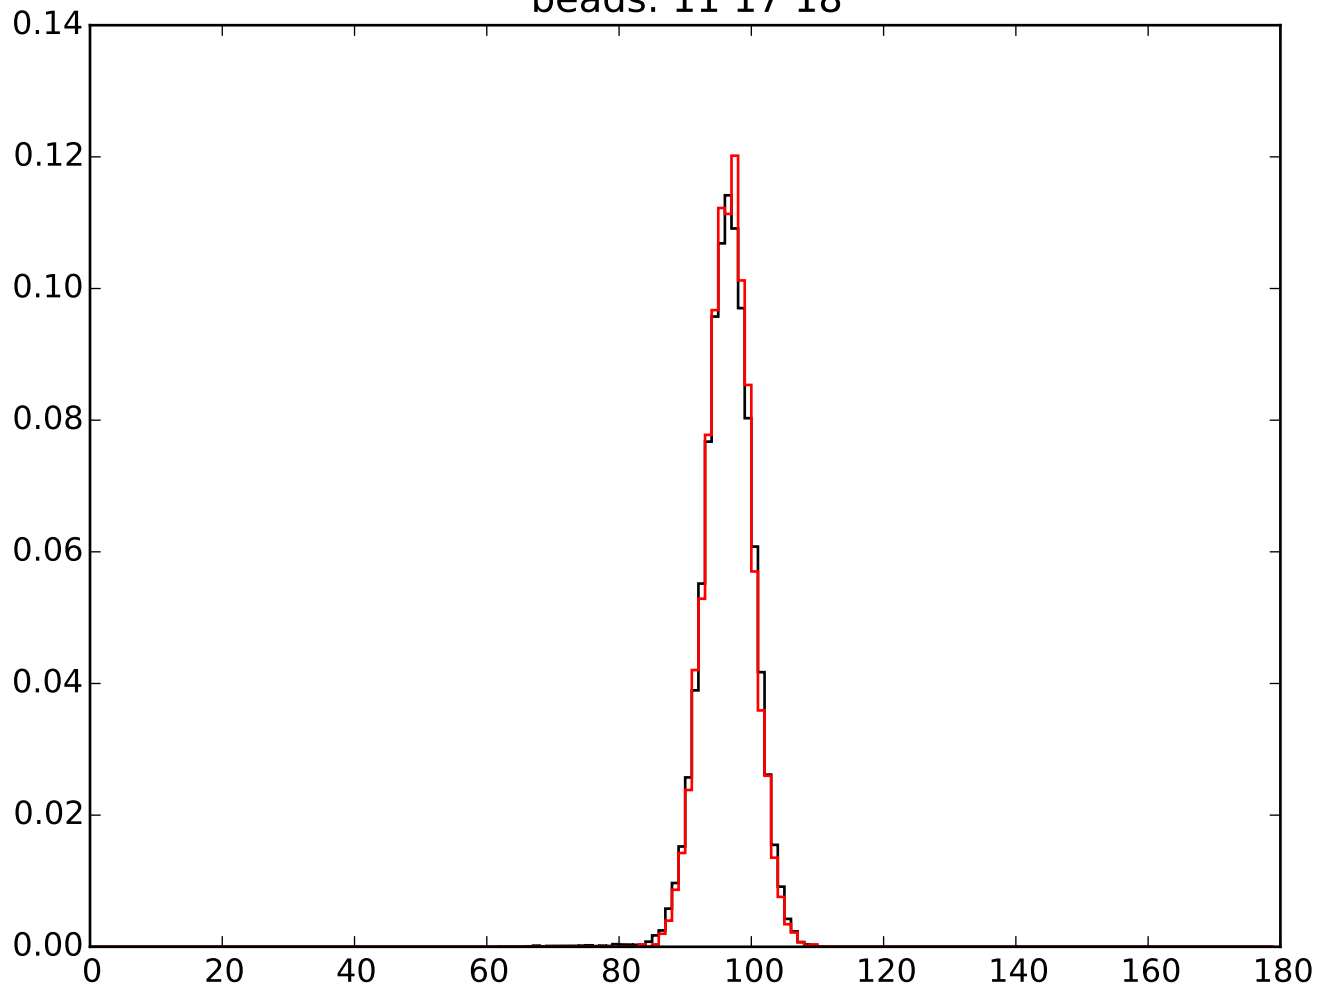

beads: 11 17 19

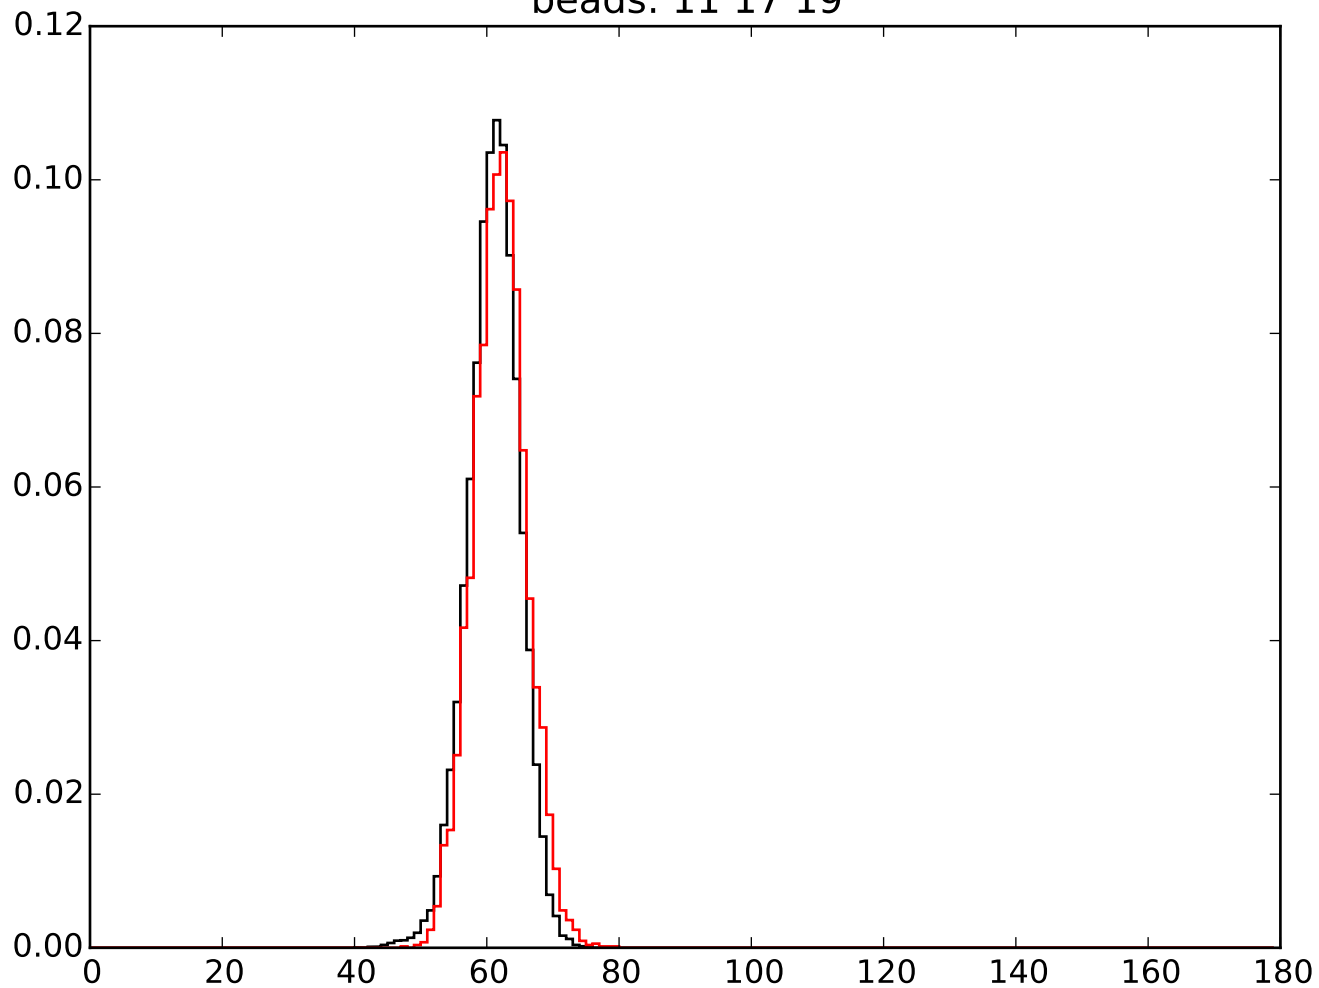

beads: 13 11 17

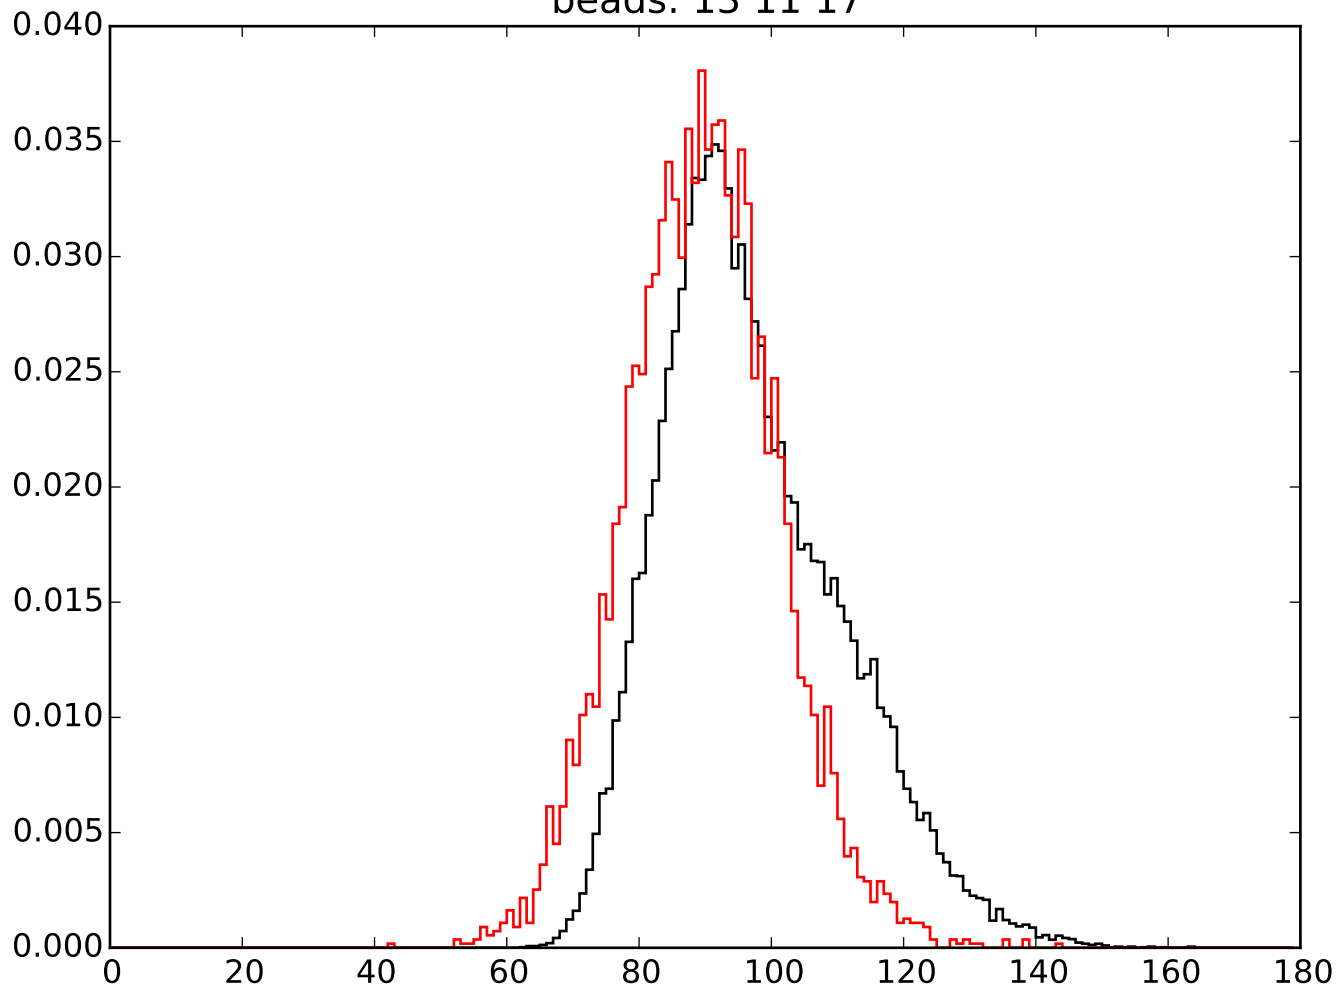

beads: 14 28 29

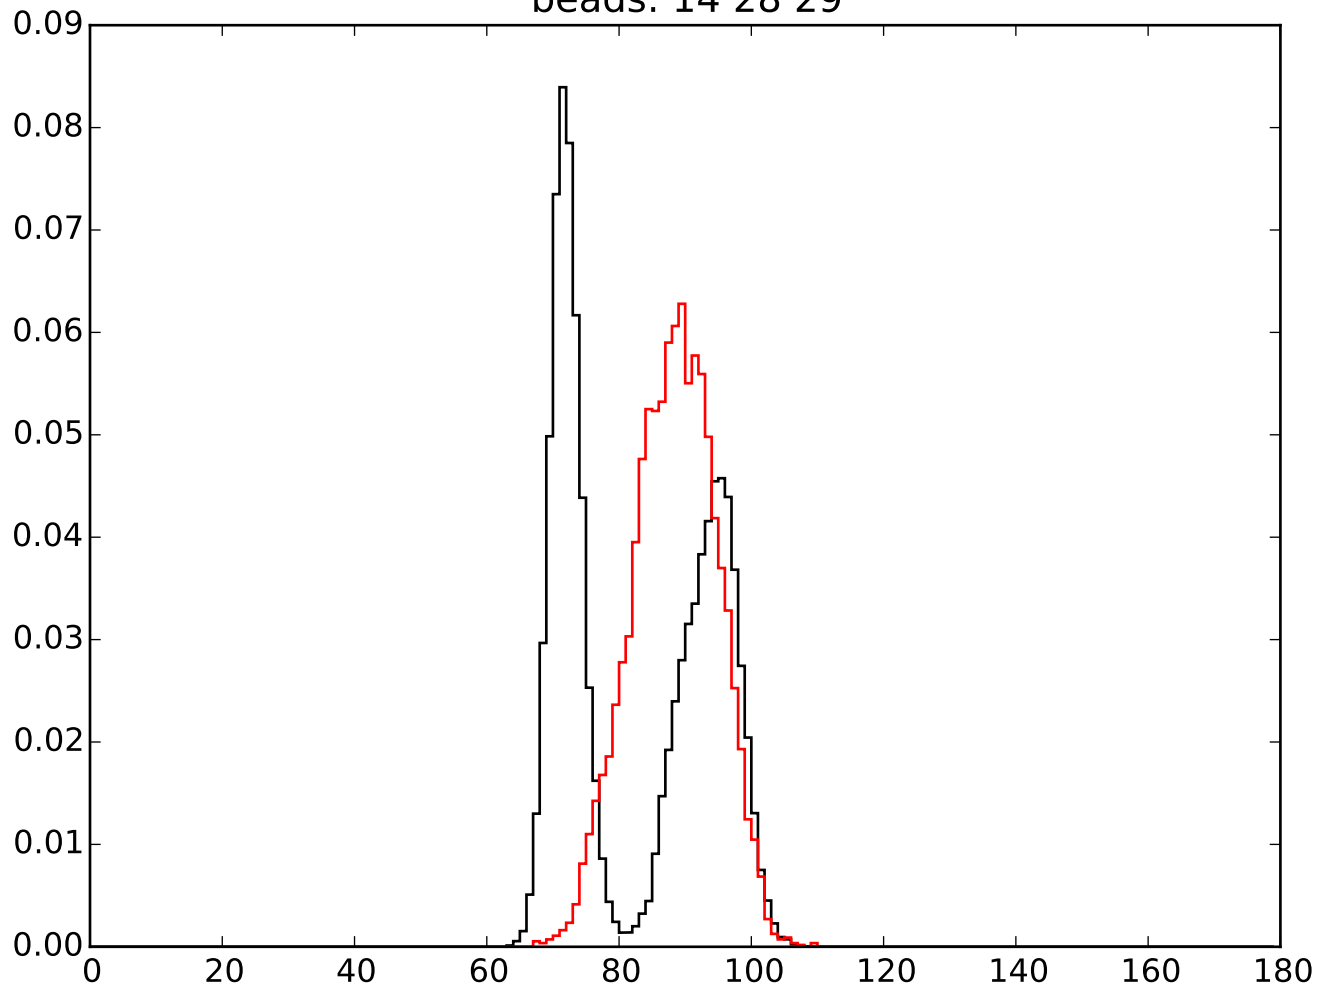



beads: 14 28 30

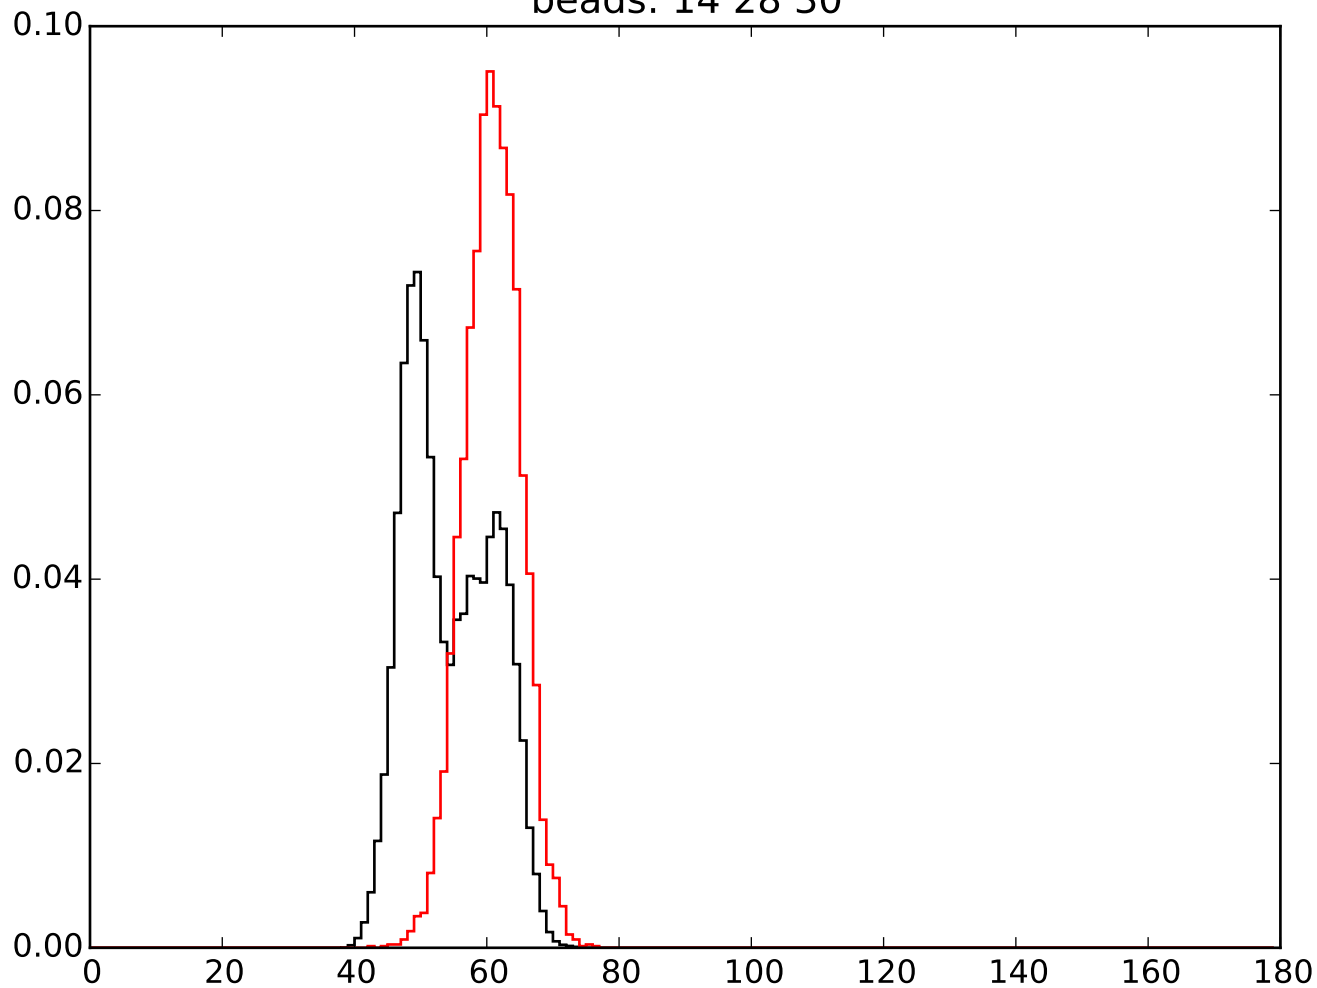

beads: 17 18 20

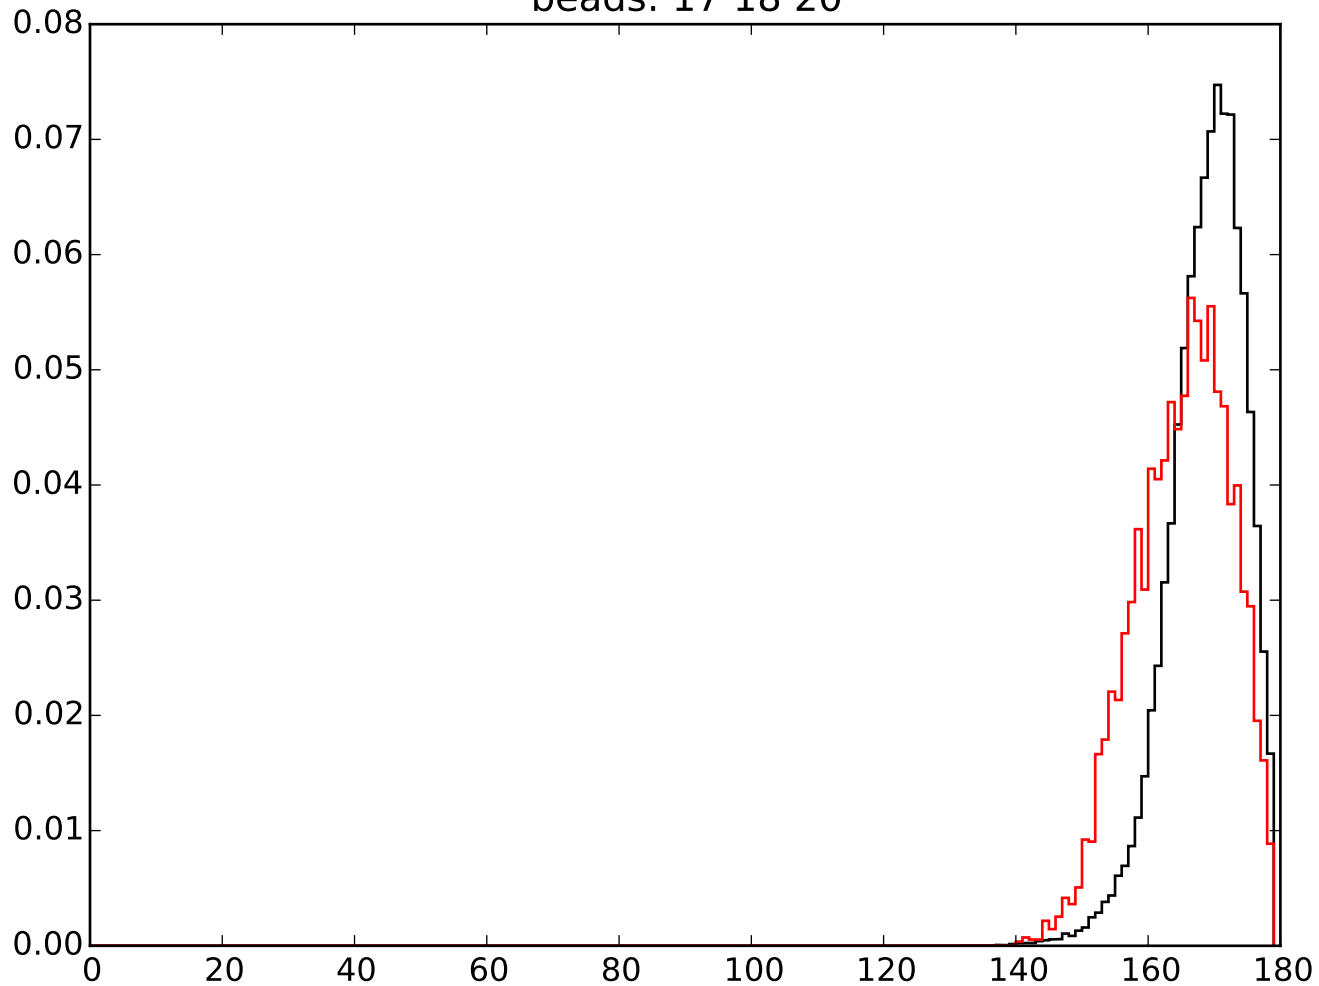

beads: 18 20 21

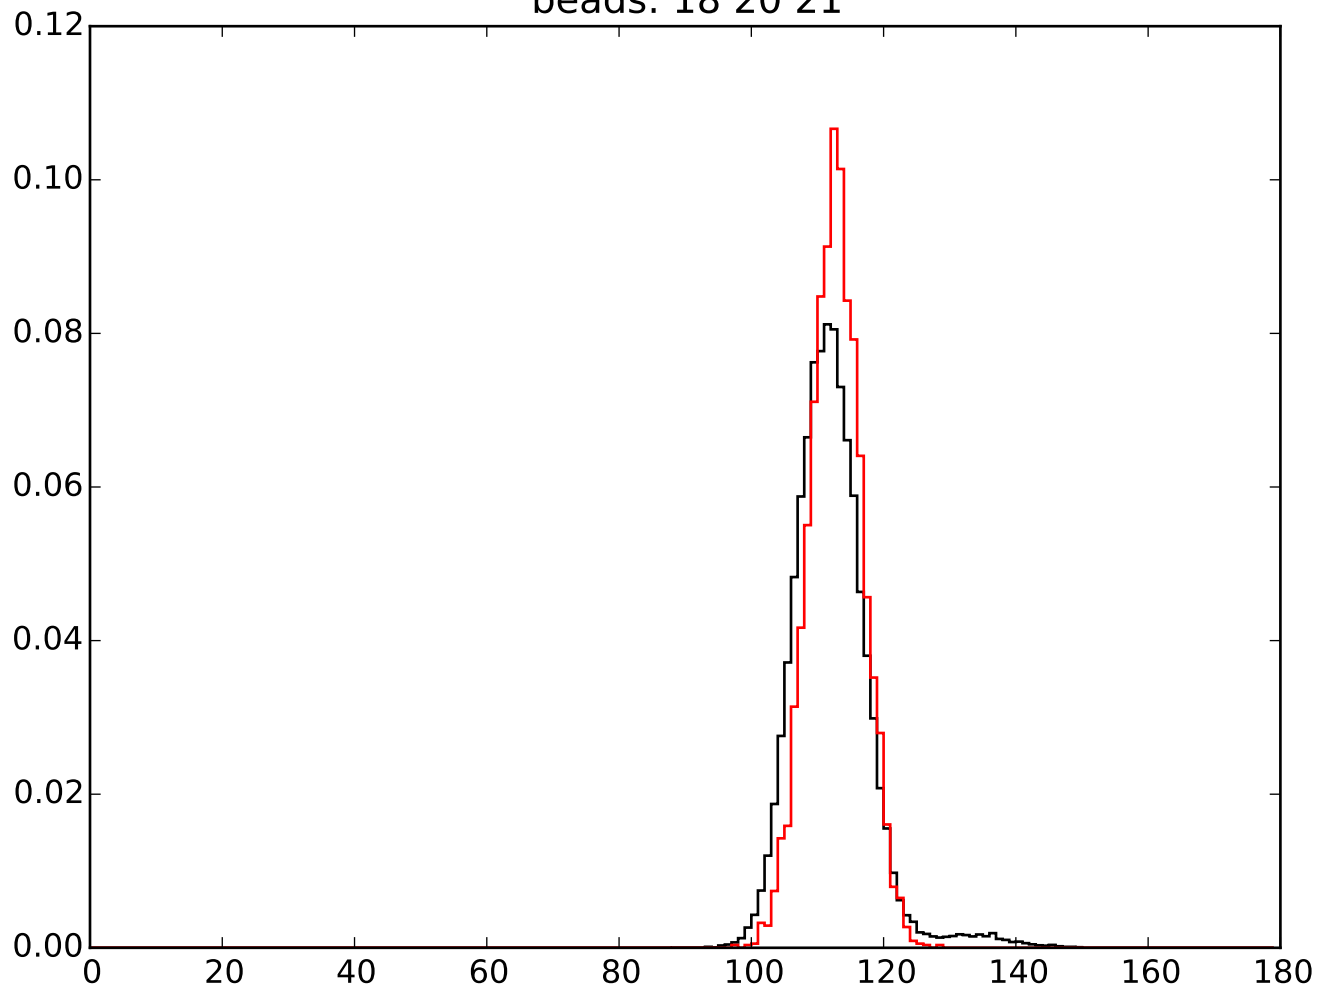

beads: 18 20 22

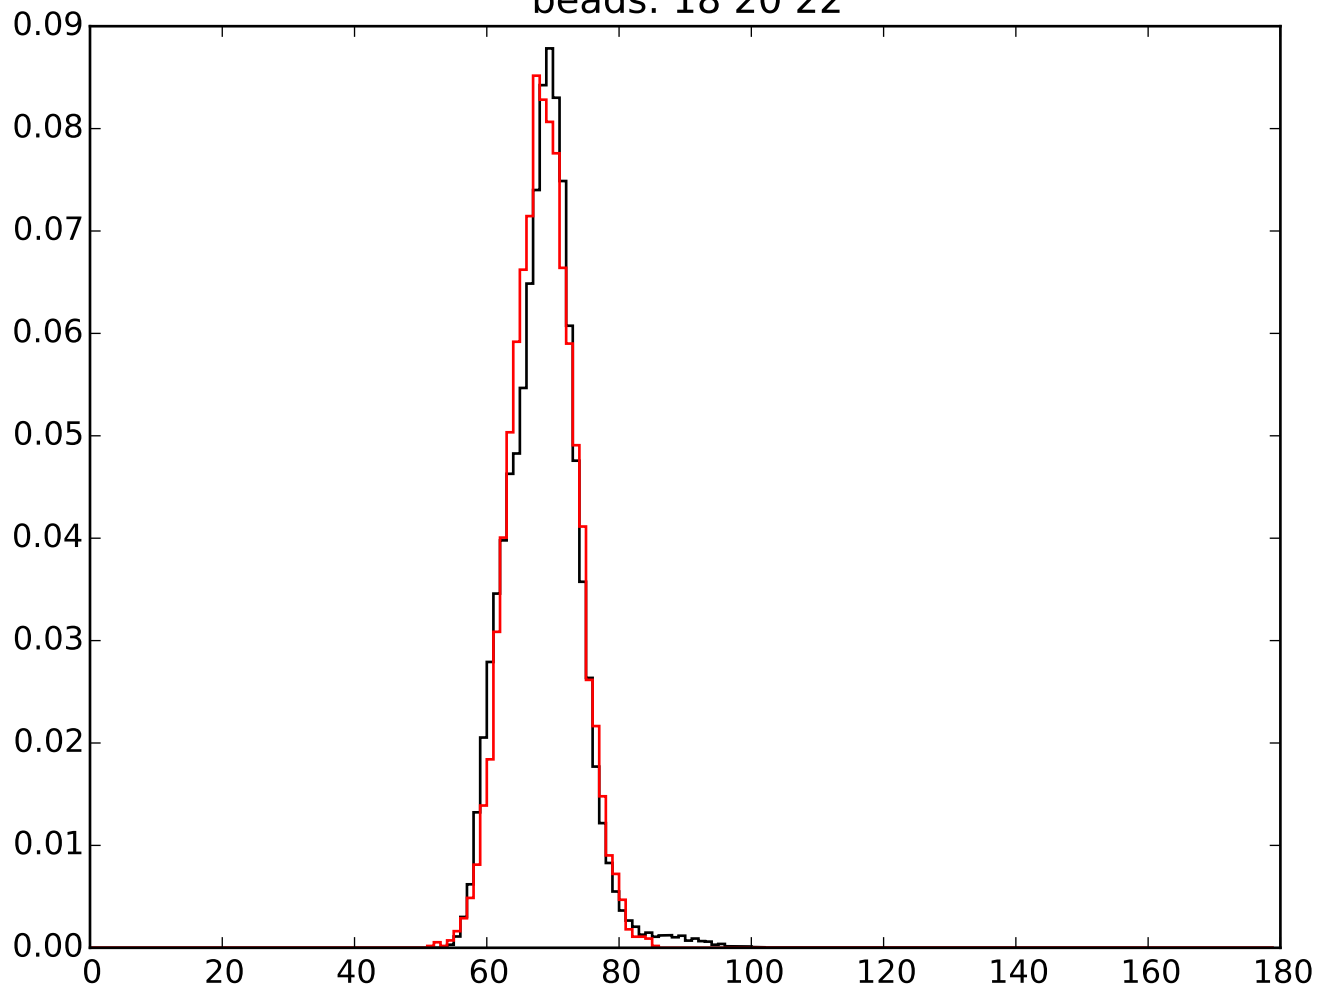

beads: 19 18 20

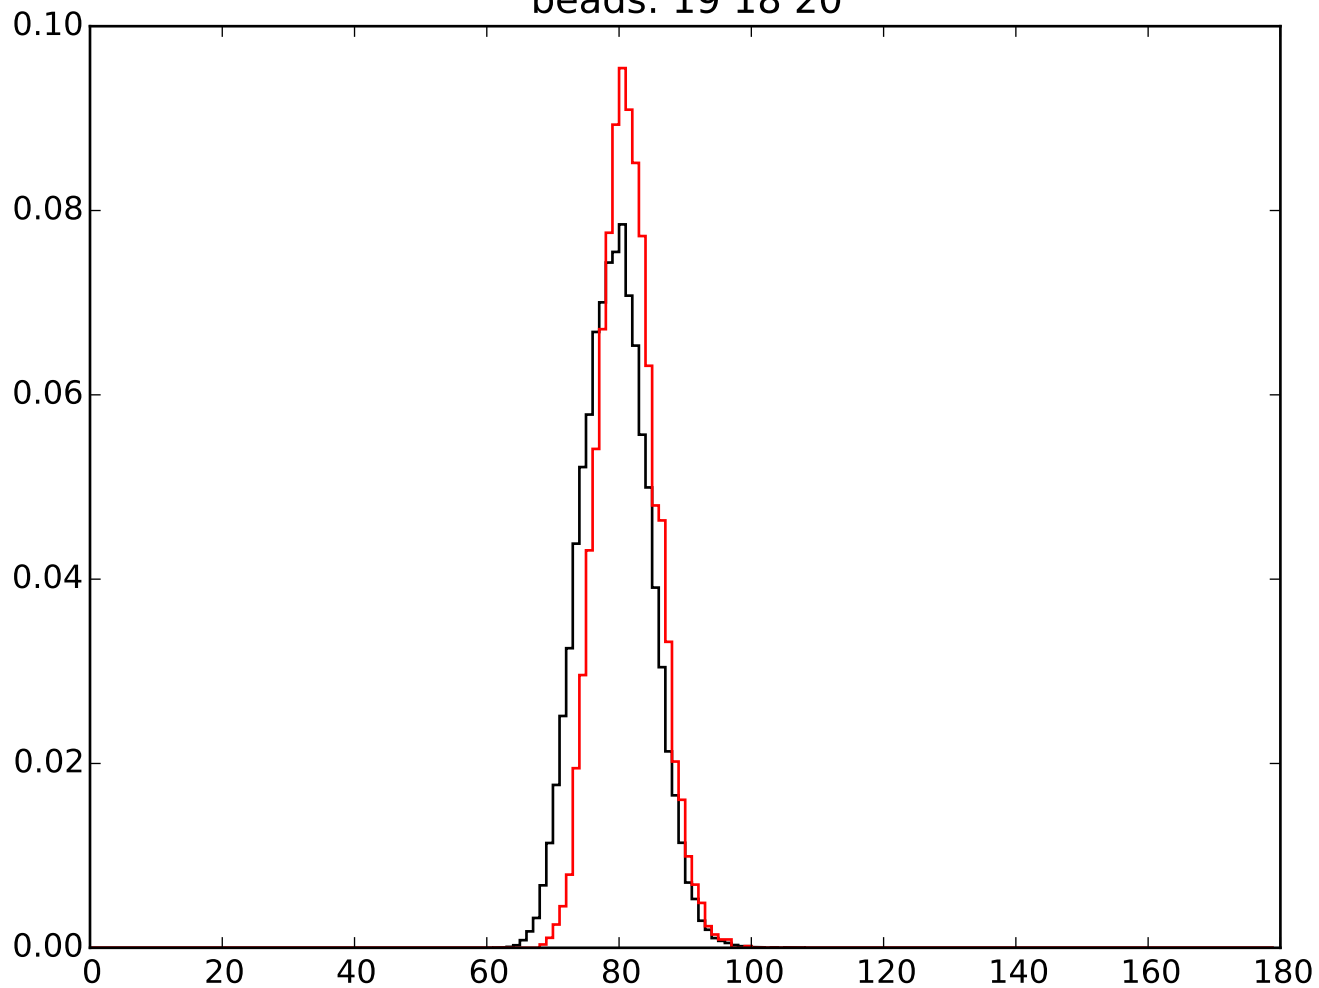

beads: 20 21 23

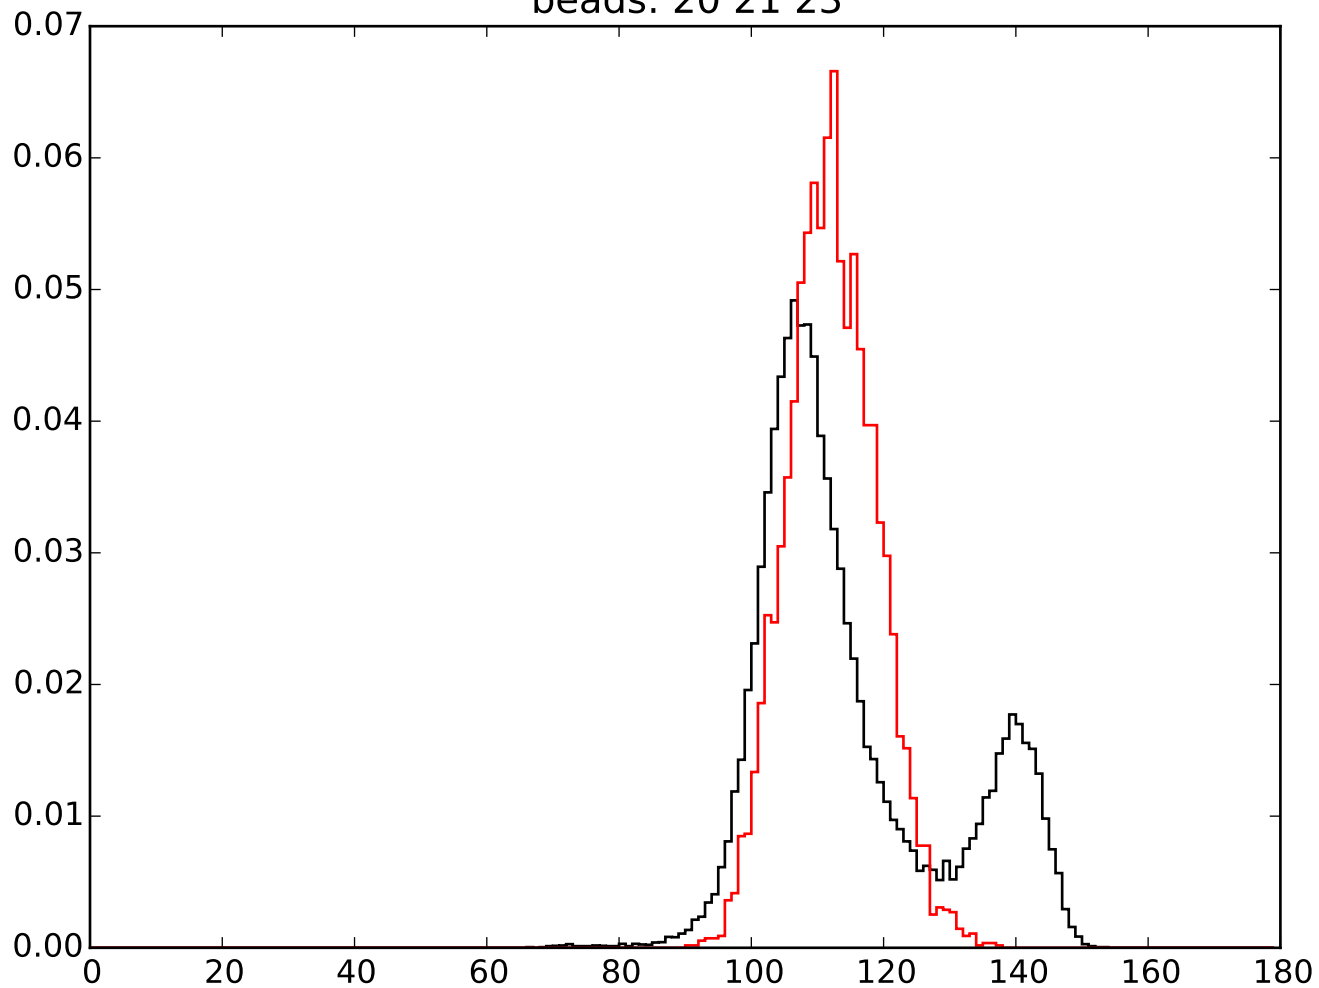

beads: 21 23 24

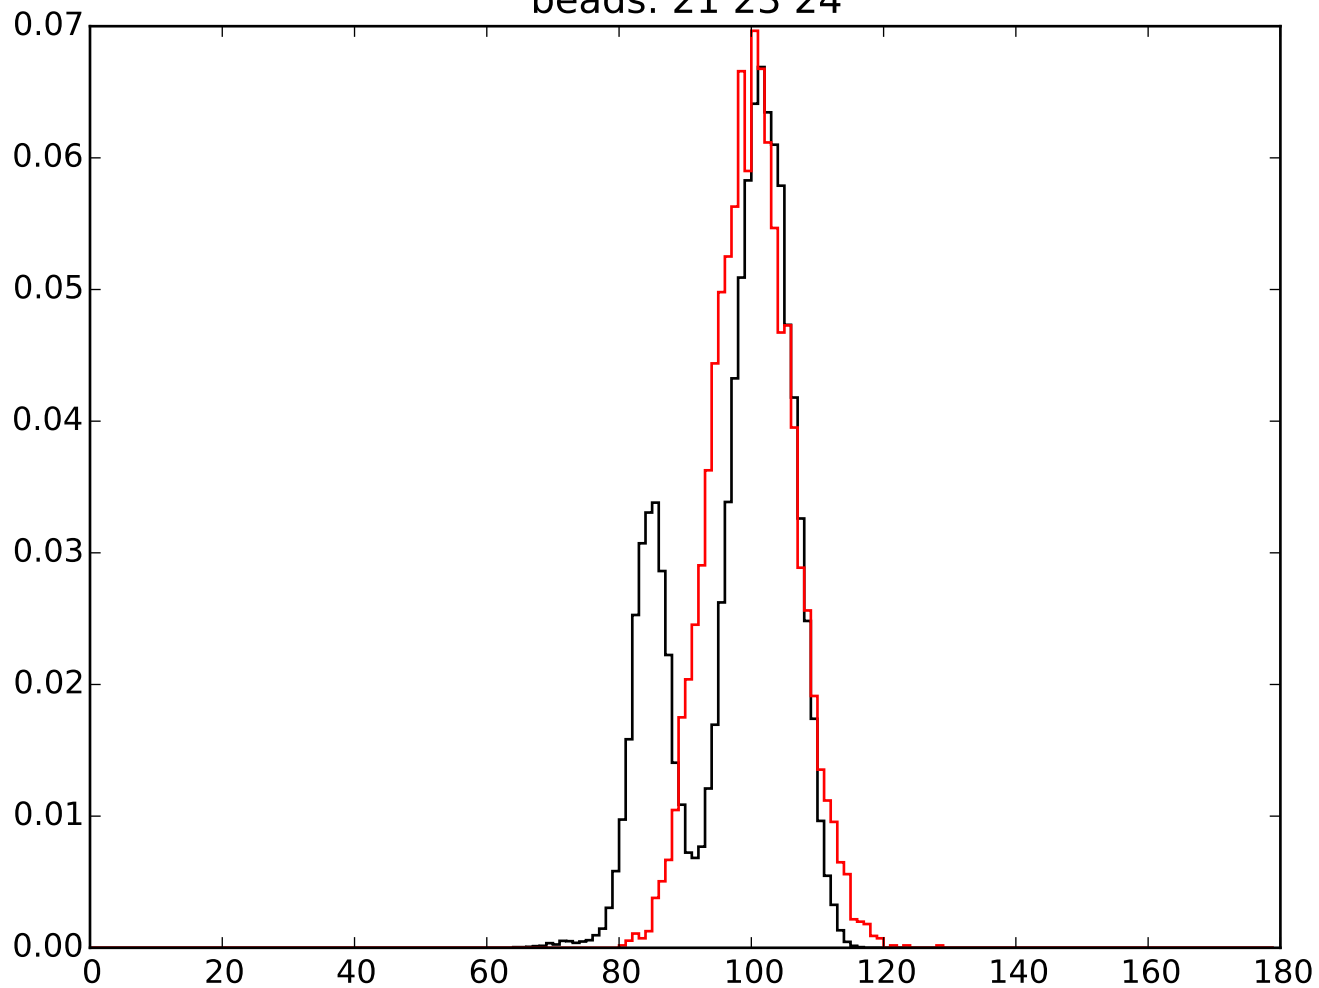

beads: 21 23 25

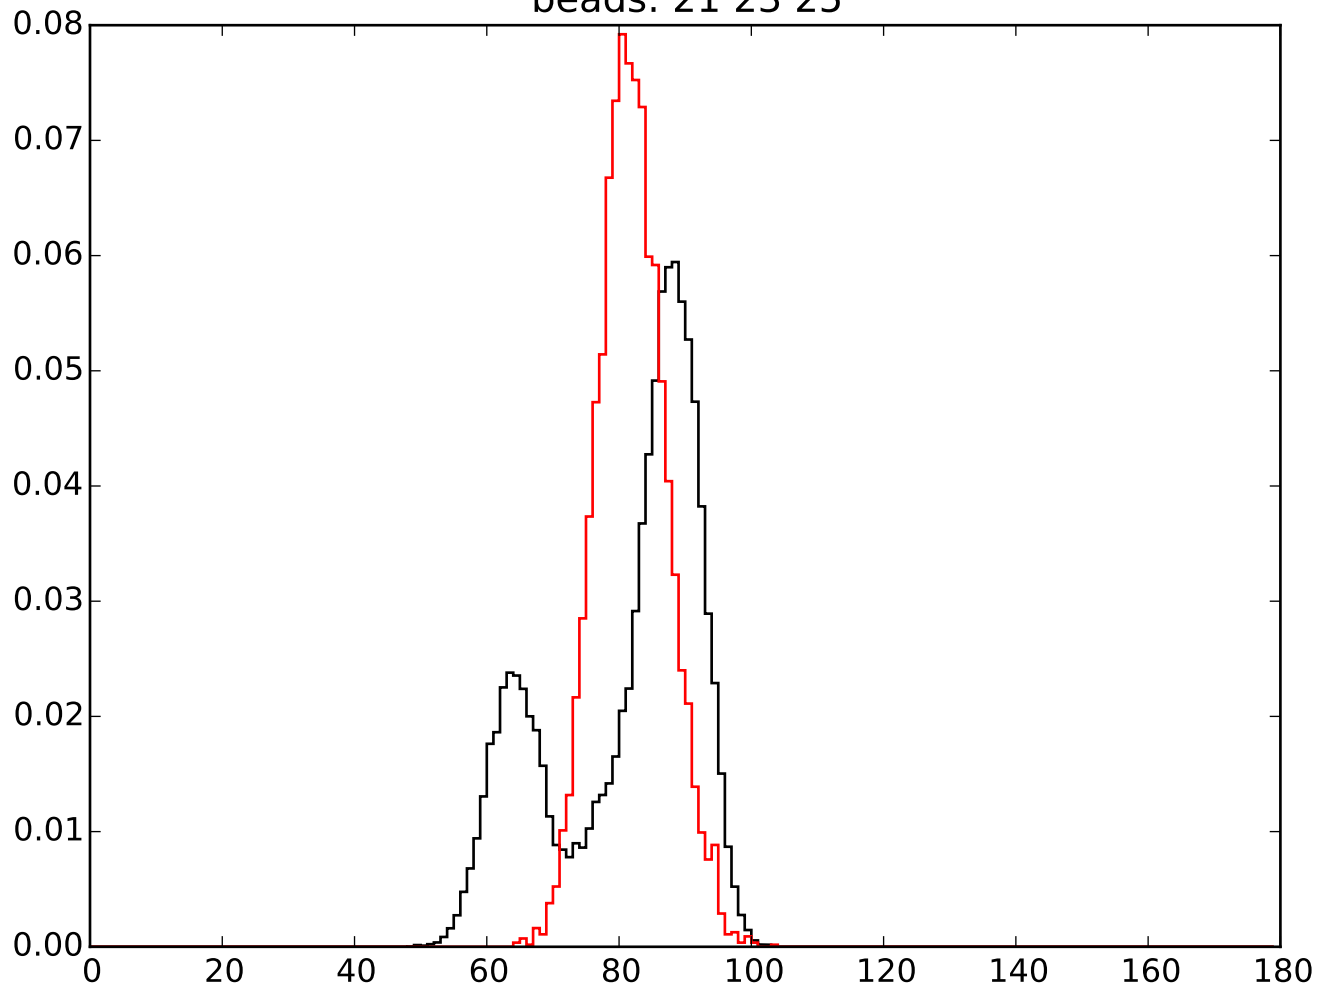



beads: 22 21 23

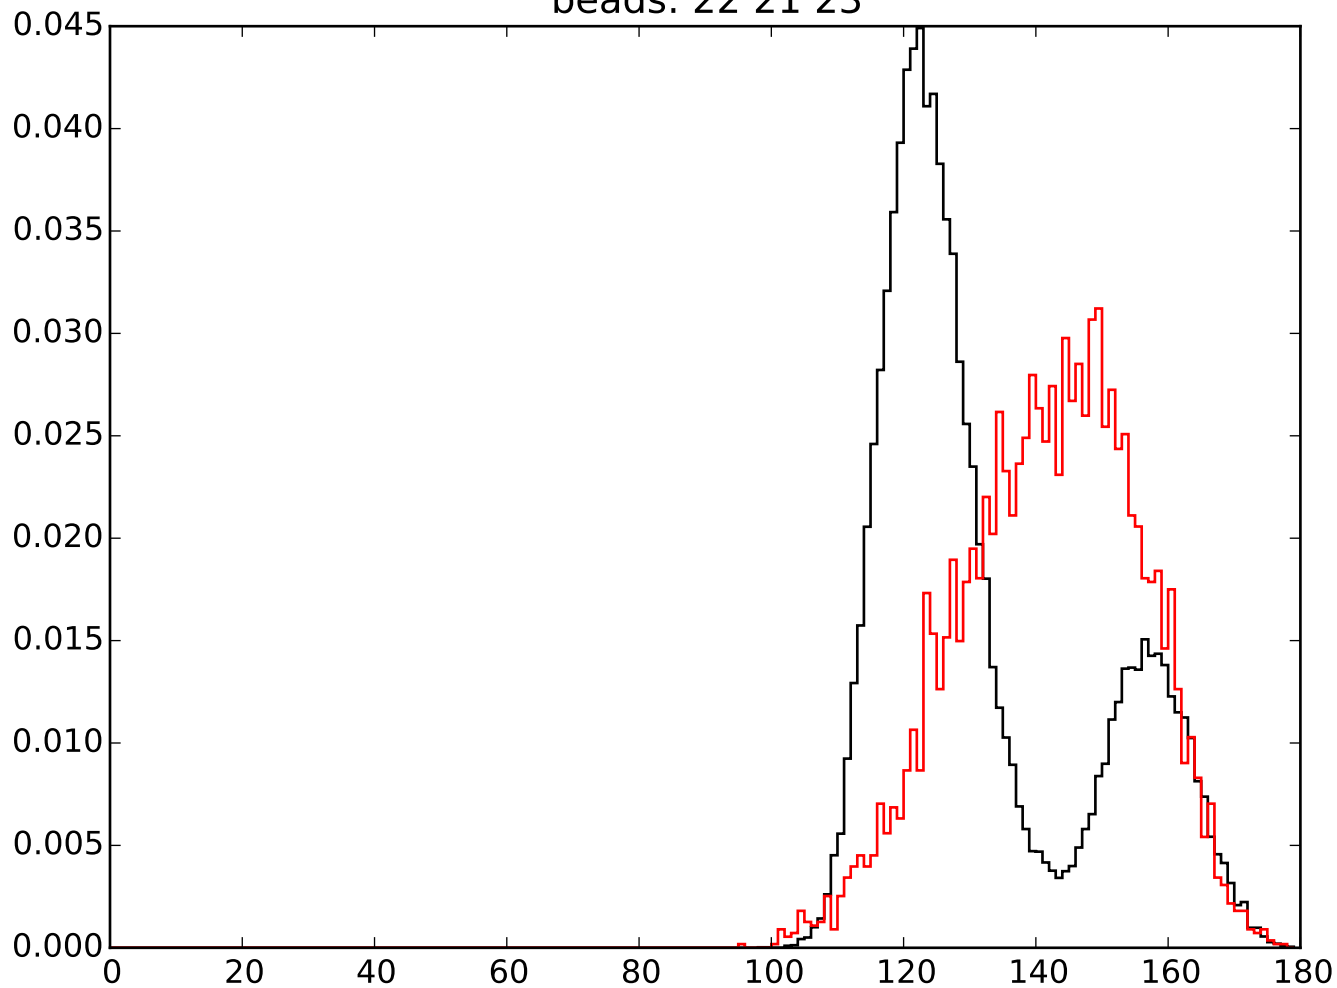

beads: 23 24 26

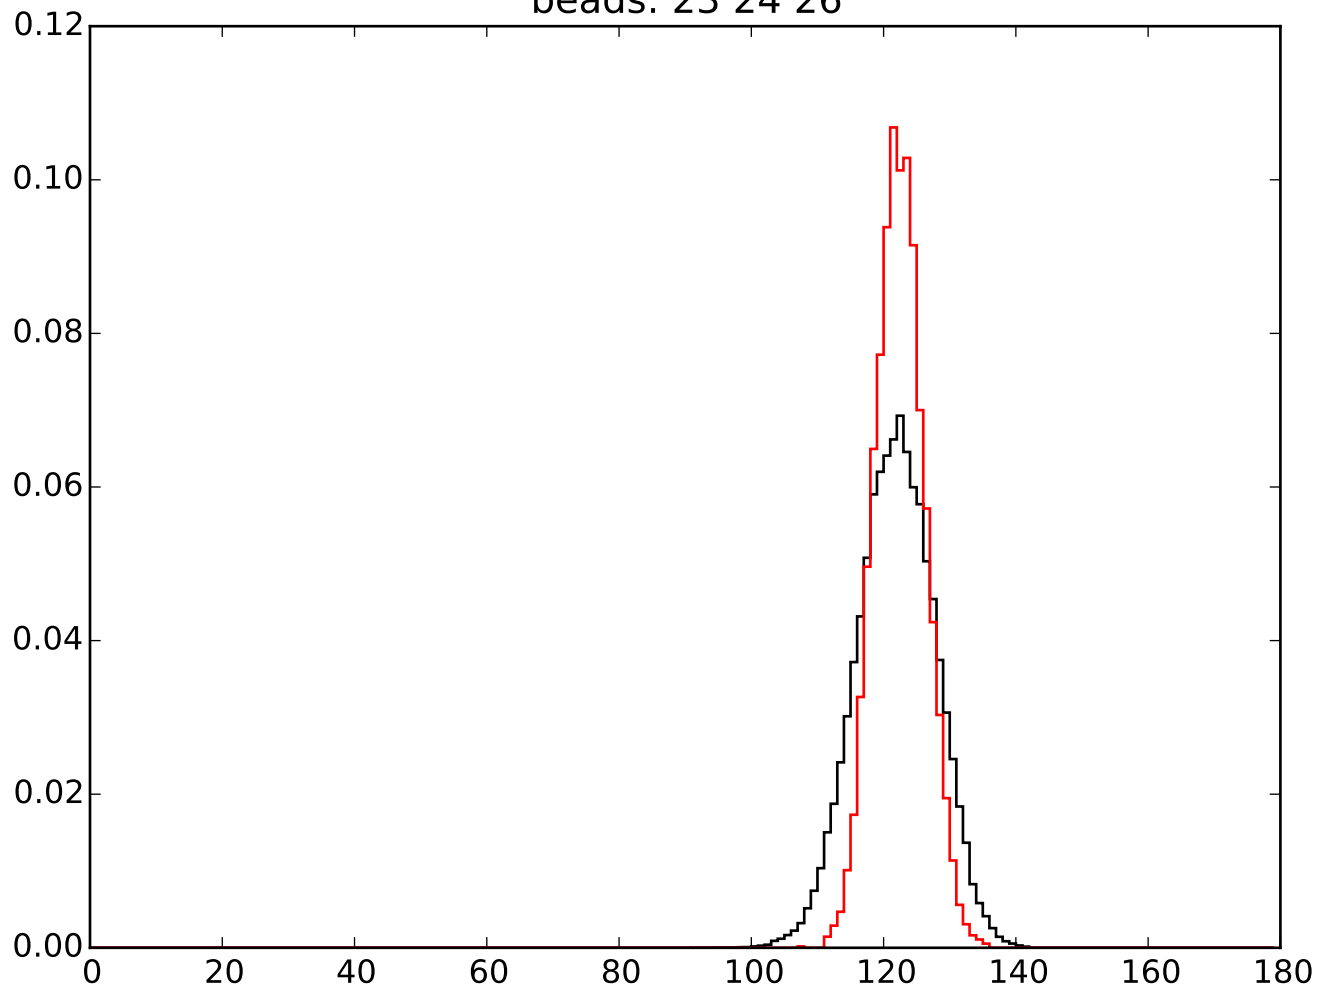

beads: 23 25 27

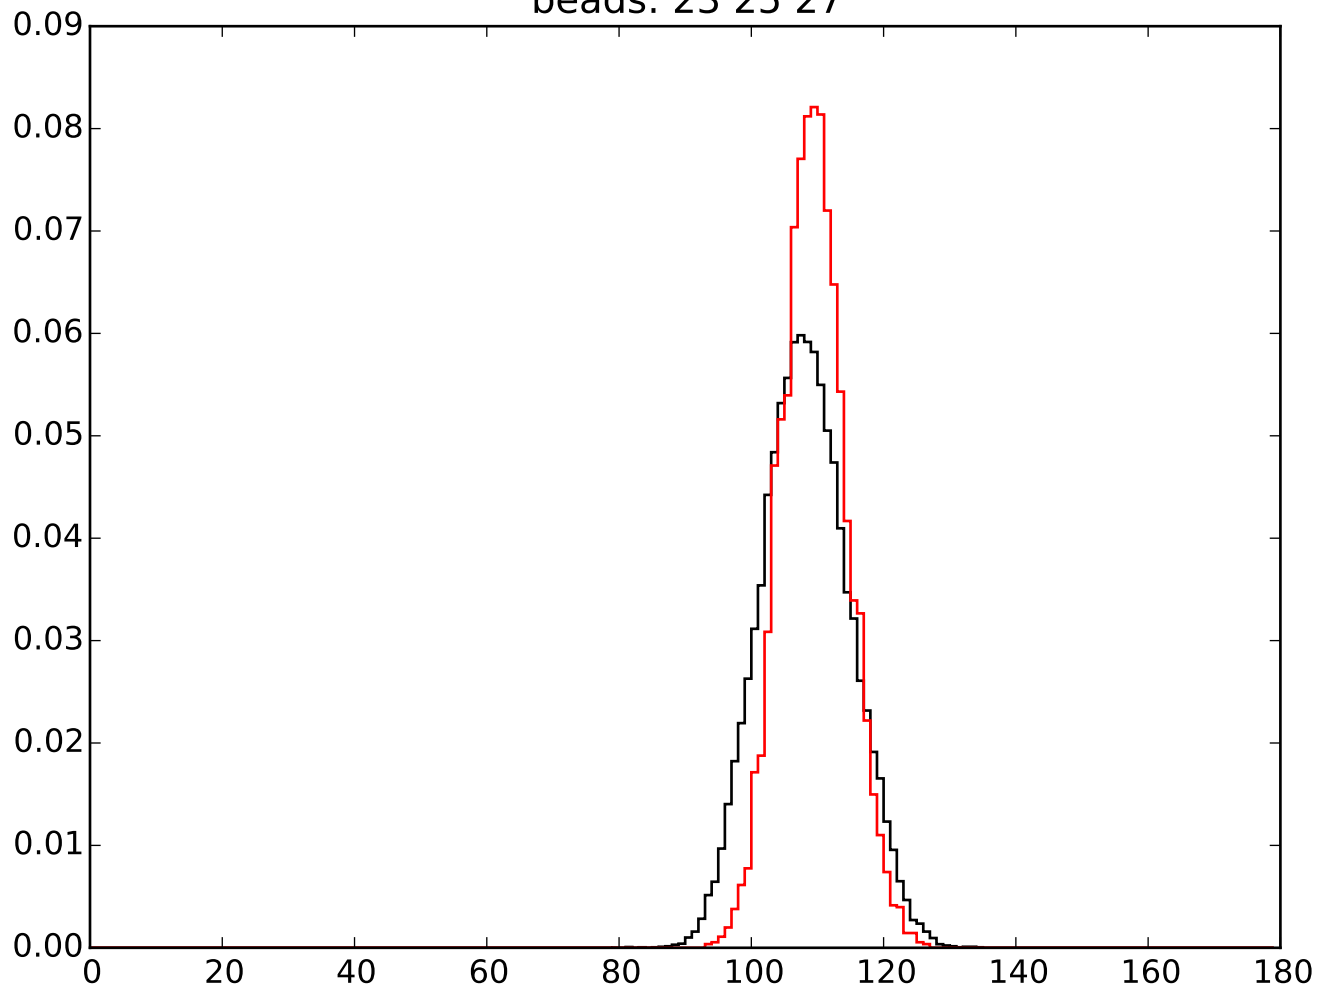

beads: 24 25 27

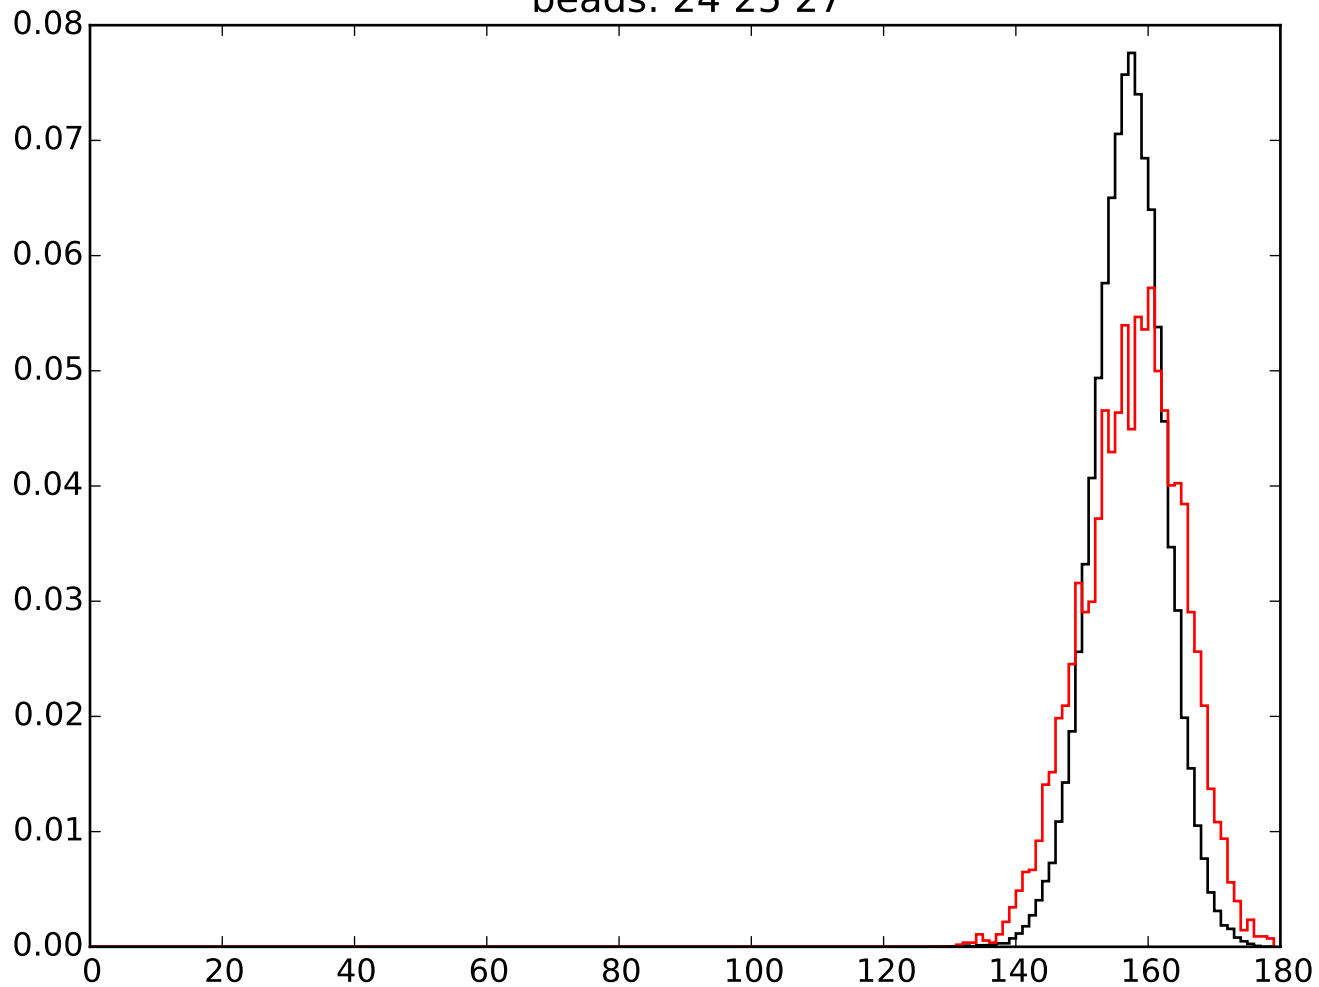

beads: 25 24 26

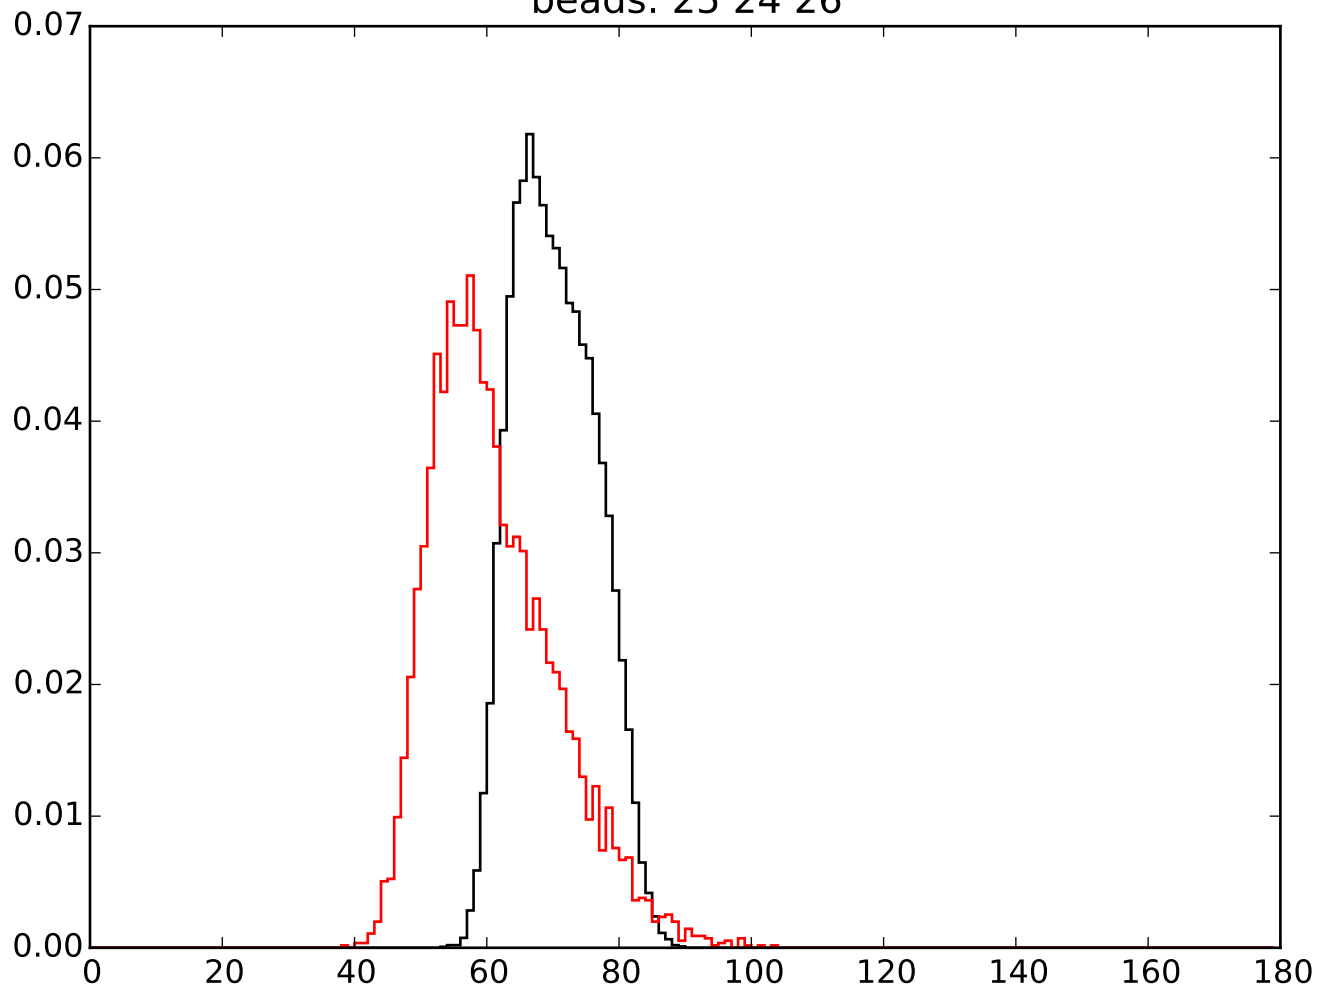

beads: 28 29 31

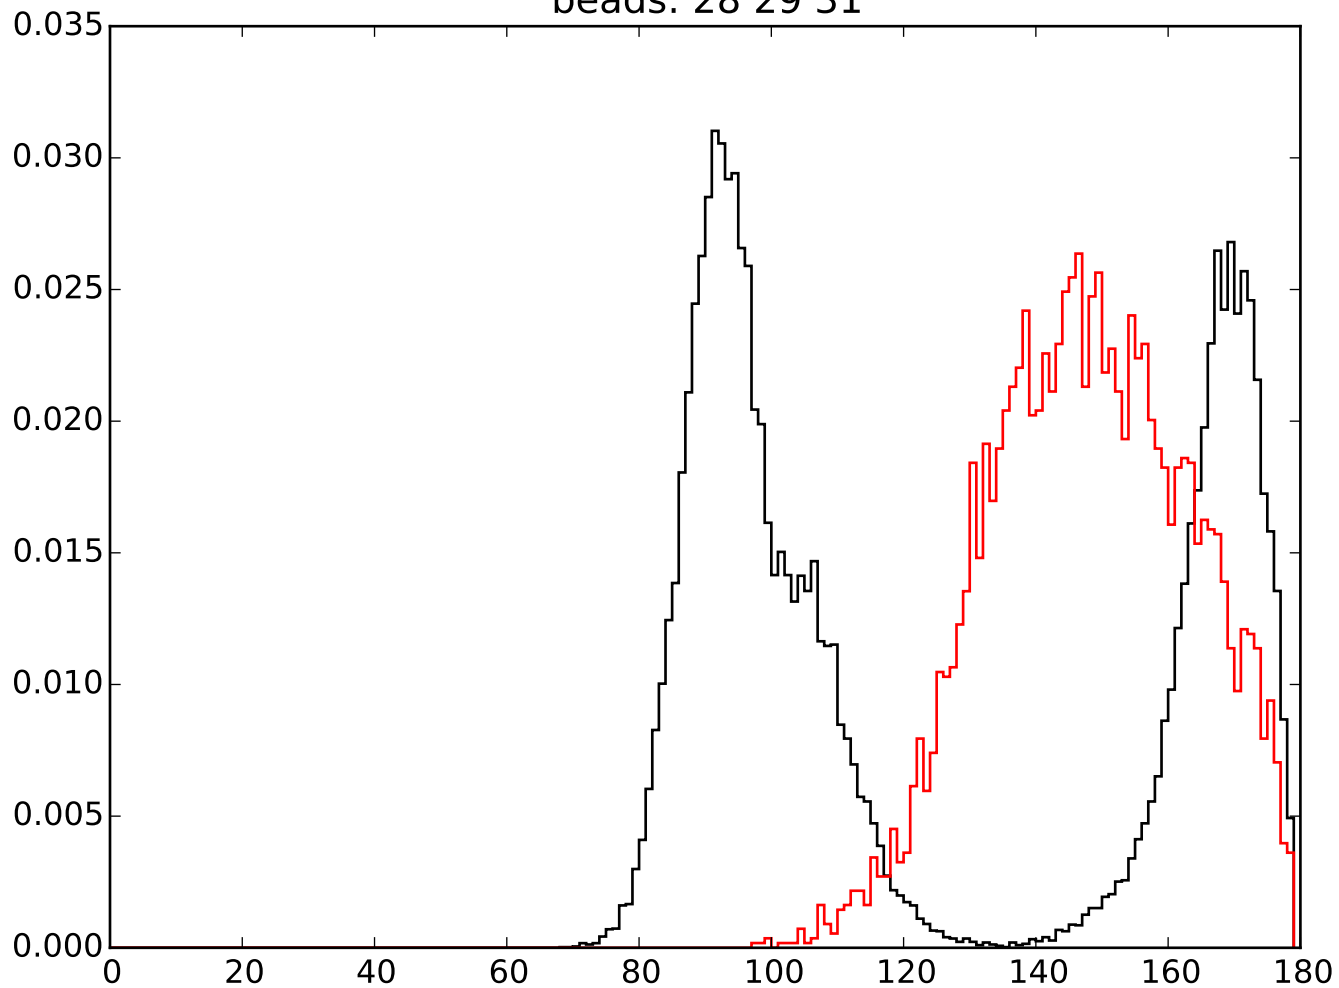

beads: 29 31 32

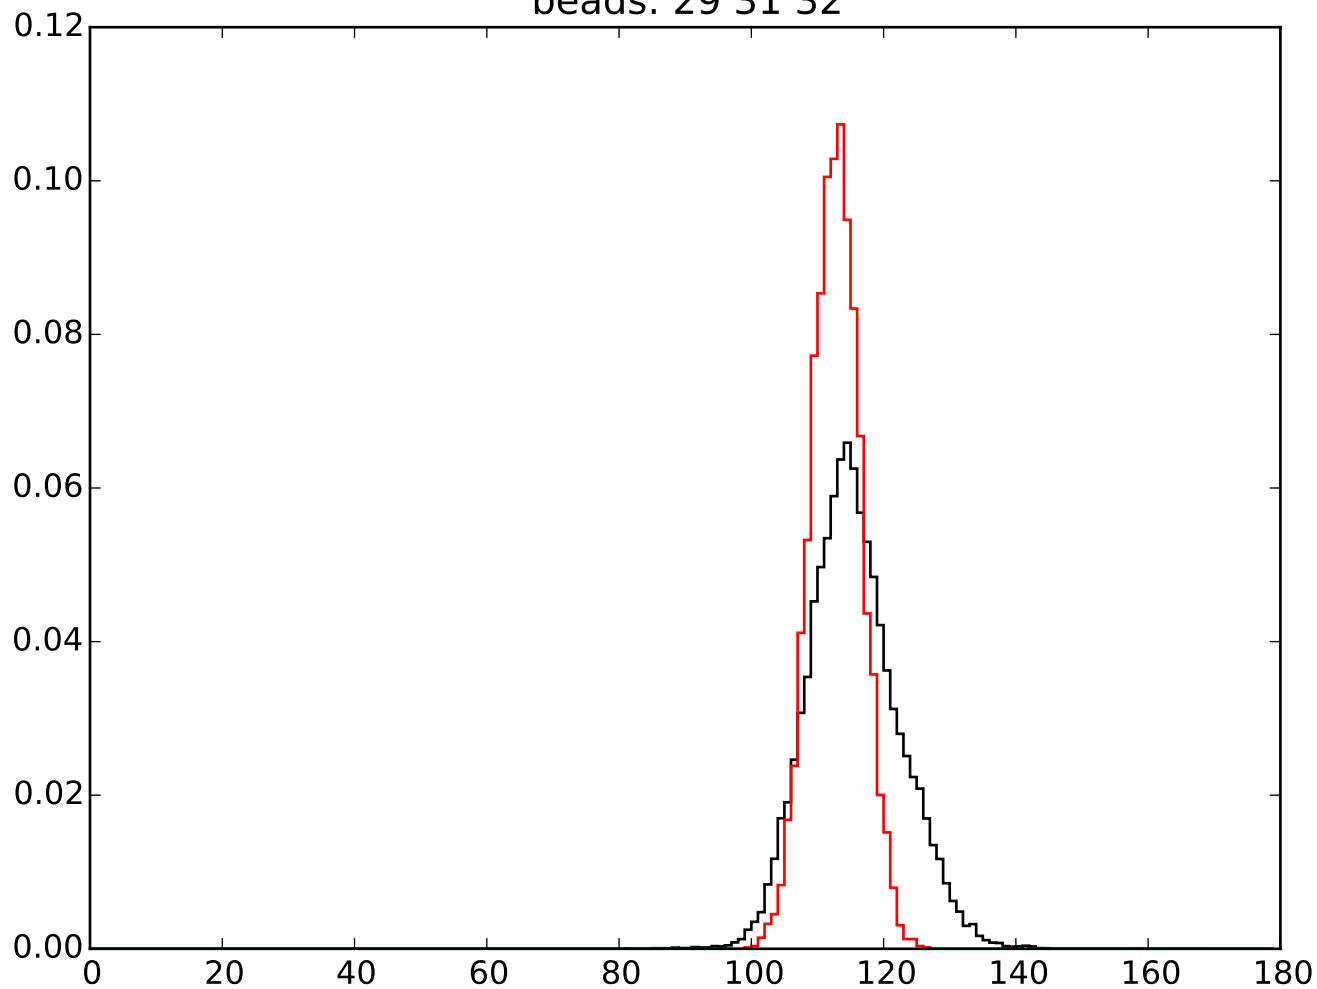

beads: 29 31 33

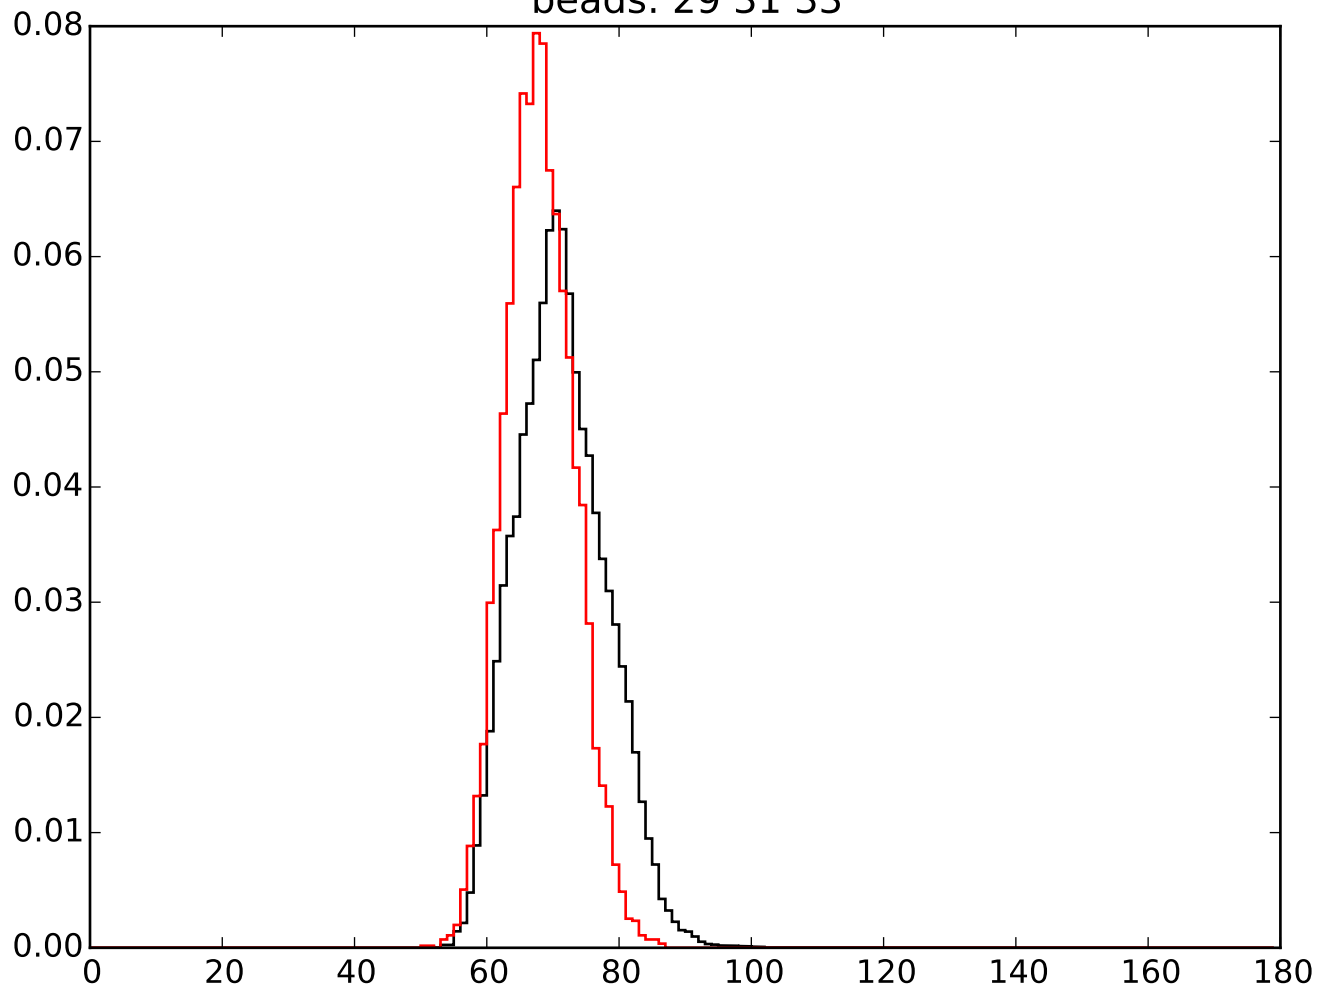



beads: 30 29 31

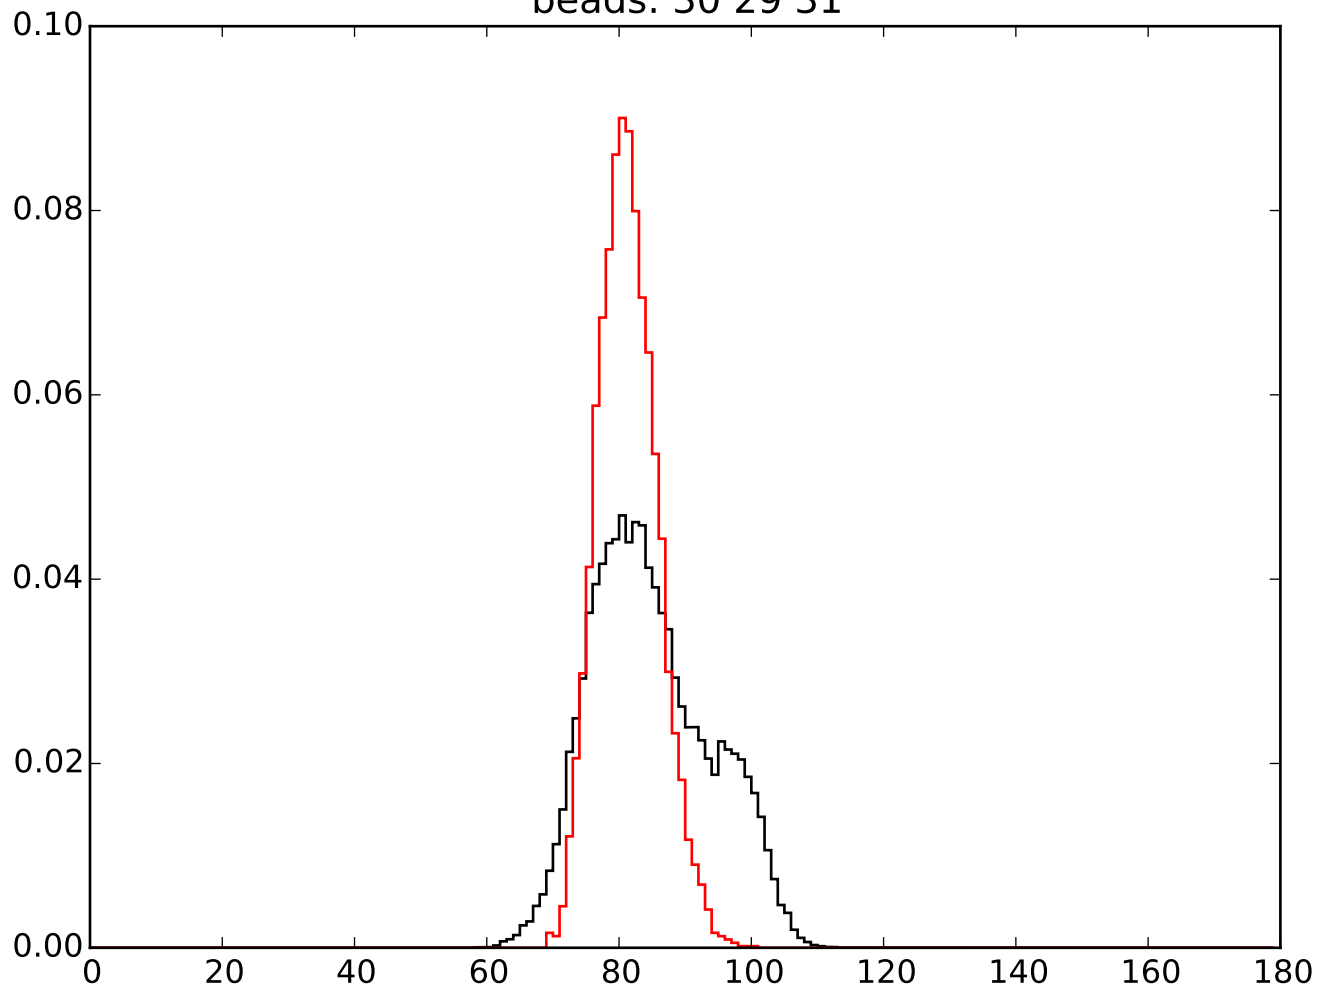

beads: 31 32 34

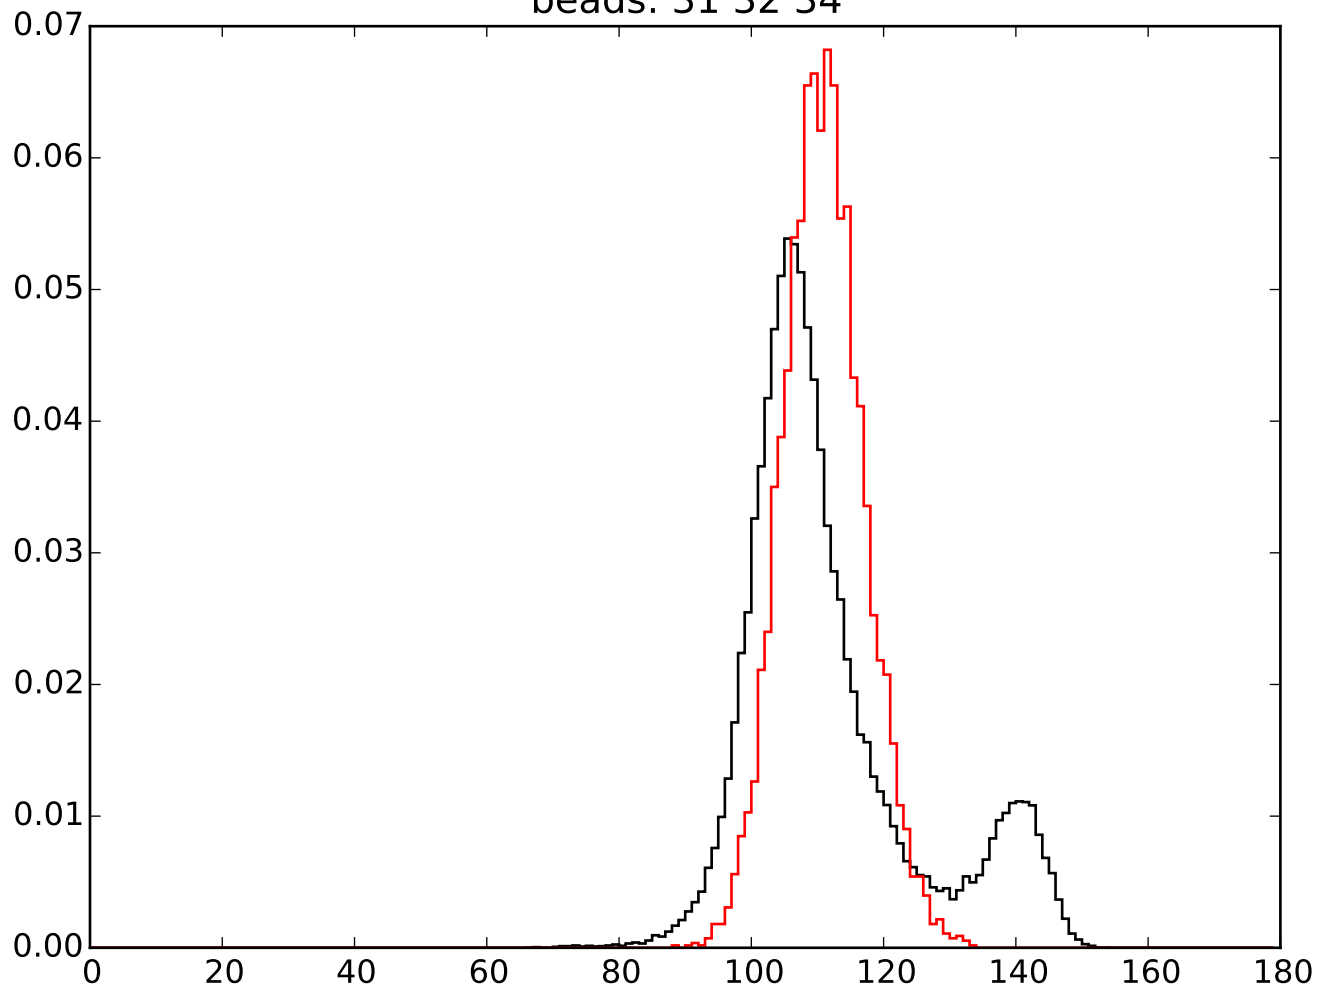

beads: 32 34 35

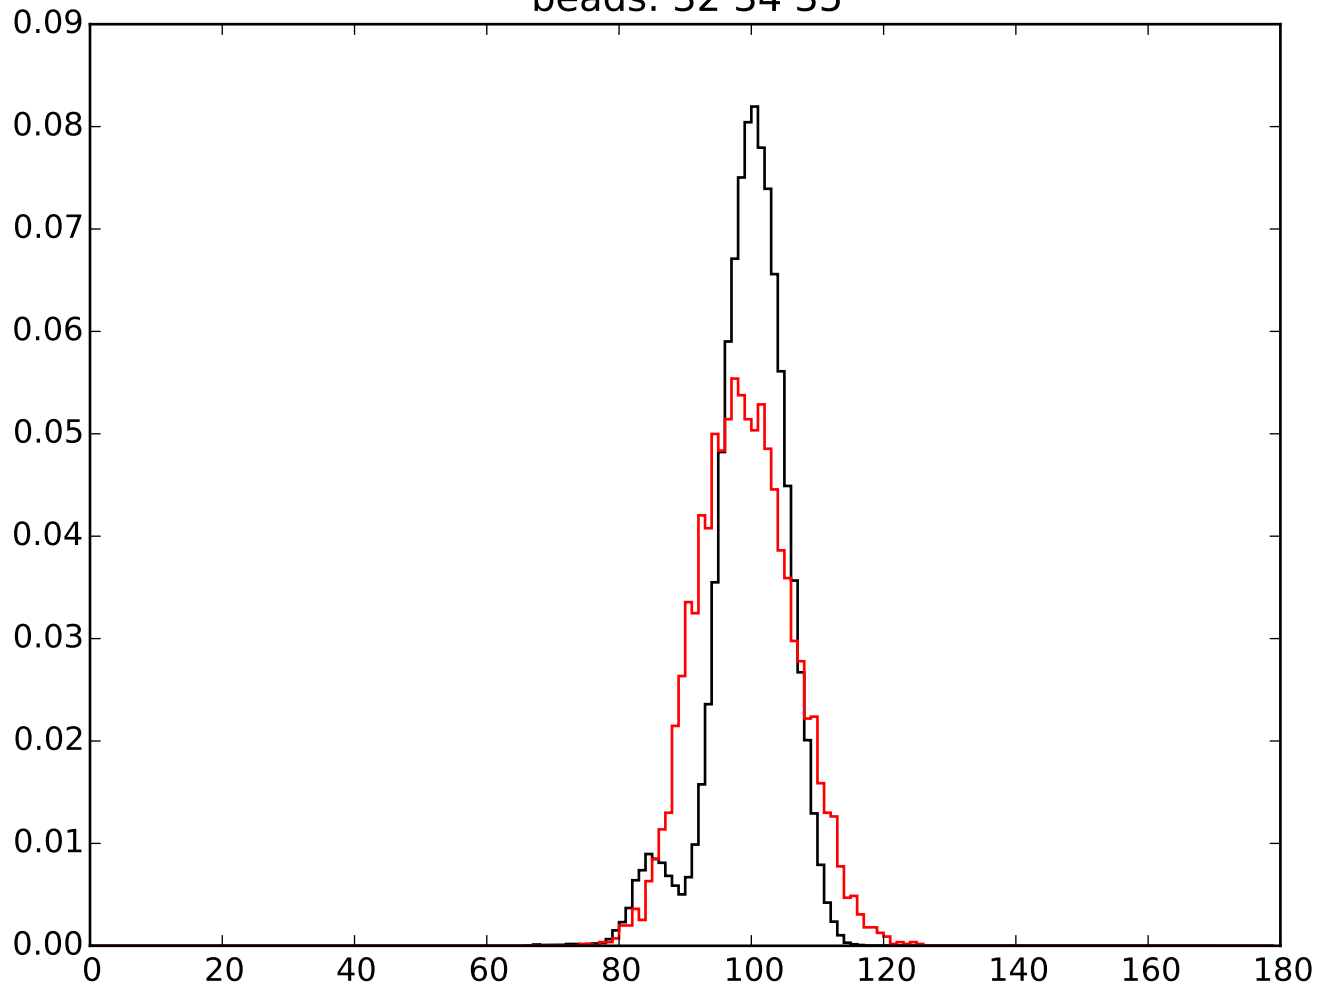

beads: 32 34 36

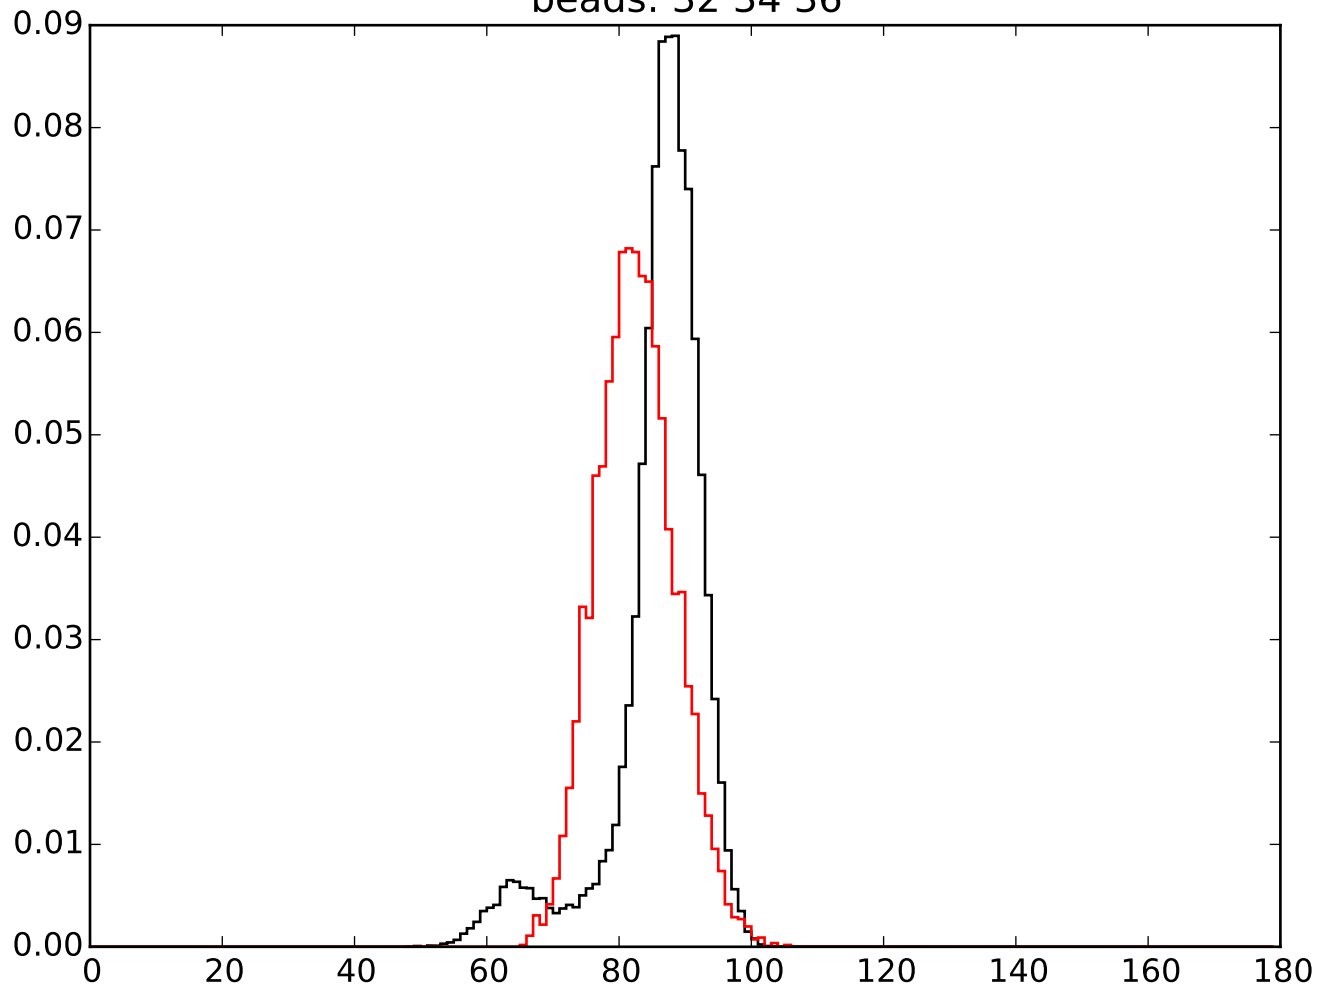

beads: 33 32 34

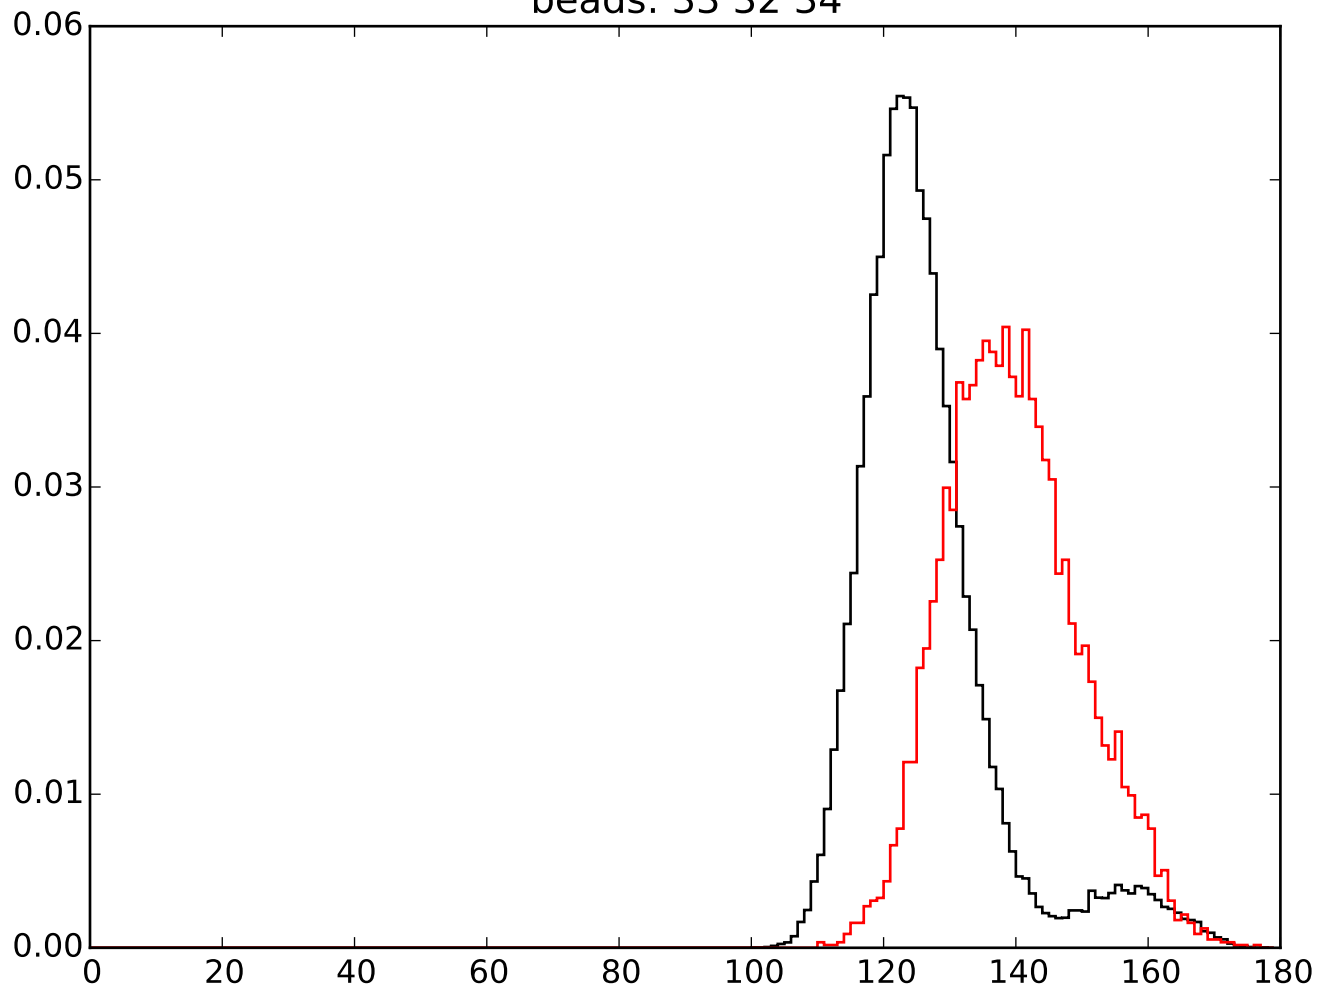

beads: 34 35 37

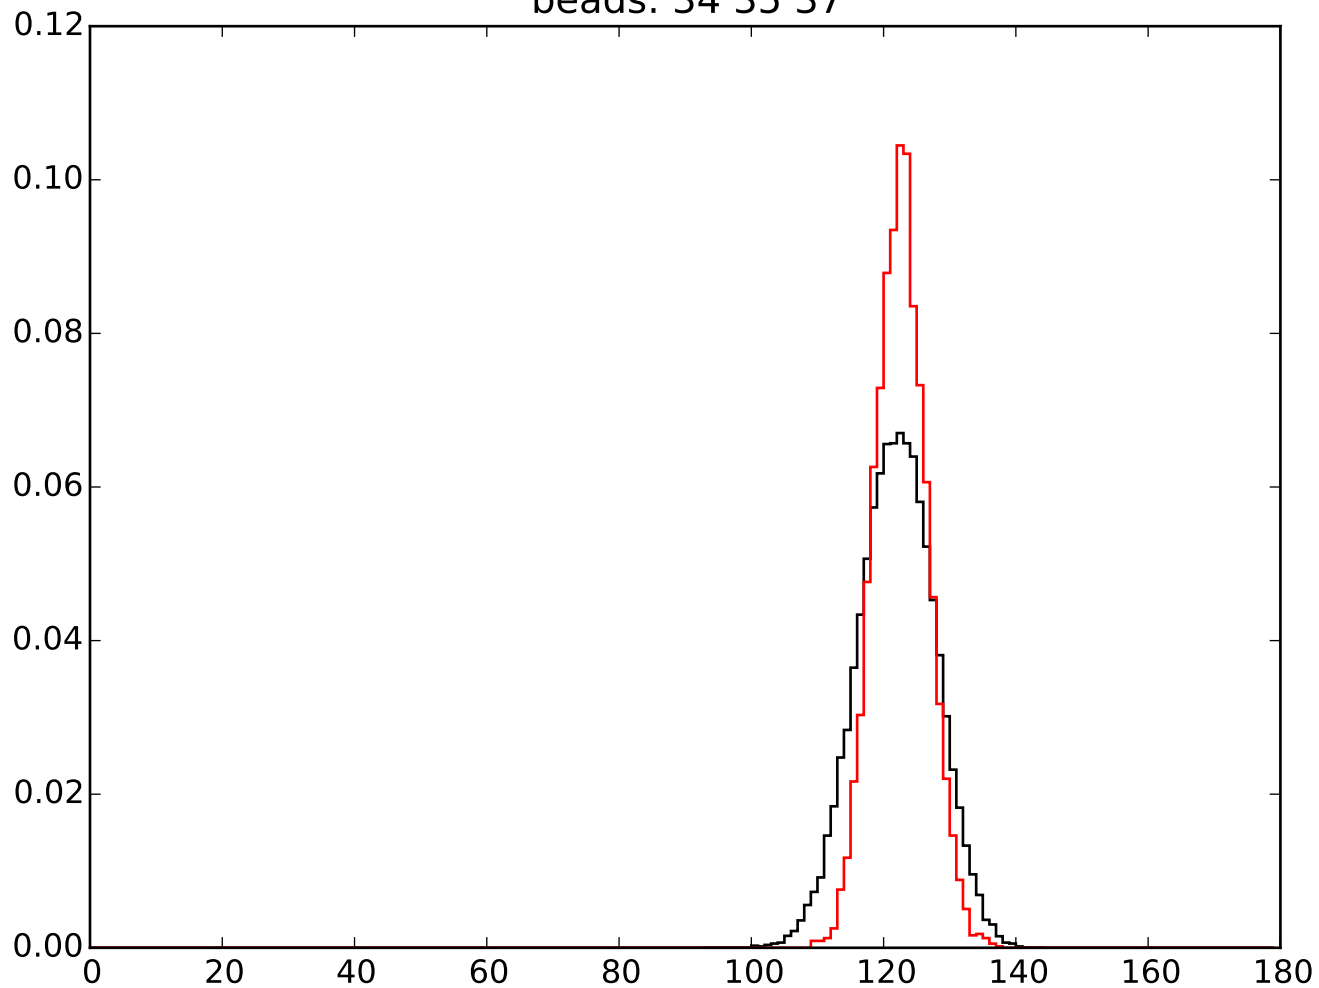

beads: 34 36 38

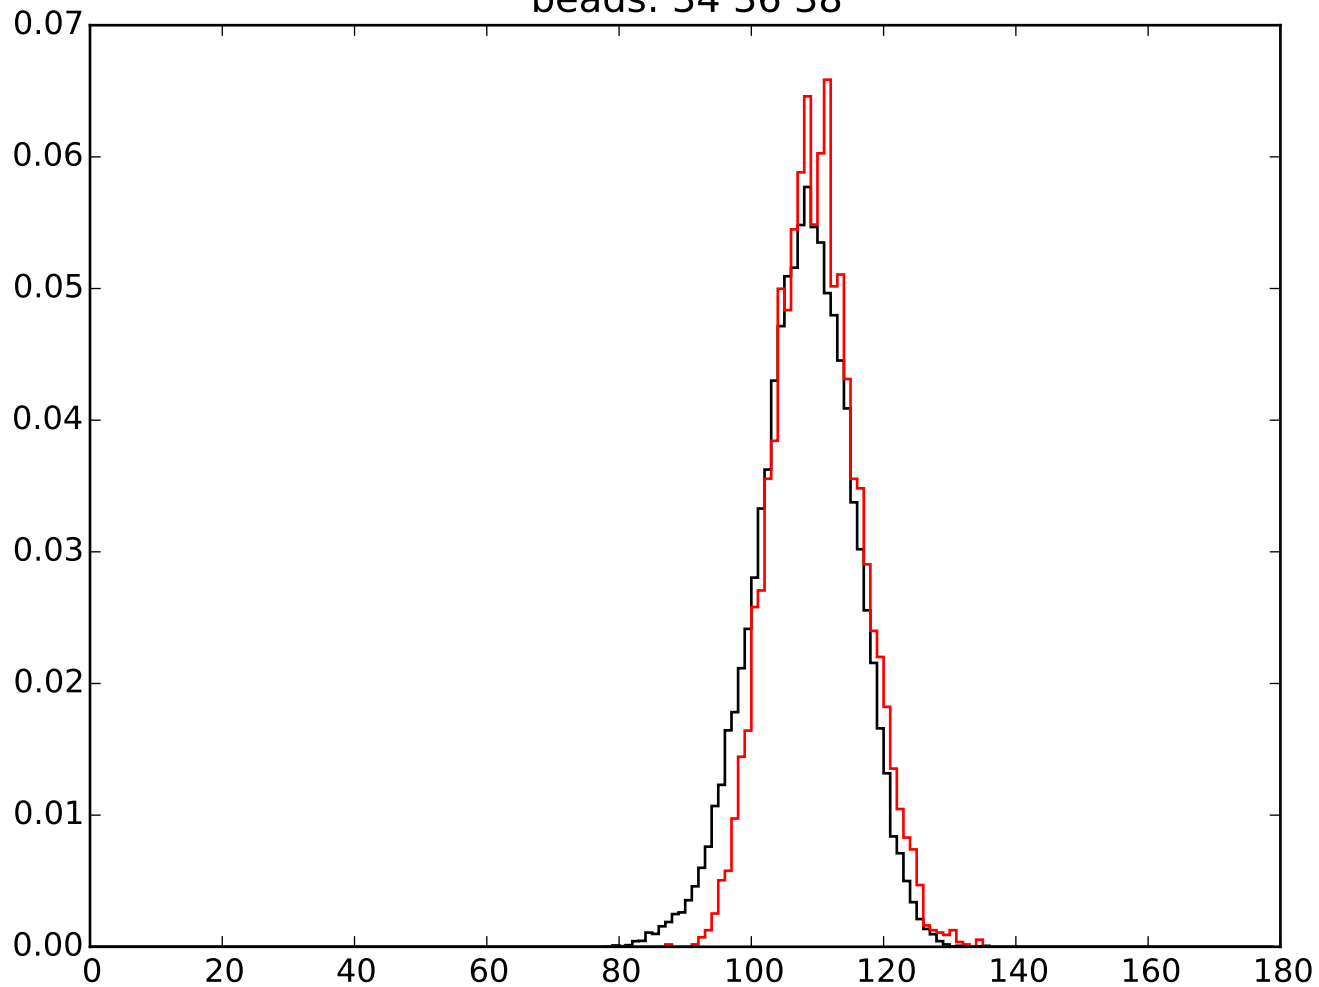

beads: 35 36 38

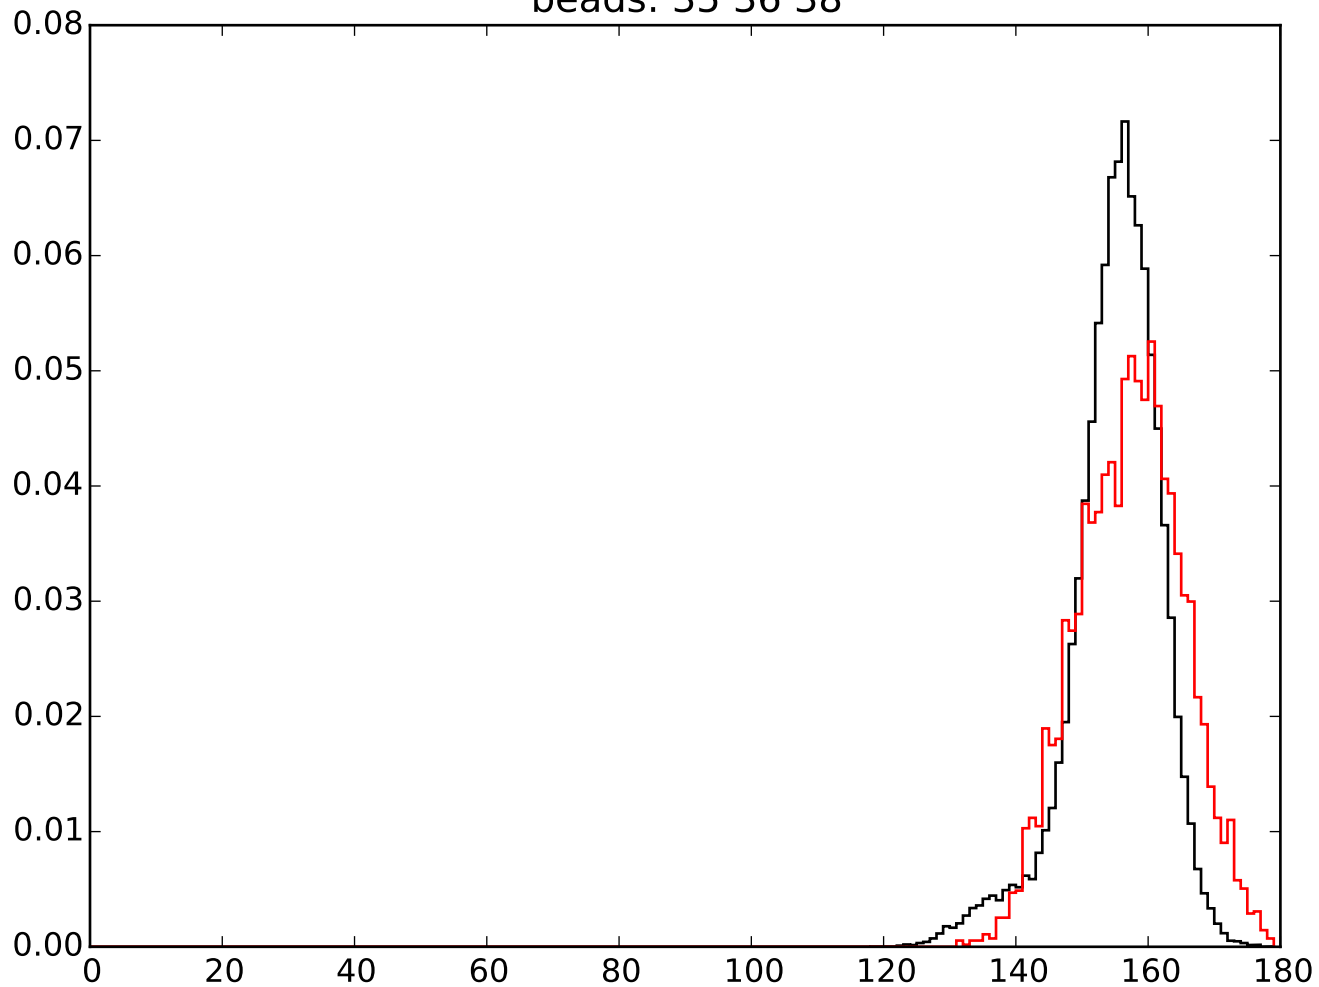



beads: 36 35 37

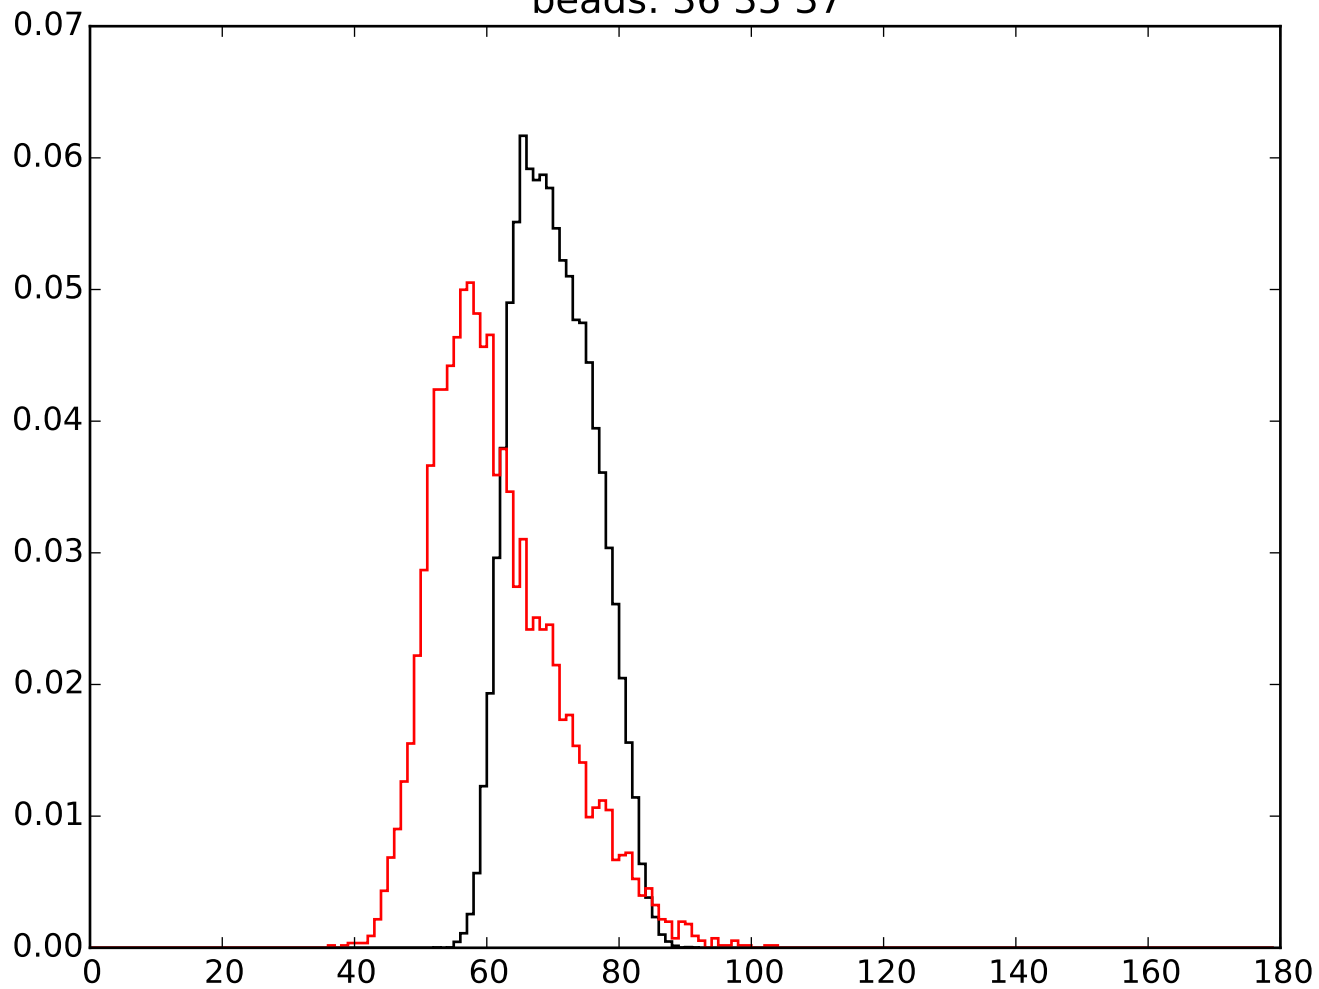

Supplement: Supplementary file 1 [file A2_angles_AA_vs_MARTINI.pdf]
