# Supplementary material for: Overcoming the limitations of the MARTINI force field in Molecular Dynamics simulations of polysaccharides
Source: arXiv:1704.03773 ancillary file (2017-06-27)

beads: 1 2

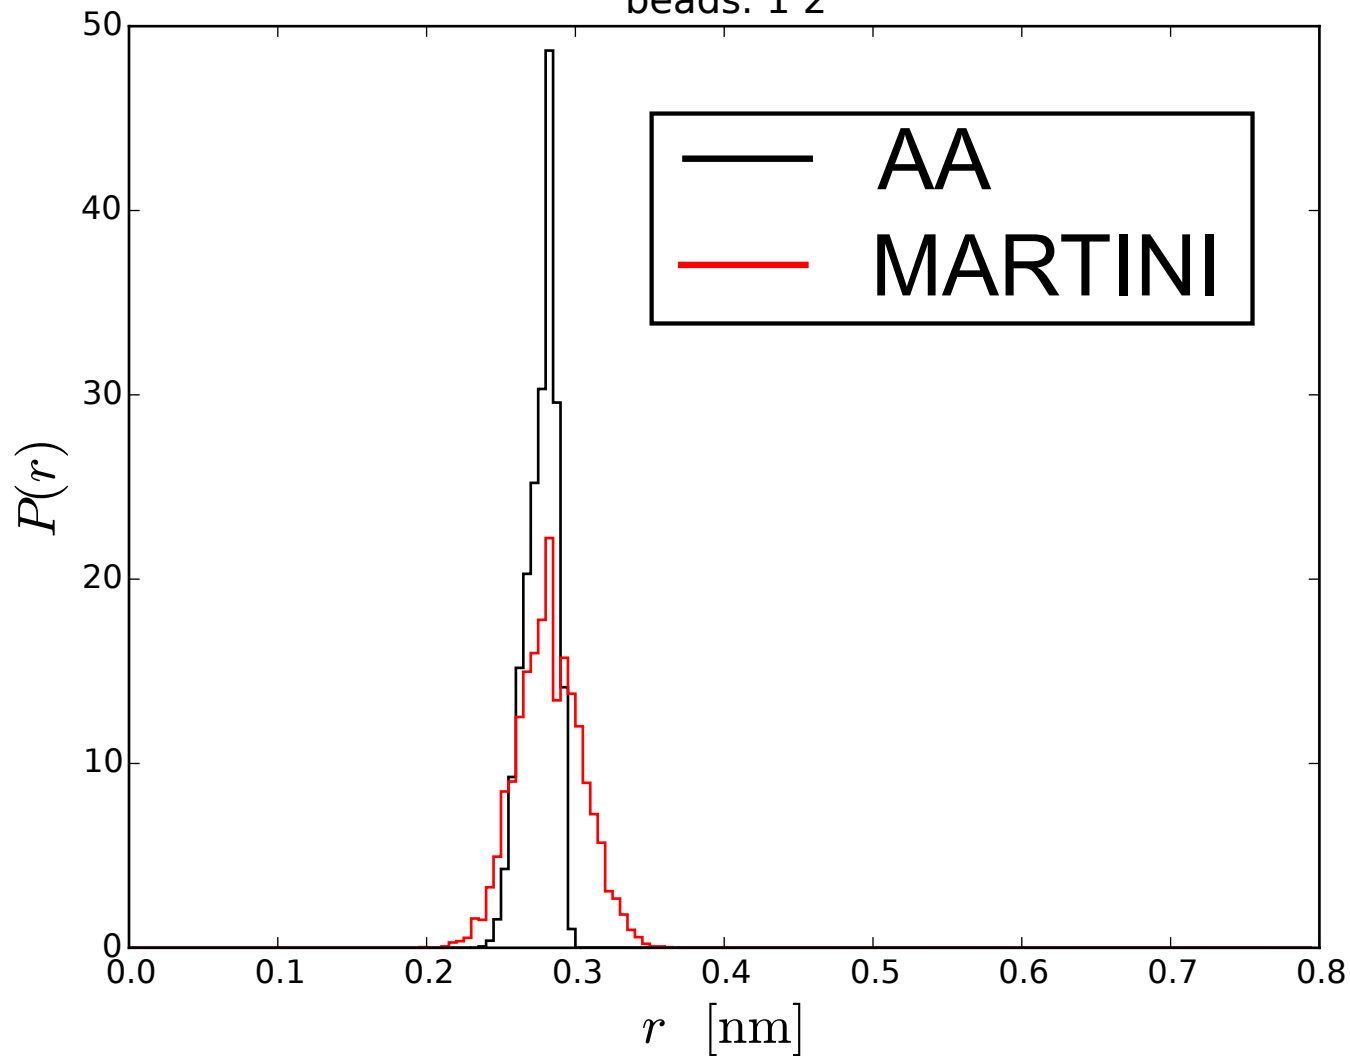

beads: 2 3

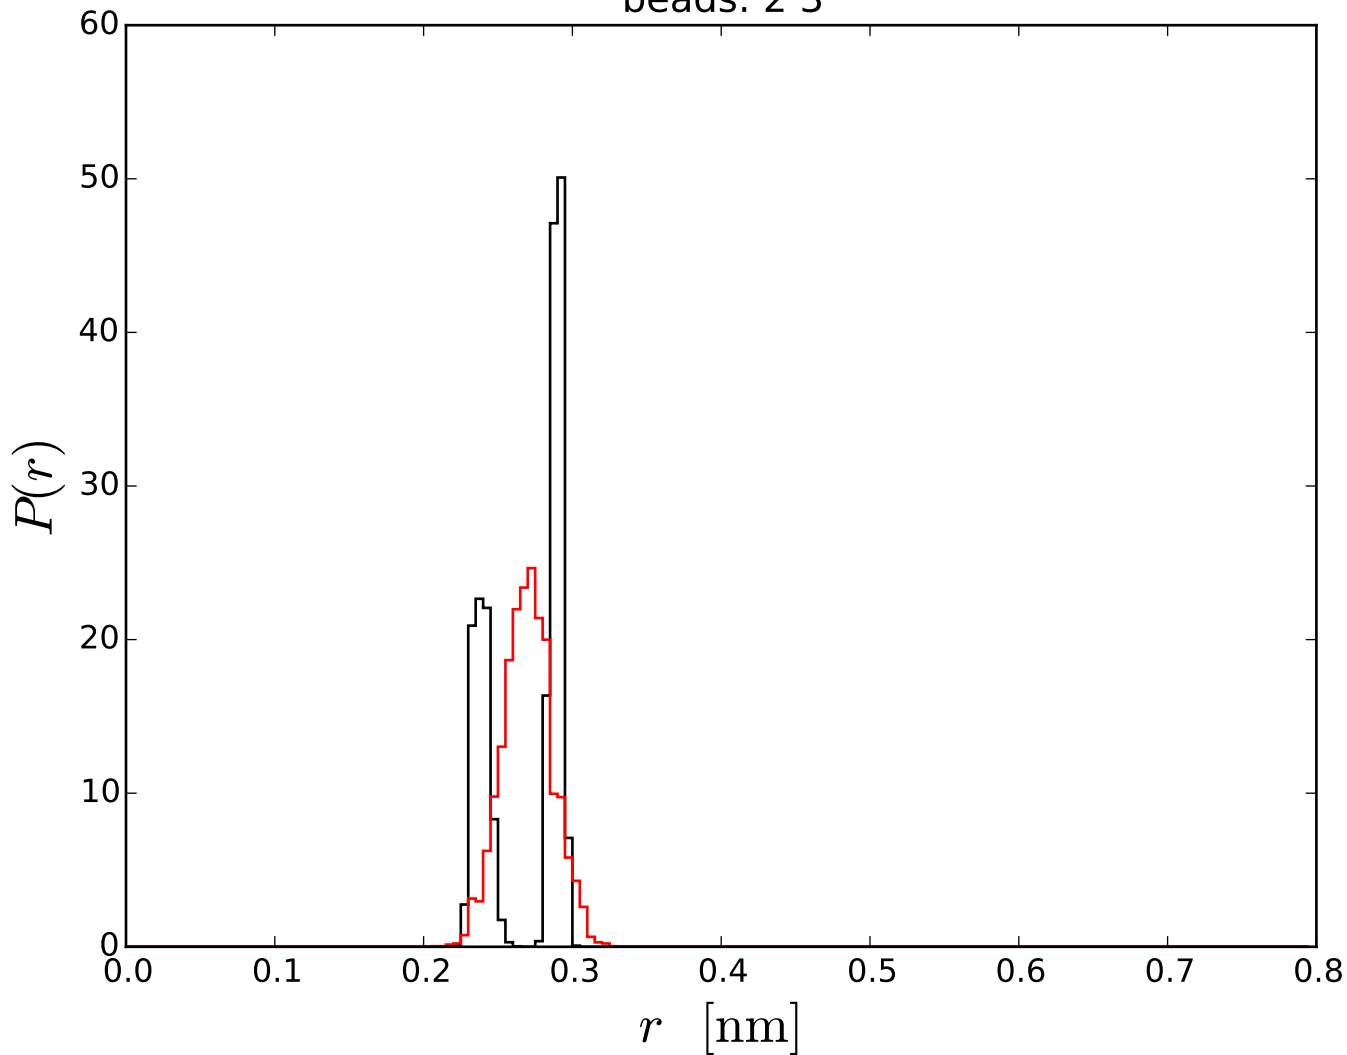

beads: 2 4

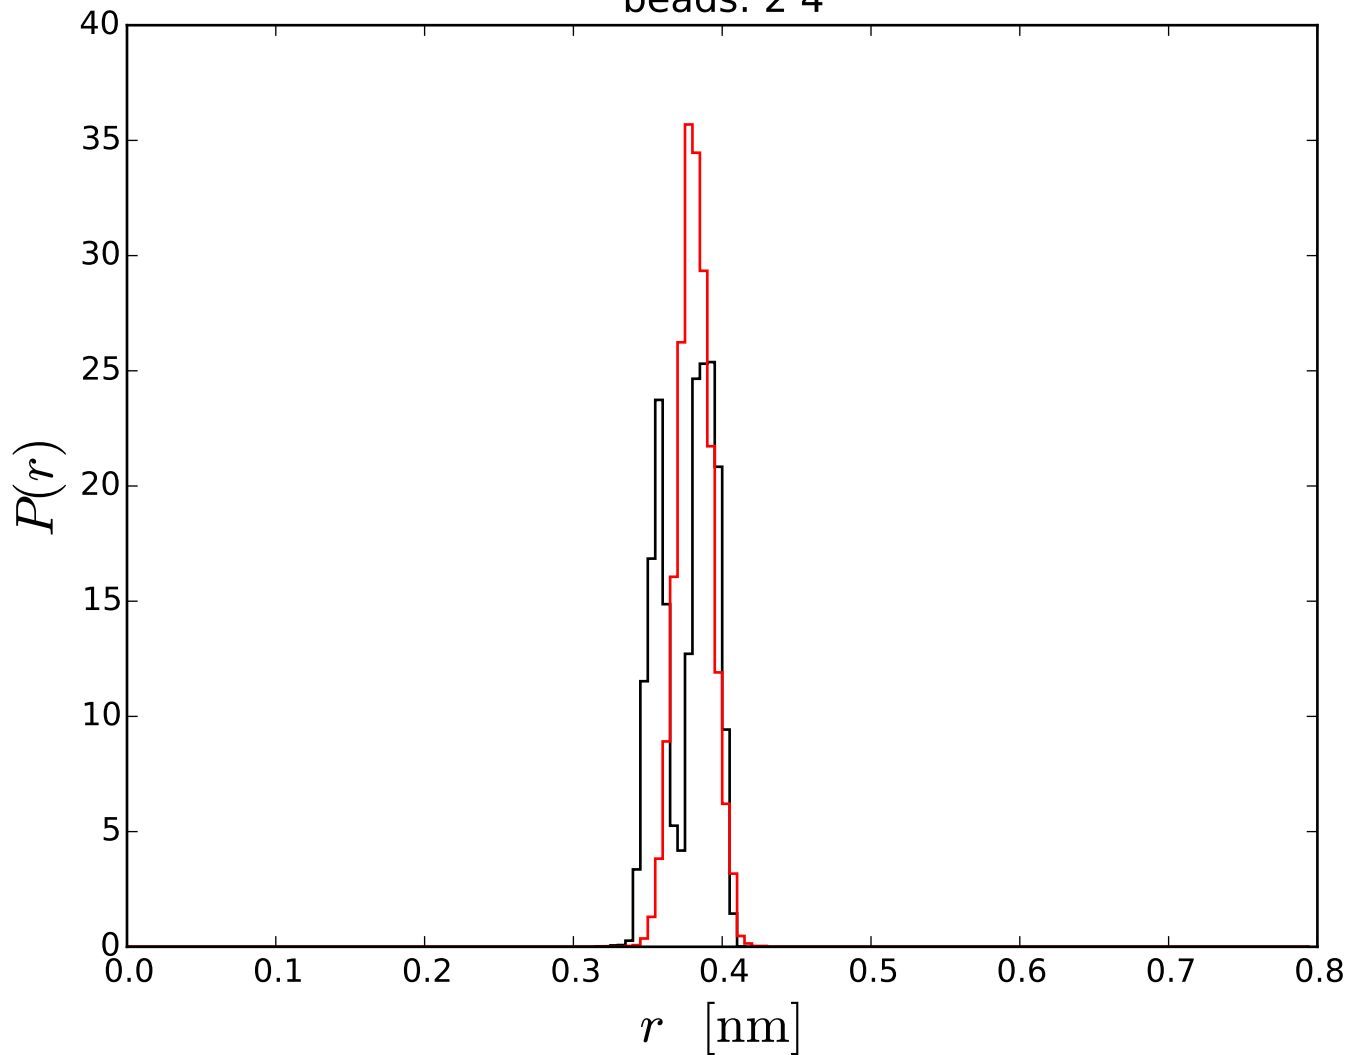

beads: 3 4

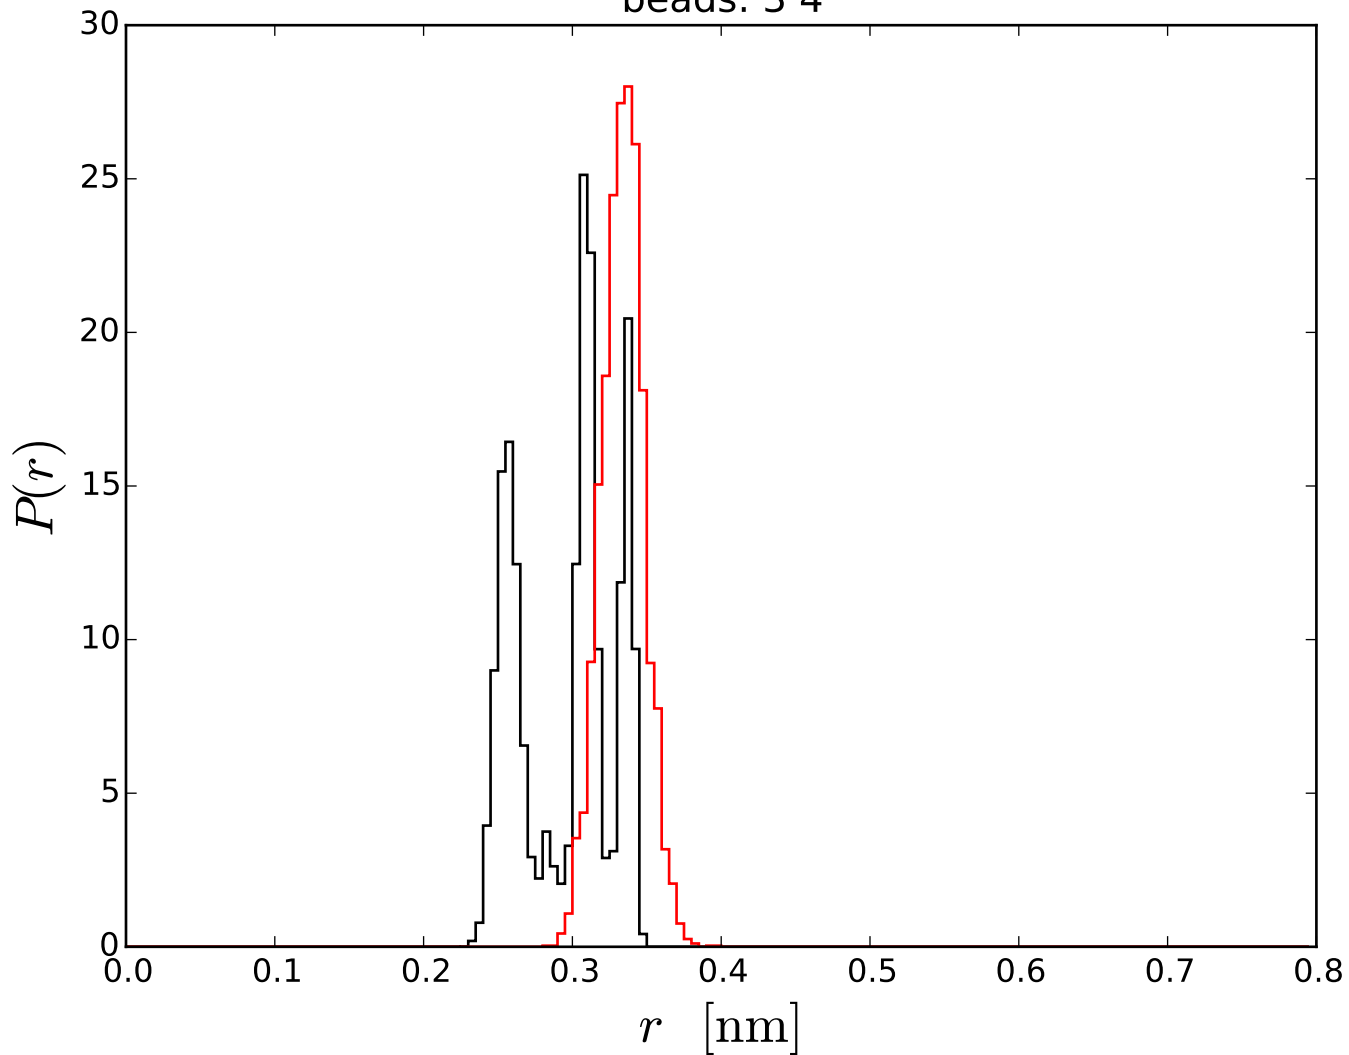

beads: 3 5

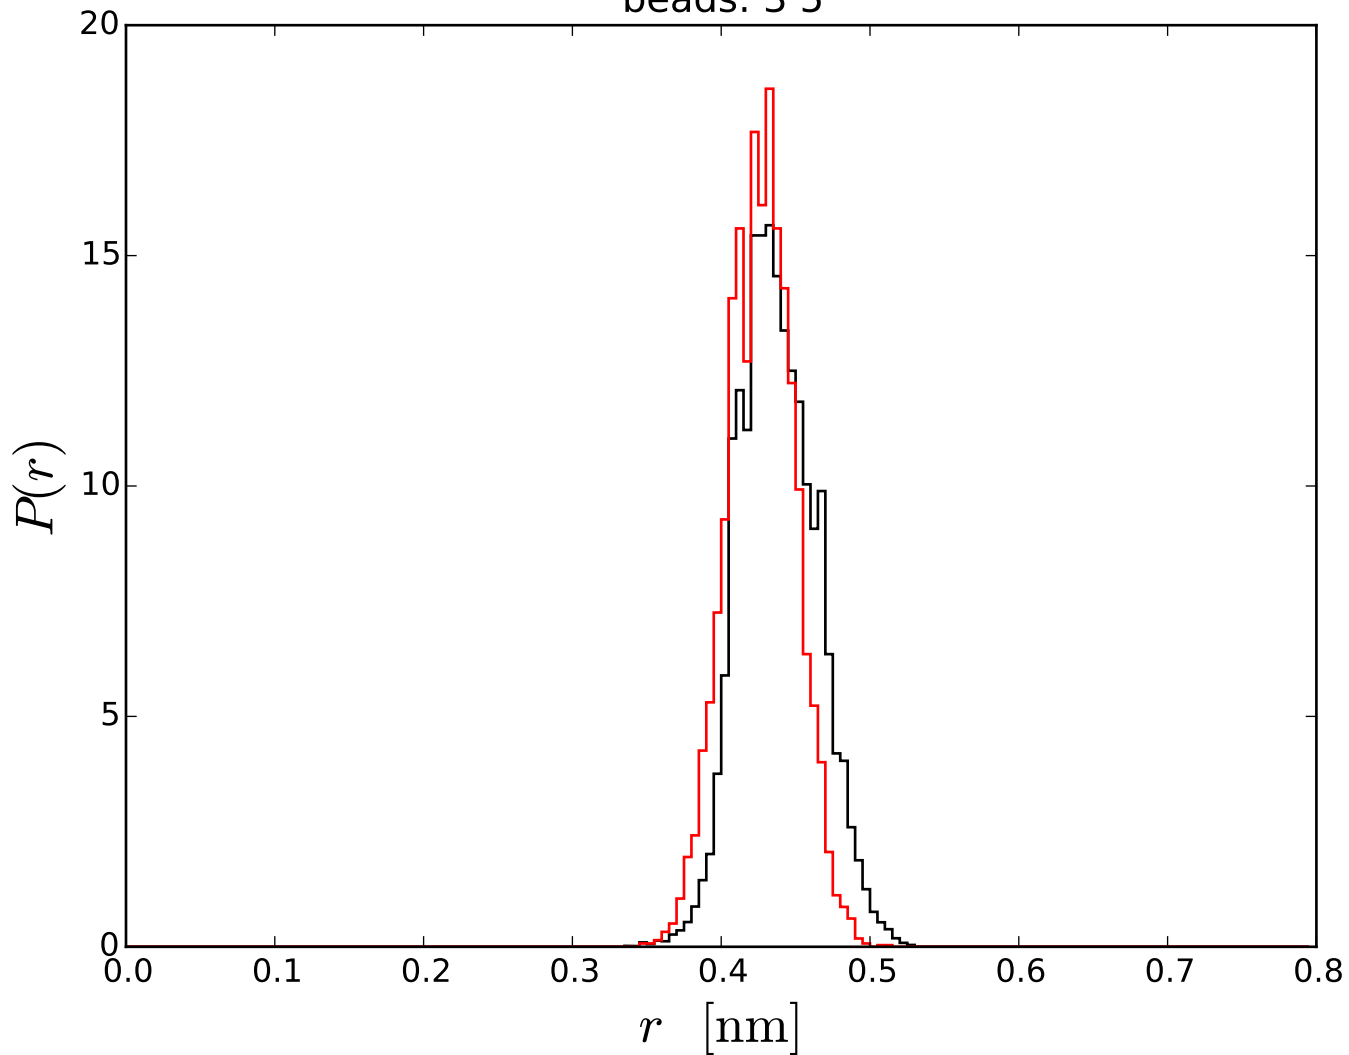

beads: 5 6

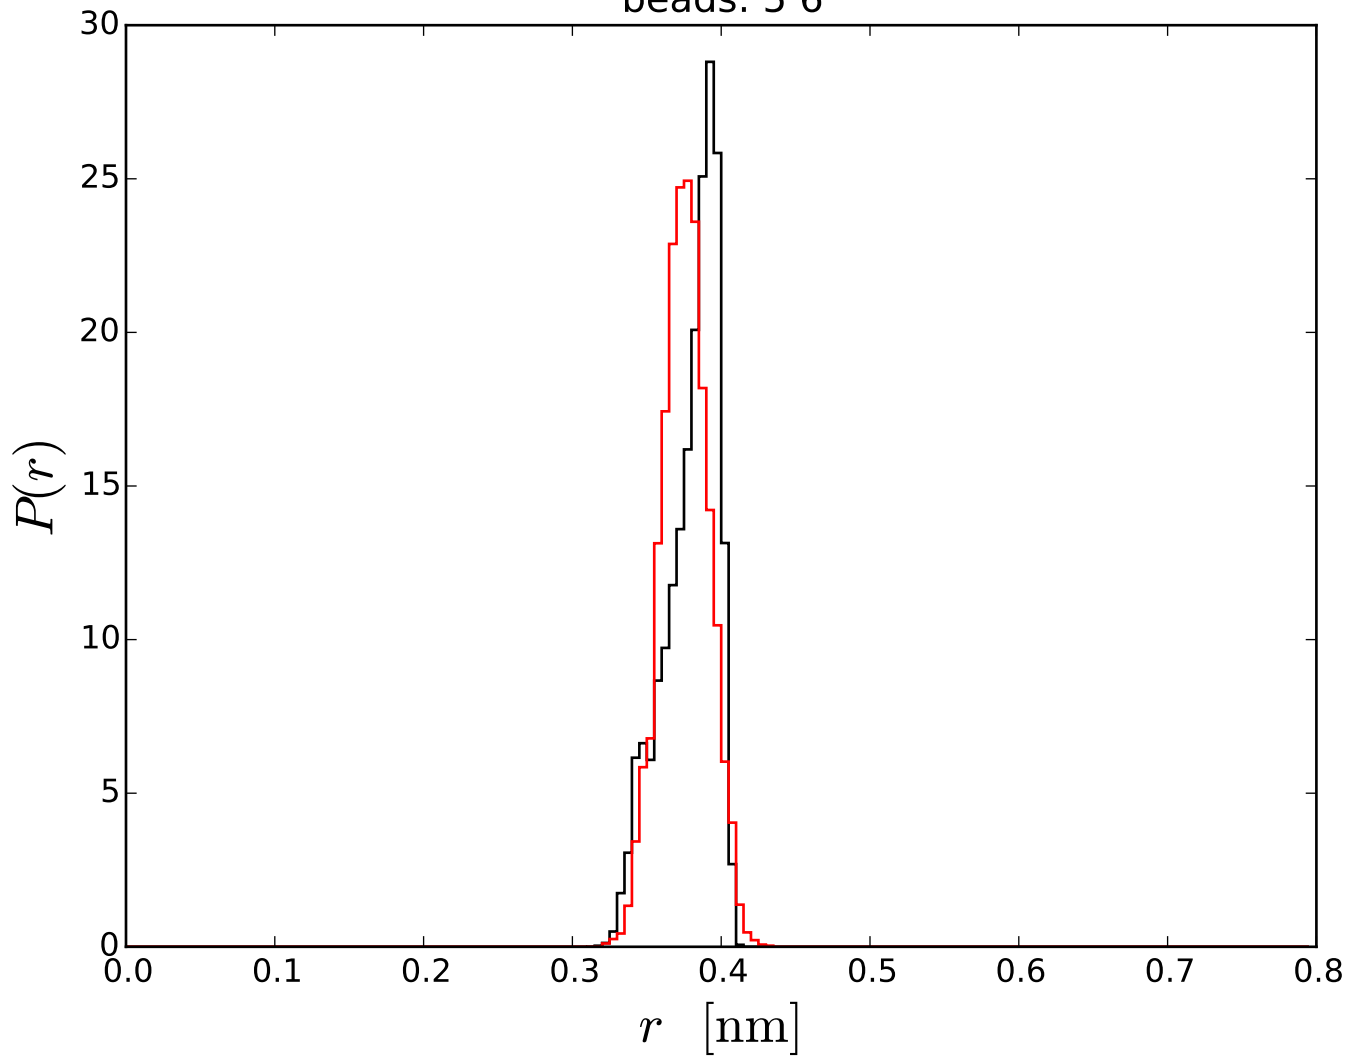

beads: 5 7

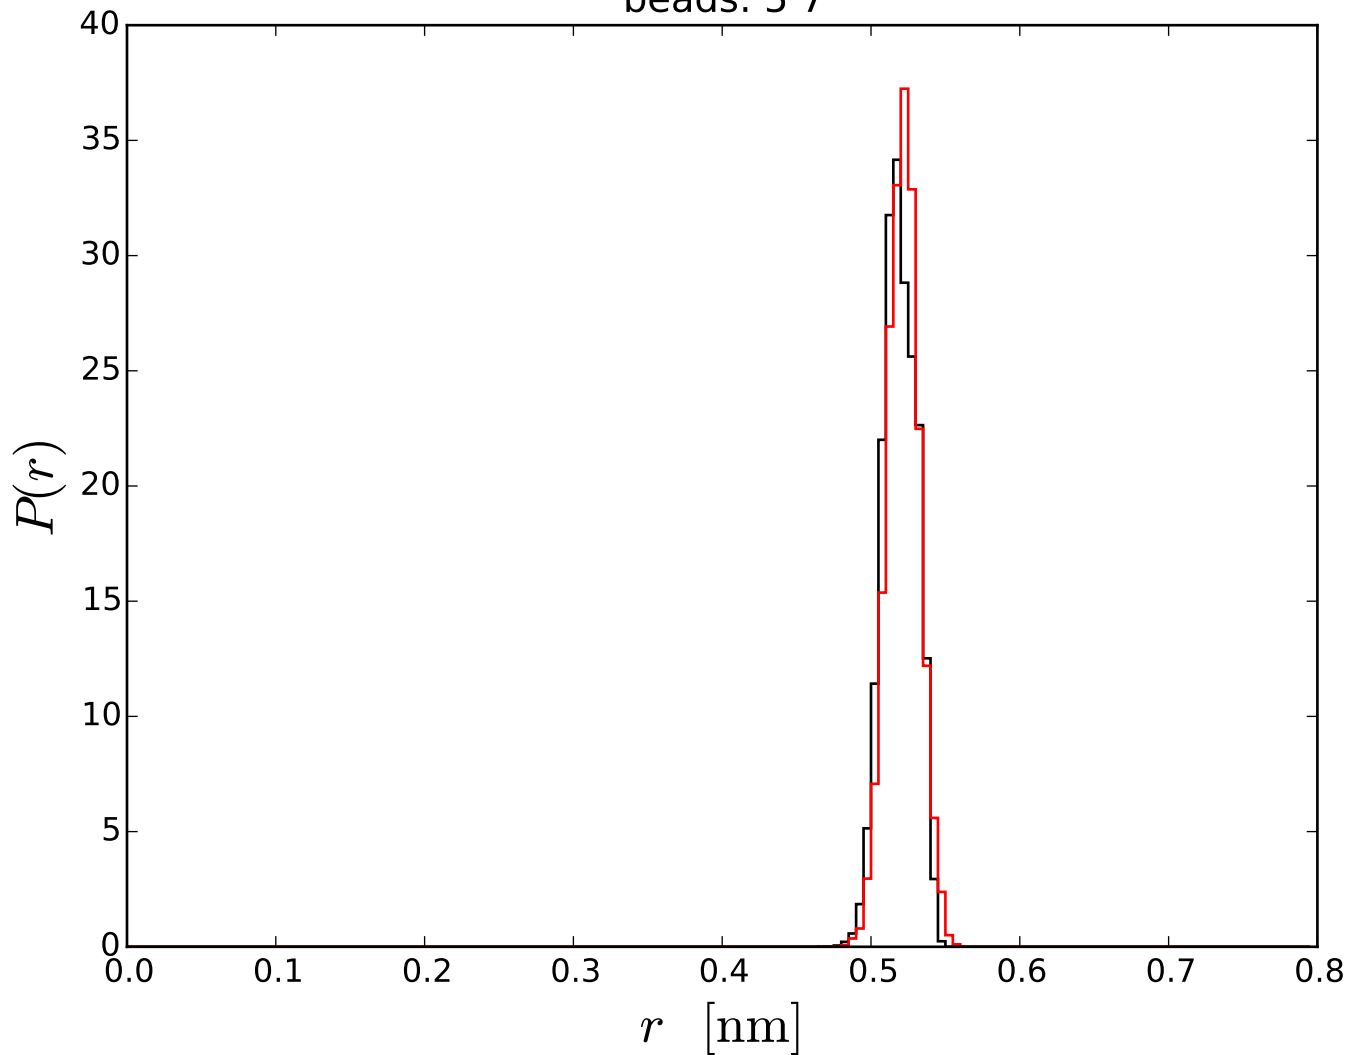

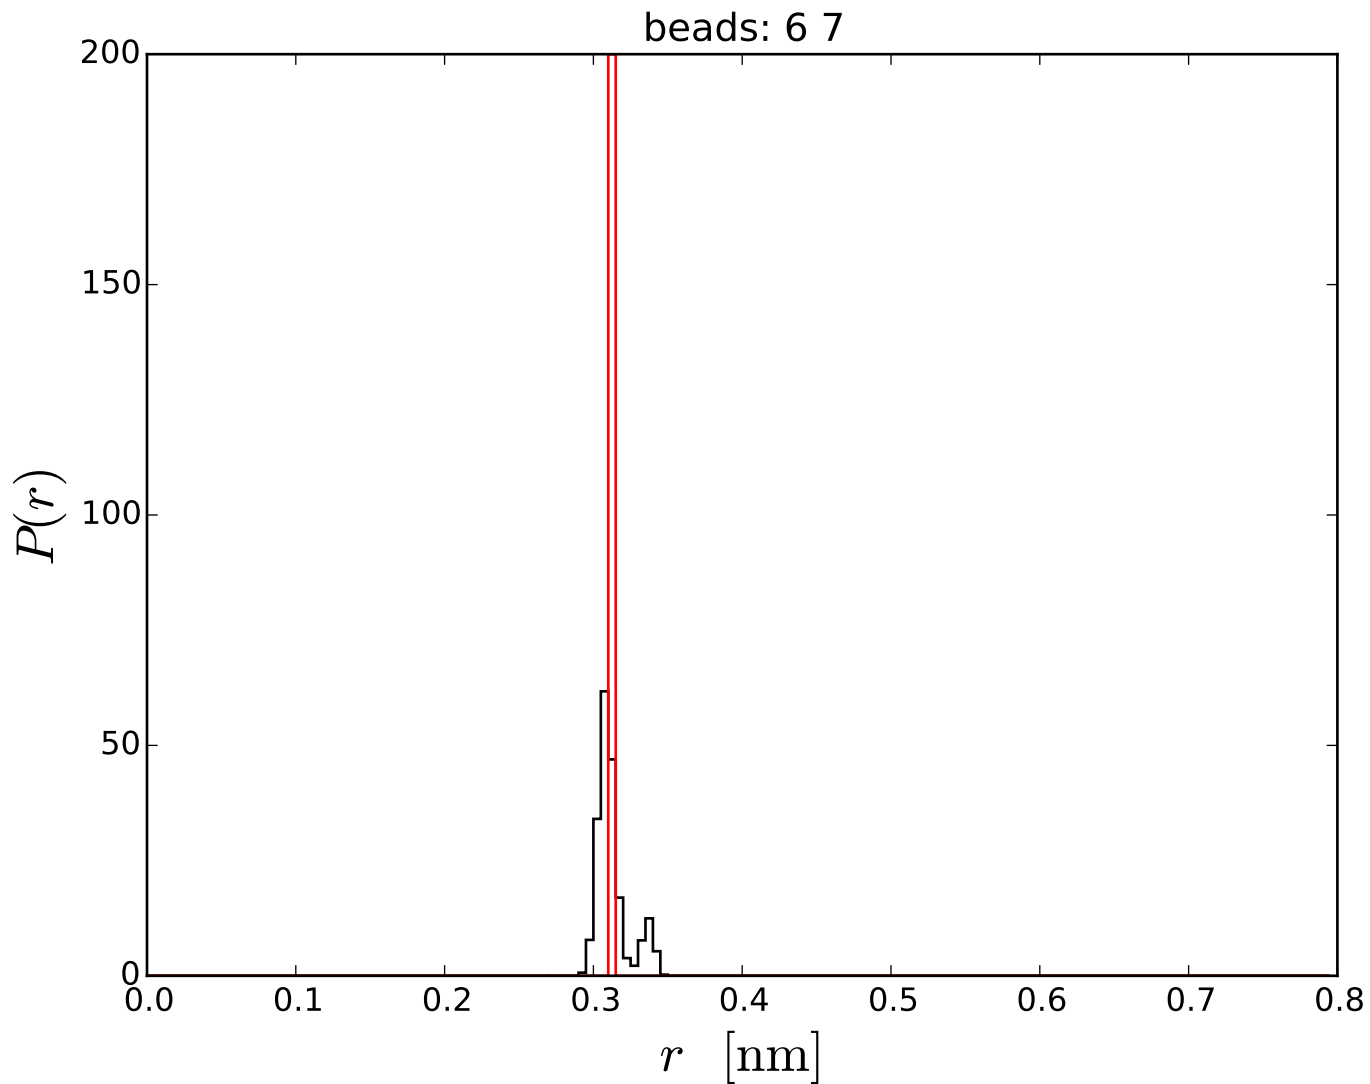



beads: 6 8

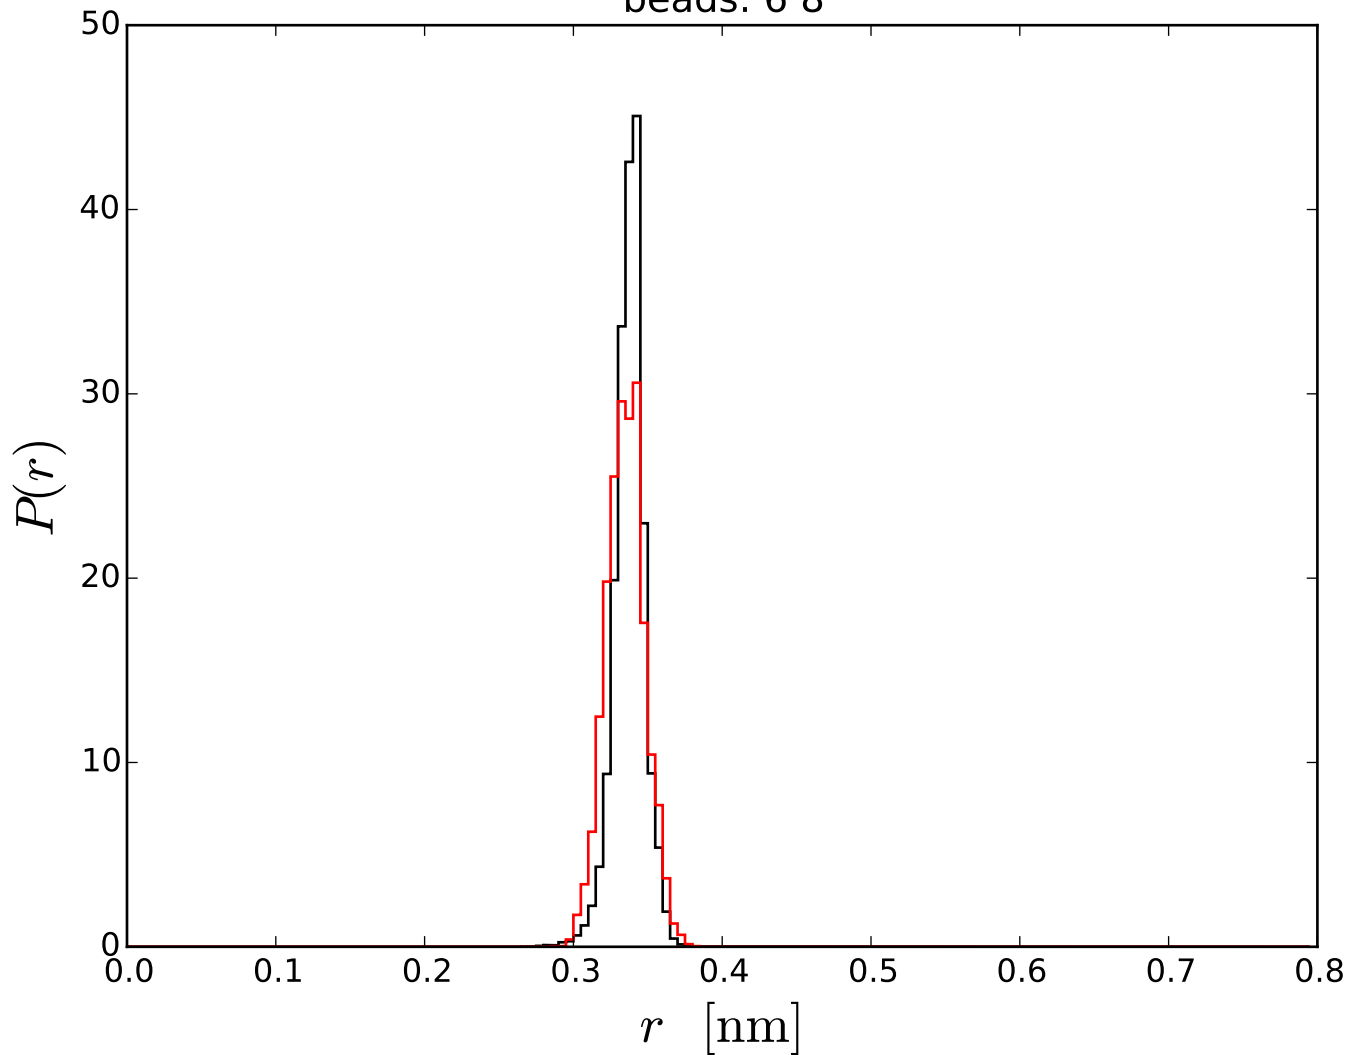

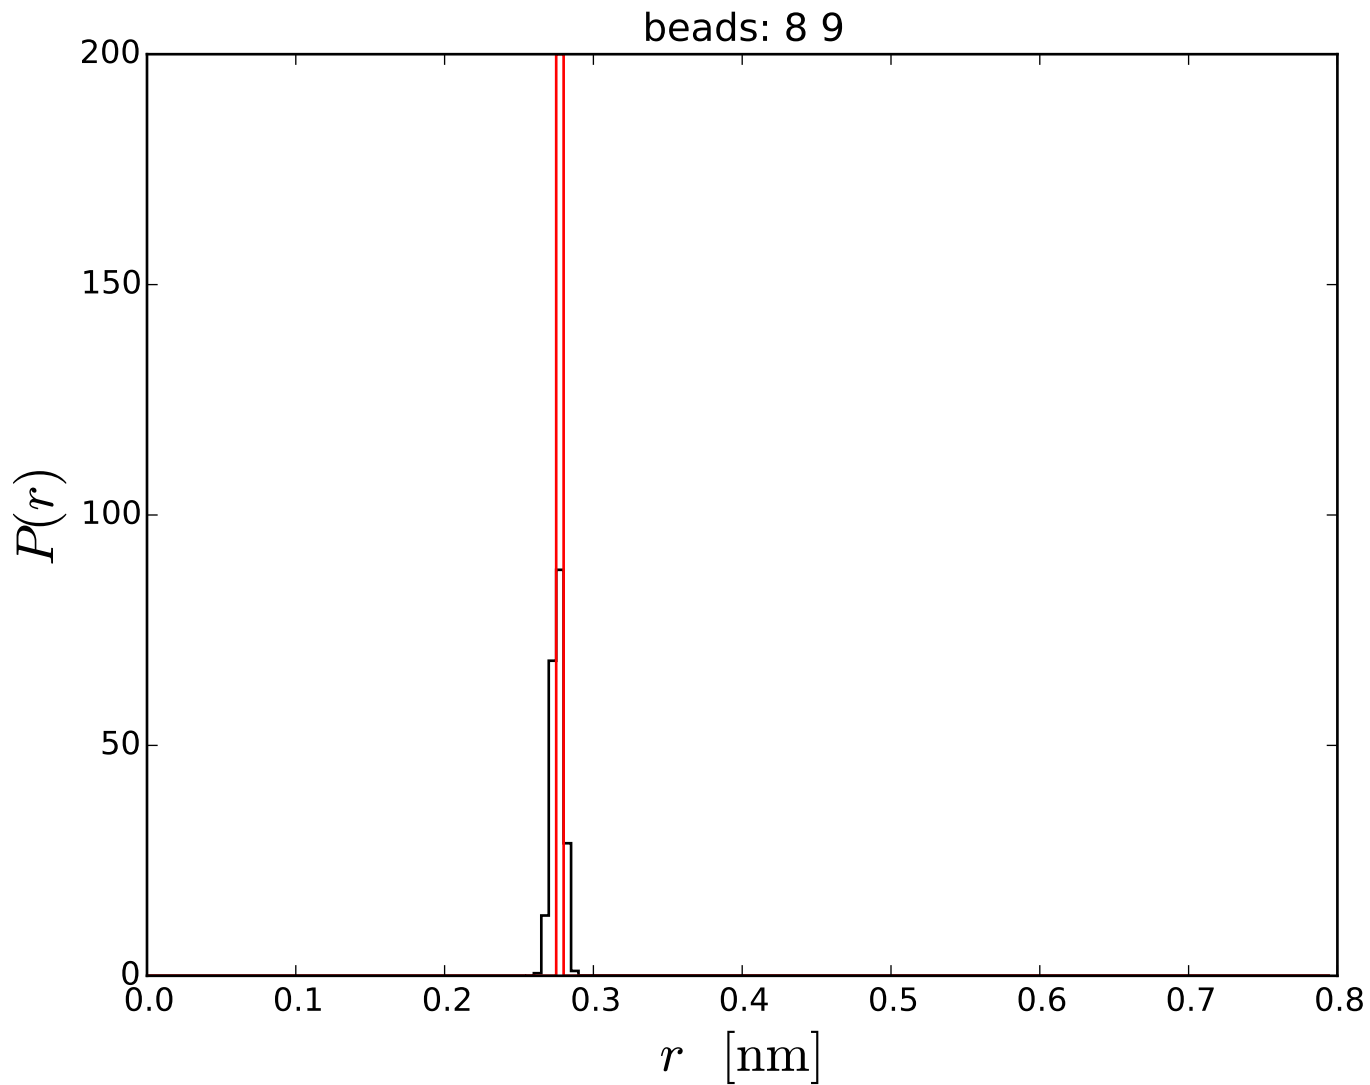

beads: 8 10

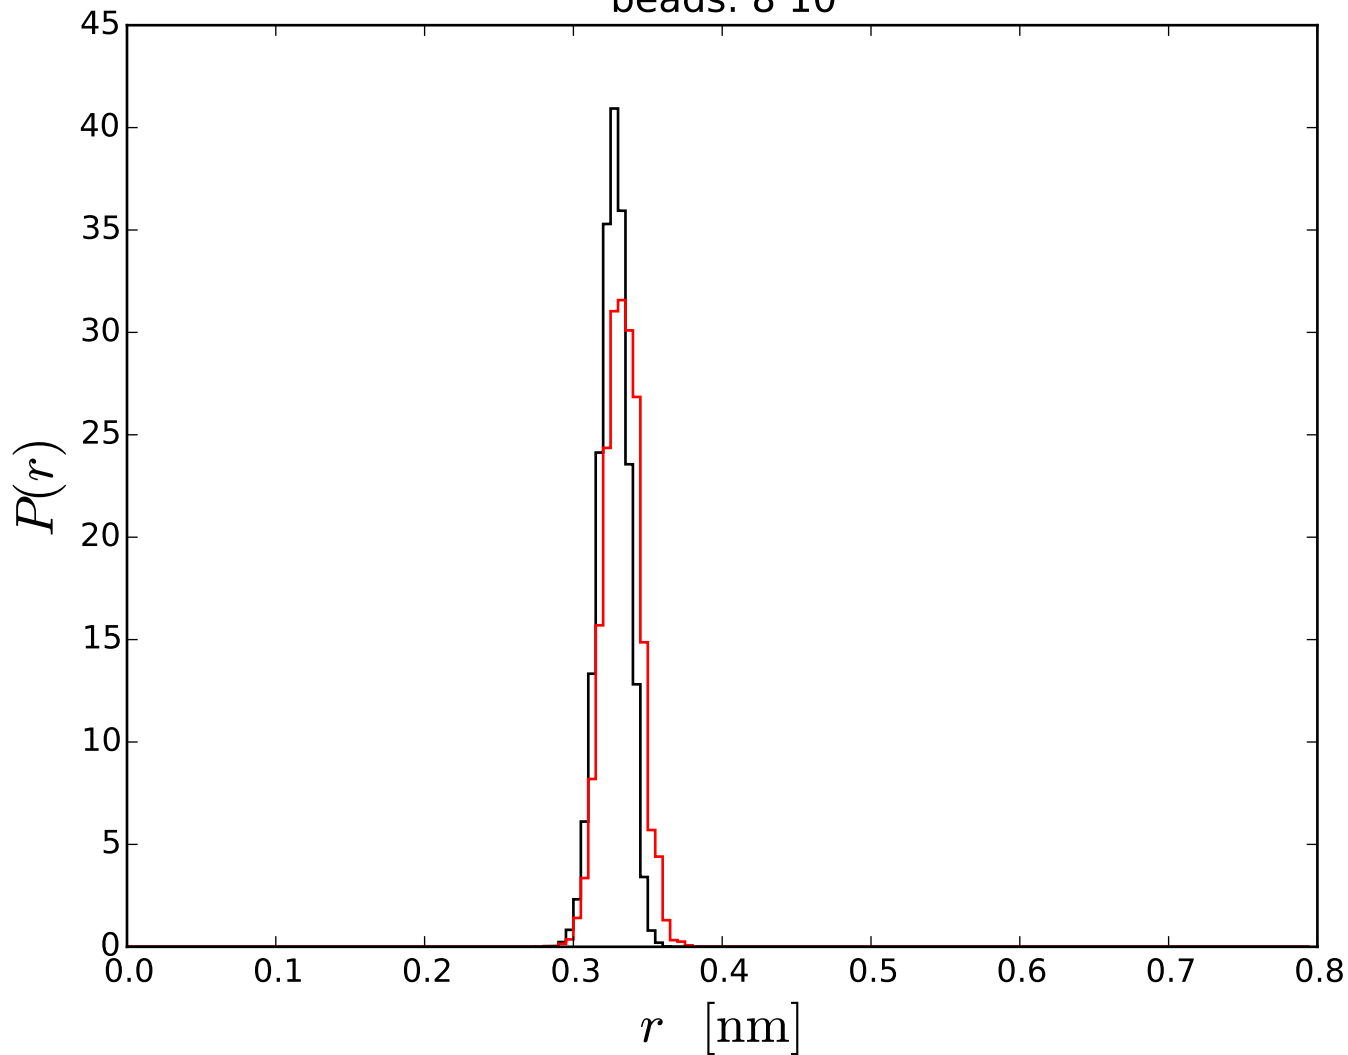

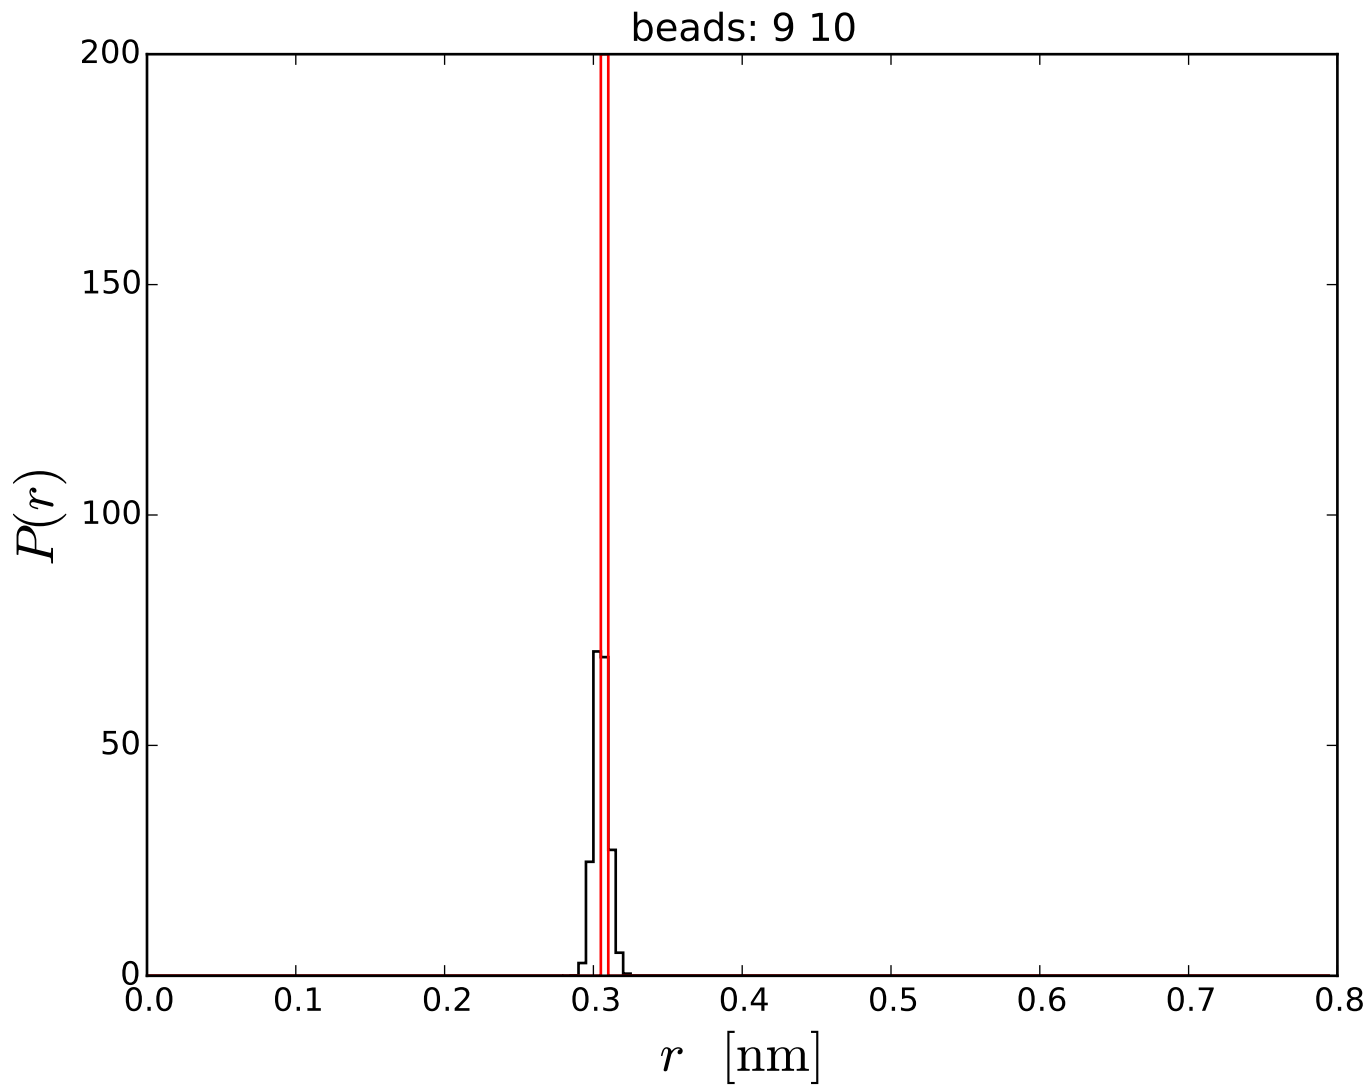

beads: 9 11

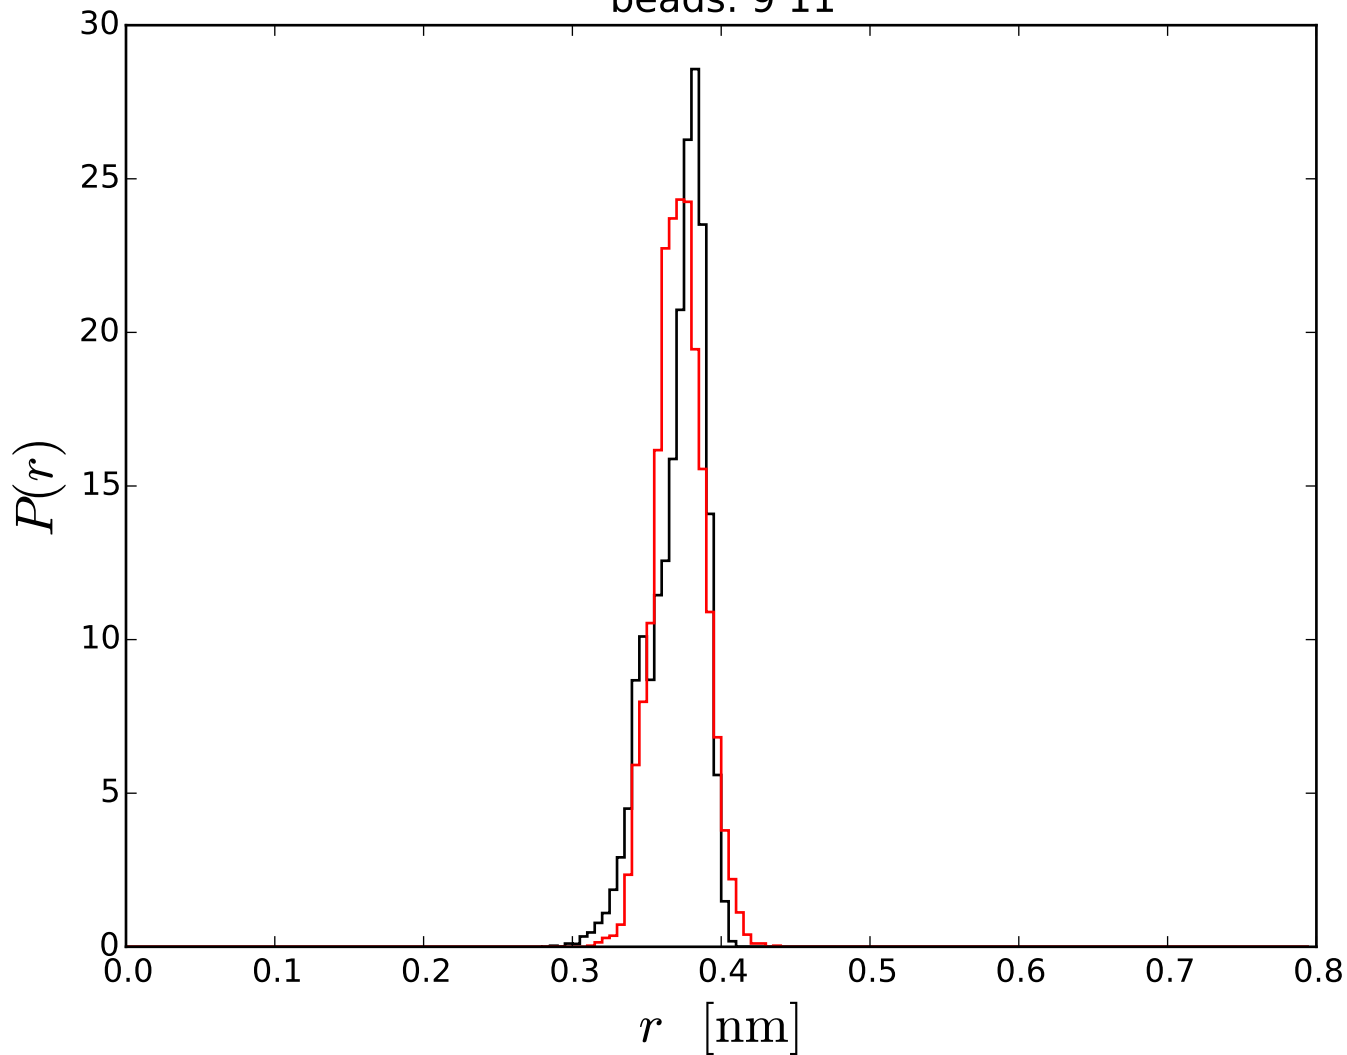

beads: 10 14

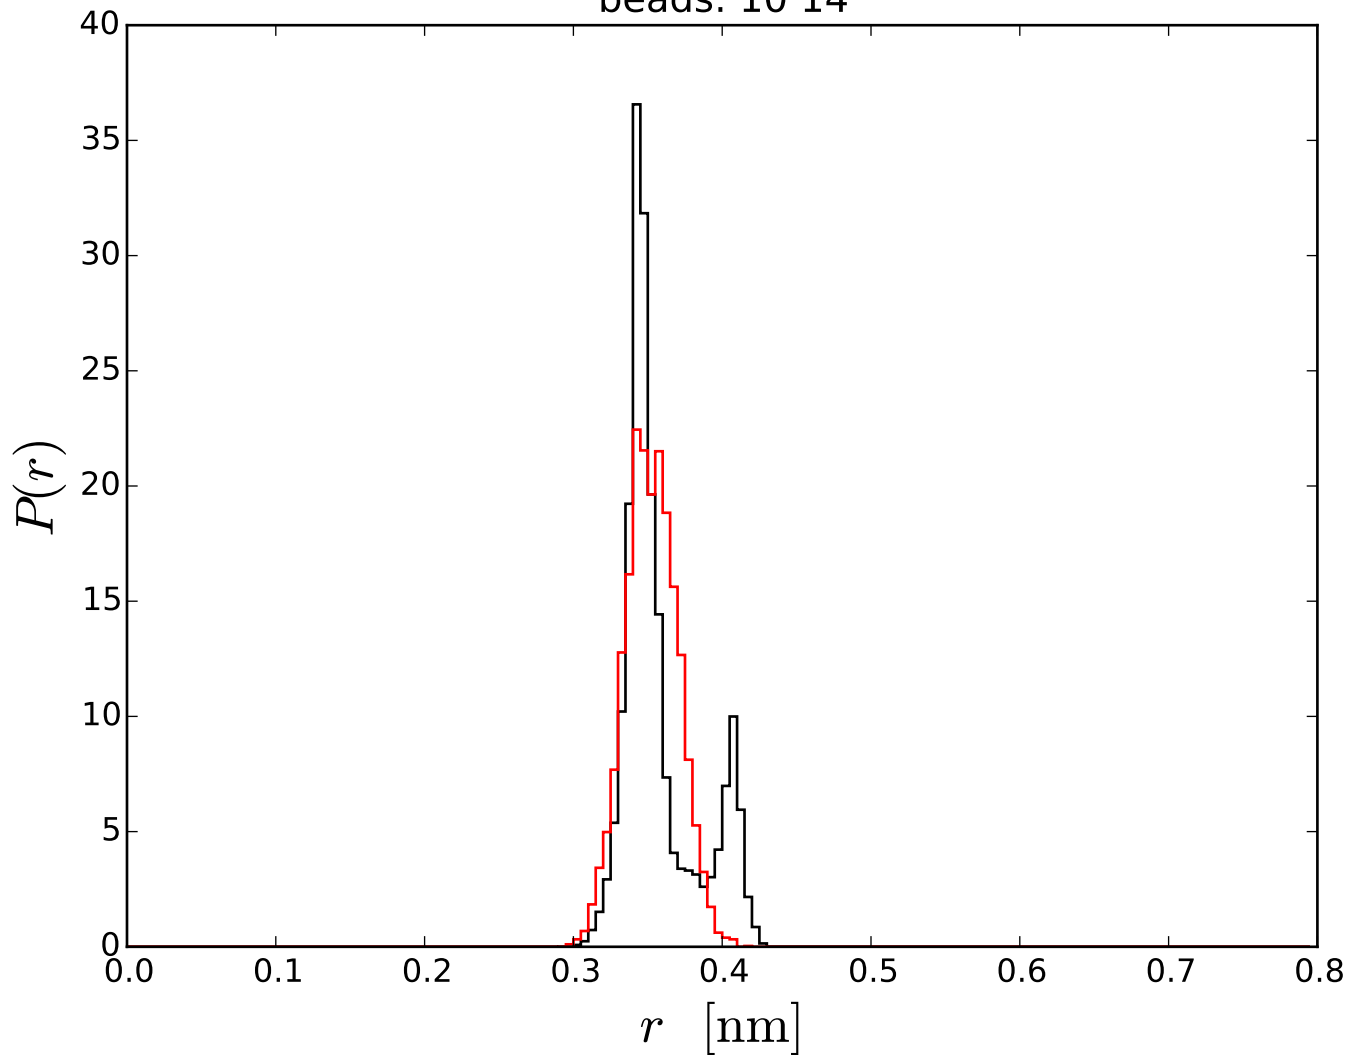

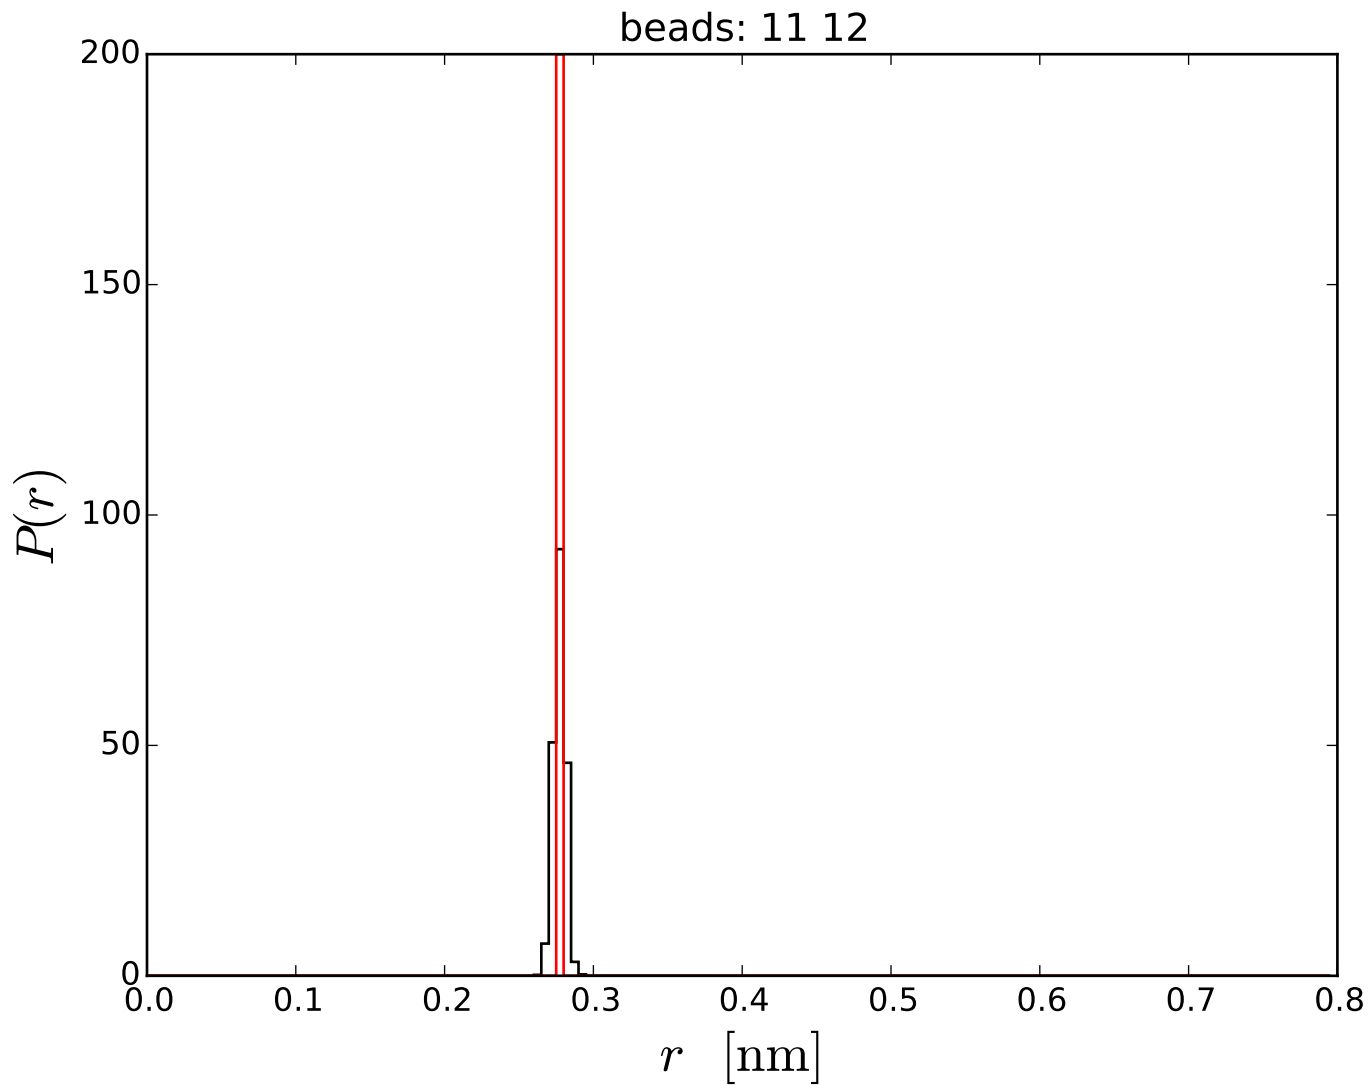

beads: 11 13

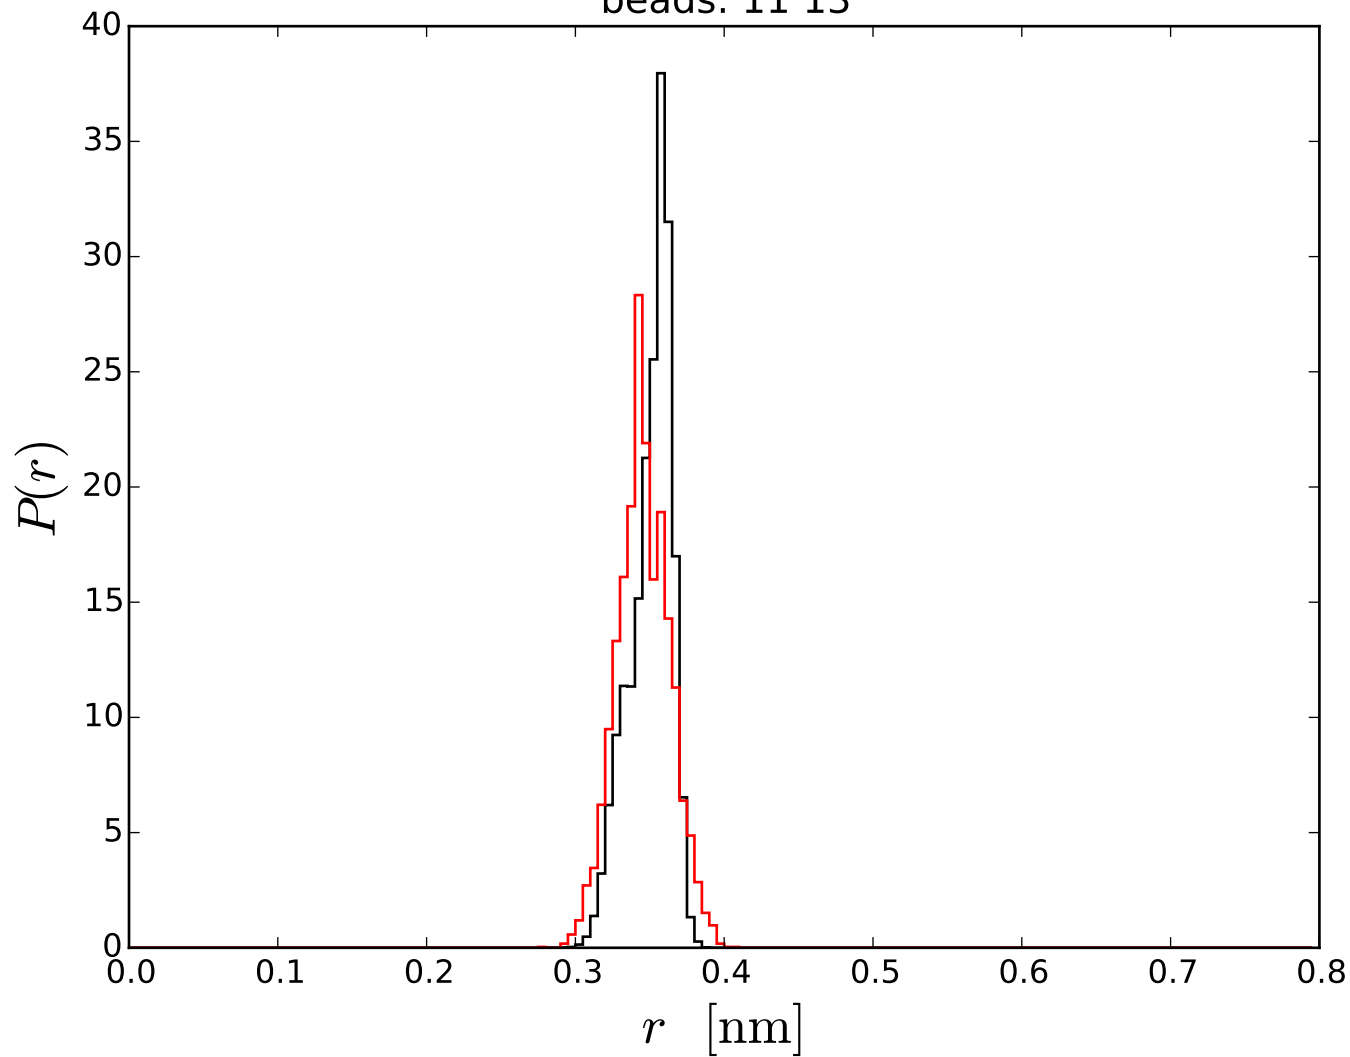



beads: 11 17

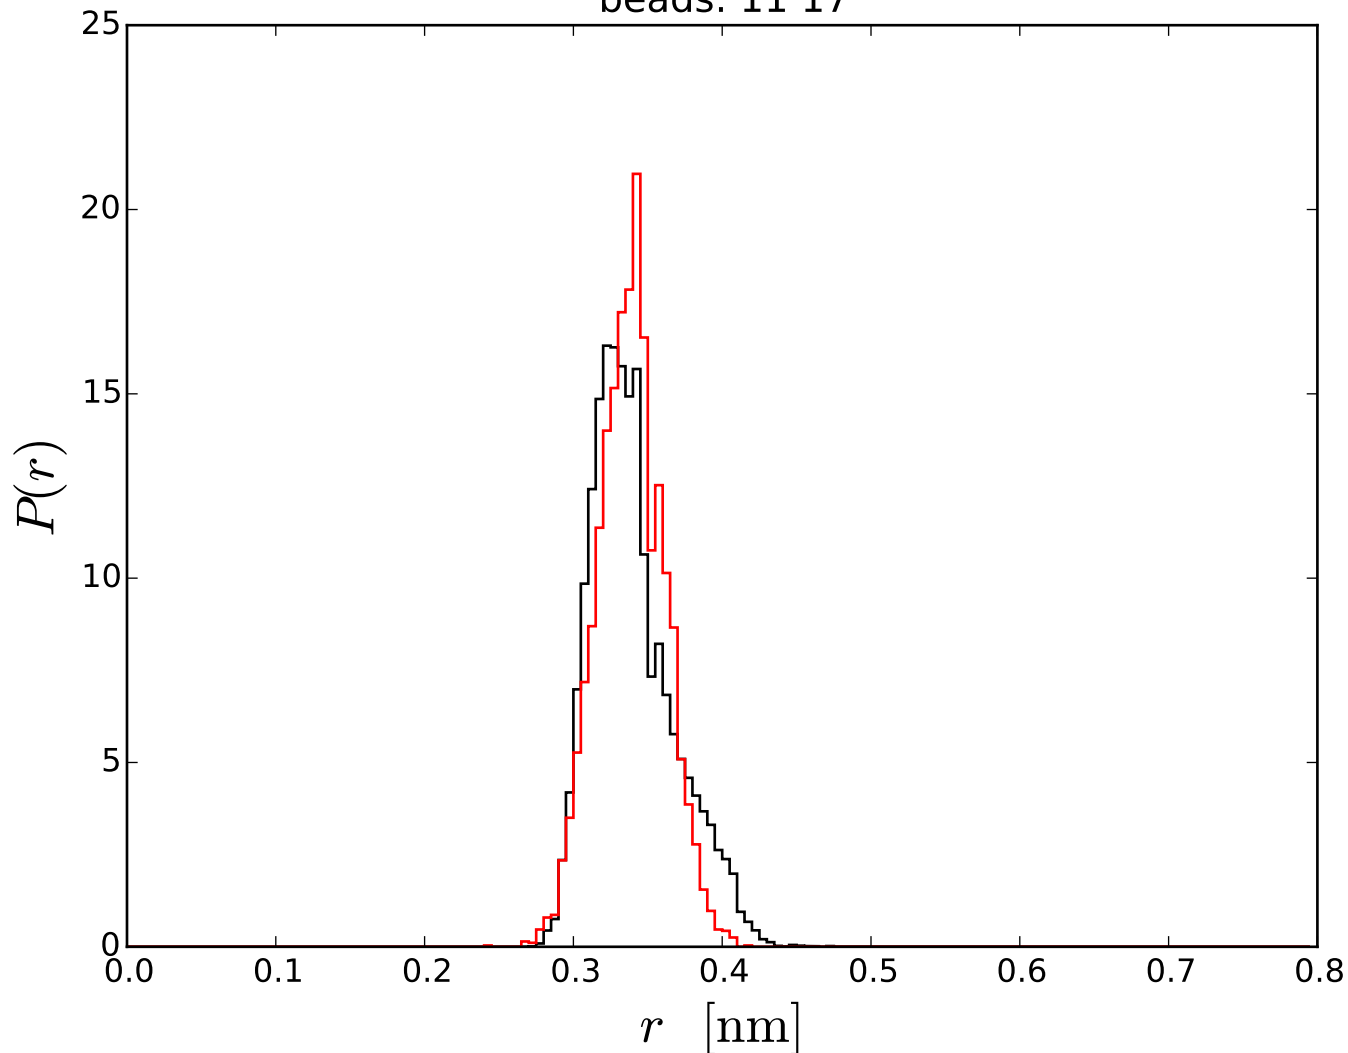

beads: 12 13

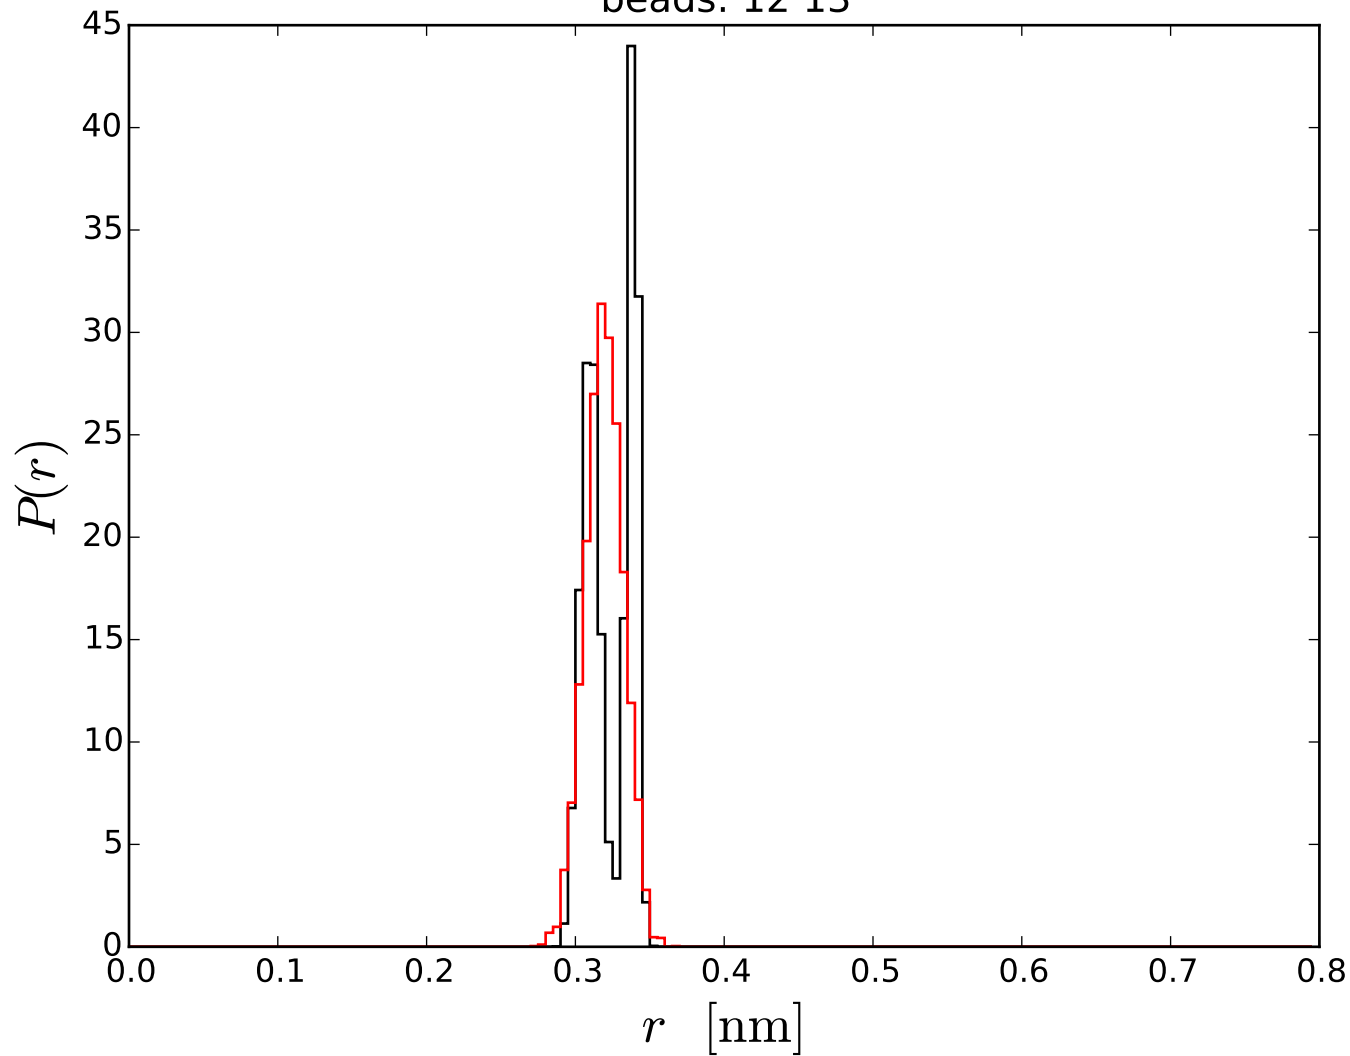

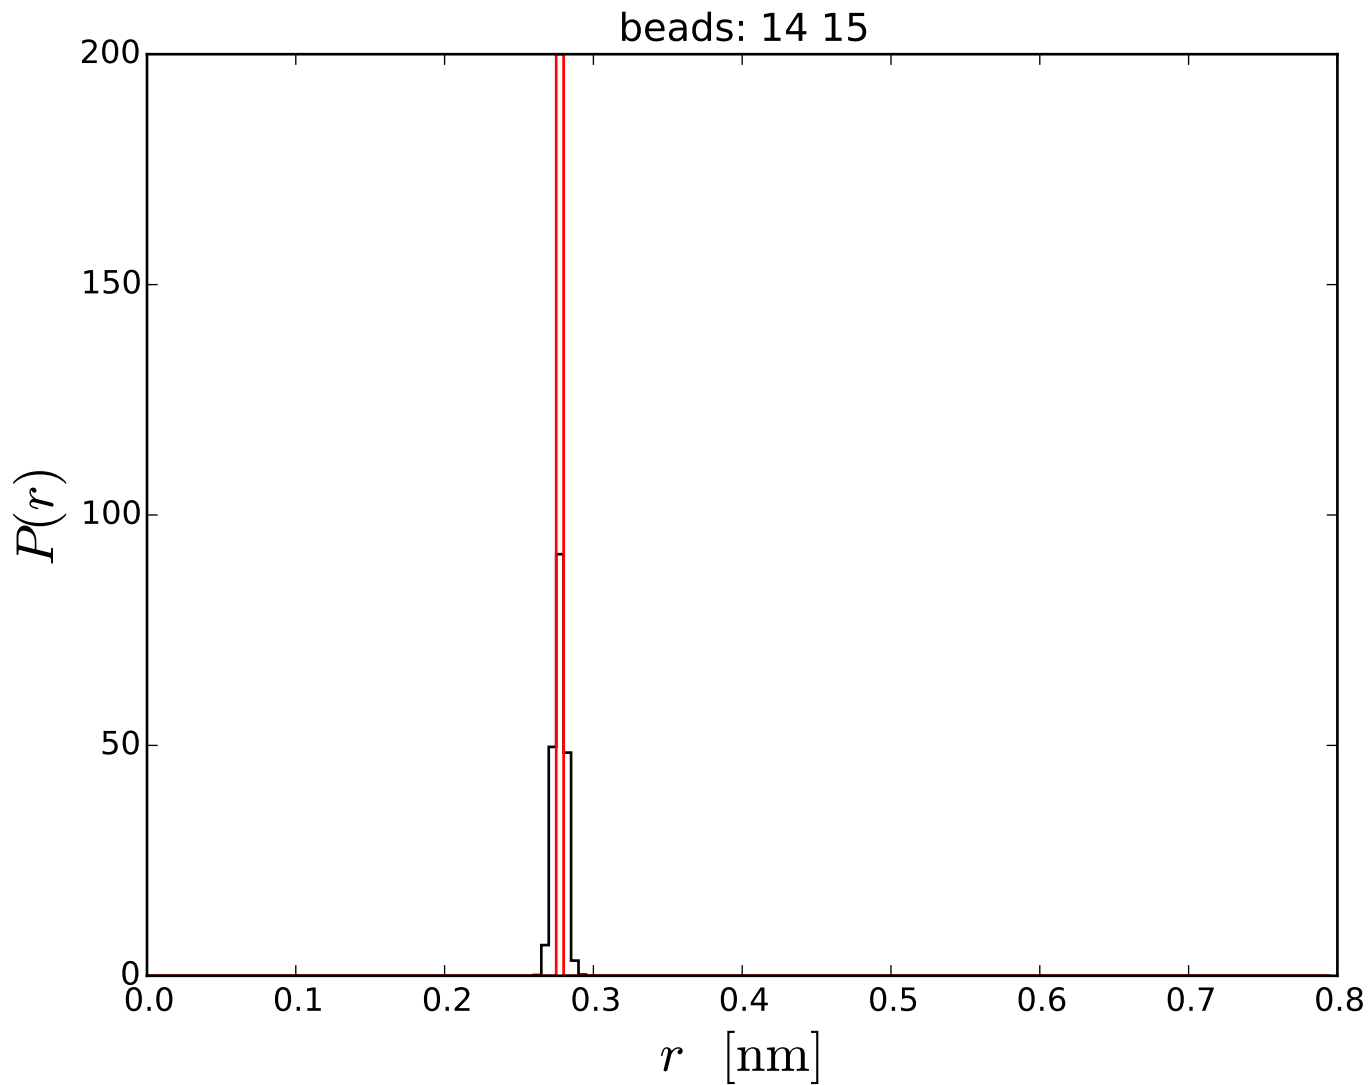

beads: 14 16

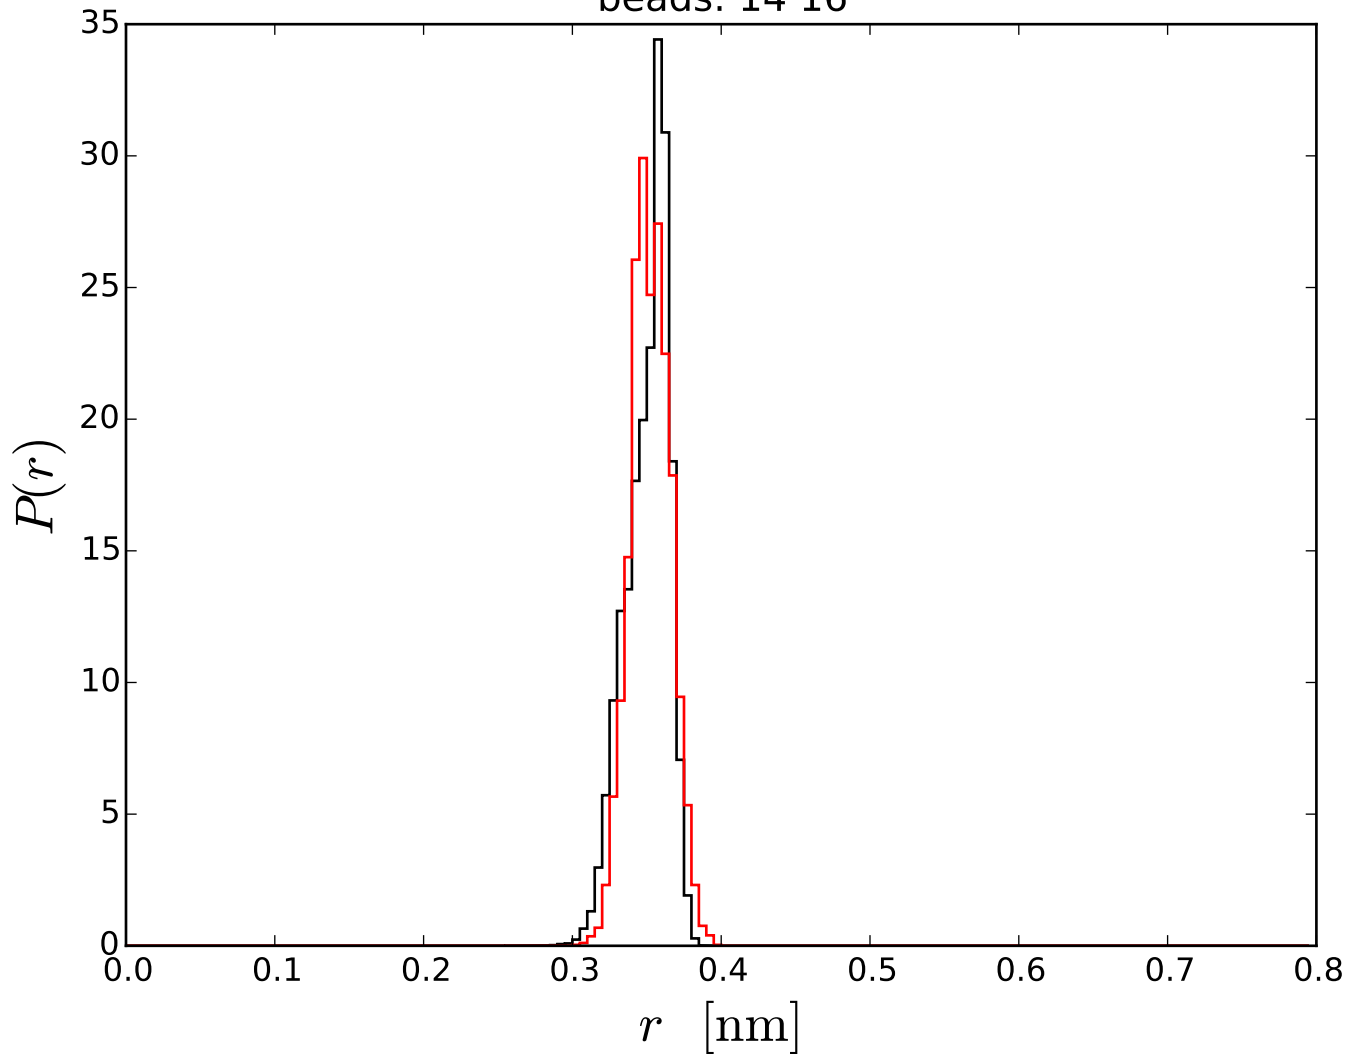

beads: 14 28

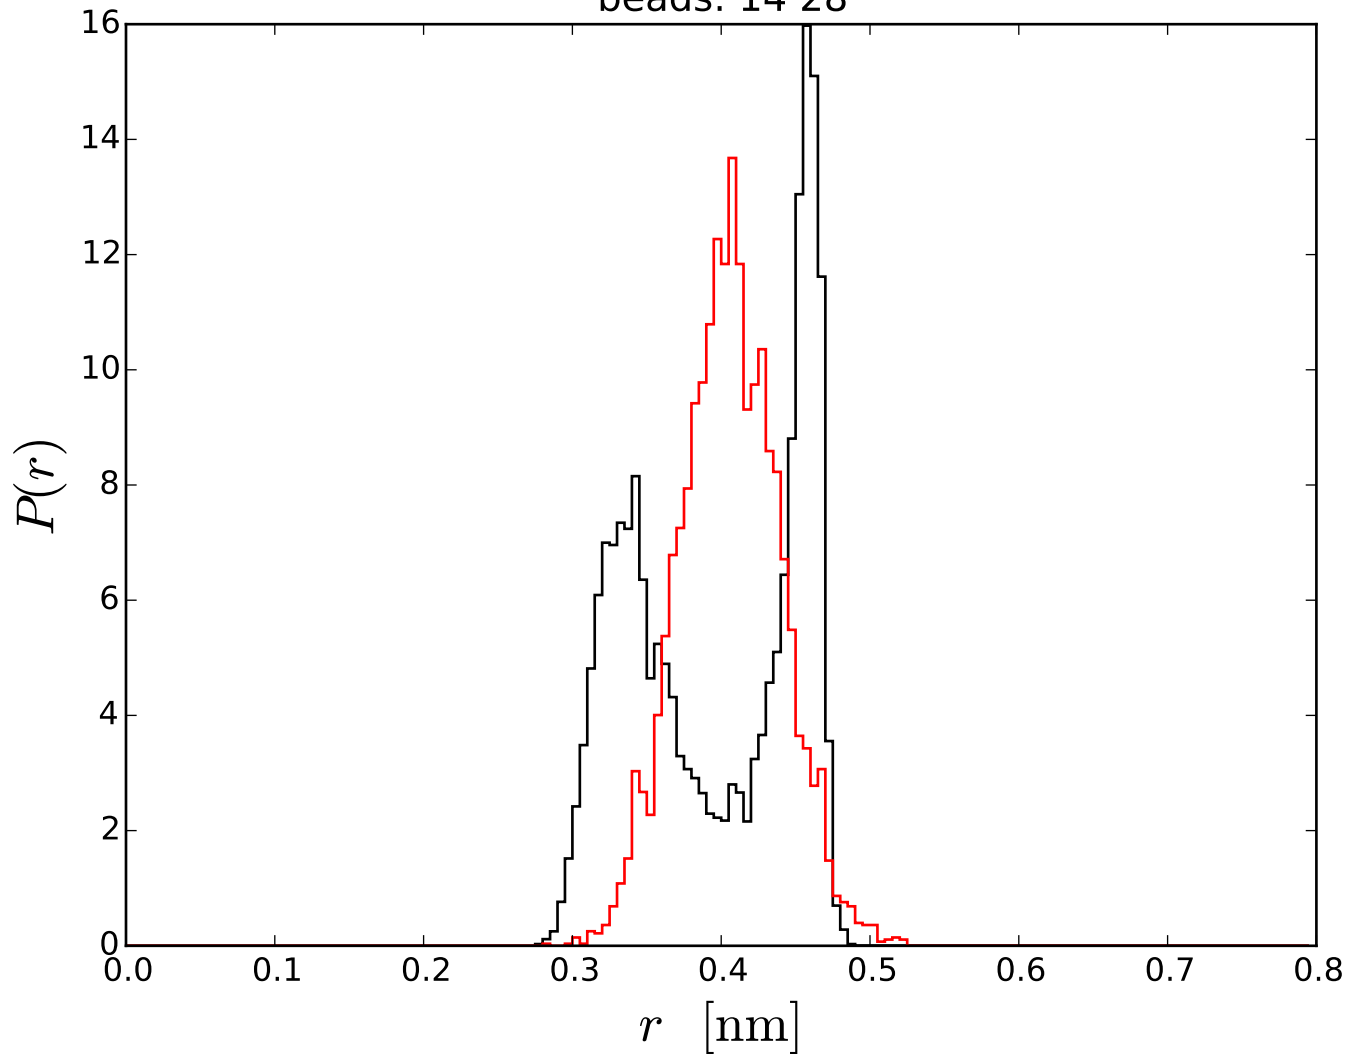

beads: 15 16

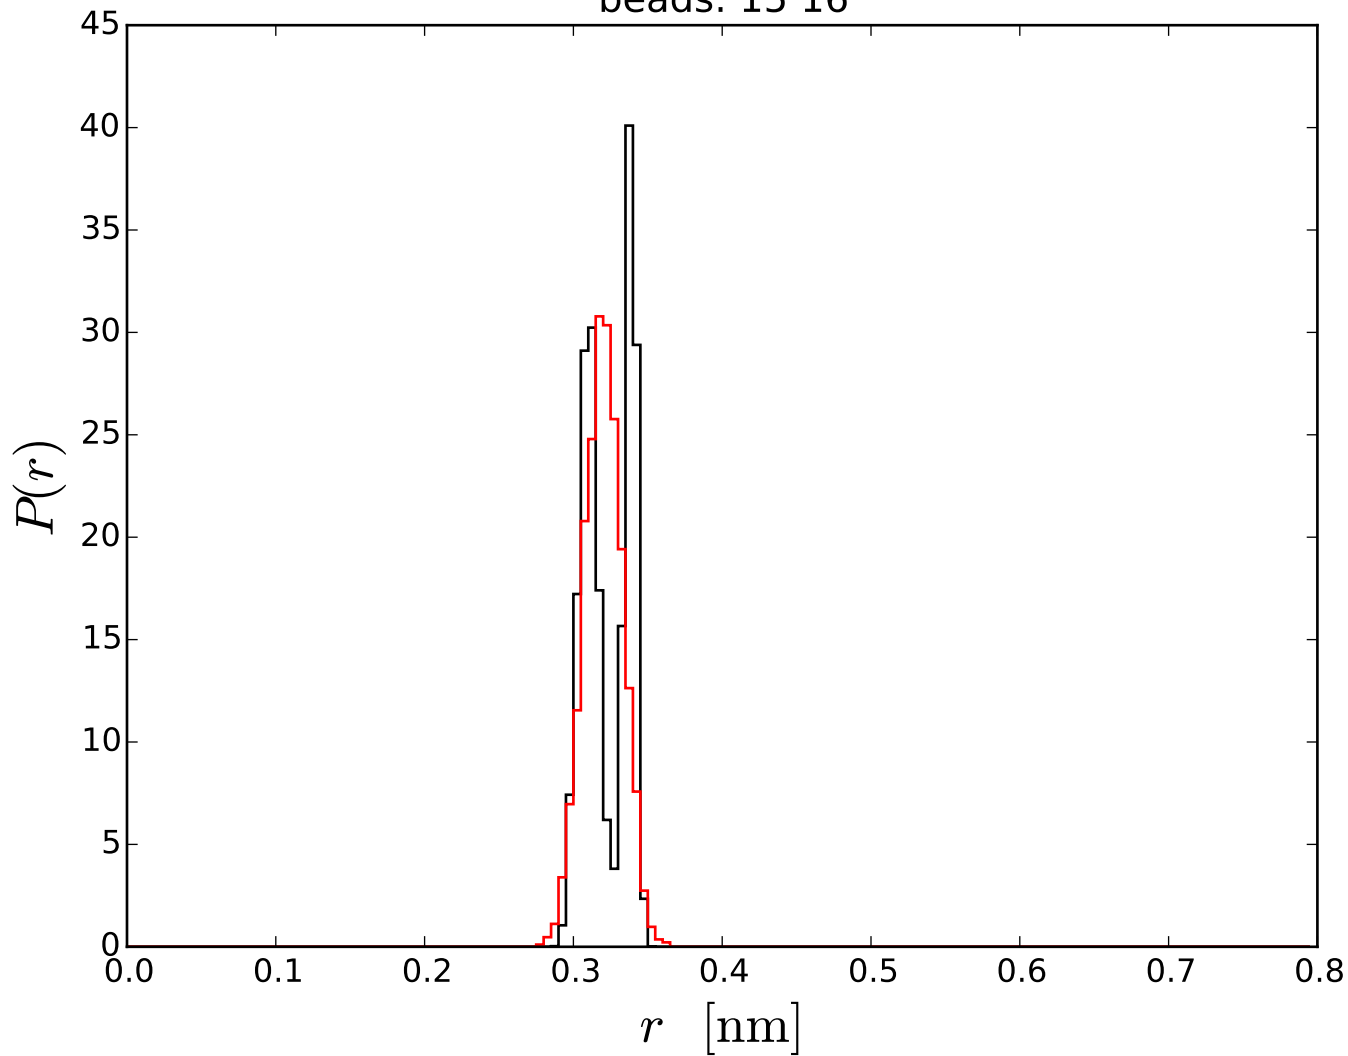

beads: 17 18

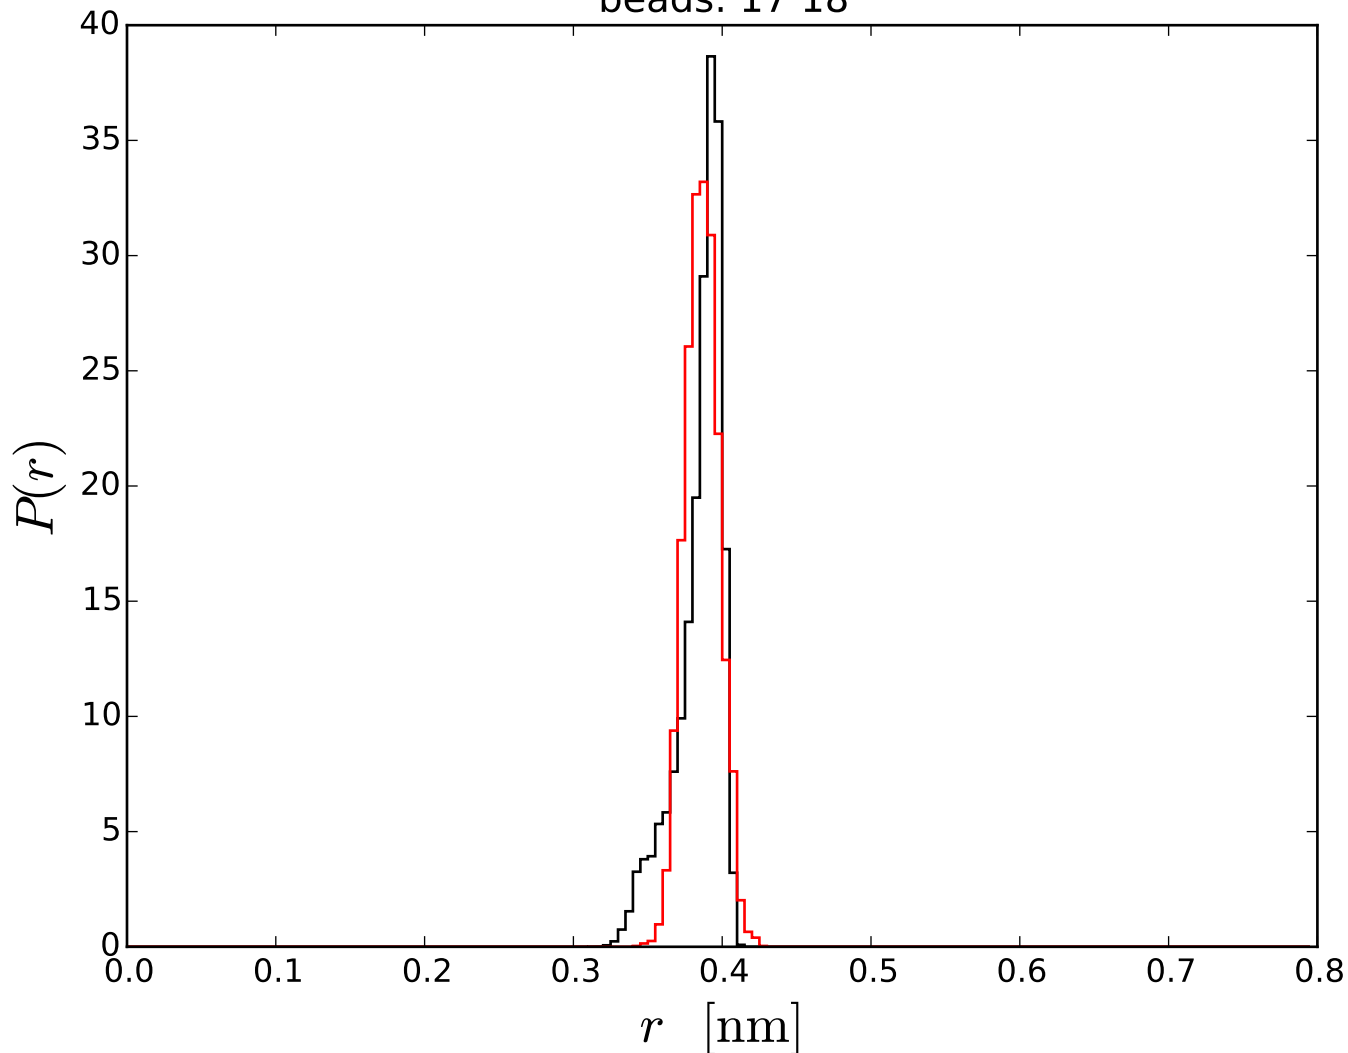

beads: 17 19

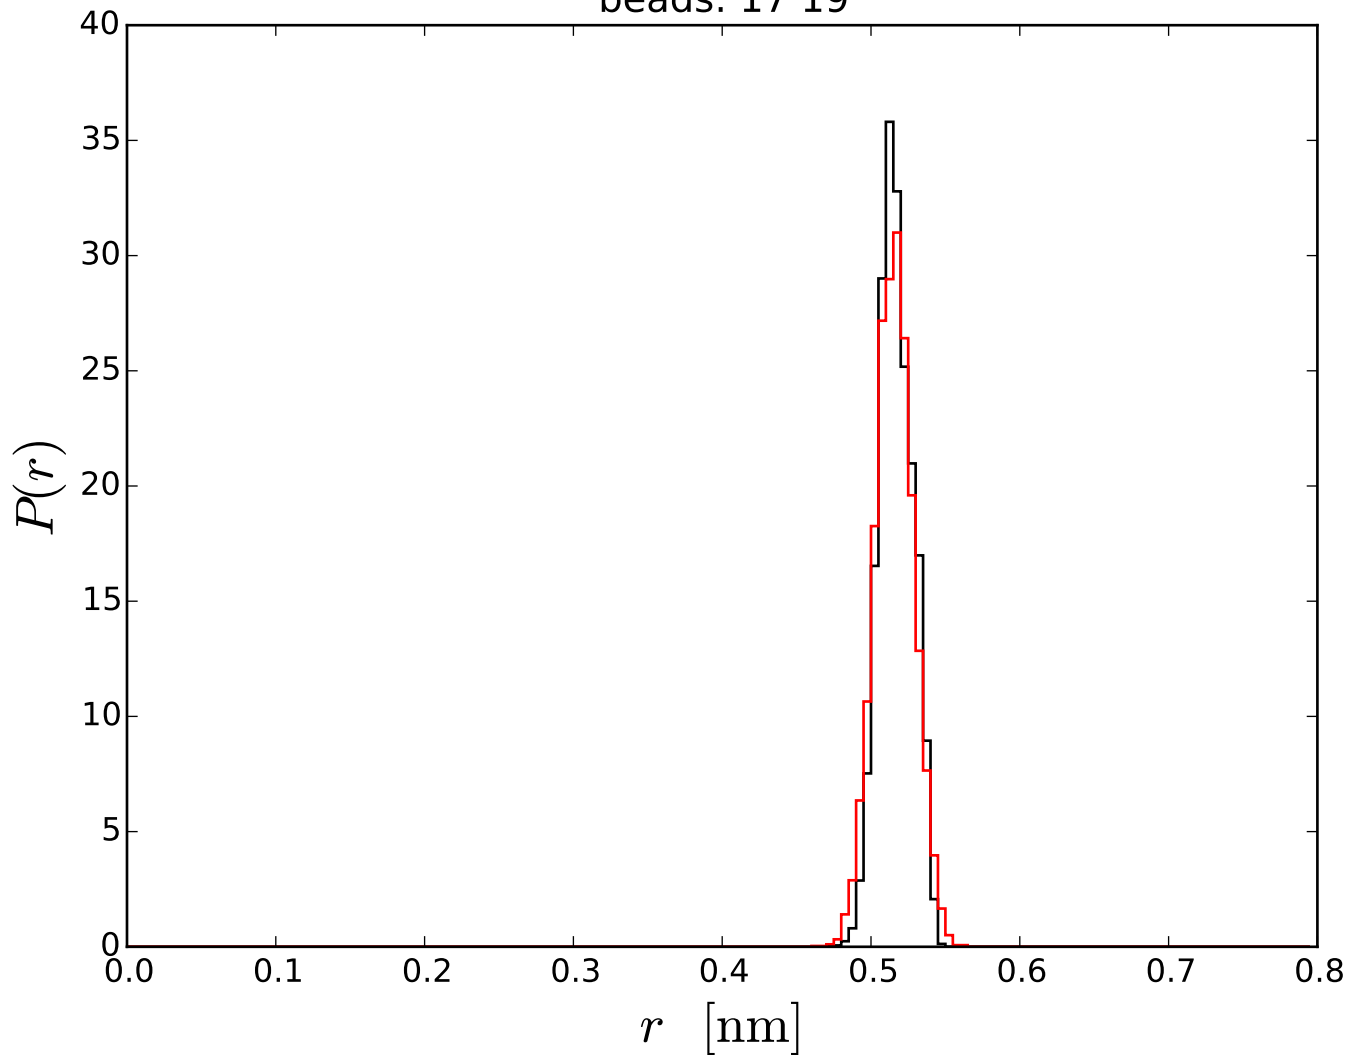



beads: 18 19

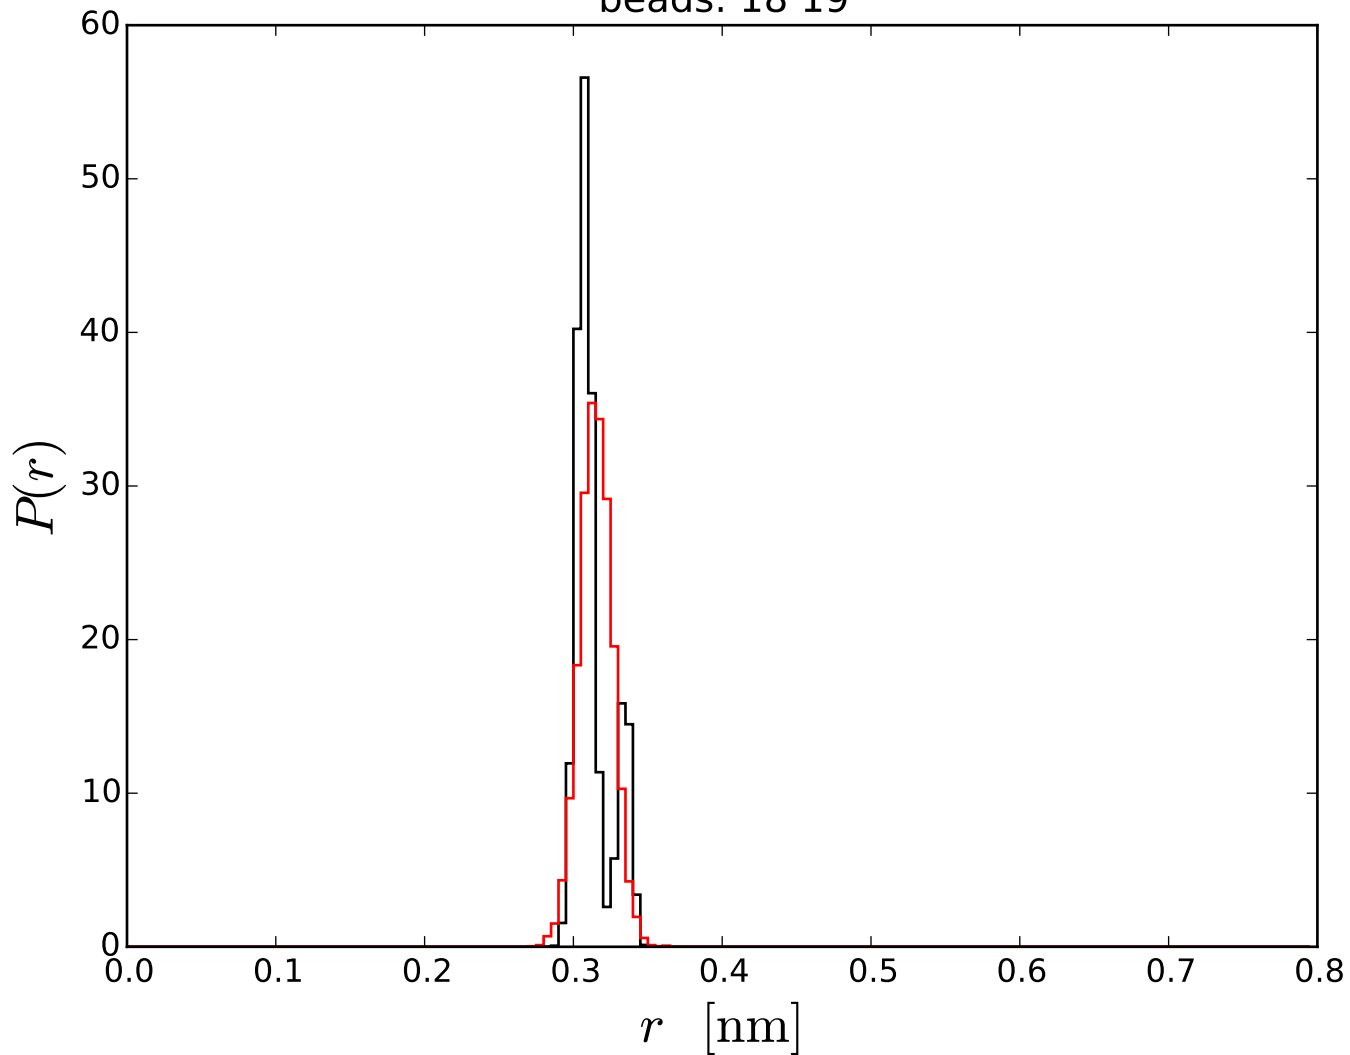

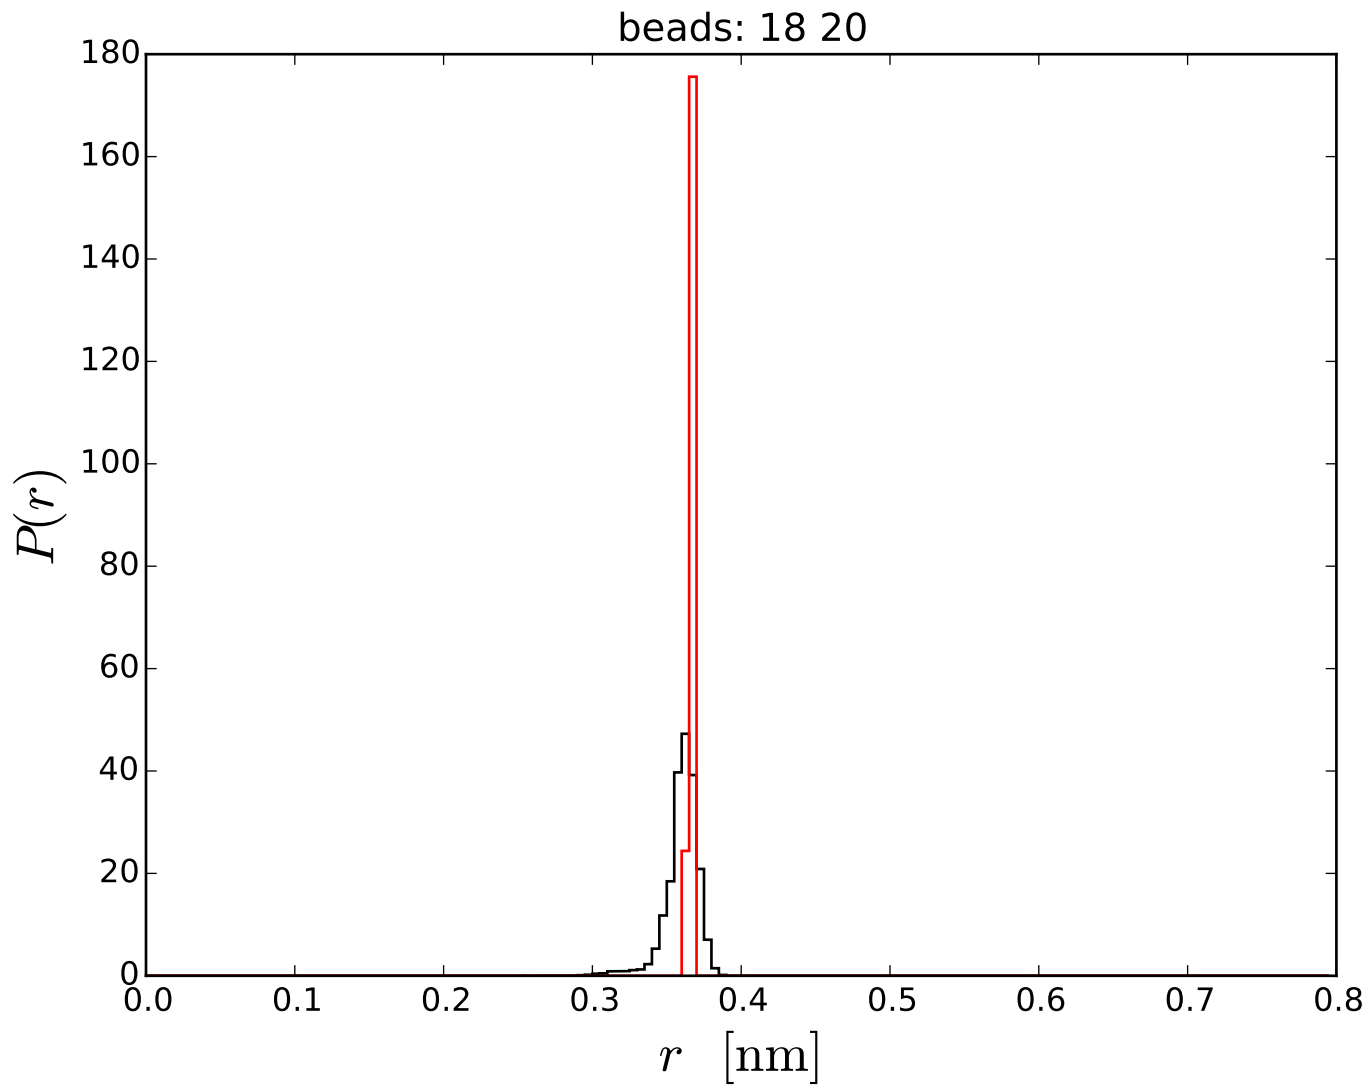

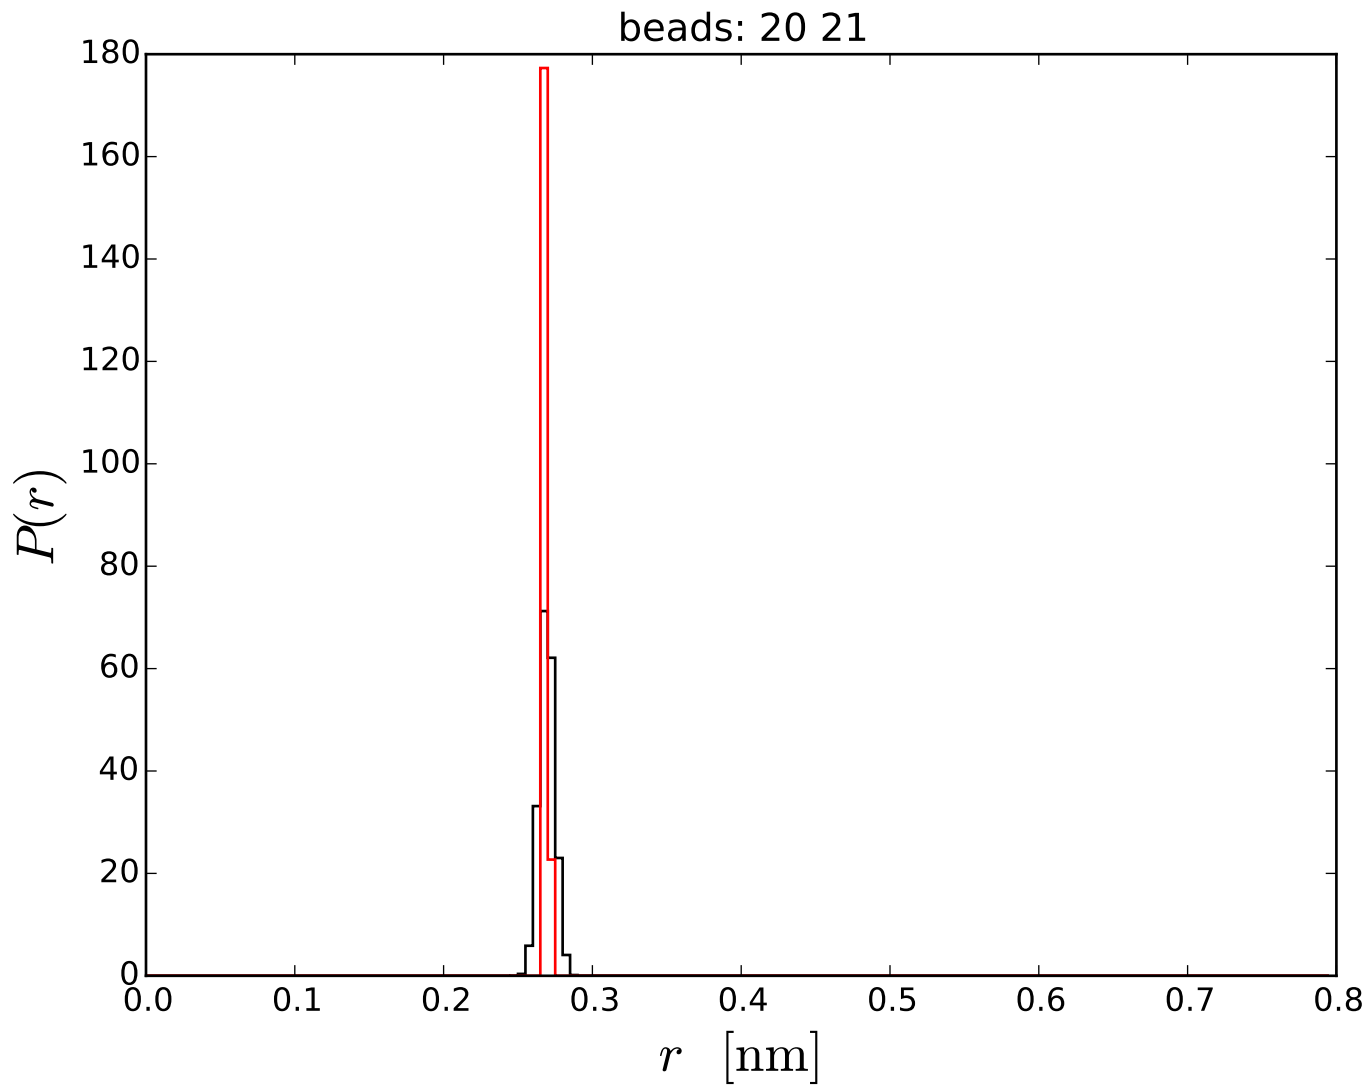

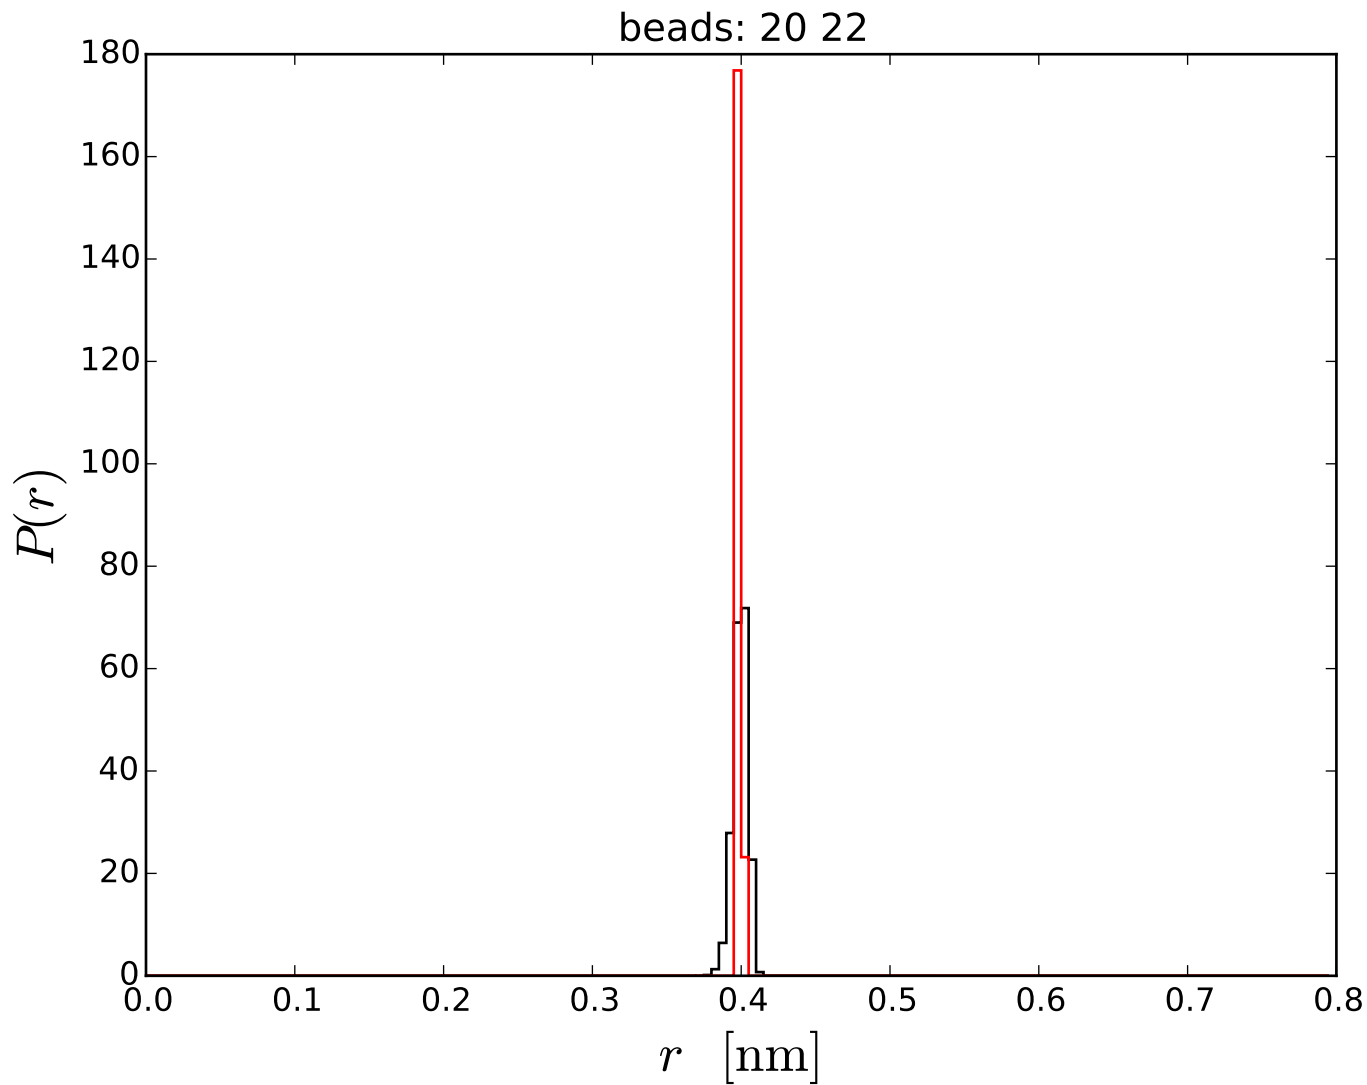

beads: 21 22

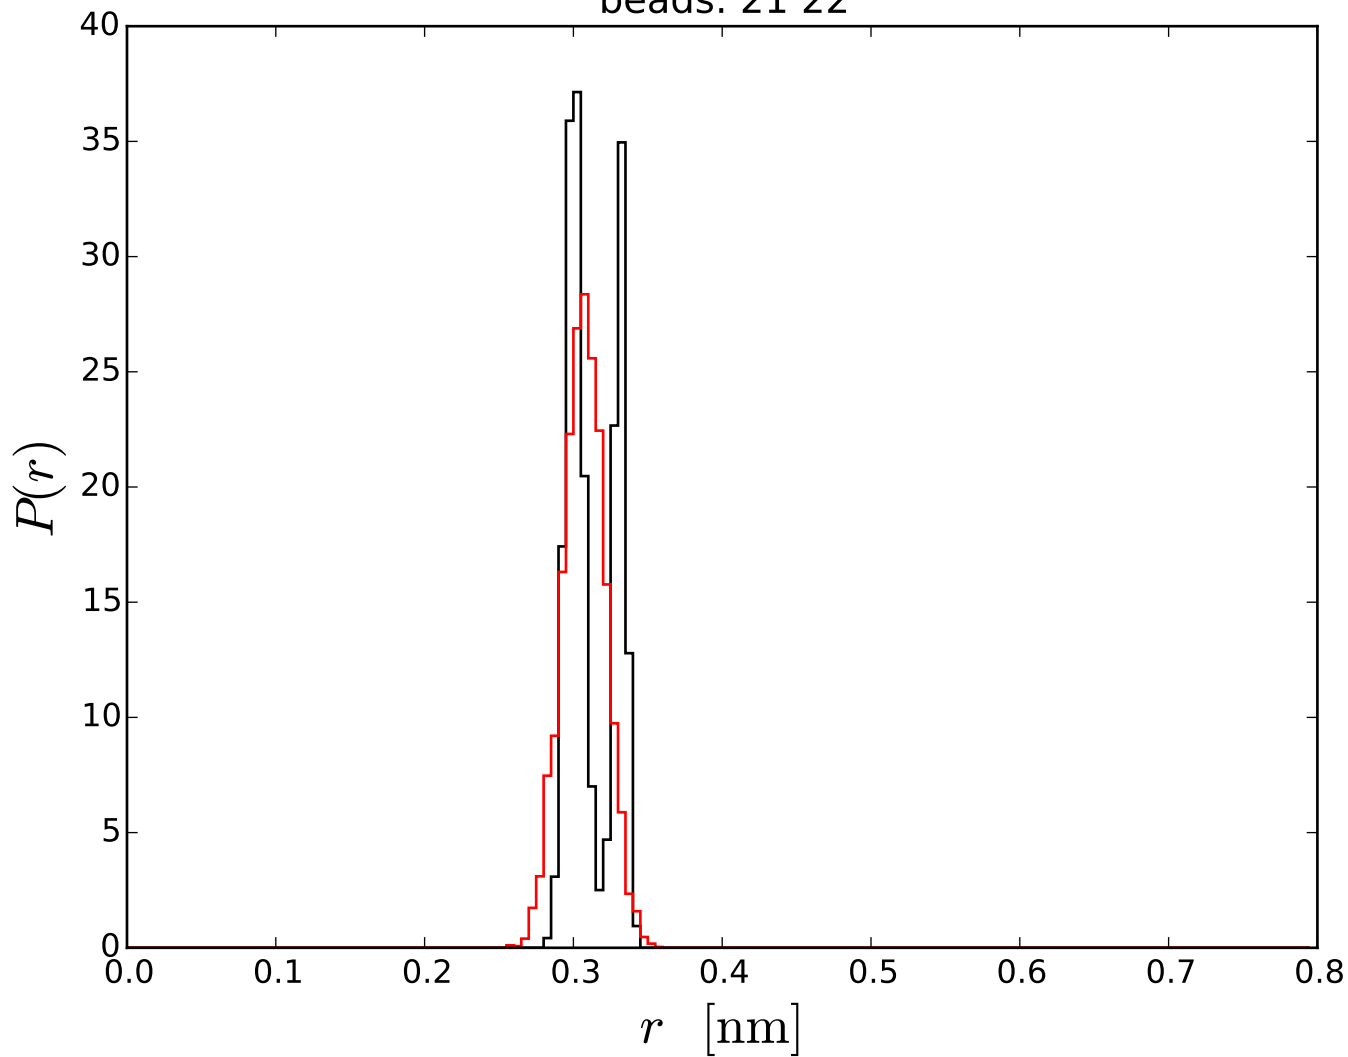

beads: 21 23

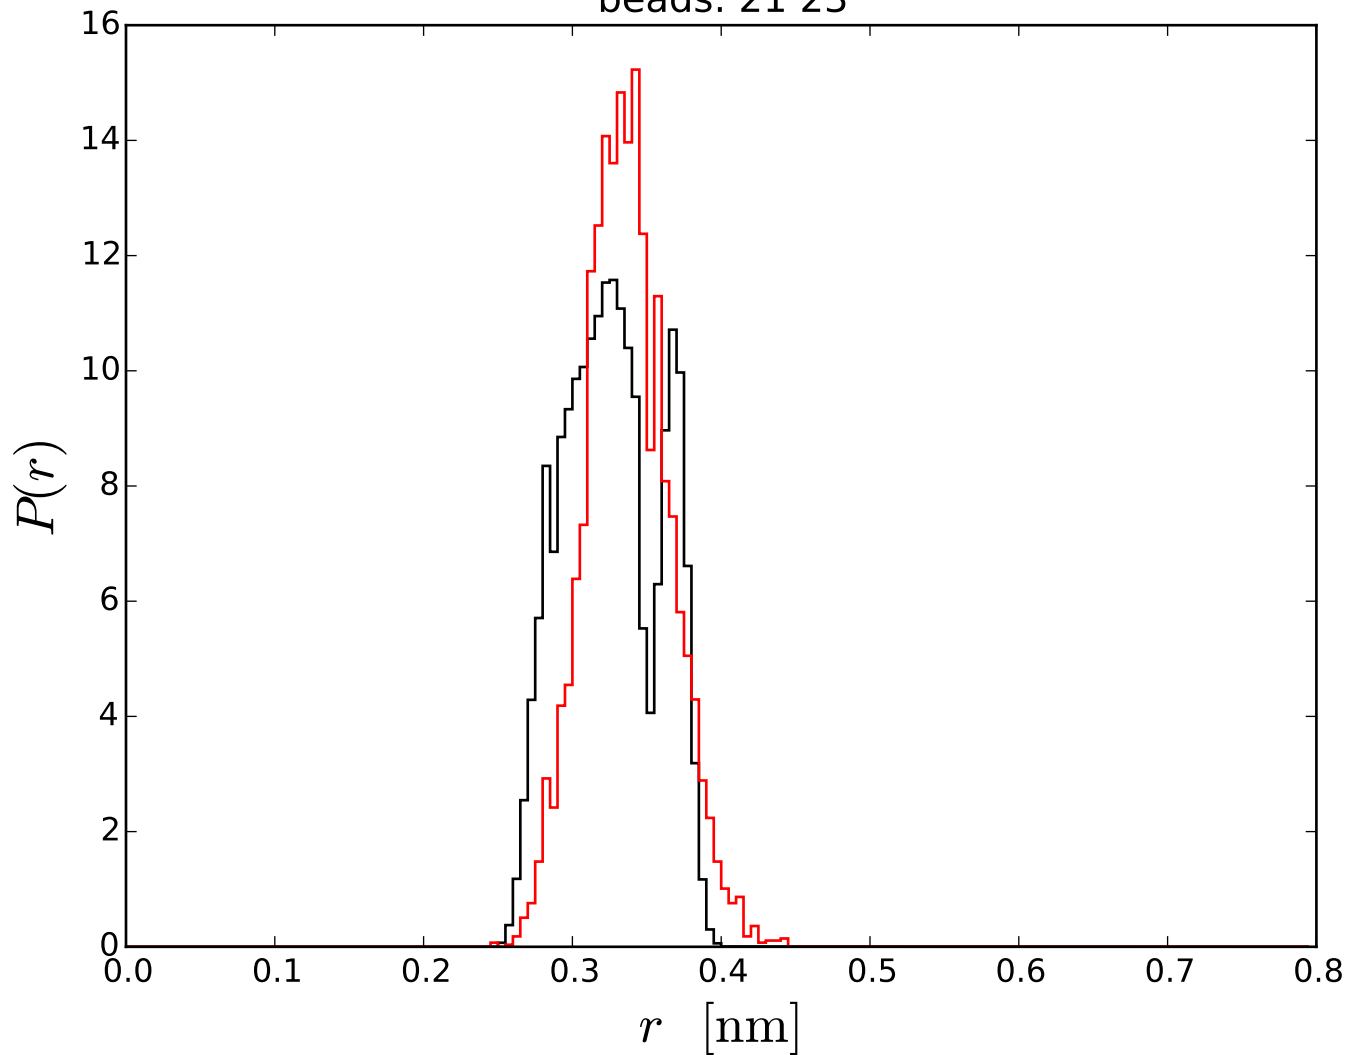

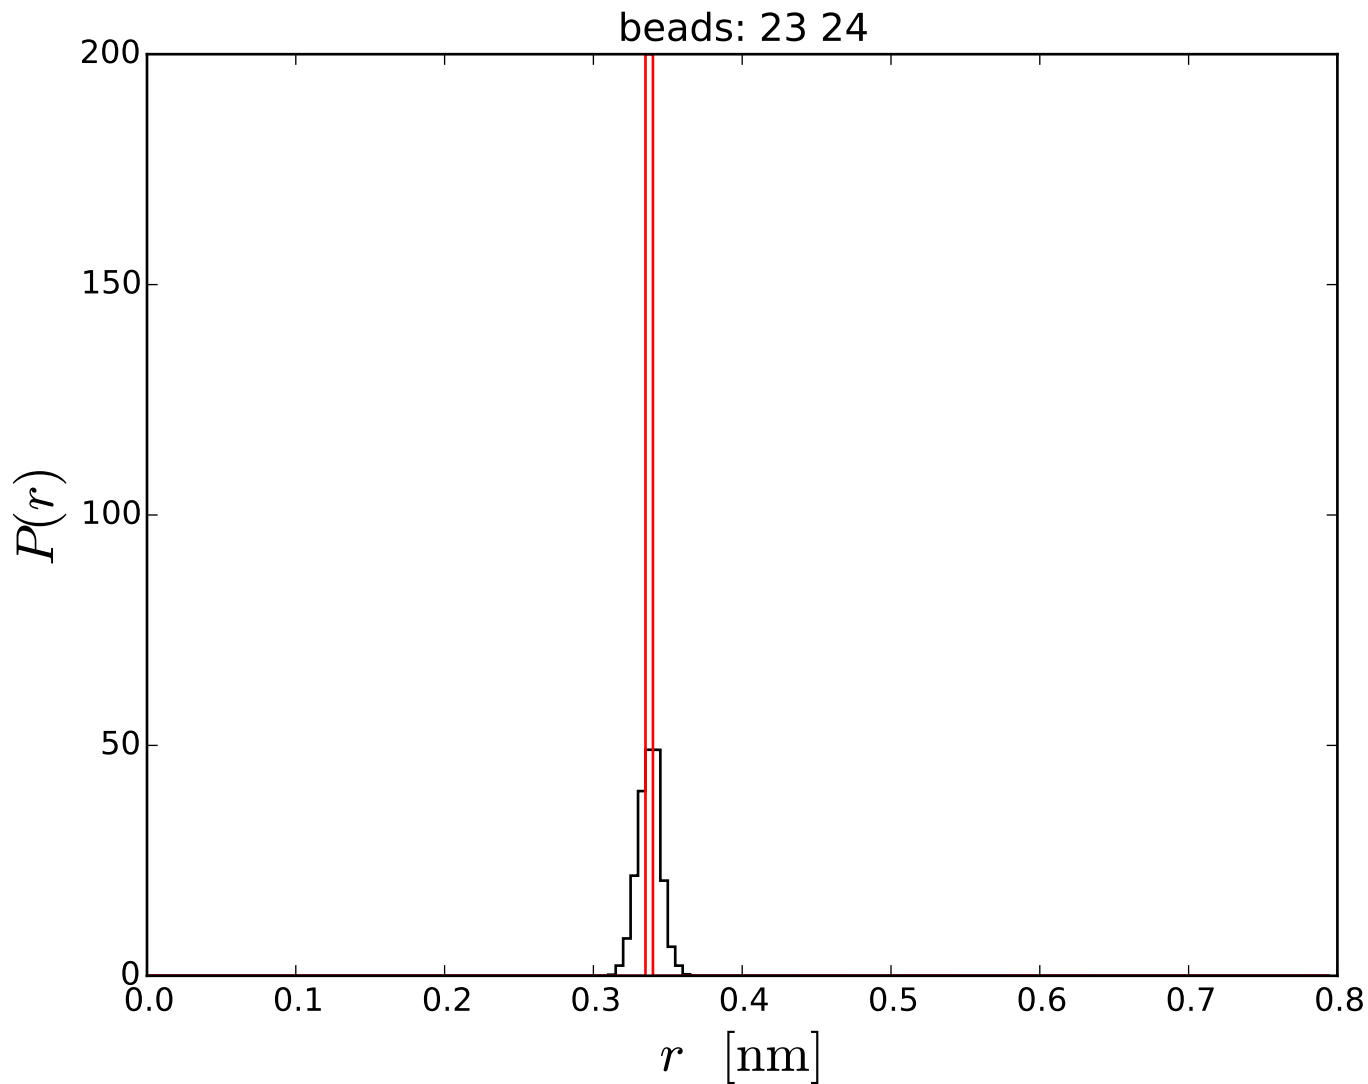

beads: 23 25

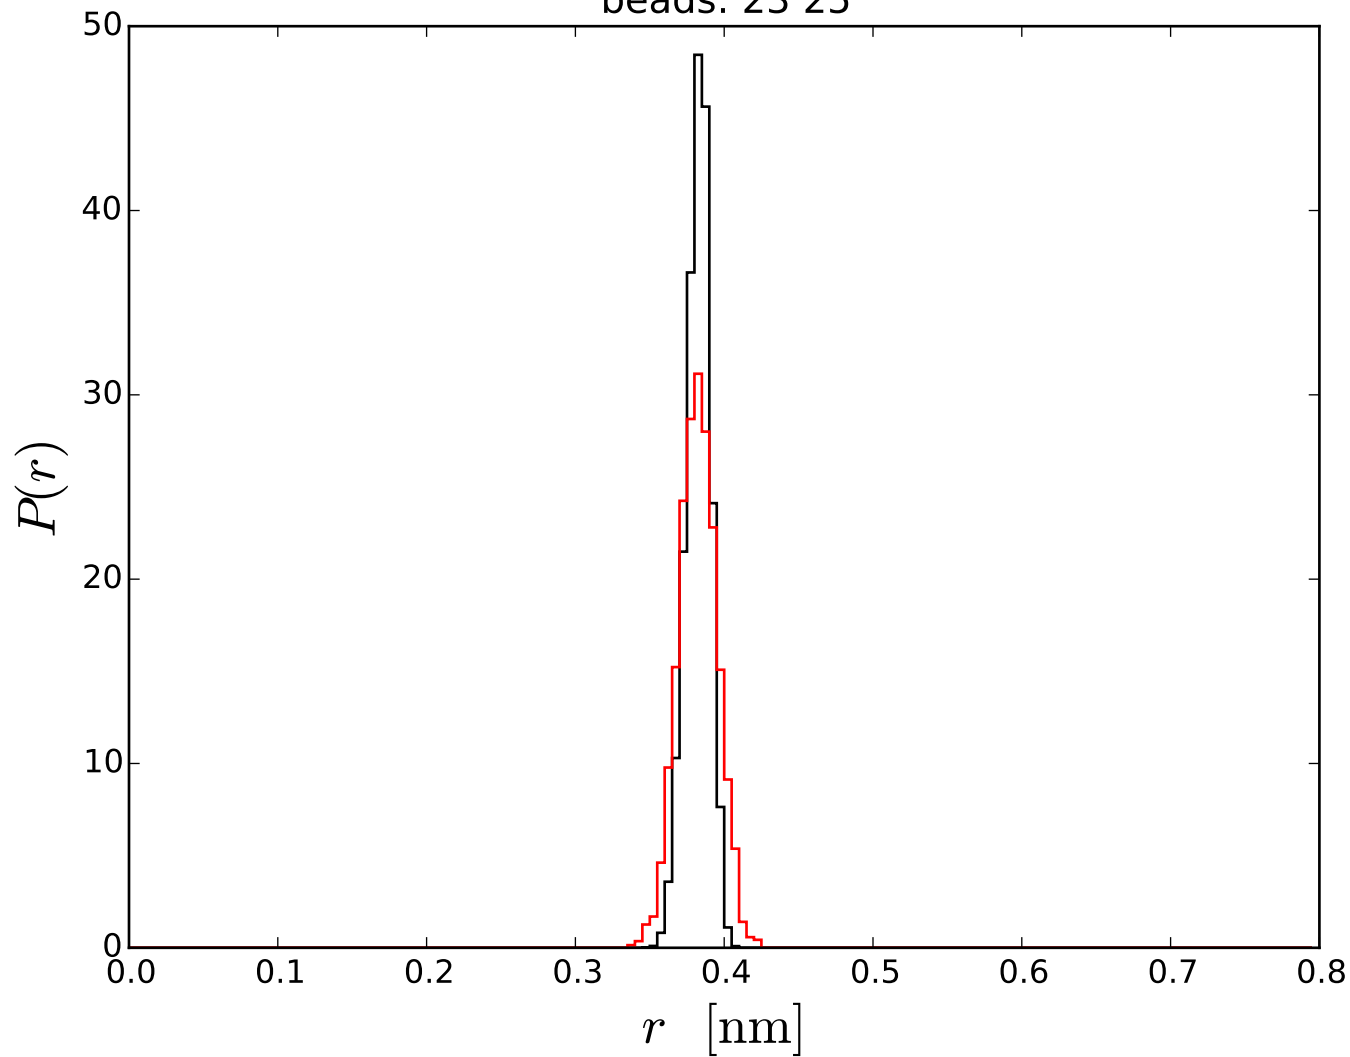



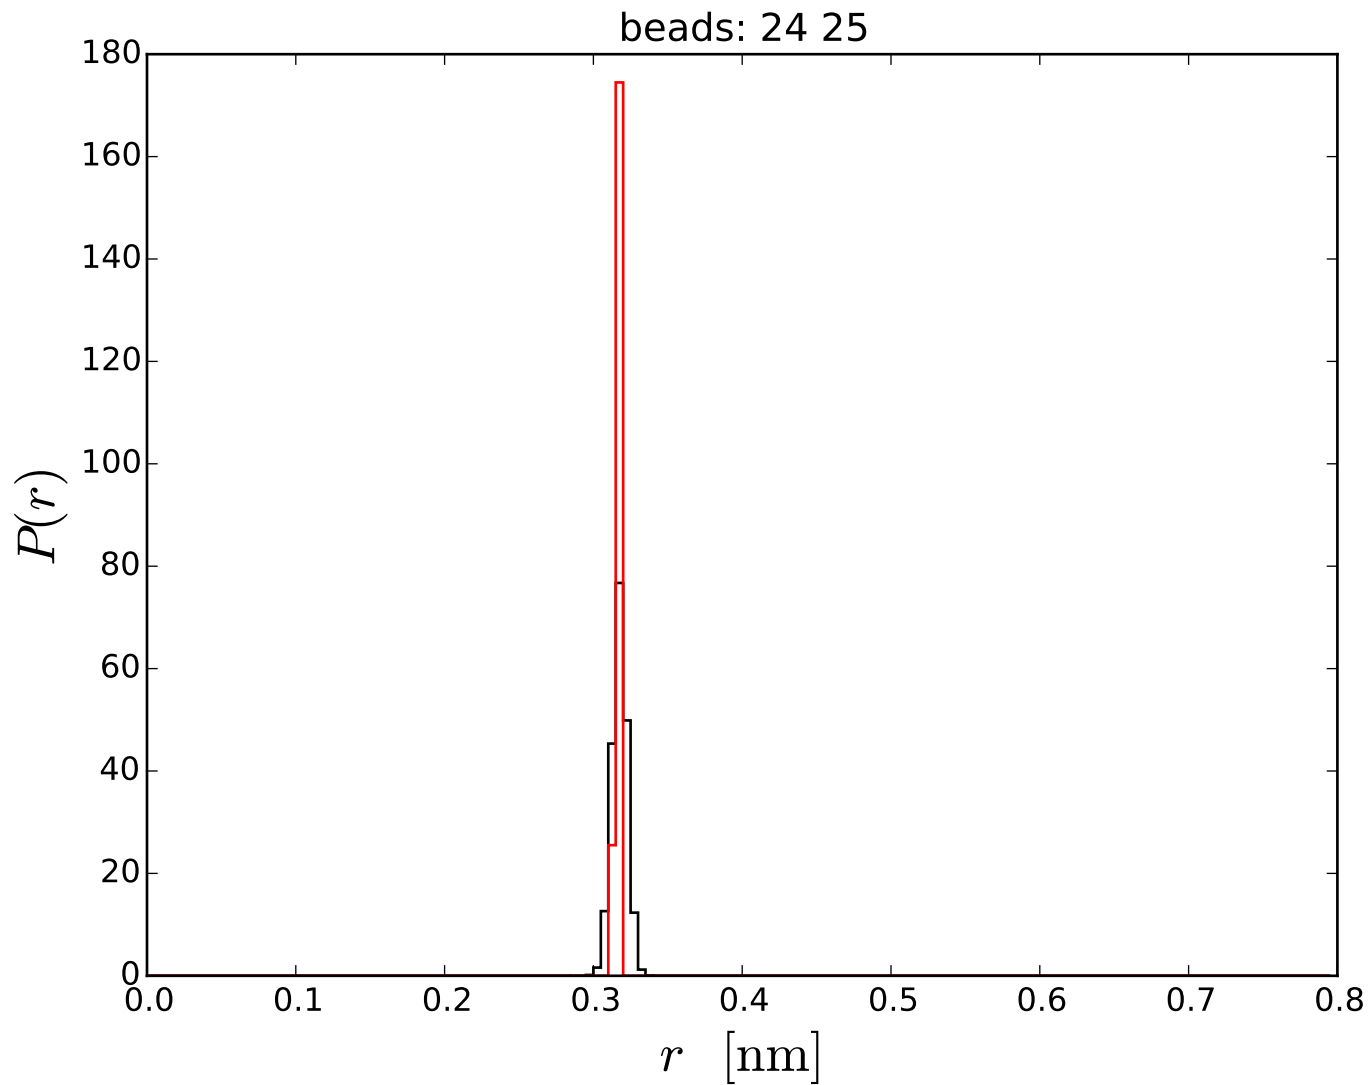

beads: 24 26

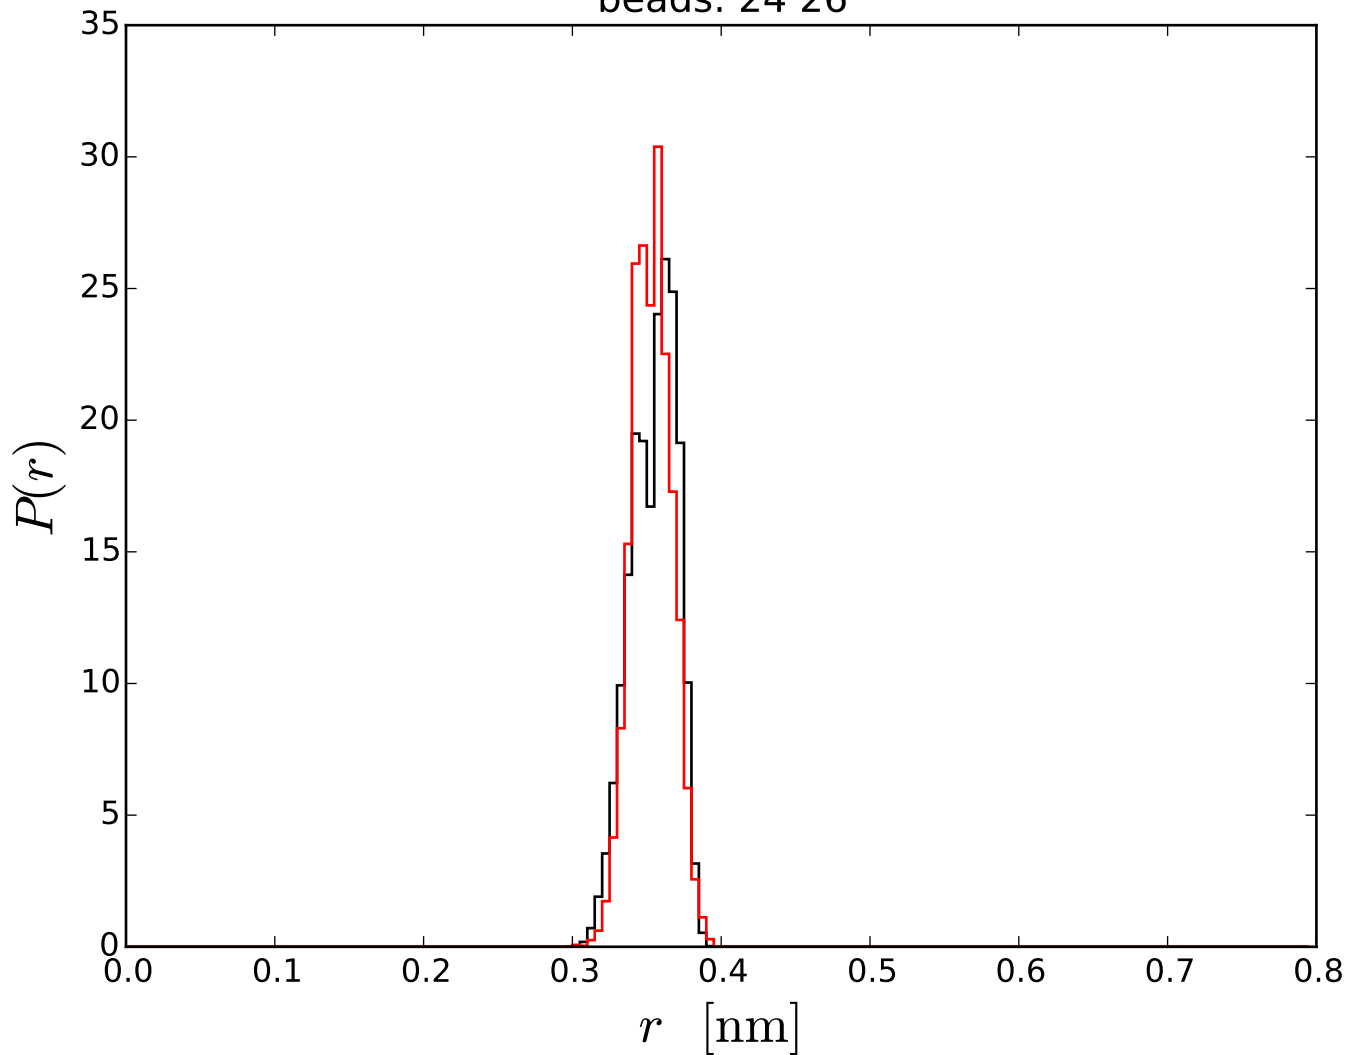

beads: 25 27

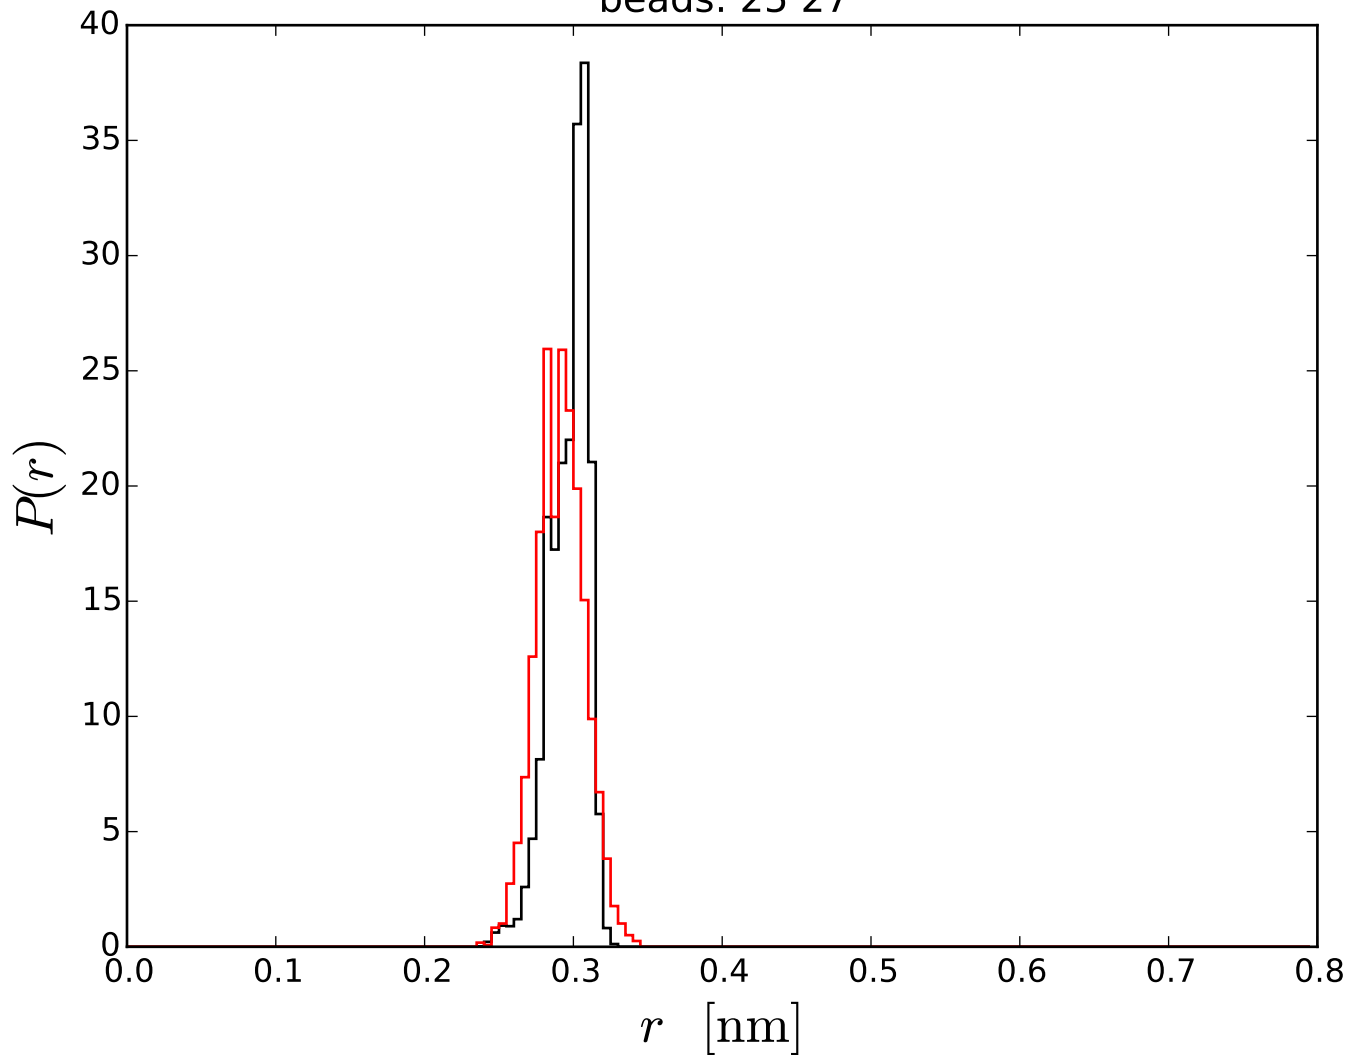

beads: 28 29

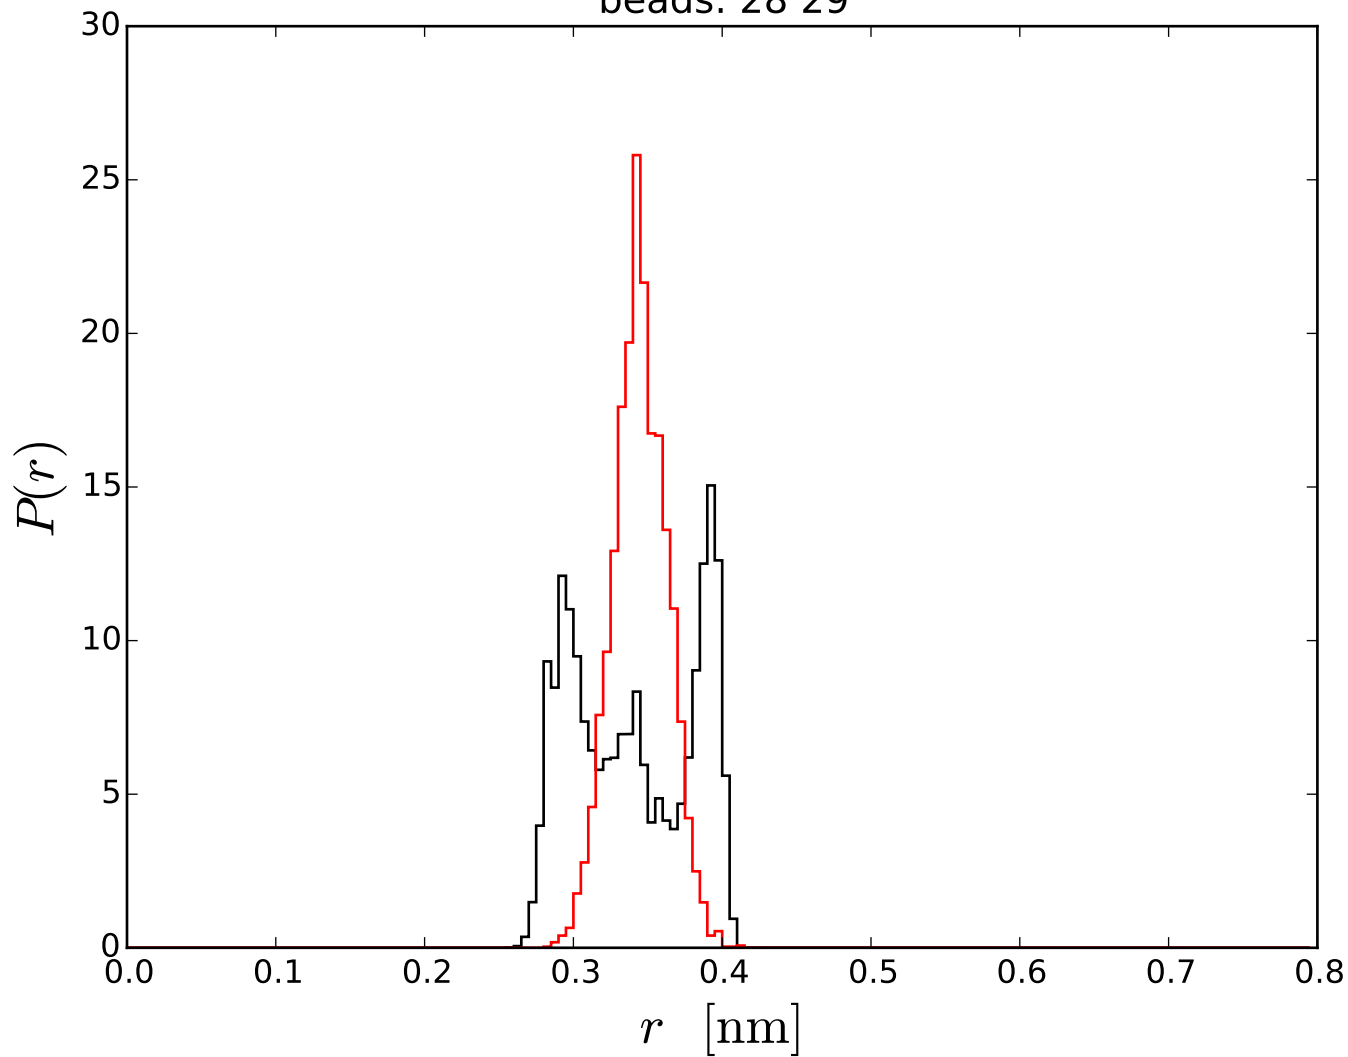

beads: 28 30

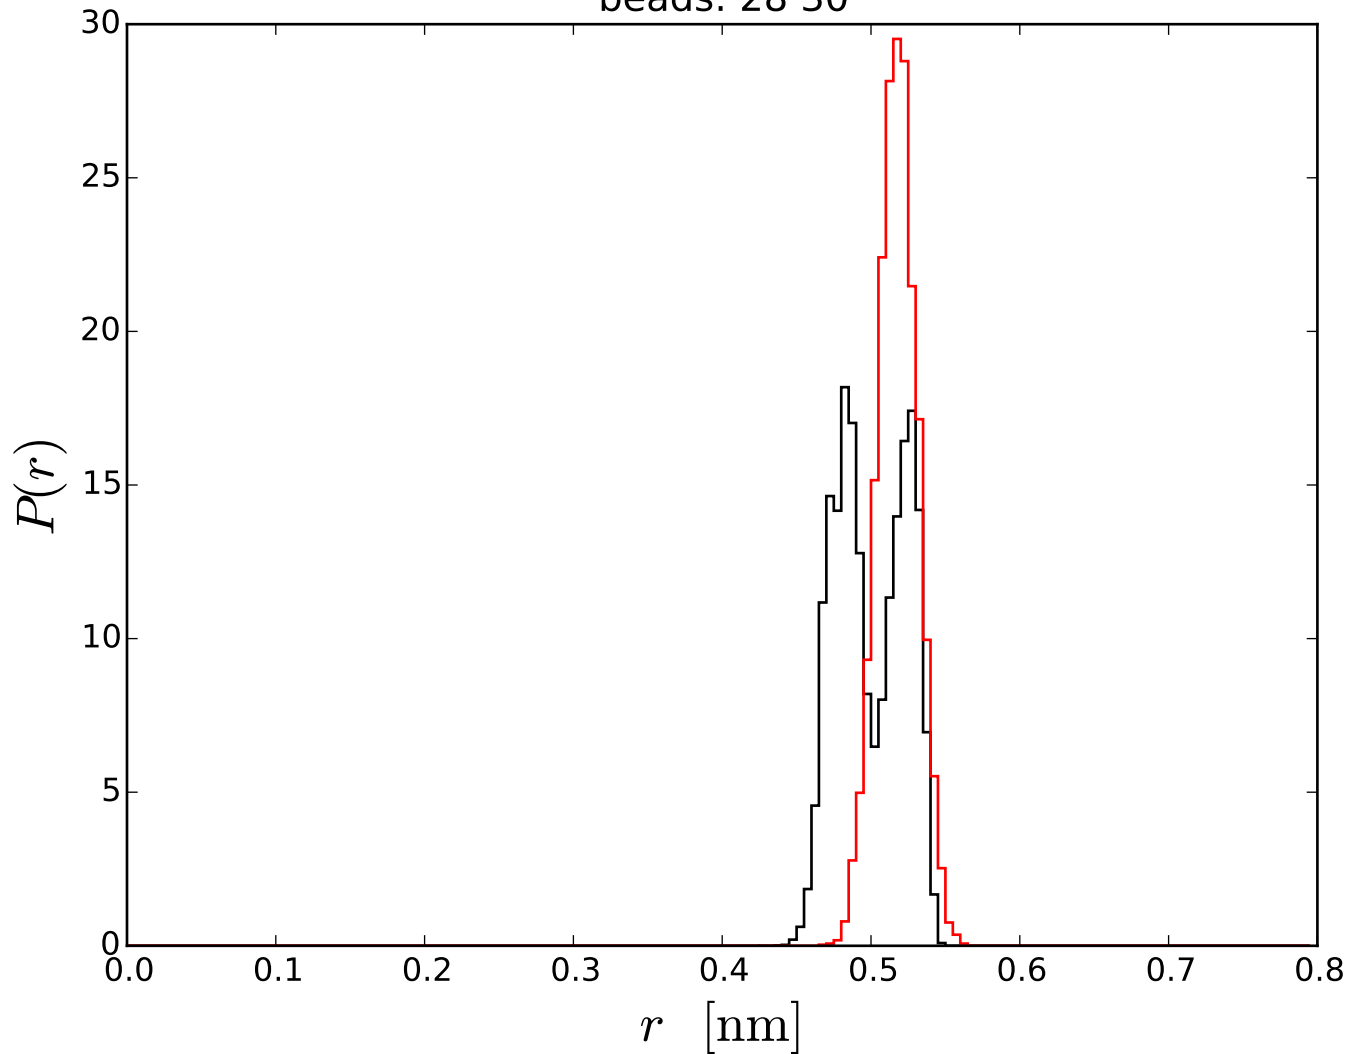

beads: 29 30

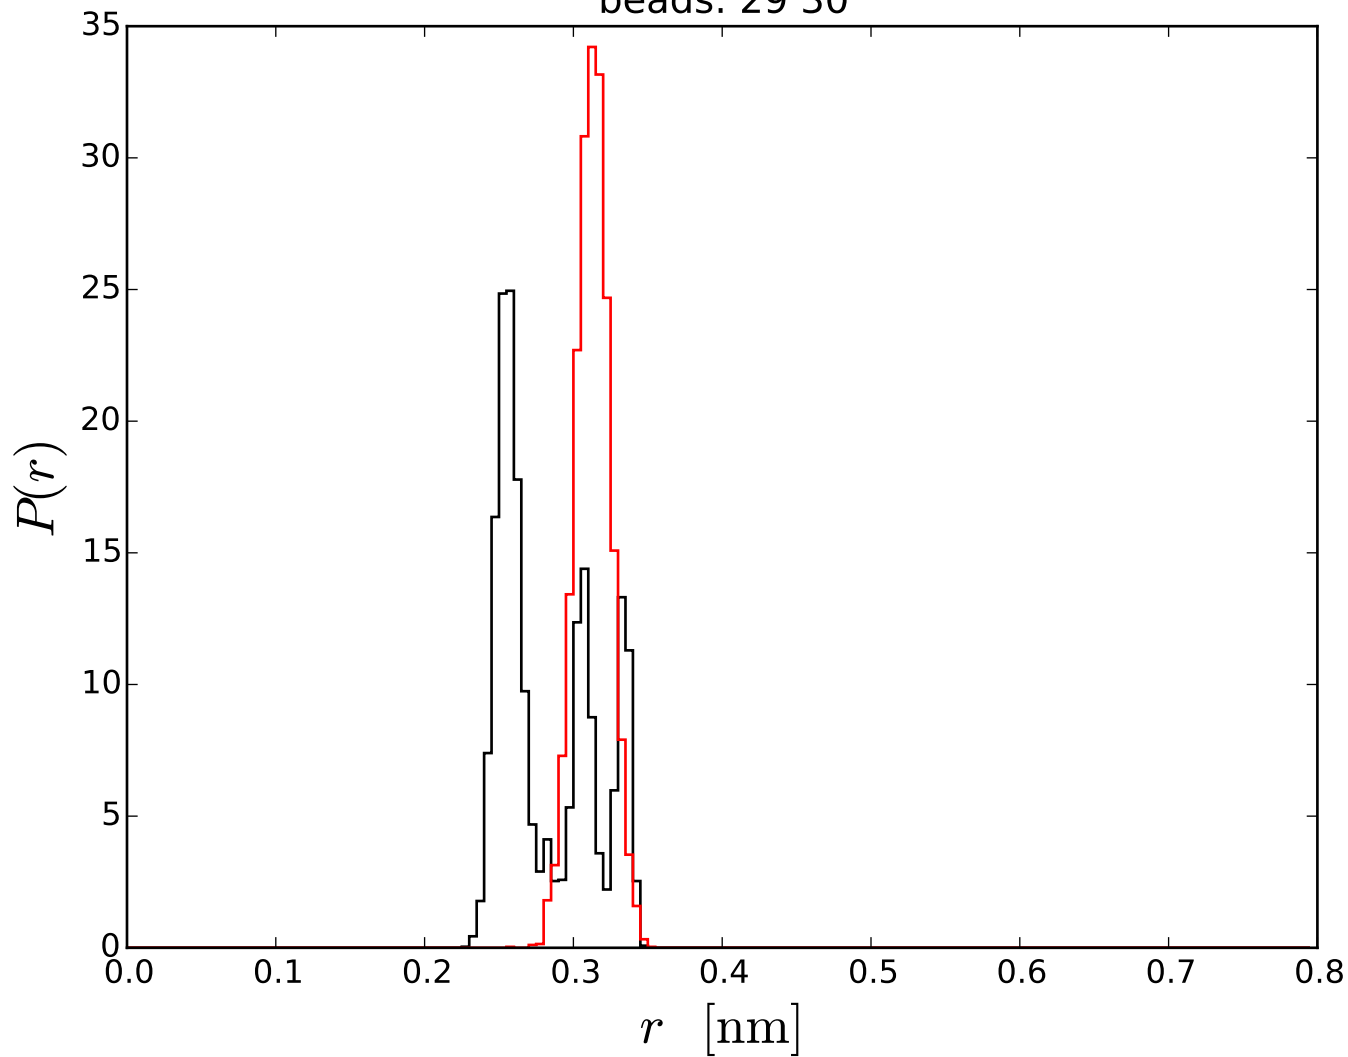

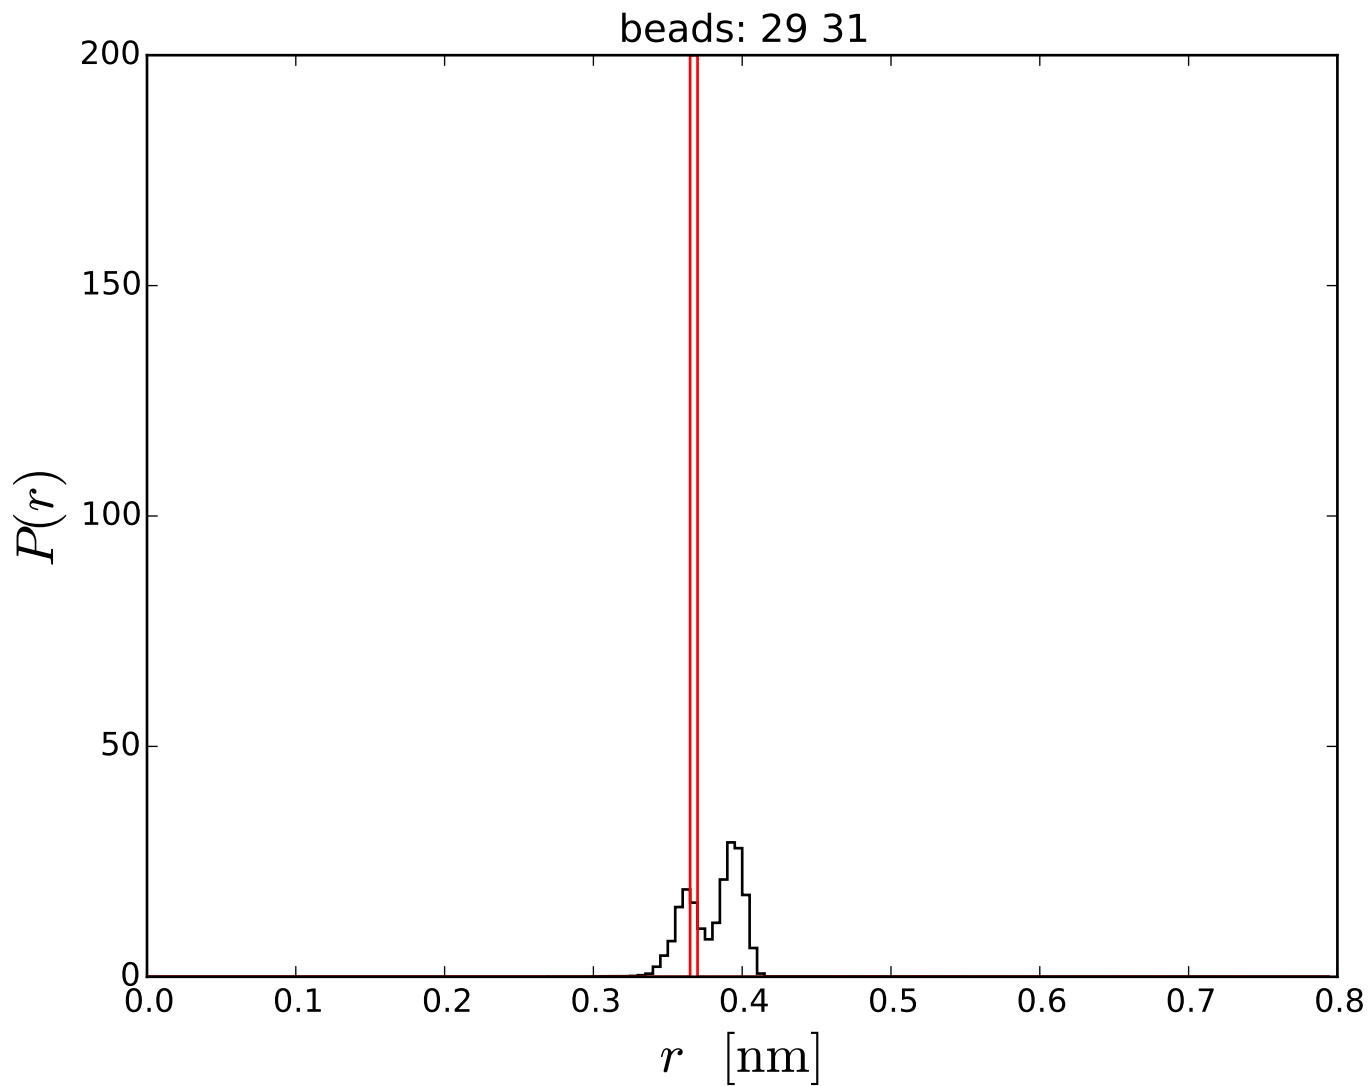

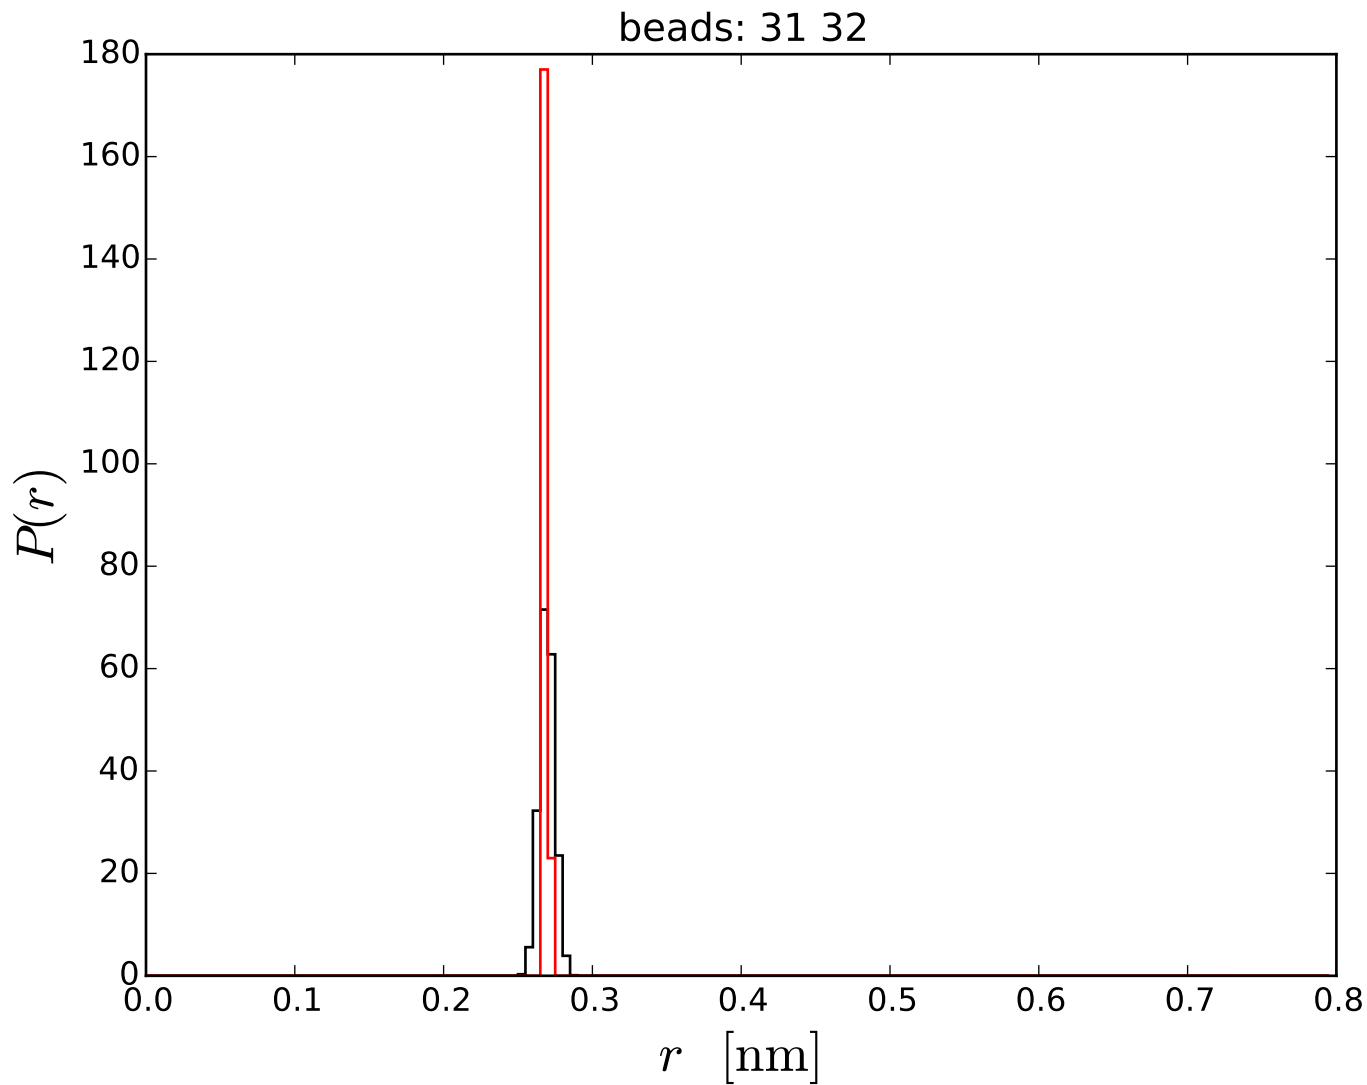



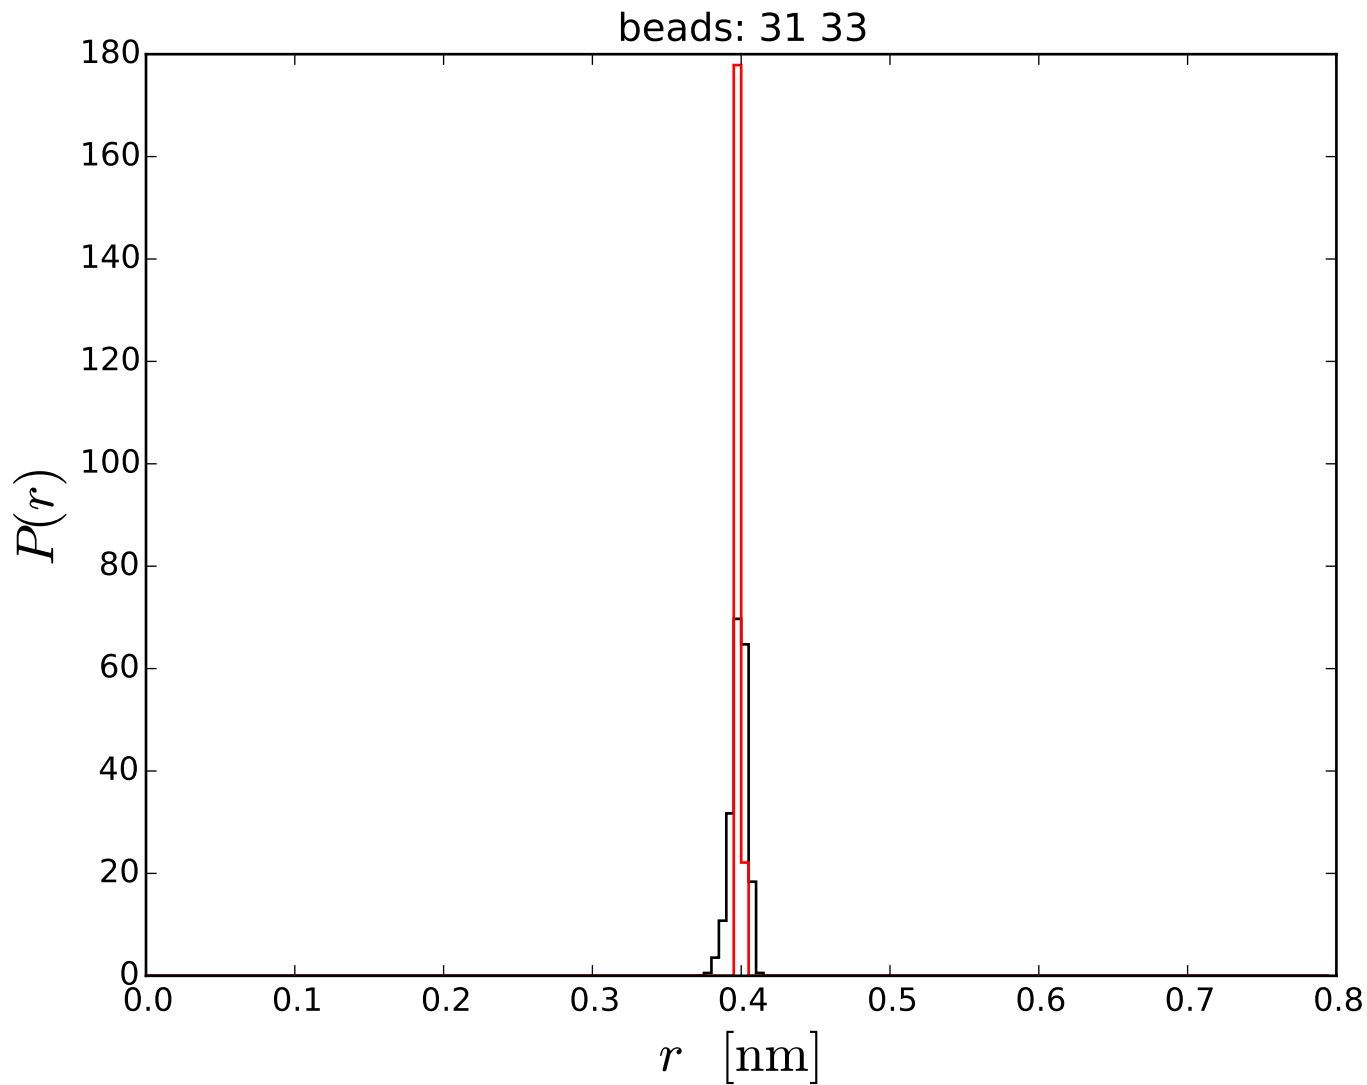

beads: 32 33

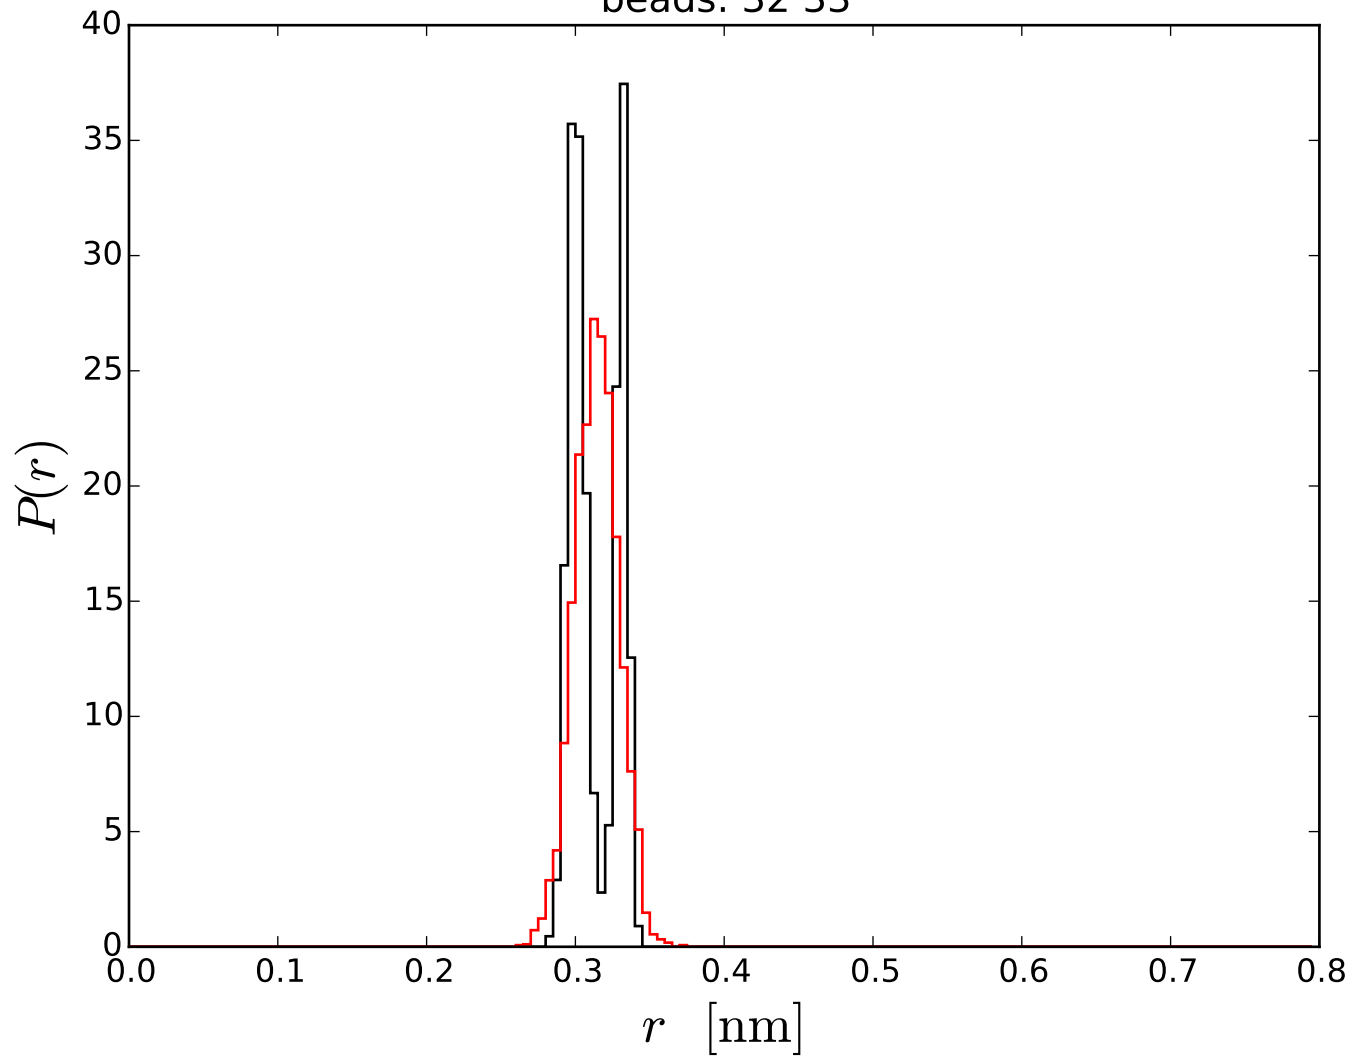

beads: 32 34

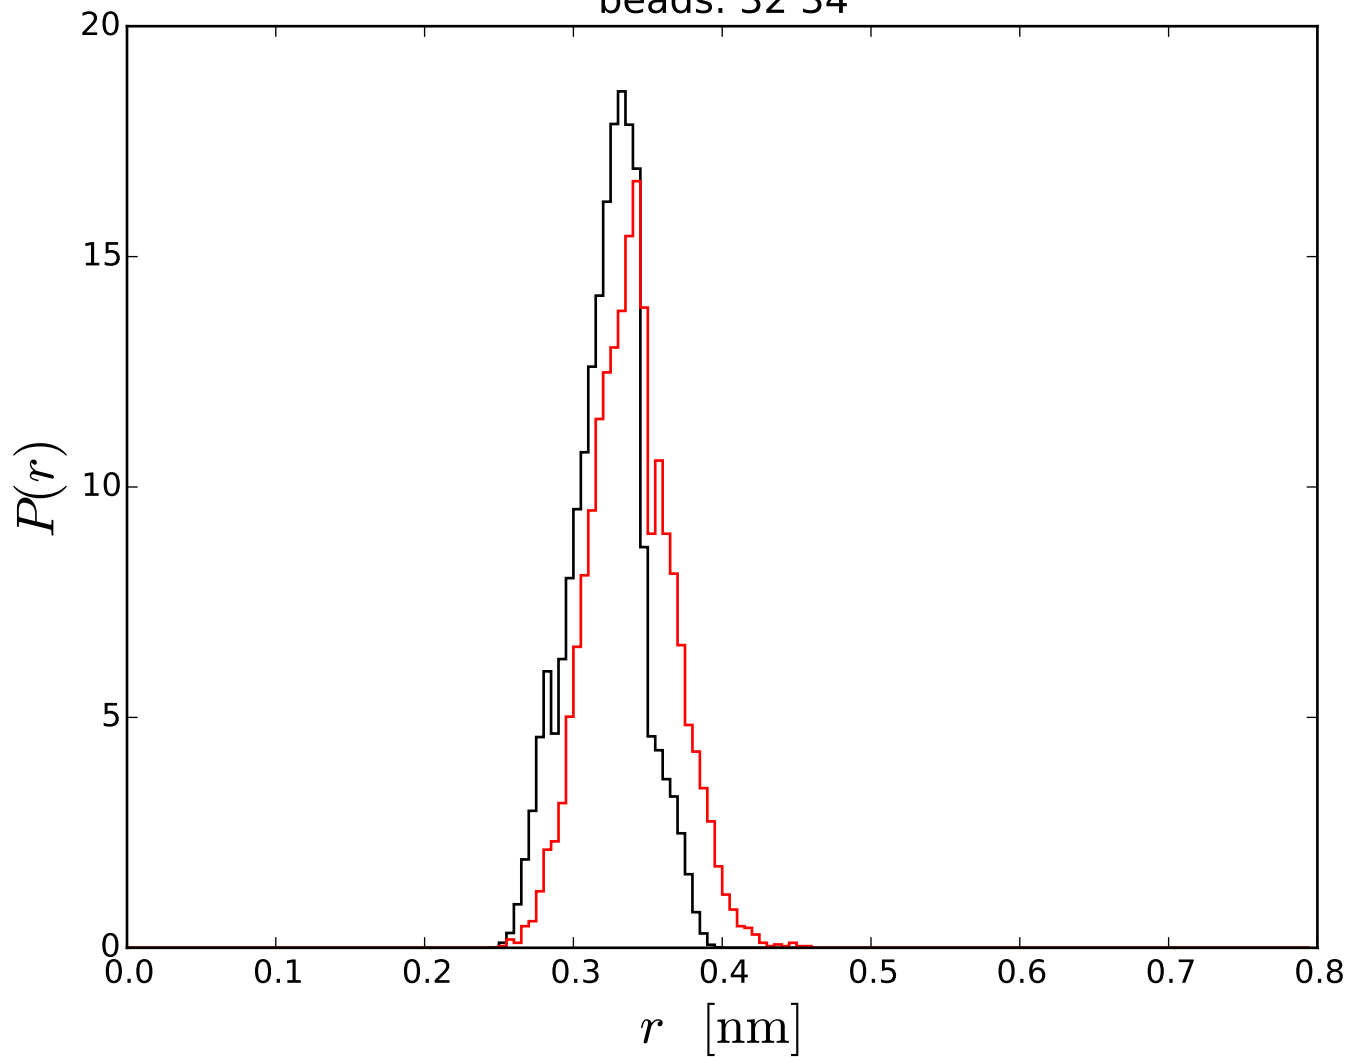

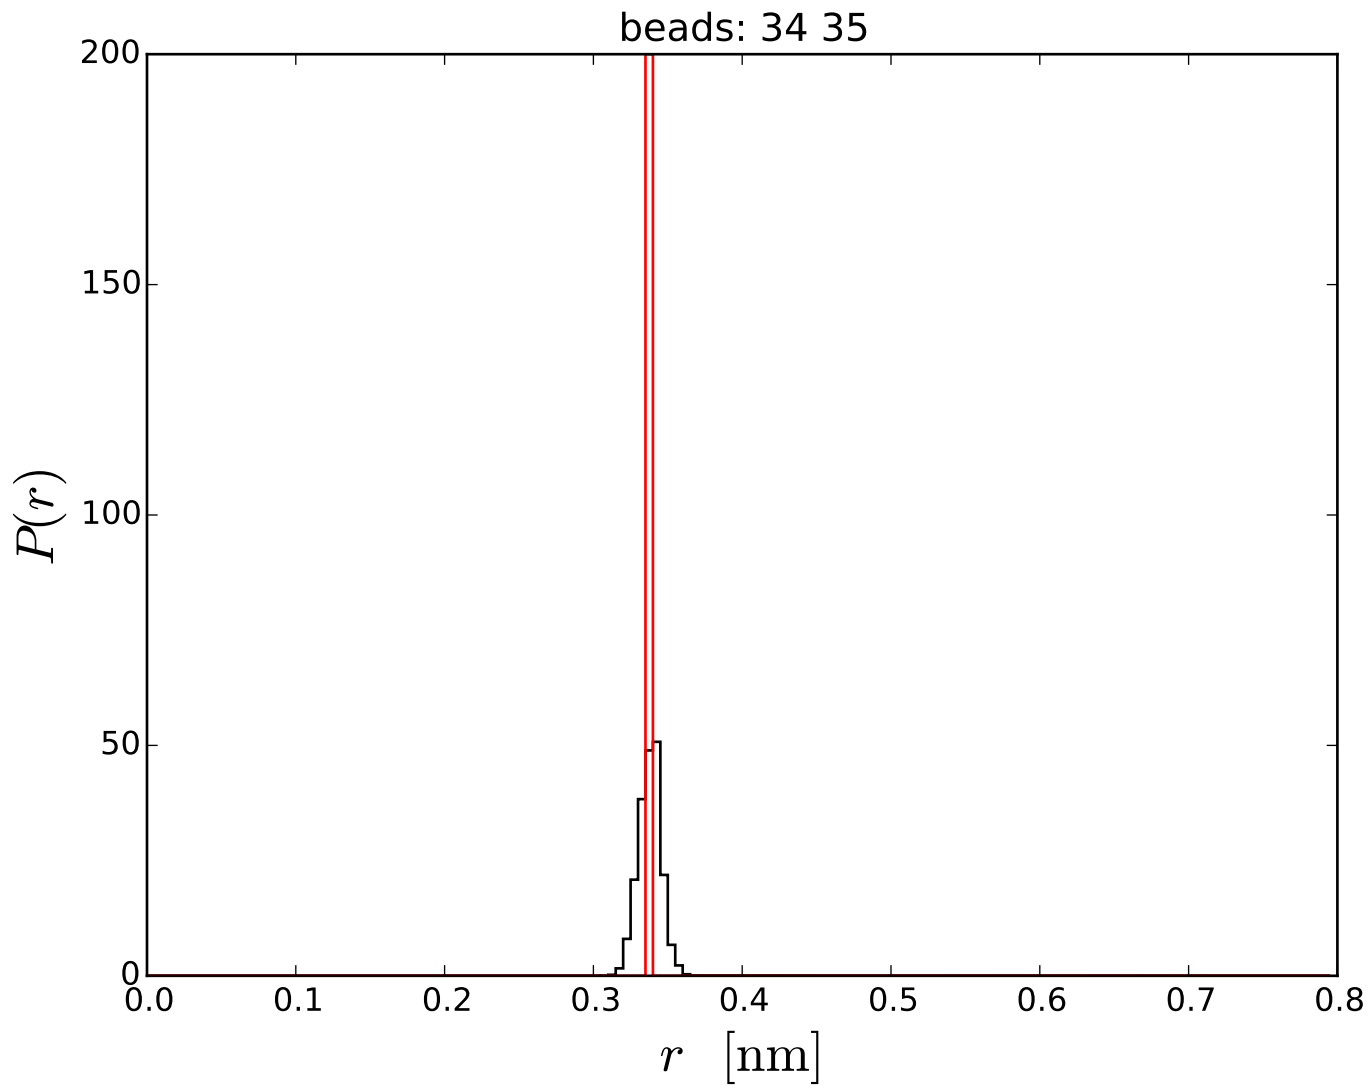

beads: 34 36

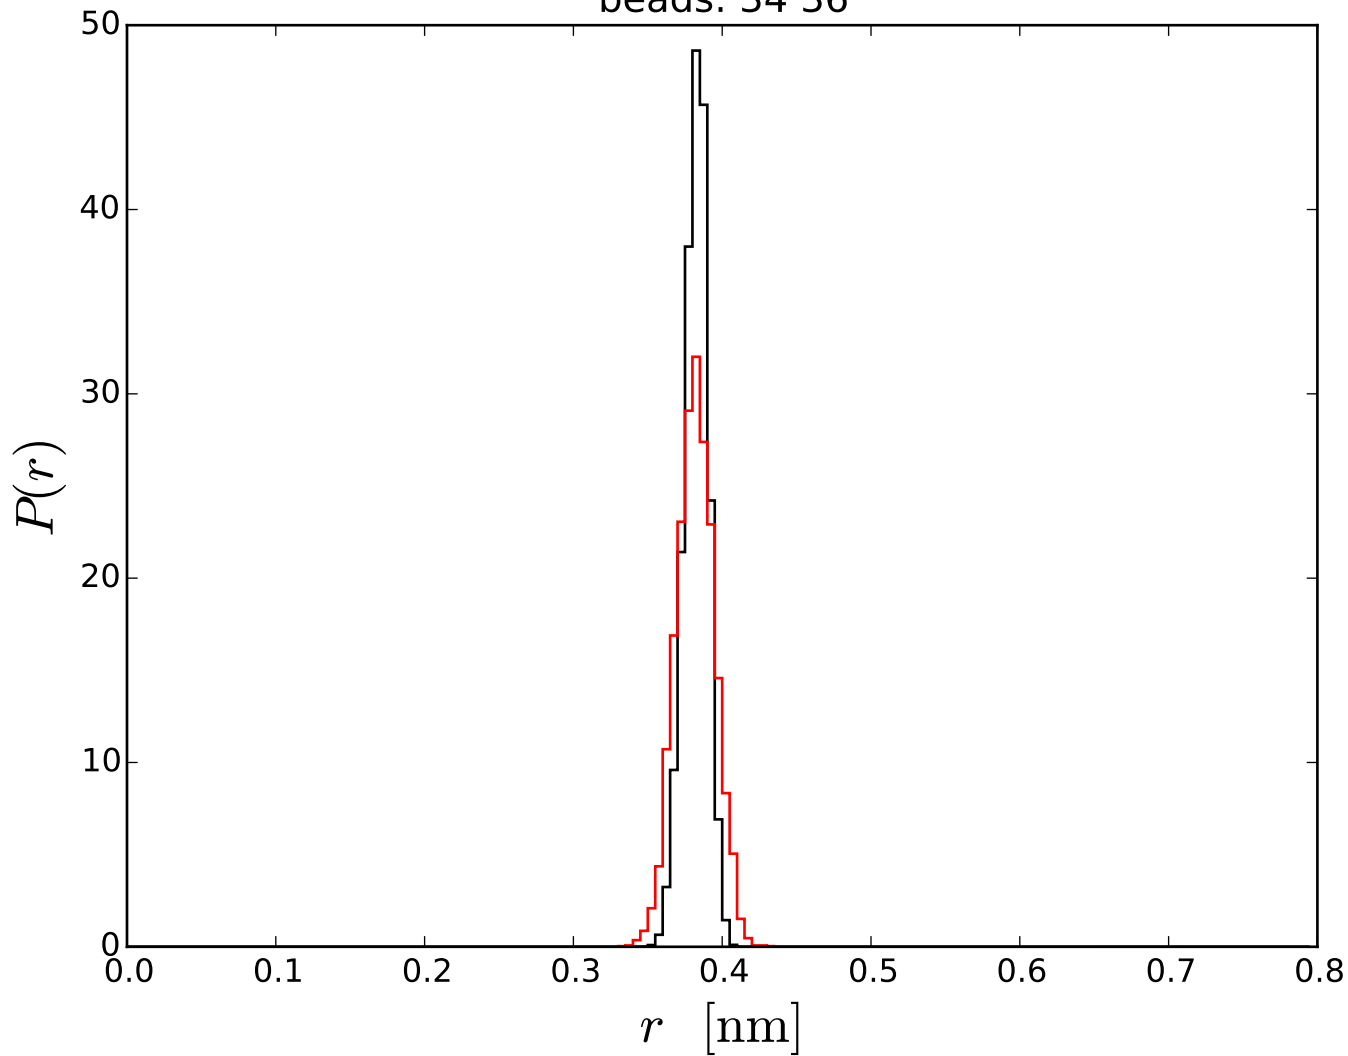

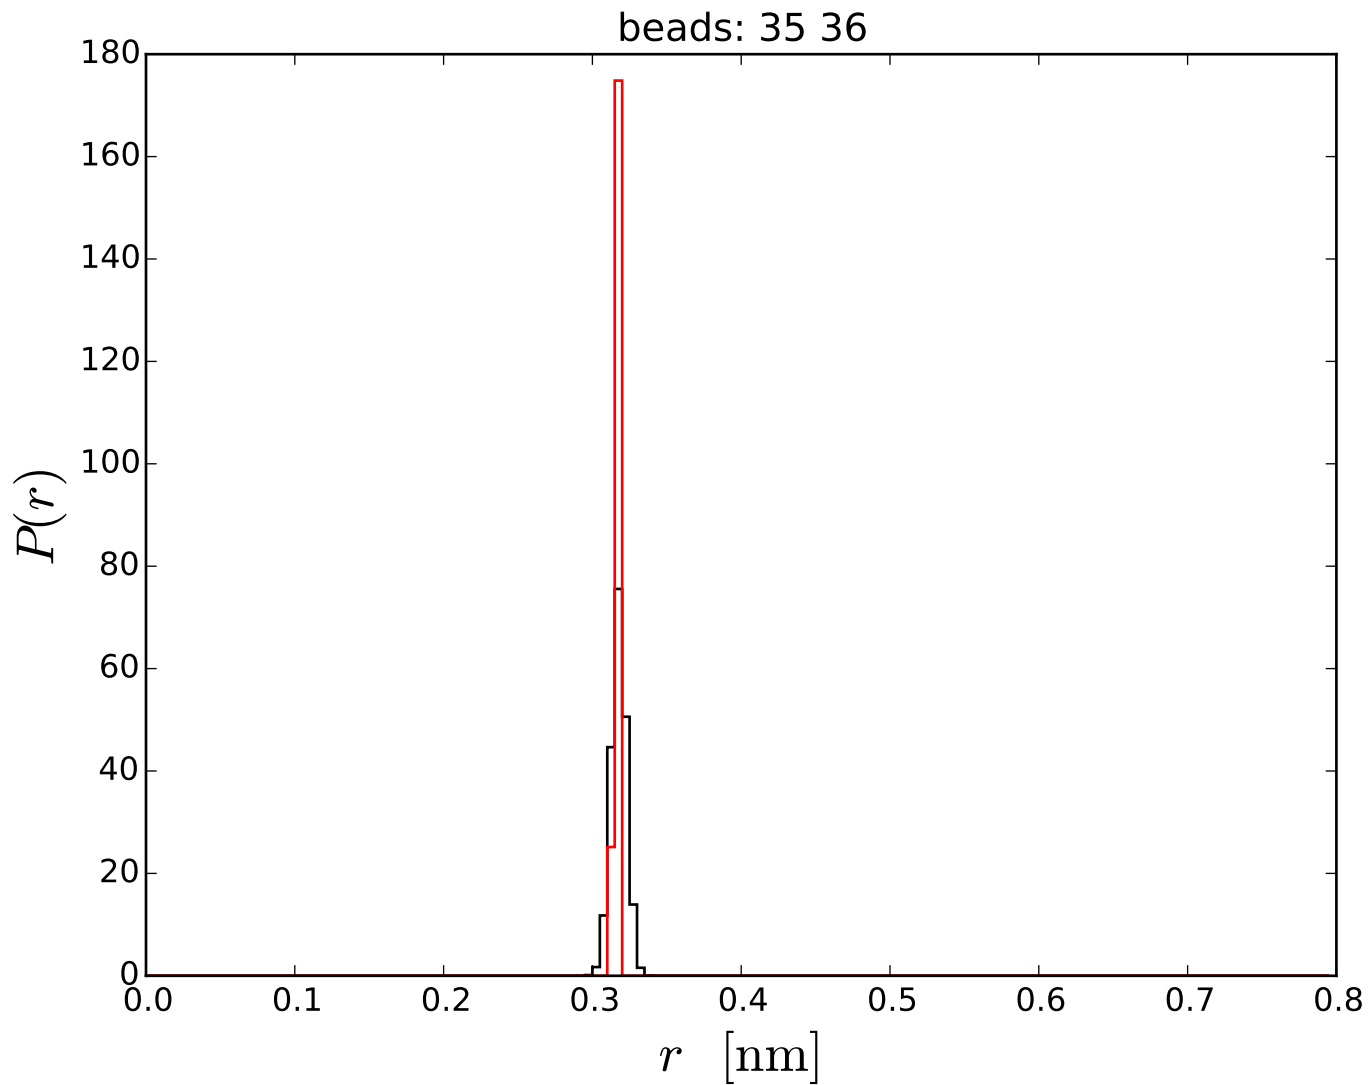

beads: 35 37

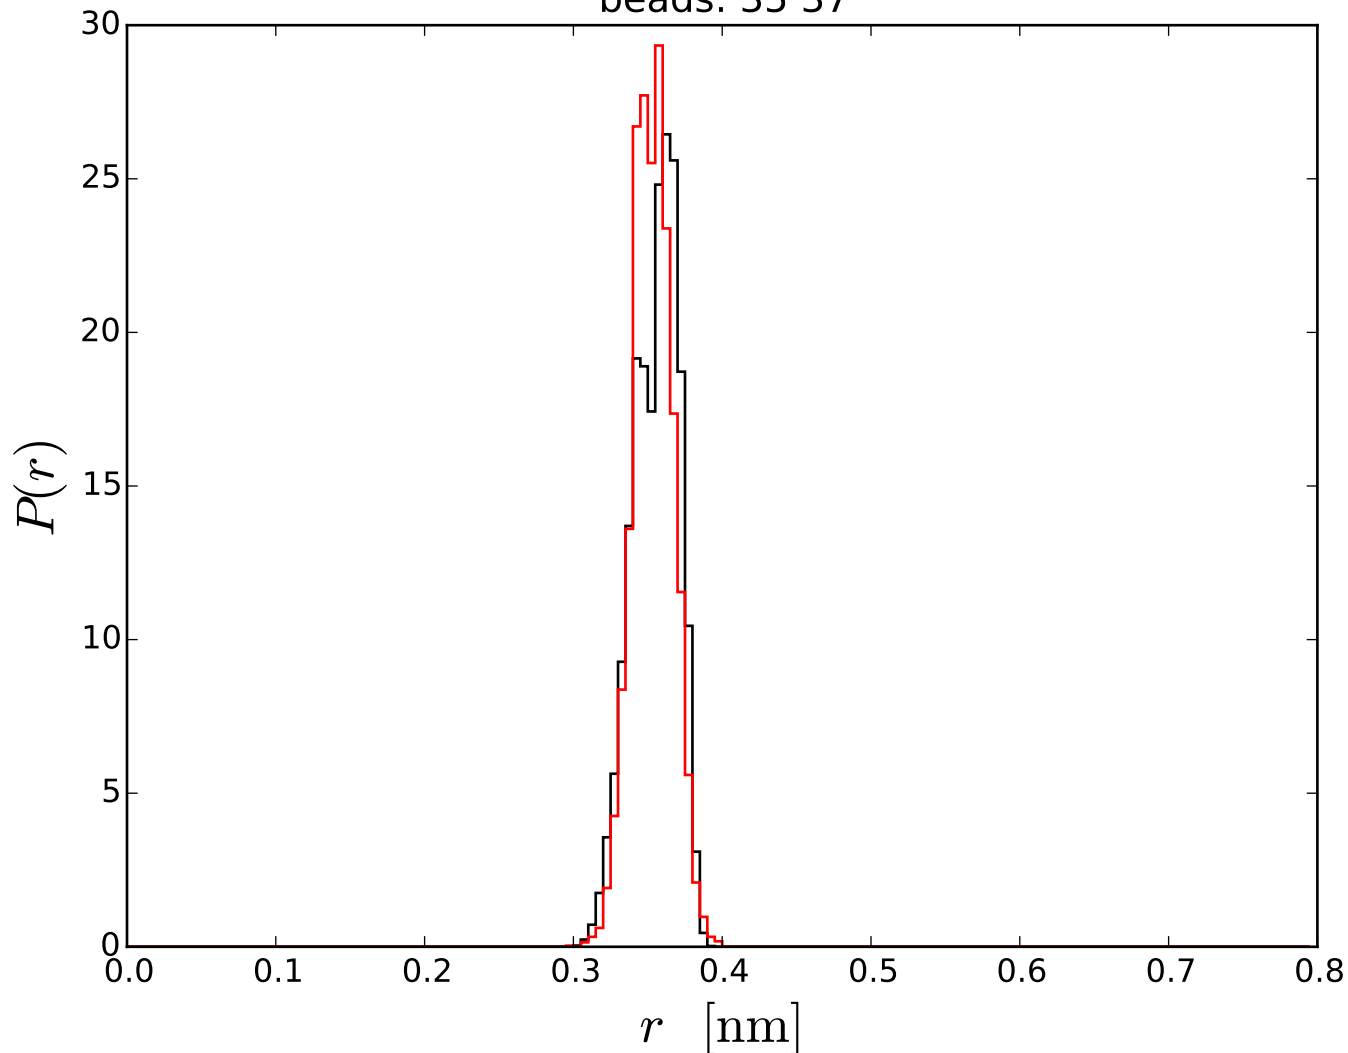

beads: 36 38

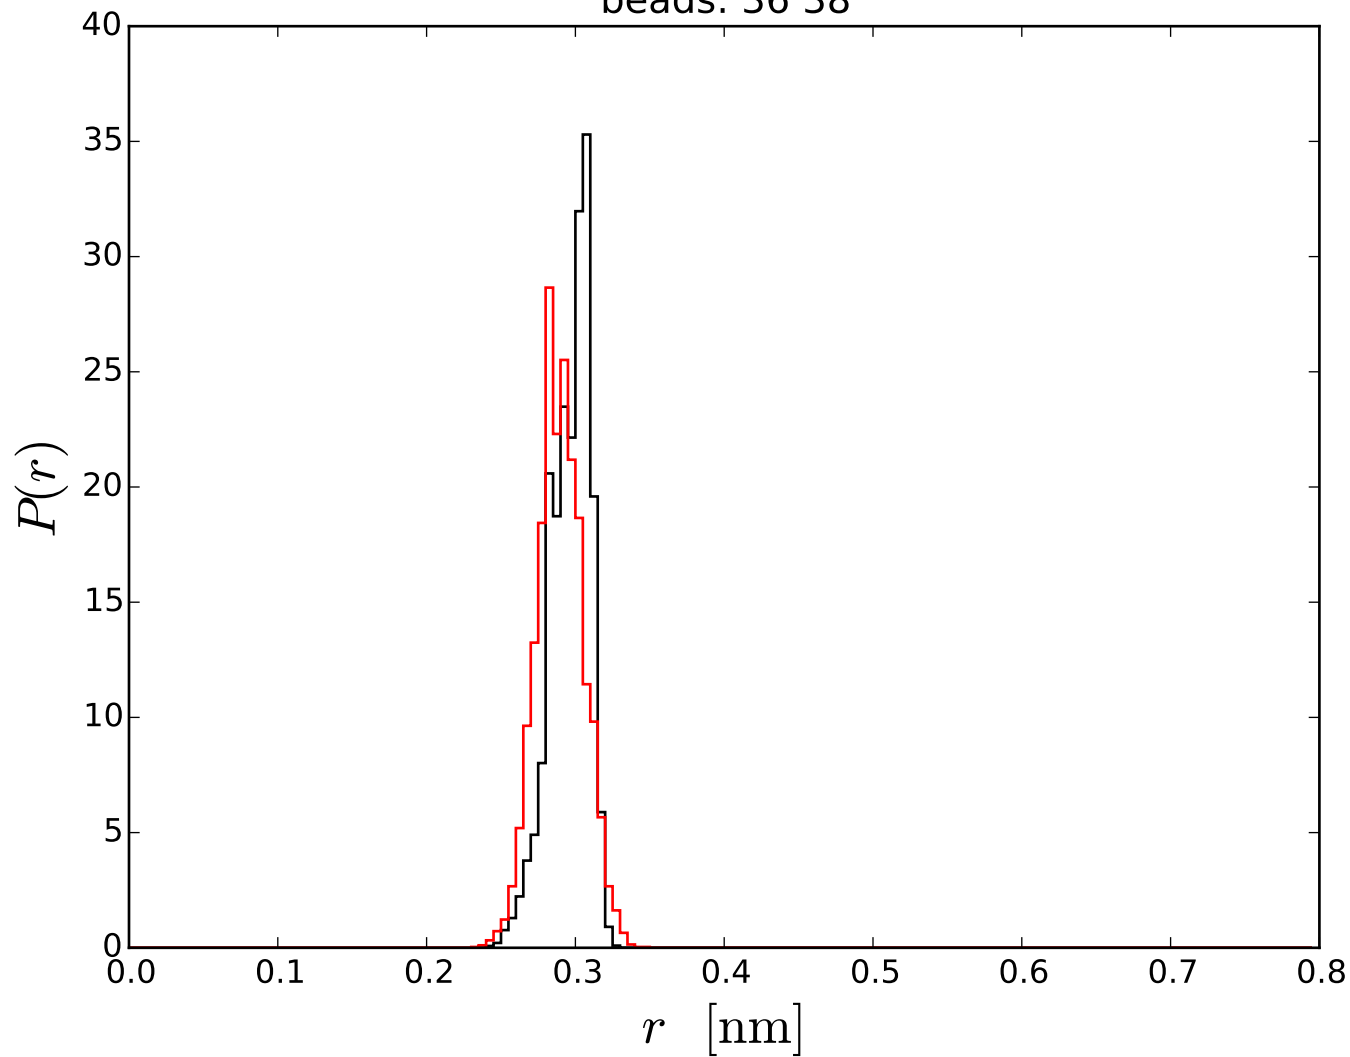

Supplement: Supplementary file 2 [file A2_bonds_AA_vs_MARTINI.pdf]
