# Supplementary material for: Overcoming the limitations of the MARTINI force field in Molecular Dynamics simulations of polysaccharides
Source: arXiv:1704.03773 ancillary file (2017-06-27)

beads: 7 5 3 2

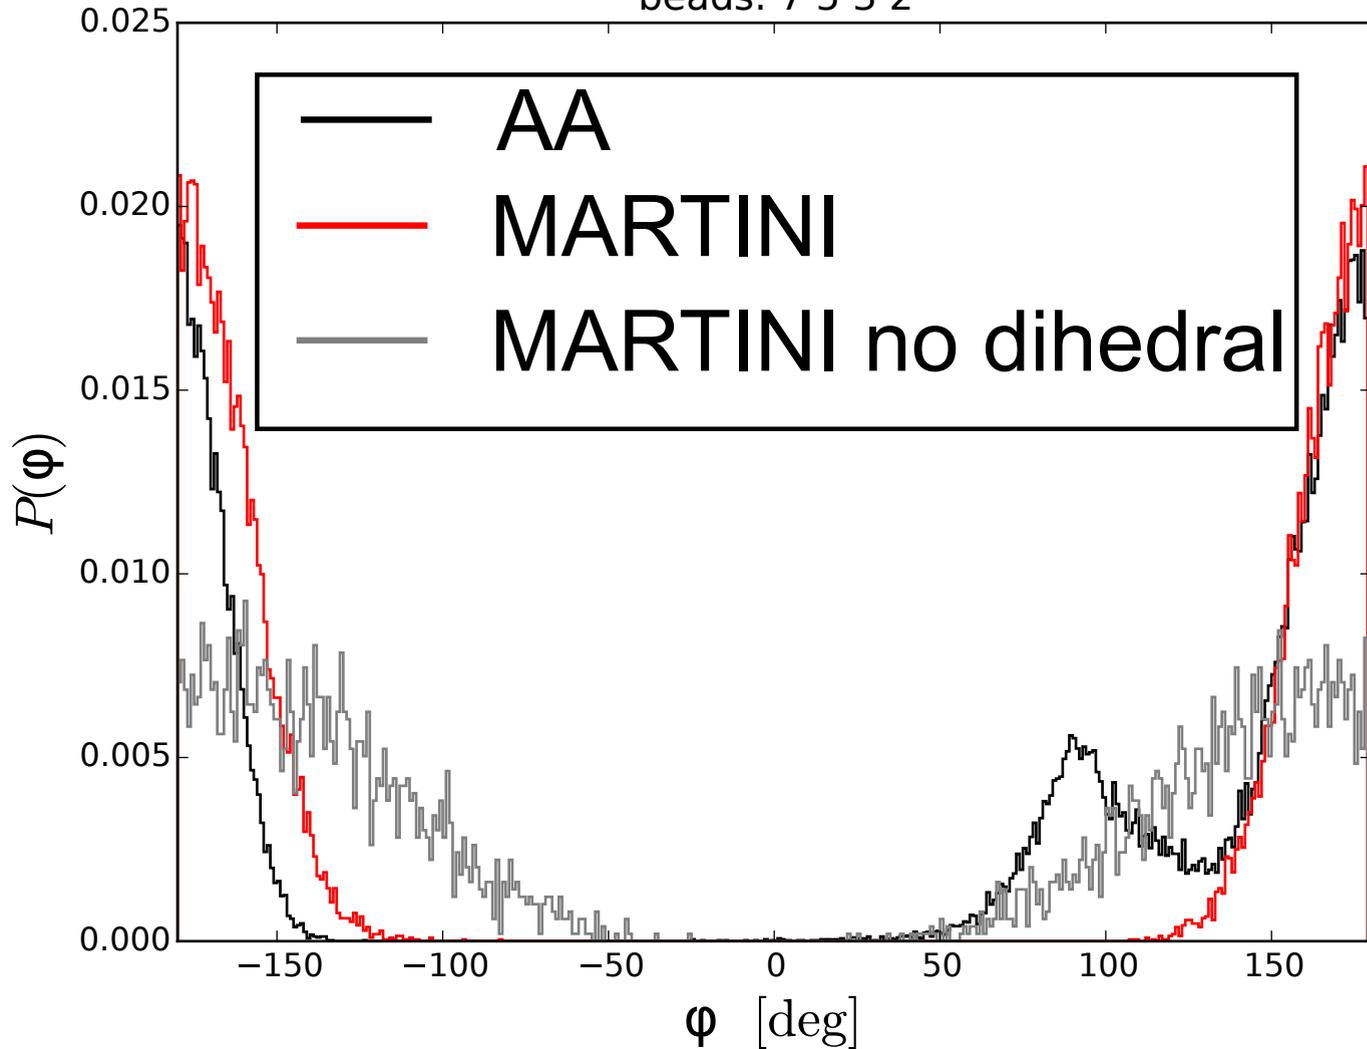

beads: 10 8 6 5

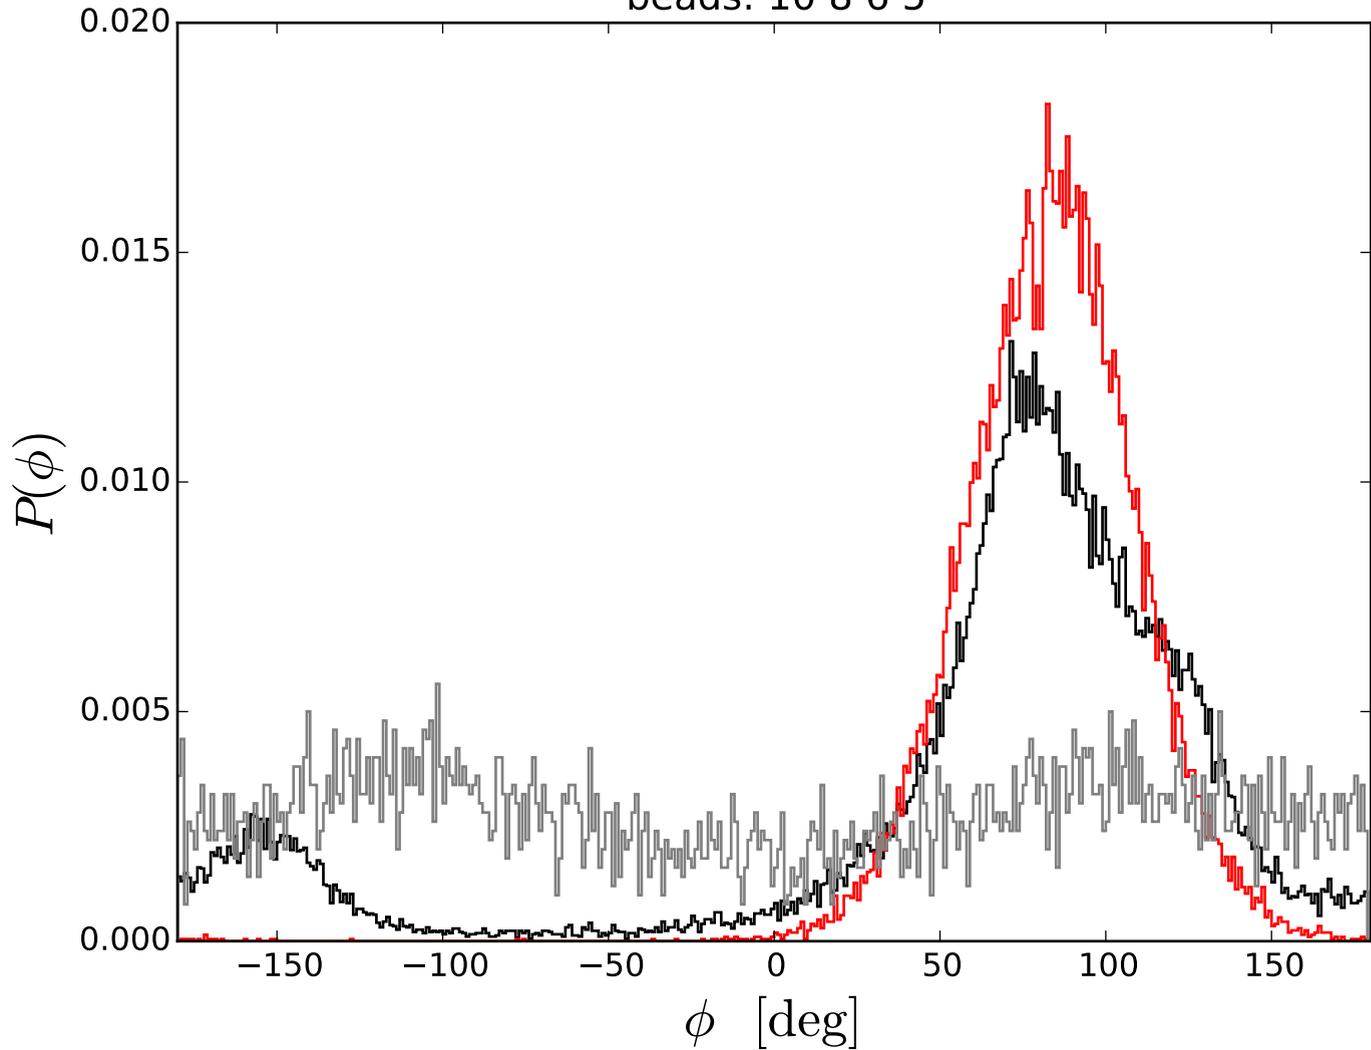

beads: 13 11 9 8

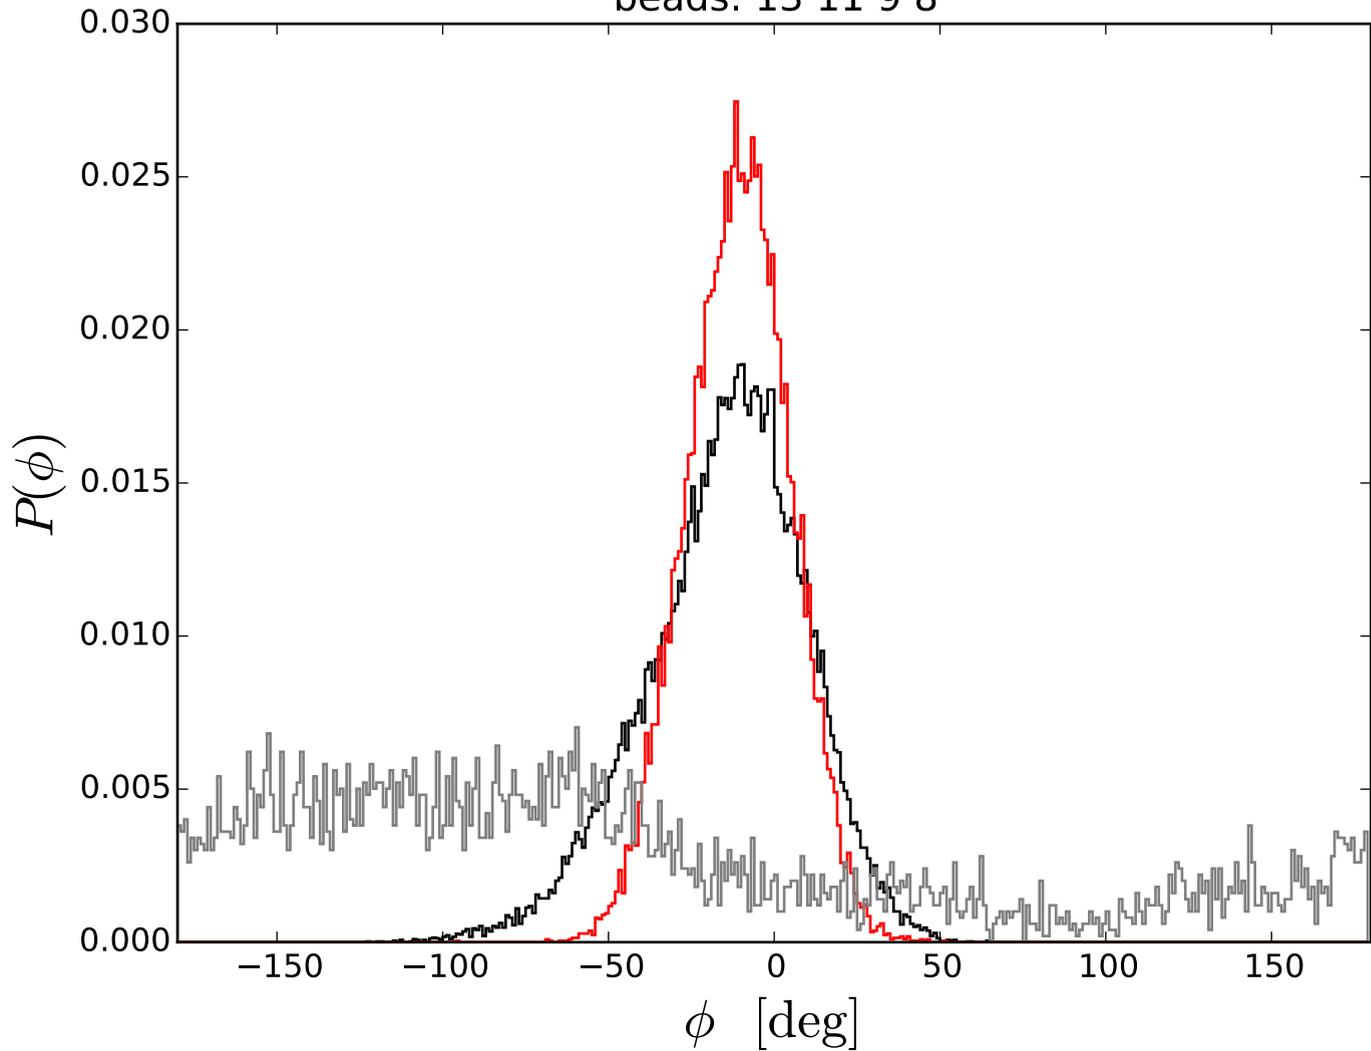

beads: 16 14 10 8

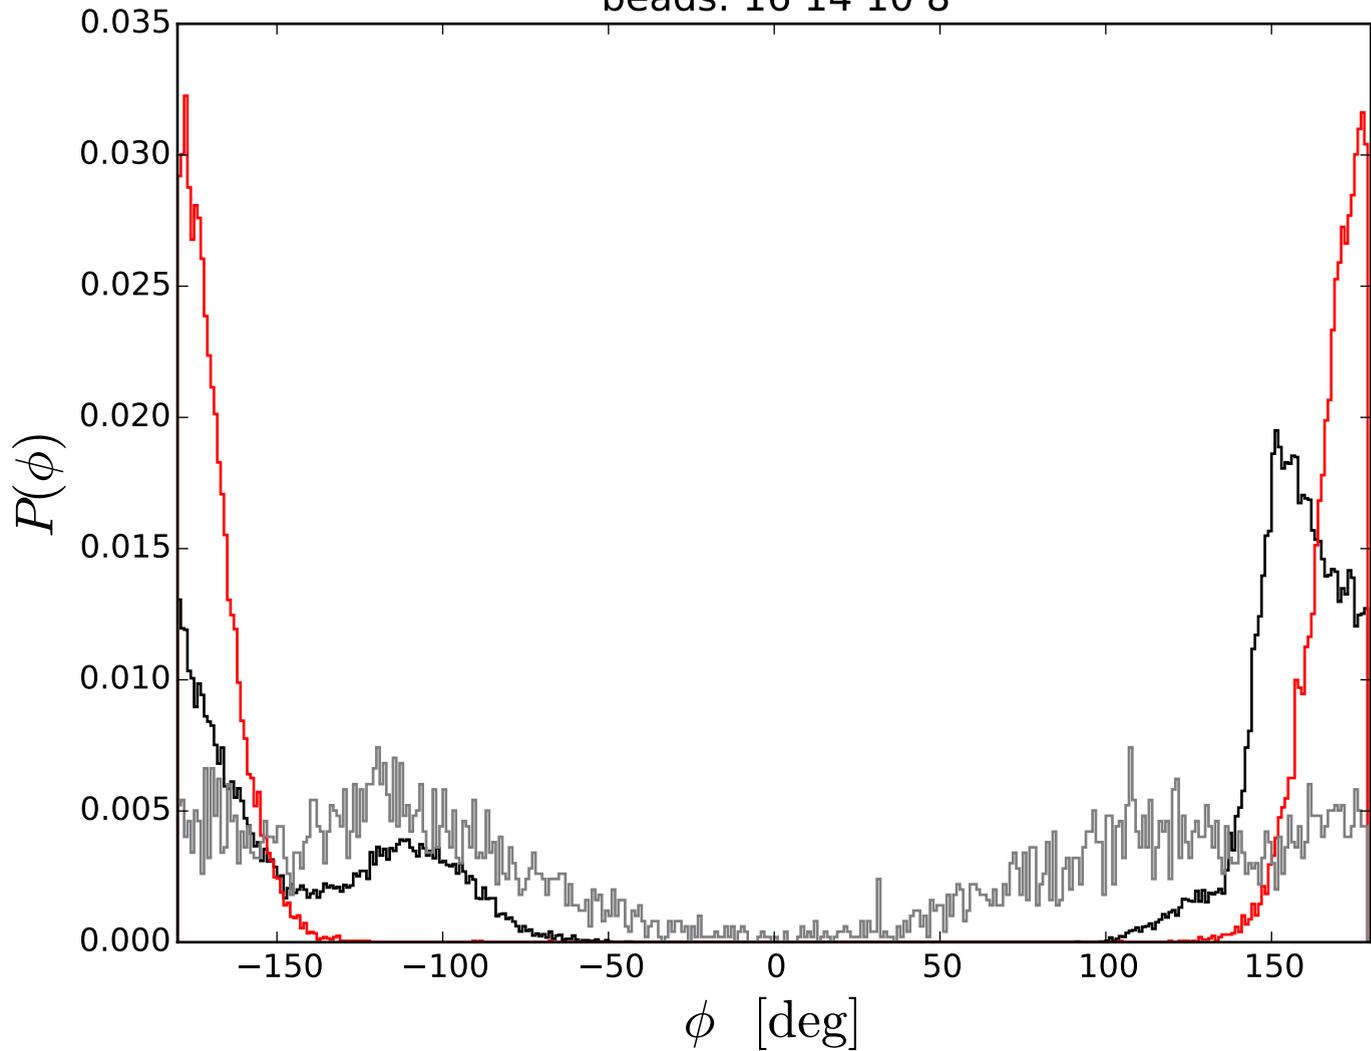

beads: 19 17 11 13

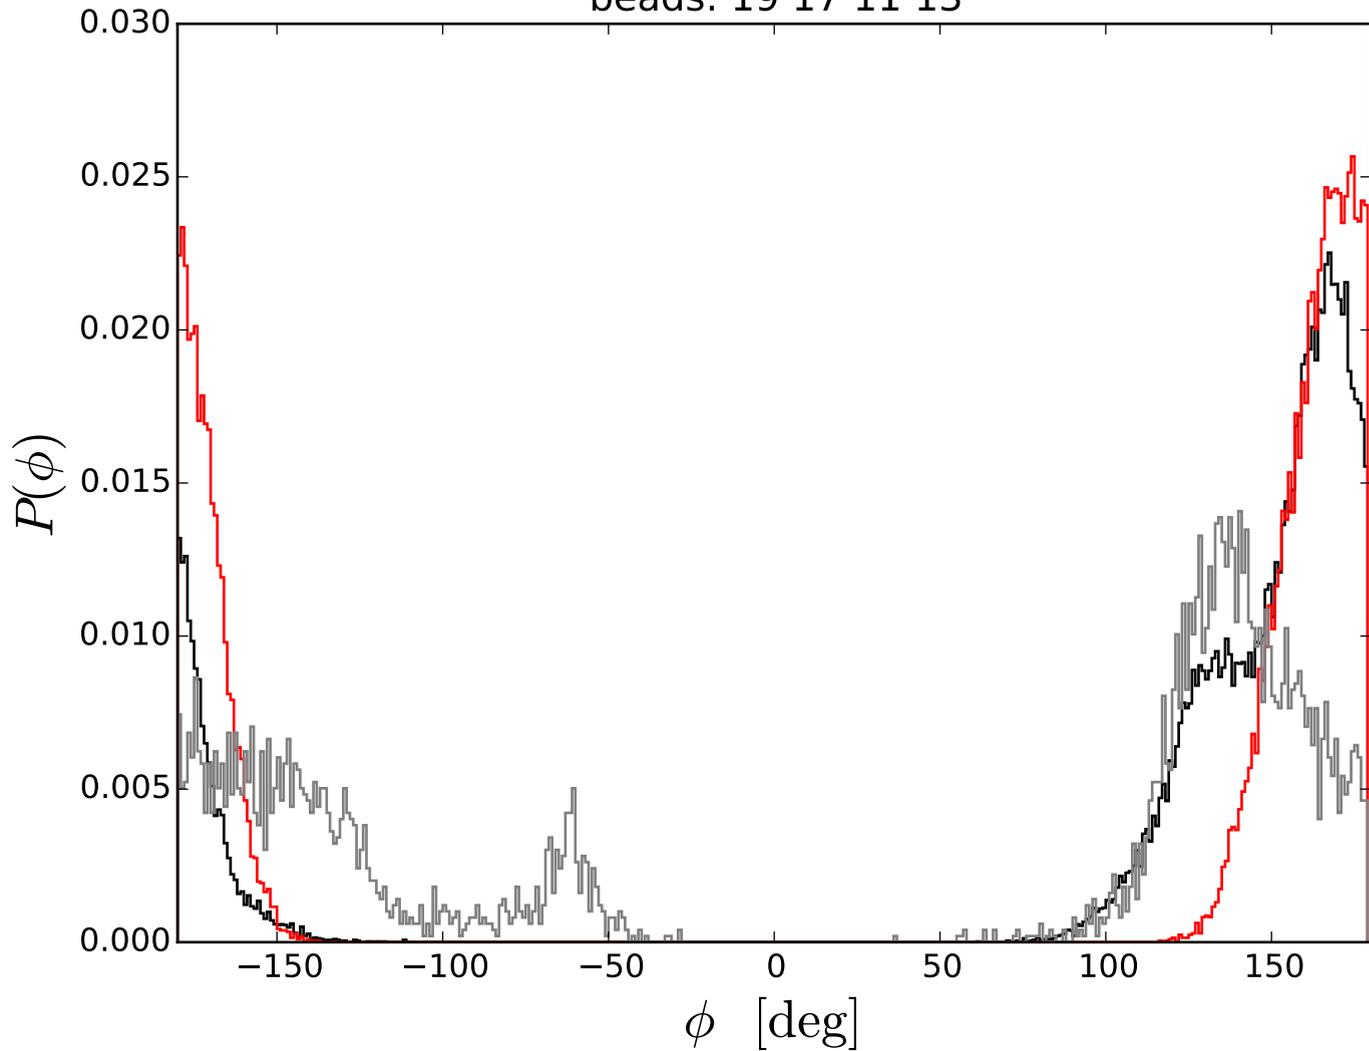

beads: 22 20 18 17

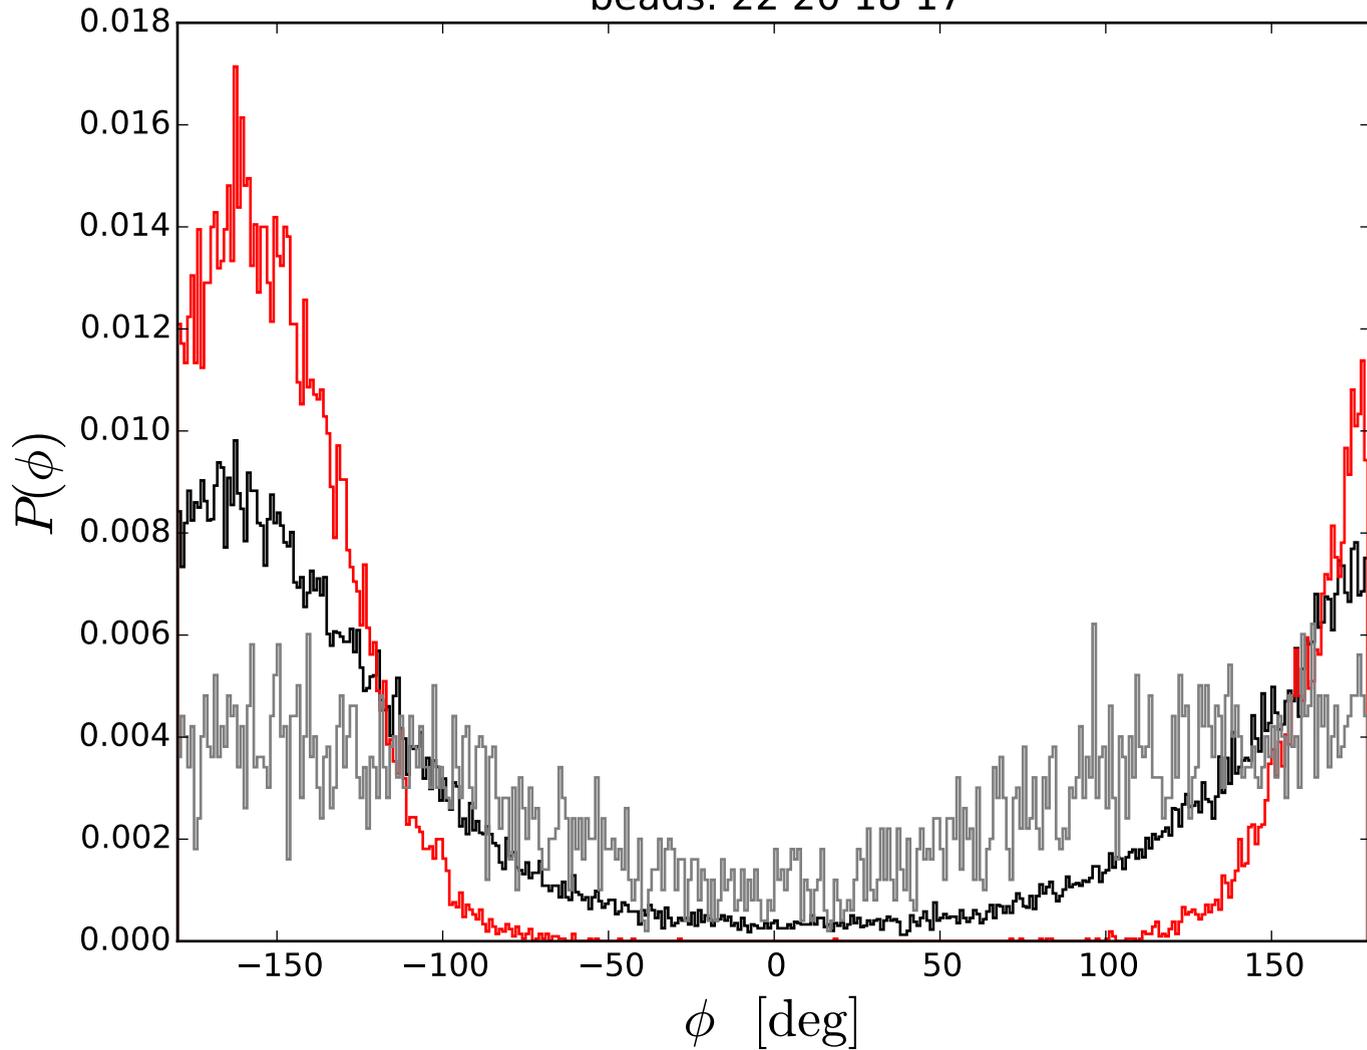

beads: 25 23 21 20

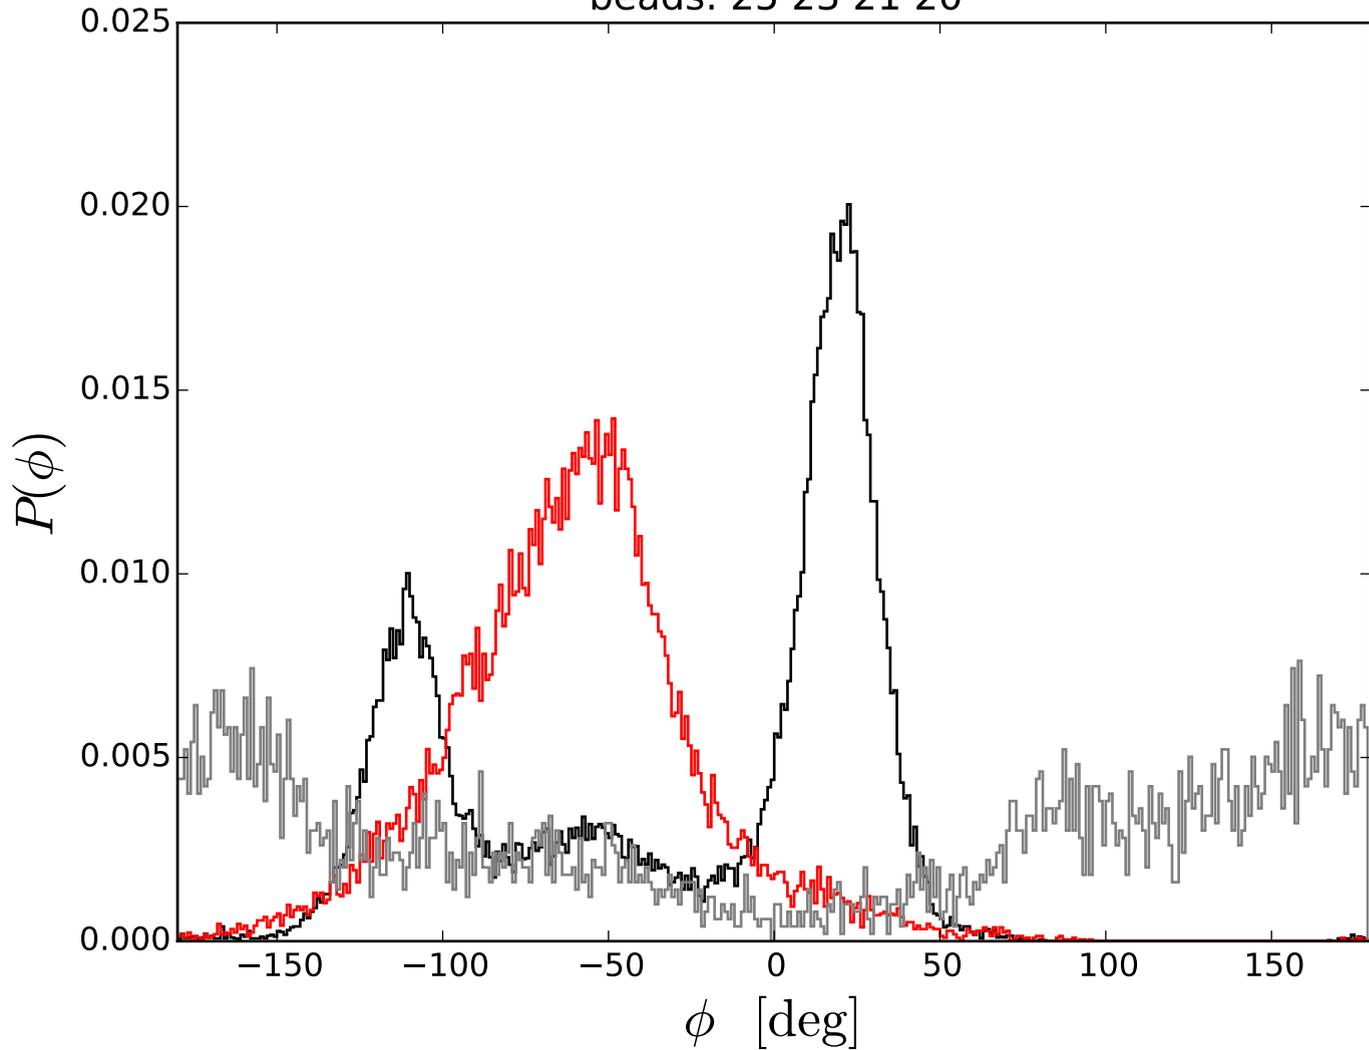

beads: 30 28 14 16

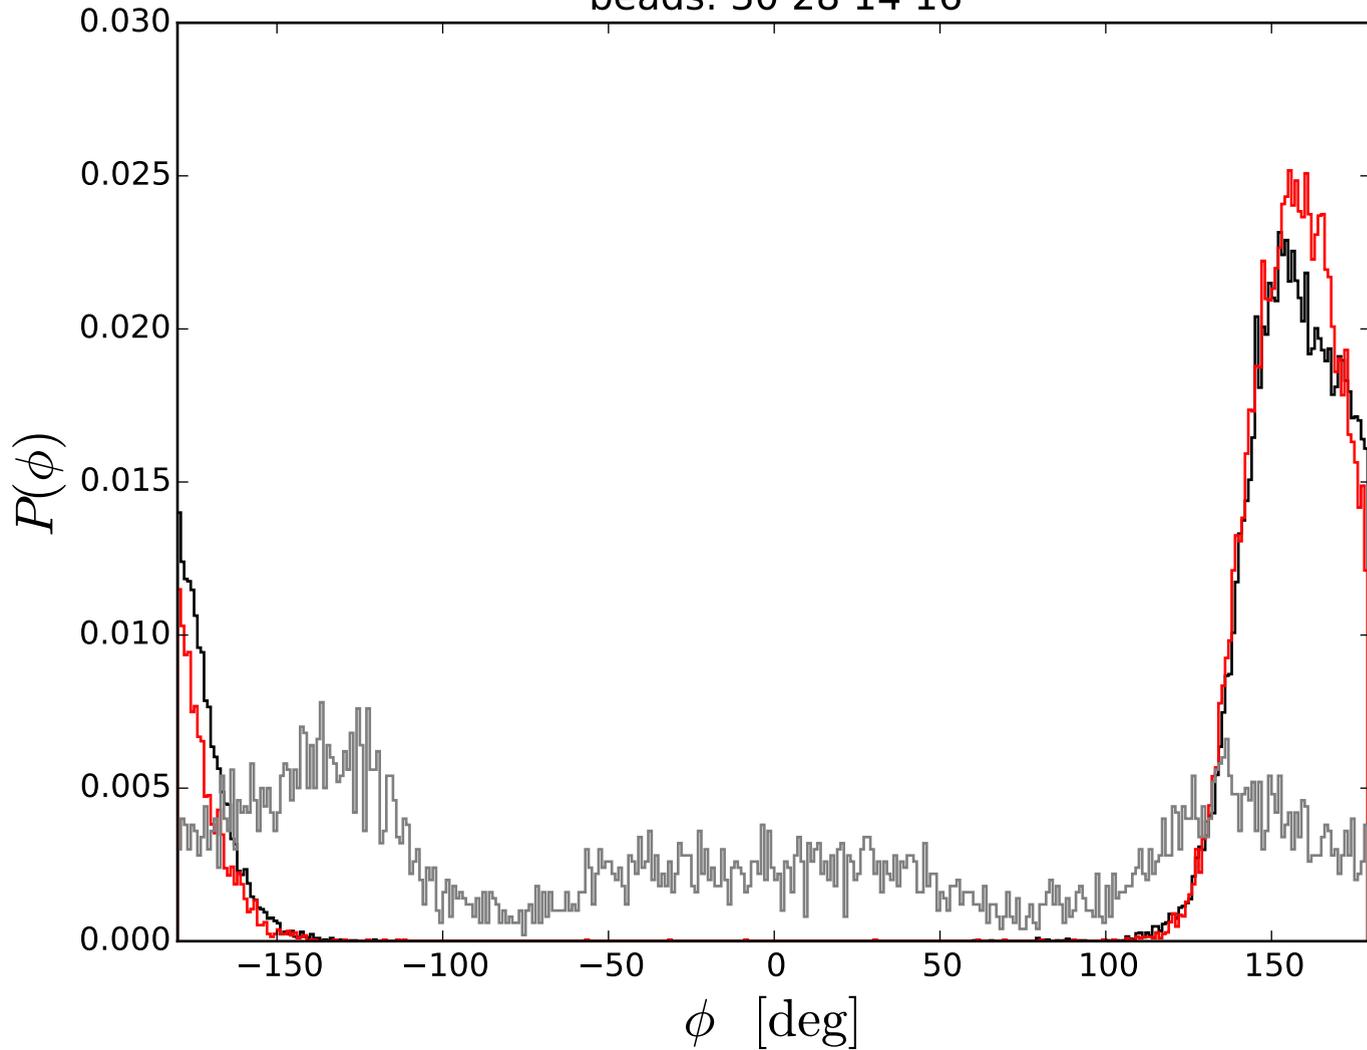

beads: 33 31 29 28

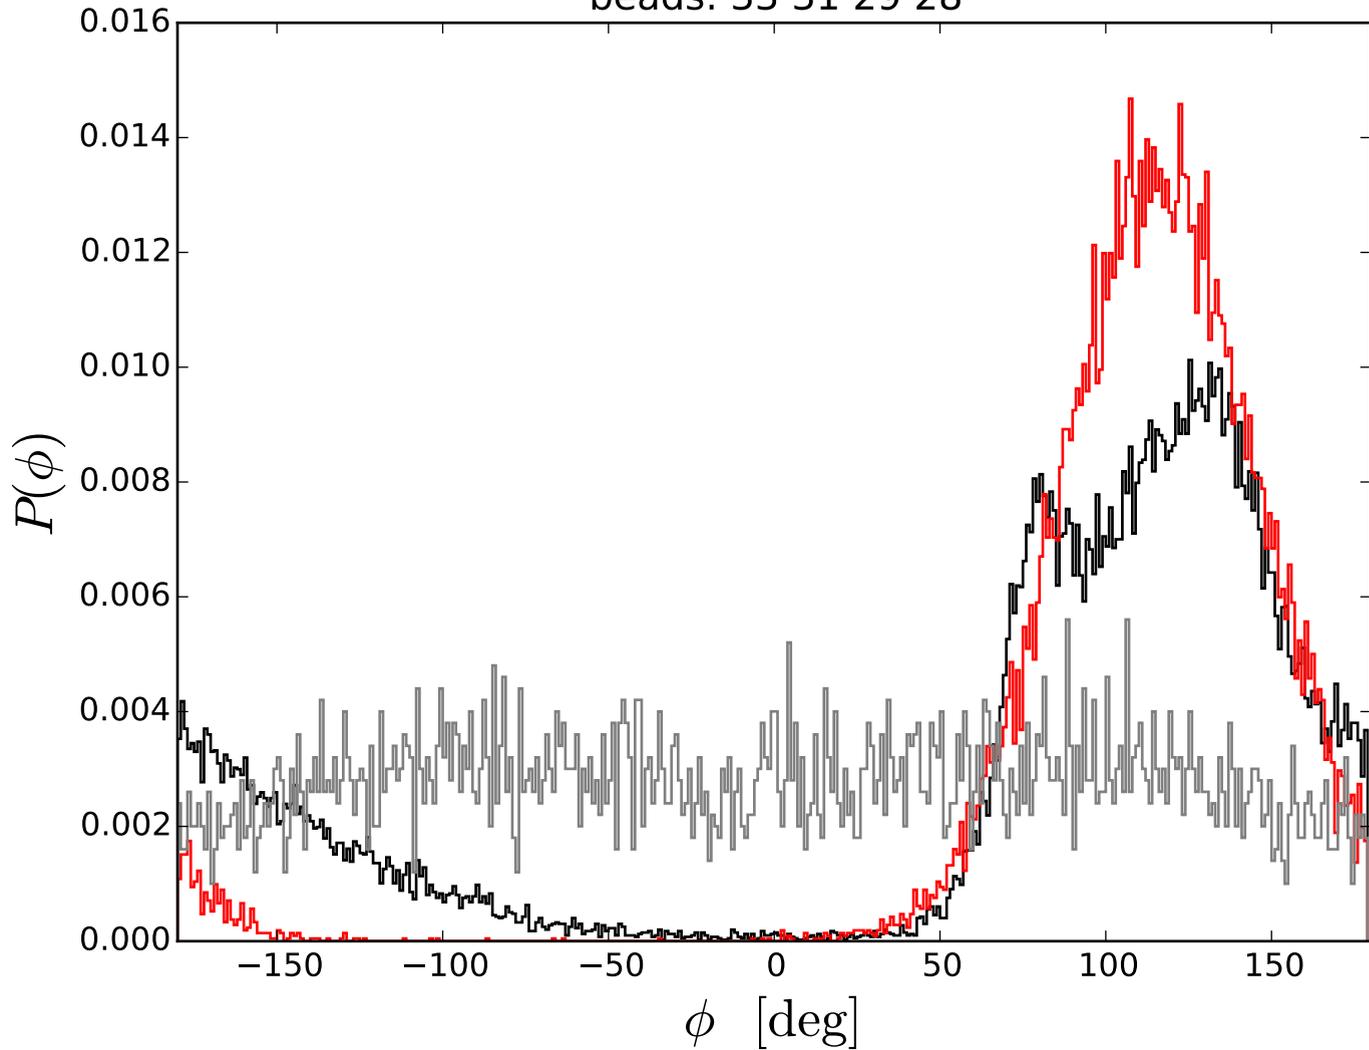

beads: 36 34 32 31

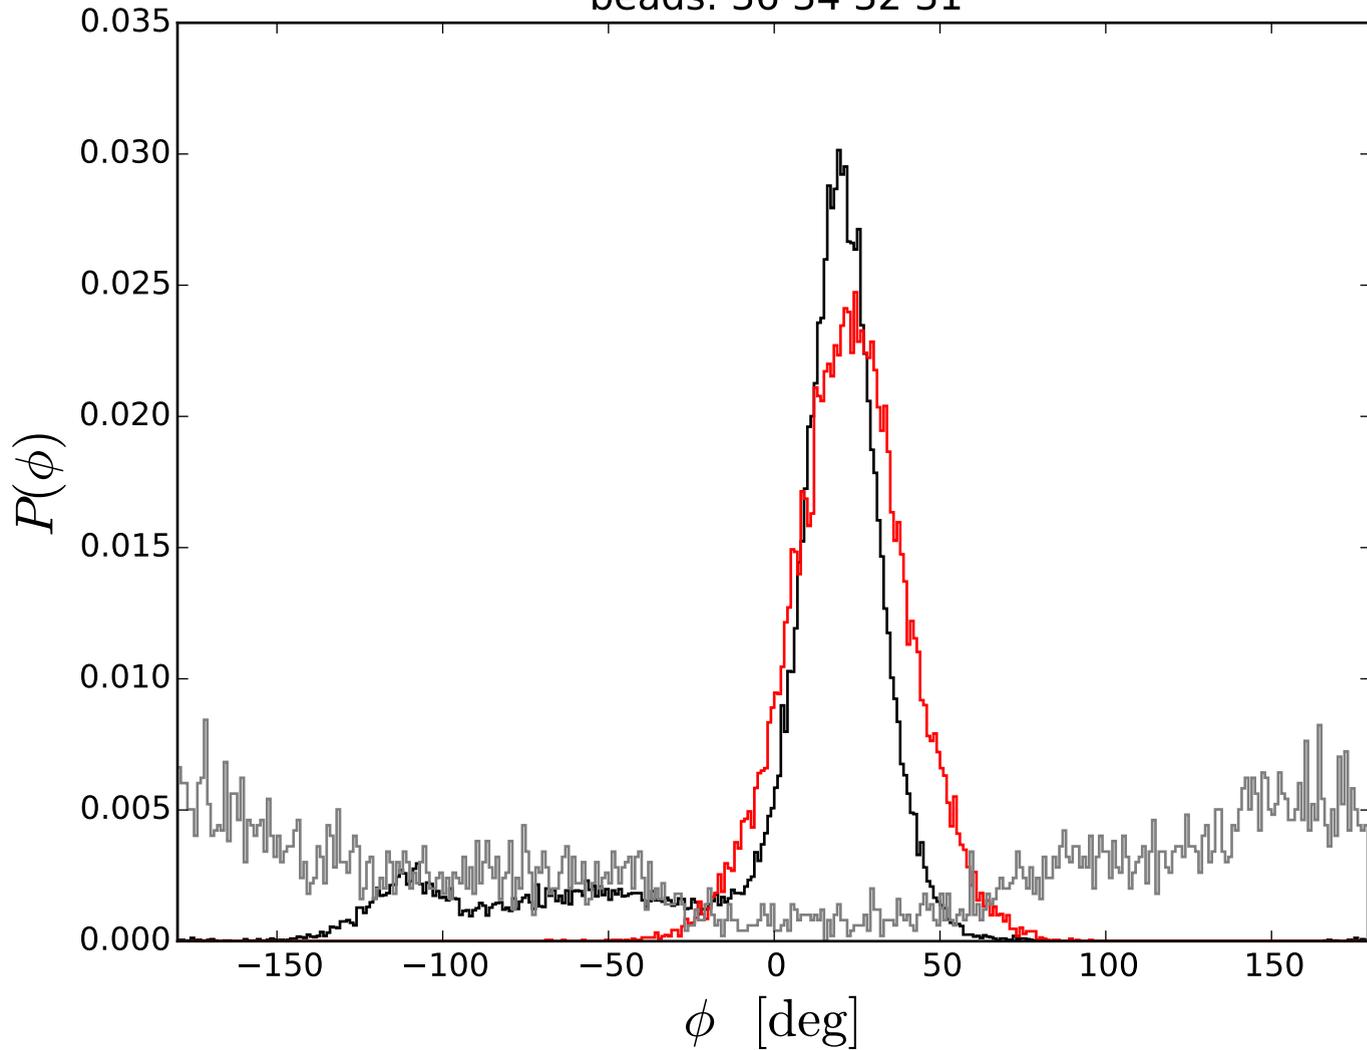

Supplement: Supplementary file 3 [file A2_dihedrals_AA_vs_MARTINI.pdf]
