# Supplementary material for: Overcoming the limitations of the MARTINI force field in Molecular Dynamics simulations of polysaccharides
Source: arXiv:1704.03773 ancillary file (2017-06-27)

beads: 1 2 5

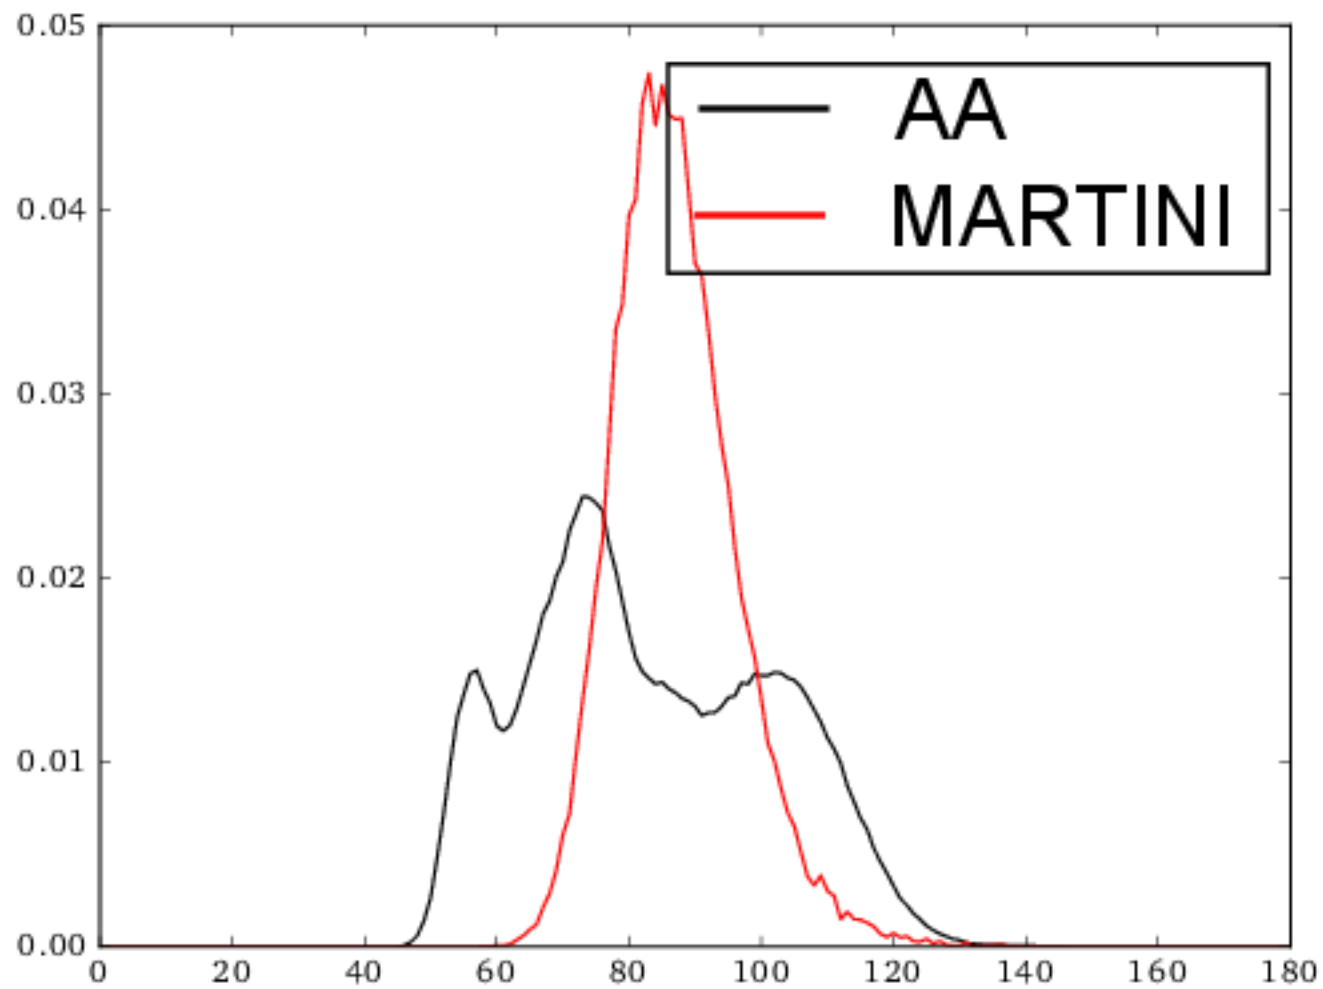

beads: 6 5 2

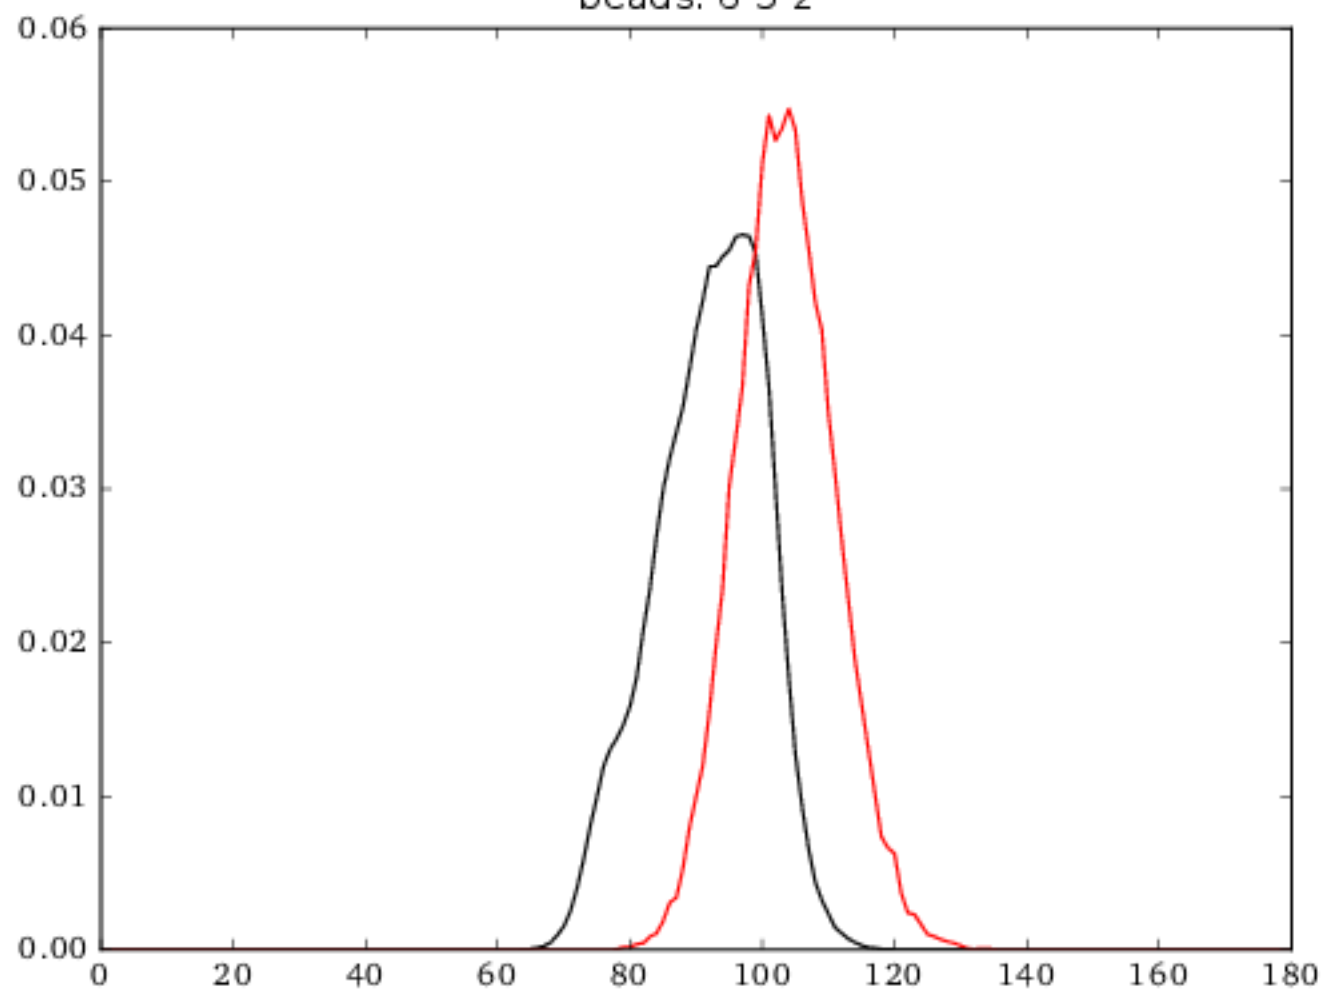

beads: 2 5 8

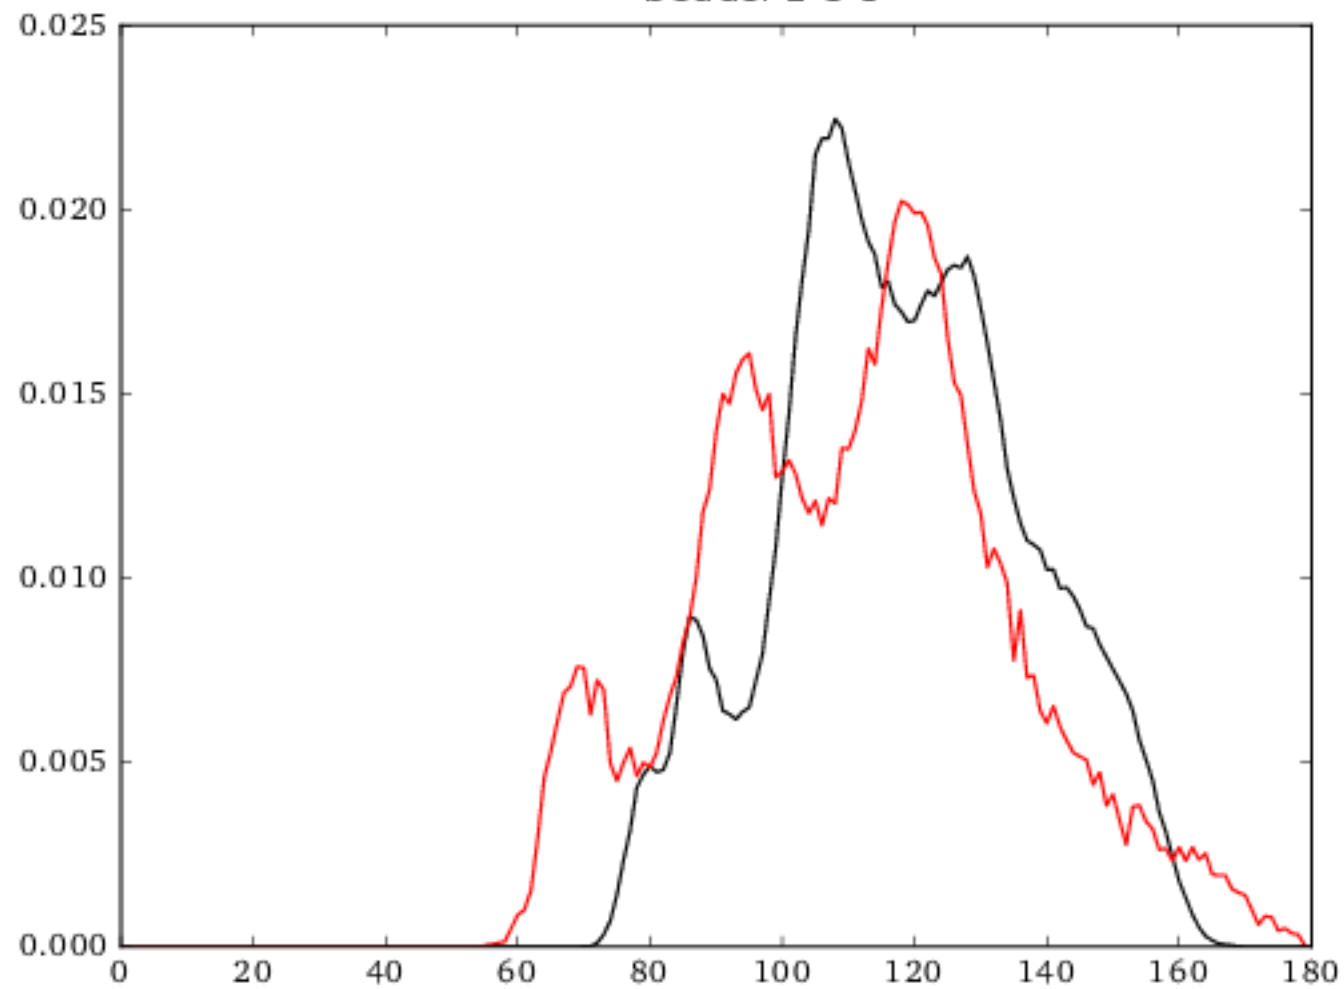

Supplement: Supplementary file 4 [file ACD_angles_AA_vs_MARTINI.pdf]
