# Supplementary material for: Overcoming the limitations of the MARTINI force field in Molecular Dynamics simulations of polysaccharides
Source: arXiv:1704.03773 ancillary file (2017-06-27)

beads: 1 2

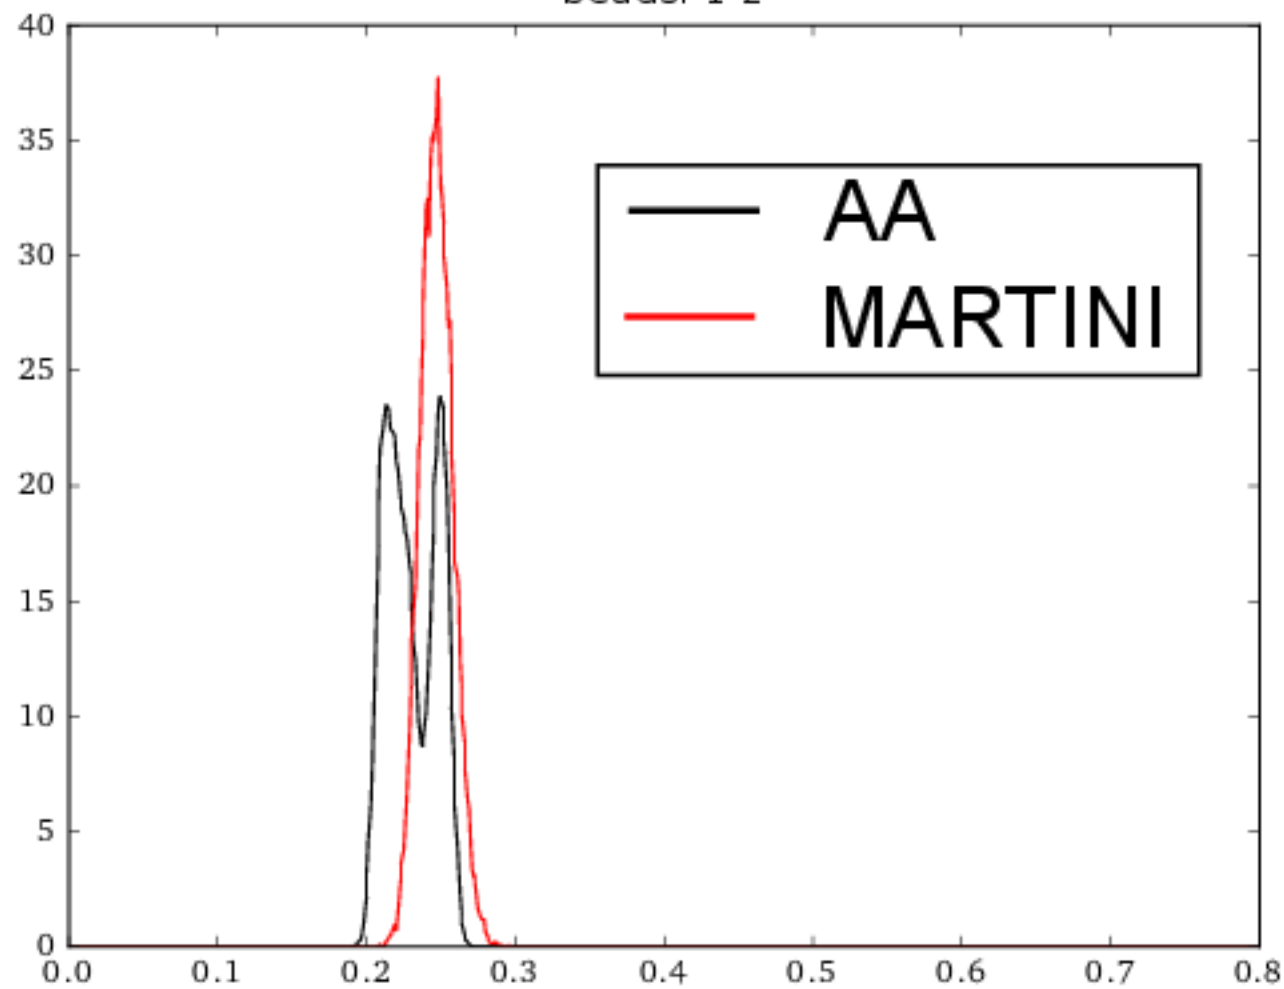

beads: 2 3

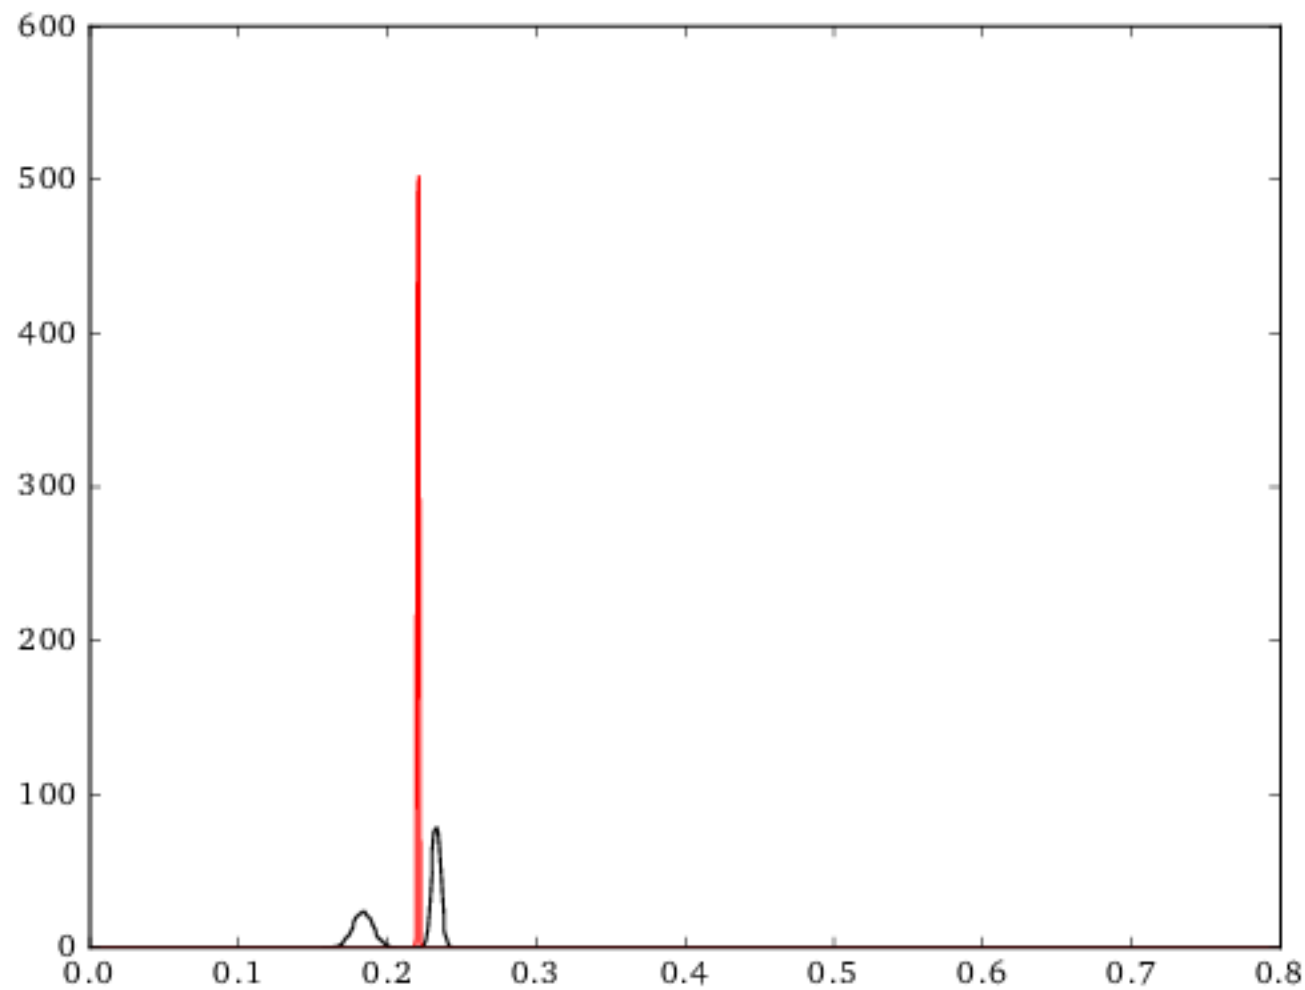

beads: 2 5

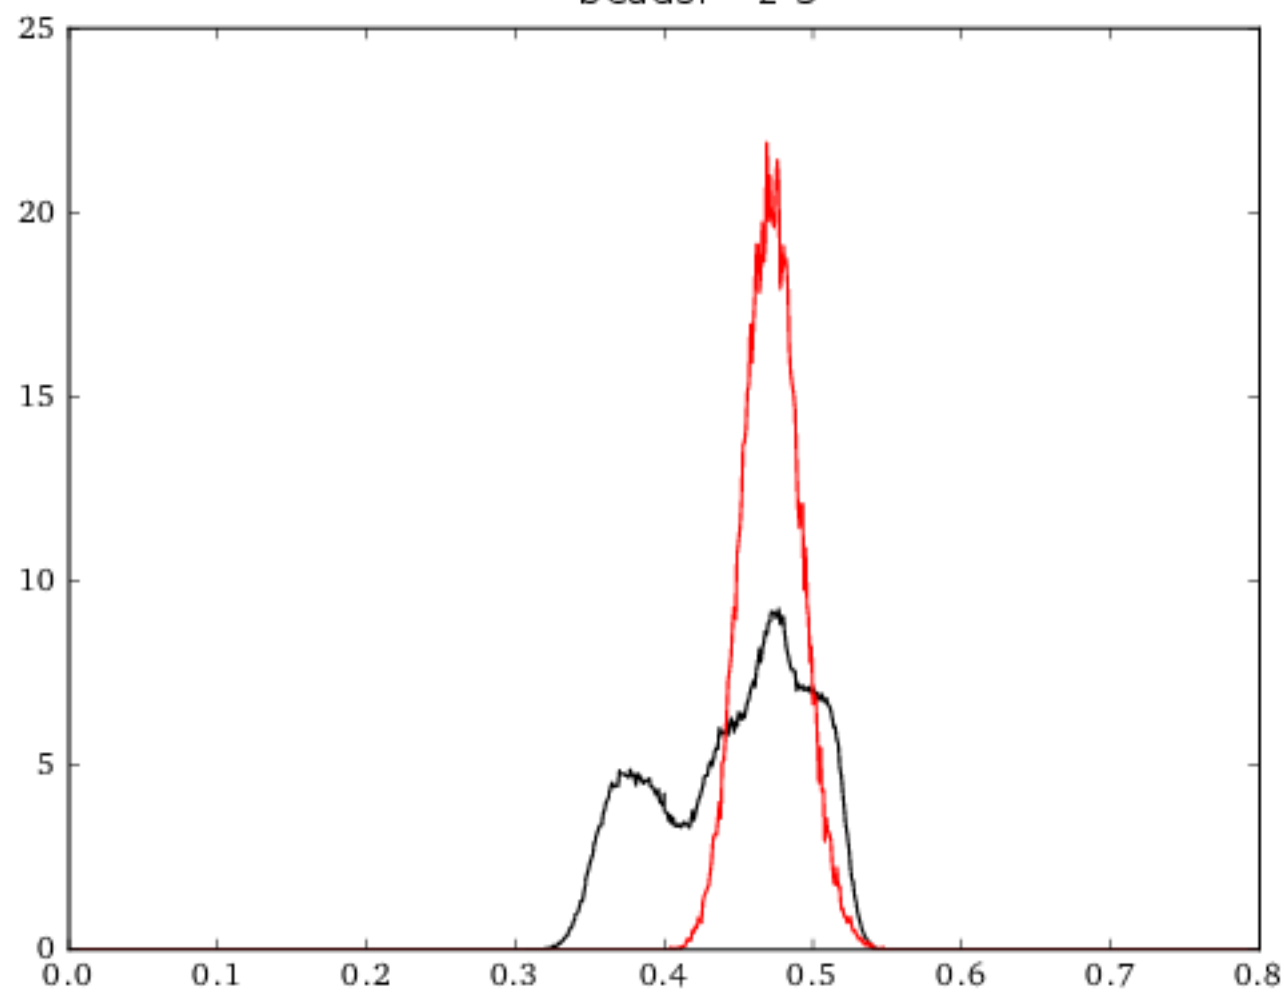

Supplement: Supplementary file 5 [file ACD_bonds_AA_vs_MARTINI.pdf]
